# Supplementary material for: Effective description of correlations for states obtained from conformal field theory
Source: arXiv:1706.03574 source file (2018-08-02)
Supplement: Supplementary file 1 [file Supplementary_Material_for_Effective_description_of_correlations_for_states_obtained_from_conformal_field_theory.pdf]

# Supplementary Material for:
# Effective description of correlations for states obtained from conformal field theory

Benedikt Herwerth[1], Germán Sierra[2],
J. Ignacio Cirac[1], Anne E.B. Nielsen[3,1,4]

[1]Max-Planck-Institut für Quantenoptik, Hans-Kopfermann-Straße 1, D-85748 Garching, Germany
[2]Instituto de Física Teórica, UAM-CSIC, Madrid, Spain
[3]Max-Planck-Institut für Physik komplexer Systeme, D-01187 Dresden, Germany
[4]Department of Physics and Astronomy, Aarhus University, DK-8000 Aarhus C, Denmark

The following pages contain plots of the correlations in the states $\psi_\alpha$ for 20 values of $\alpha$ between $0.025$ and $0.5$. For each value of $\alpha$, there is one plot on a separate page.

We consider three systems: $N = 100$ sites uniformly distributed on the circle, $N = 100$ sites with an approximately uniform distribution on the sphere, and a cylinder with $N_y = 160$ sites in the periodical direction. For the continuum approximation, the cylinder is half infinite ($N_x = \infty$) while it has $N_x = 14$ sites otherwise.

The data in continuum approximation was computed according to the expressions given in the second column of Tab. I of the main text. The expression for the cylinder contains an infinite Fourier sum, which we truncated to some cutoff momentum. We then applied a fast Fourier transform to the resulting finite sum, repeated the computation with increasing cutoff momenta, and extrapolated to the case of an infinite cutoff.

Monte Carlo data are plotted with error bars. In the other cases, we determined an estimate of the numerical error. Whenever this estimated error is larger than $1\%$ of the corresponding value, the data point is plotted in gray.

I. Circle

II. Sphere

III. Cylinder (edge)

IV. Cylinder (bulk)

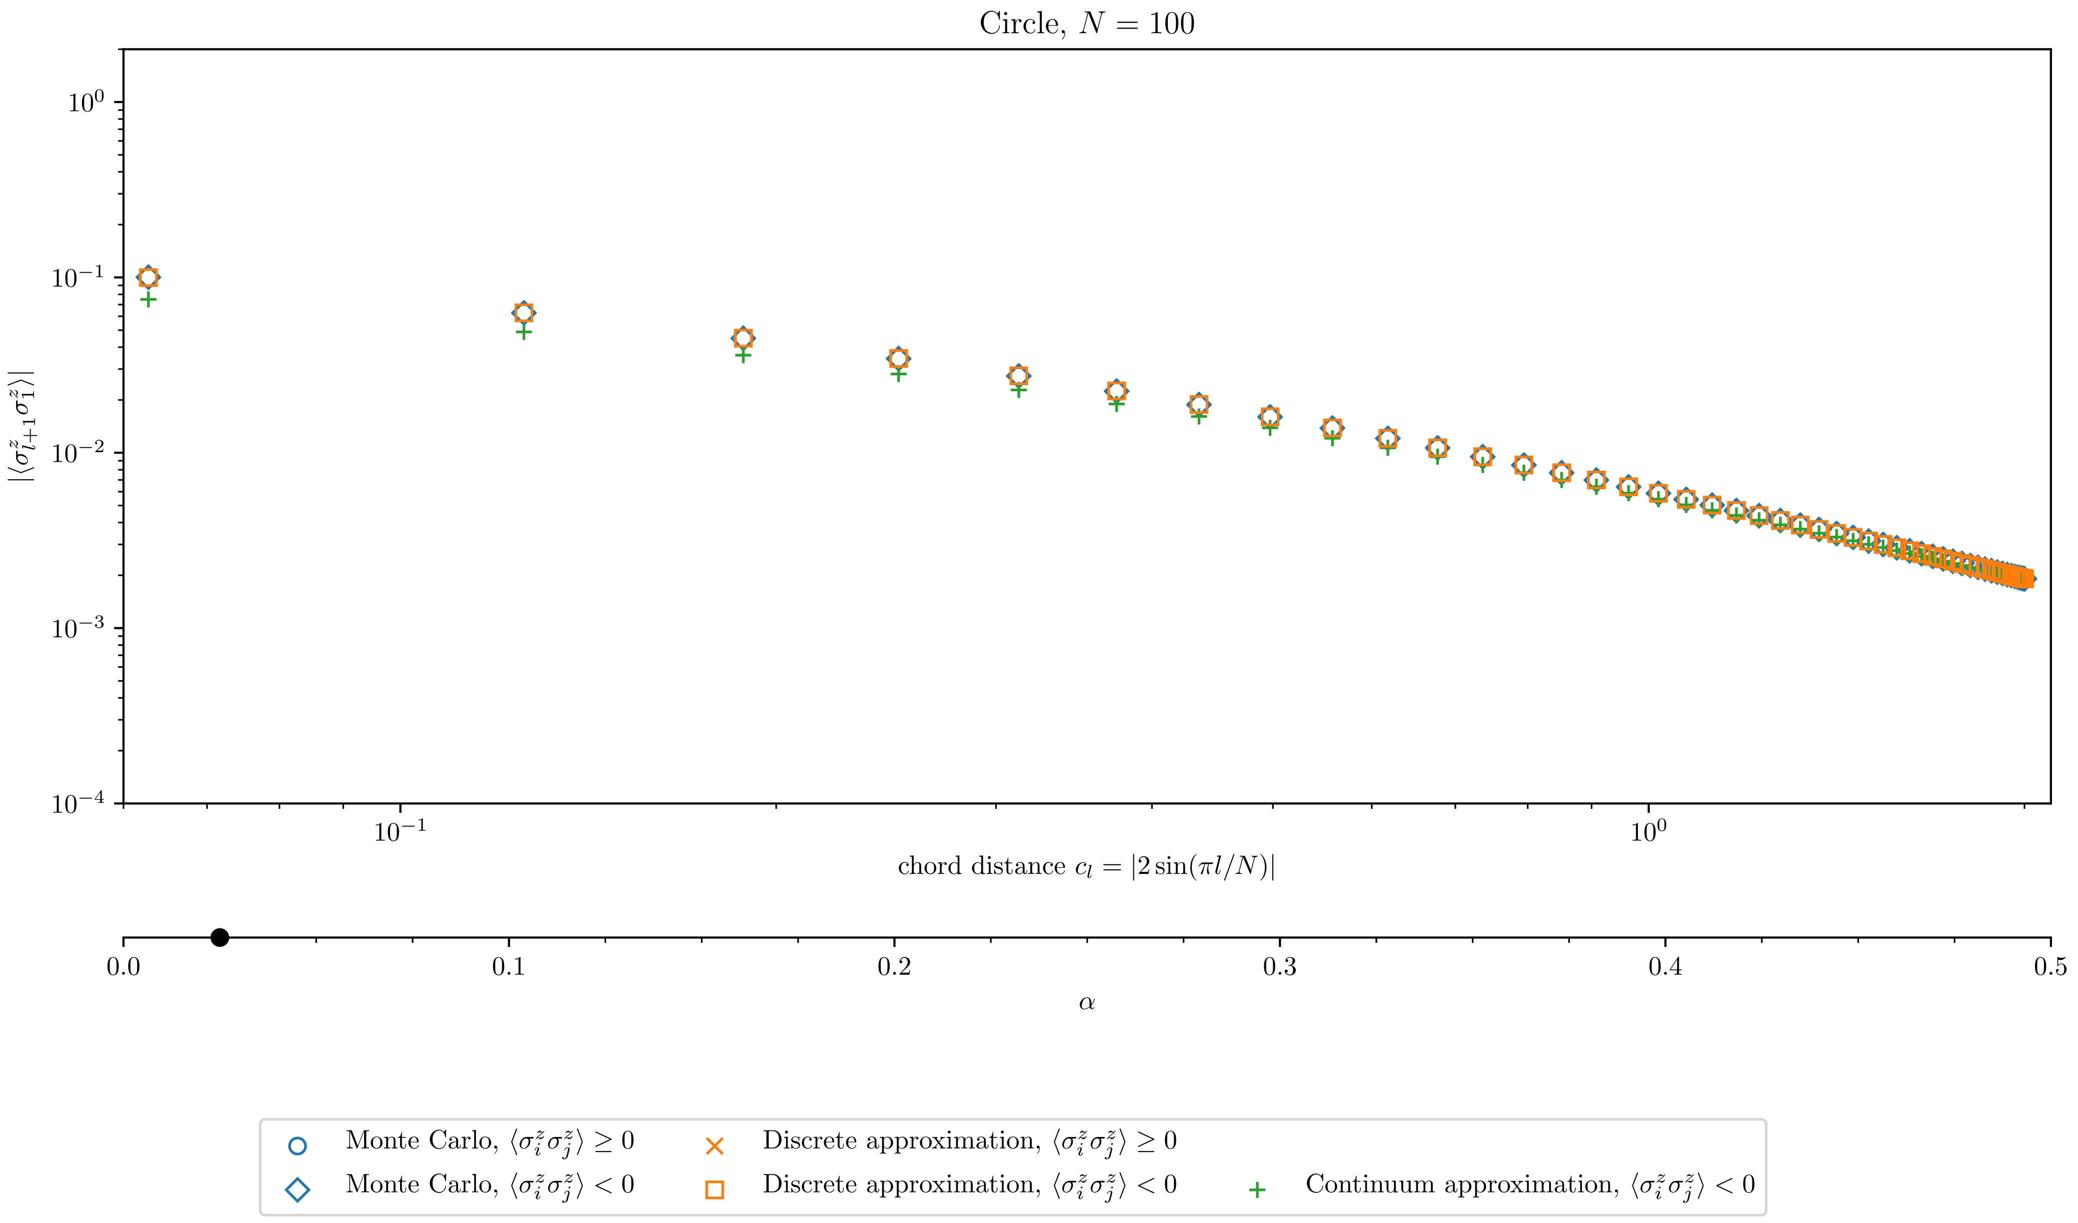

Circle, $N = 100$
$|\langle\sigma^z_{l+1}\sigma^z_1\rangle|$
$10^0$
$10^{-1}$
$10^{-2}$
$10^{-3}$
$10^{-4}$
$10^{-1}$
$10^0$
chord distance $c_l = |2\sin(\pi l/N)|$
0.0
0.1
0.2
0.3
0.4
0.5
$\alpha$
Monte Carlo, $\langle\sigma^z_i\sigma^z_j\rangle \geq 0$
Monte Carlo, $\langle\sigma^z_i\sigma^z_j\rangle < 0$
Discrete approximation, $\langle\sigma^z_i\sigma^z_j\rangle \geq 0$
Discrete approximation, $\langle\sigma^z_i\sigma^z_j\rangle < 0$
Continuum approximation, $\langle\sigma^z_i\sigma^z_j\rangle < 0$

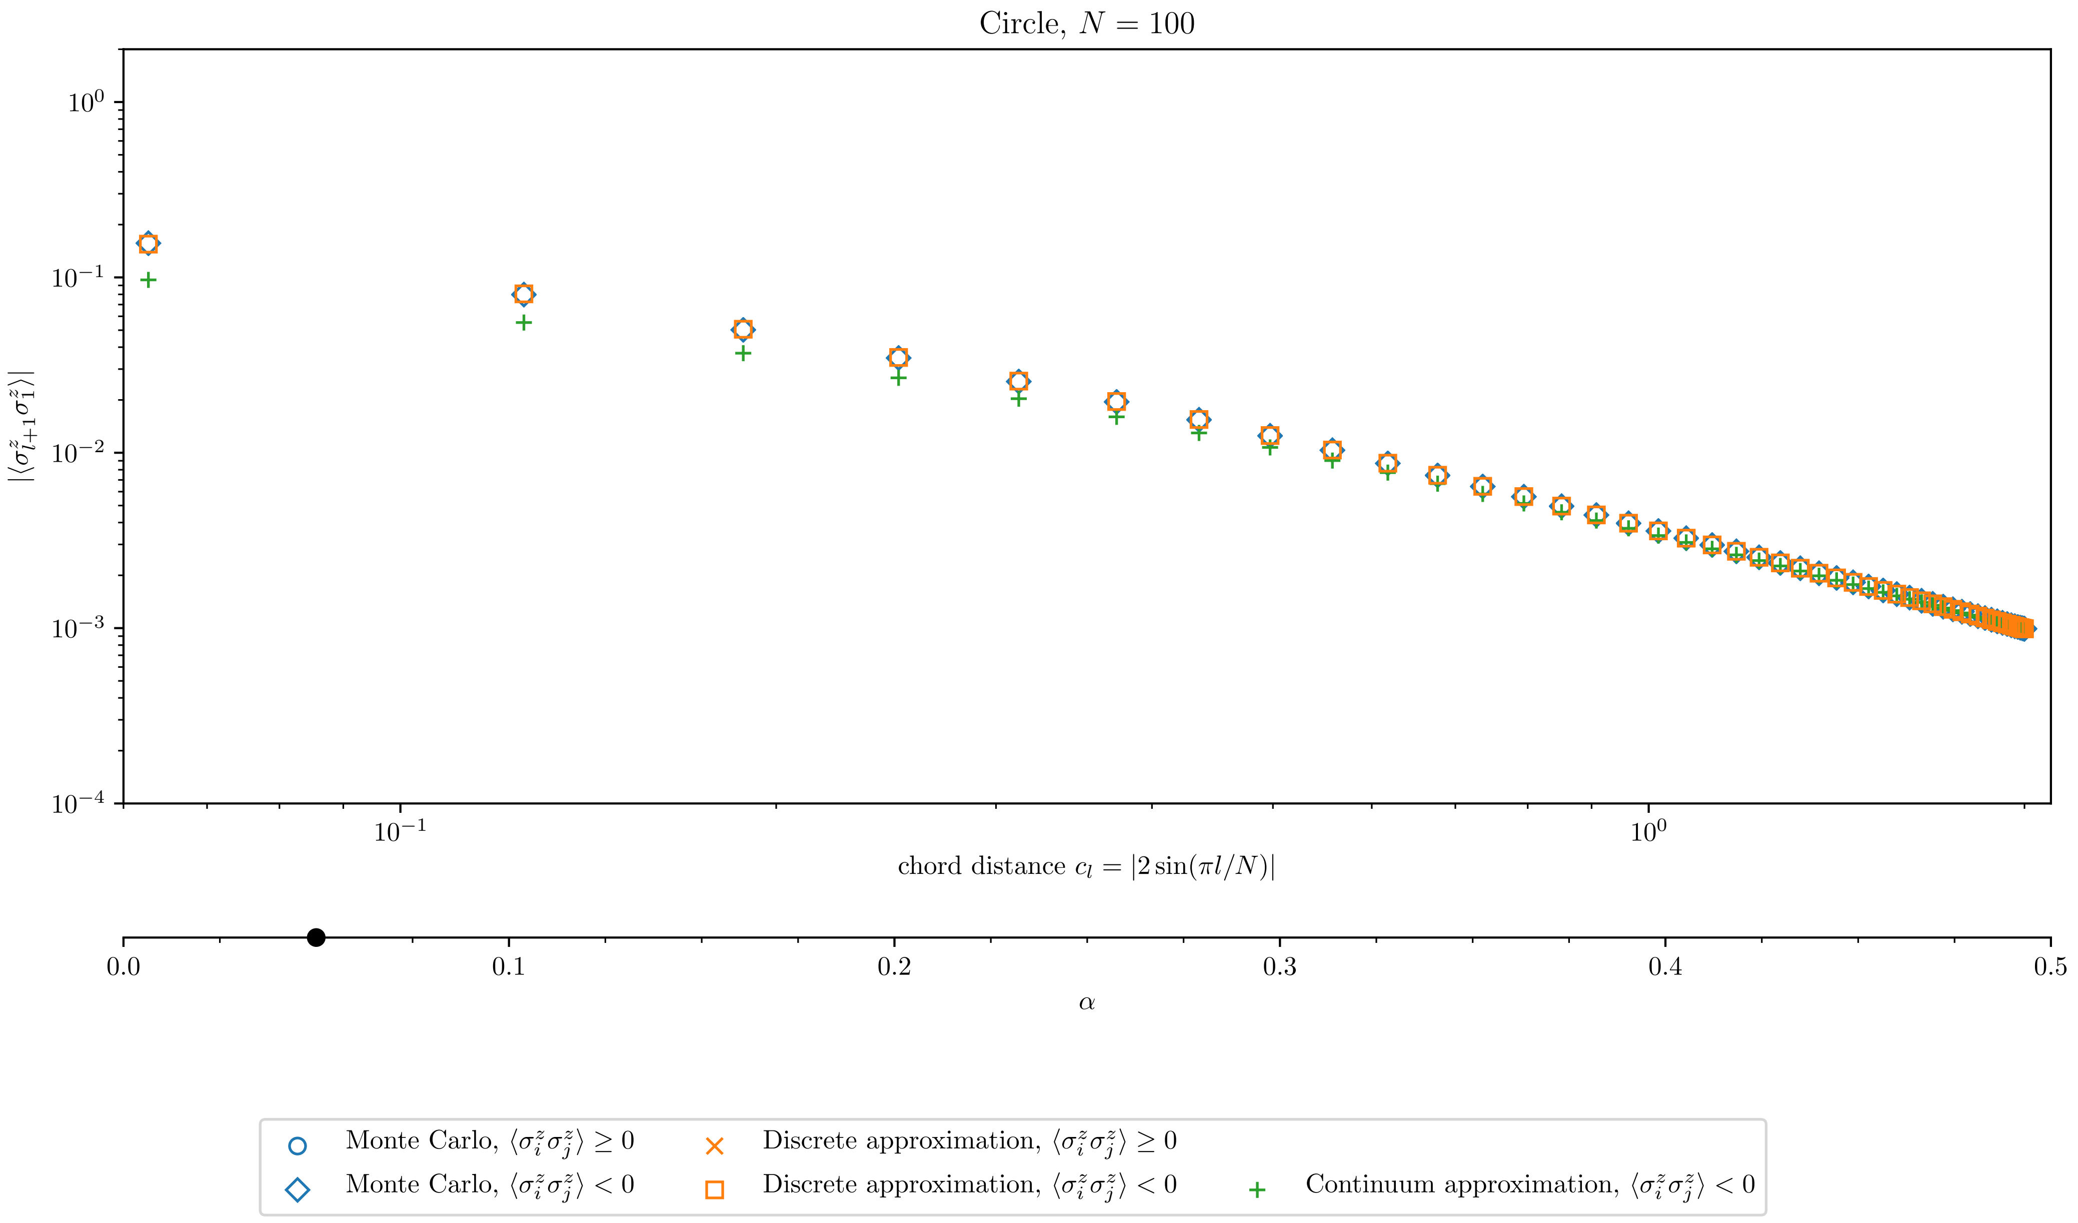

Circle, $N = 100$
$|\langle \sigma^z_{l+1} \sigma^z_1 \rangle|$
$10^0$
$10^{-1}$
$10^{-2}$
$10^{-3}$
$10^{-4}$
$10^{-1}$
$10^0$
chord distance $c_l = |2\sin(\pi l/N)|$
0.0
0.1
0.2
0.3
0.4
0.5
$\alpha$
Monte Carlo, $\langle \sigma^z_i \sigma^z_j \rangle \geq 0$
Monte Carlo, $\langle \sigma^z_i \sigma^z_j \rangle < 0$
Discrete approximation, $\langle \sigma^z_i \sigma^z_j \rangle \geq 0$
Discrete approximation, $\langle \sigma^z_i \sigma^z_j \rangle < 0$
Continuum approximation, $\langle \sigma^z_i \sigma^z_j \rangle < 0$

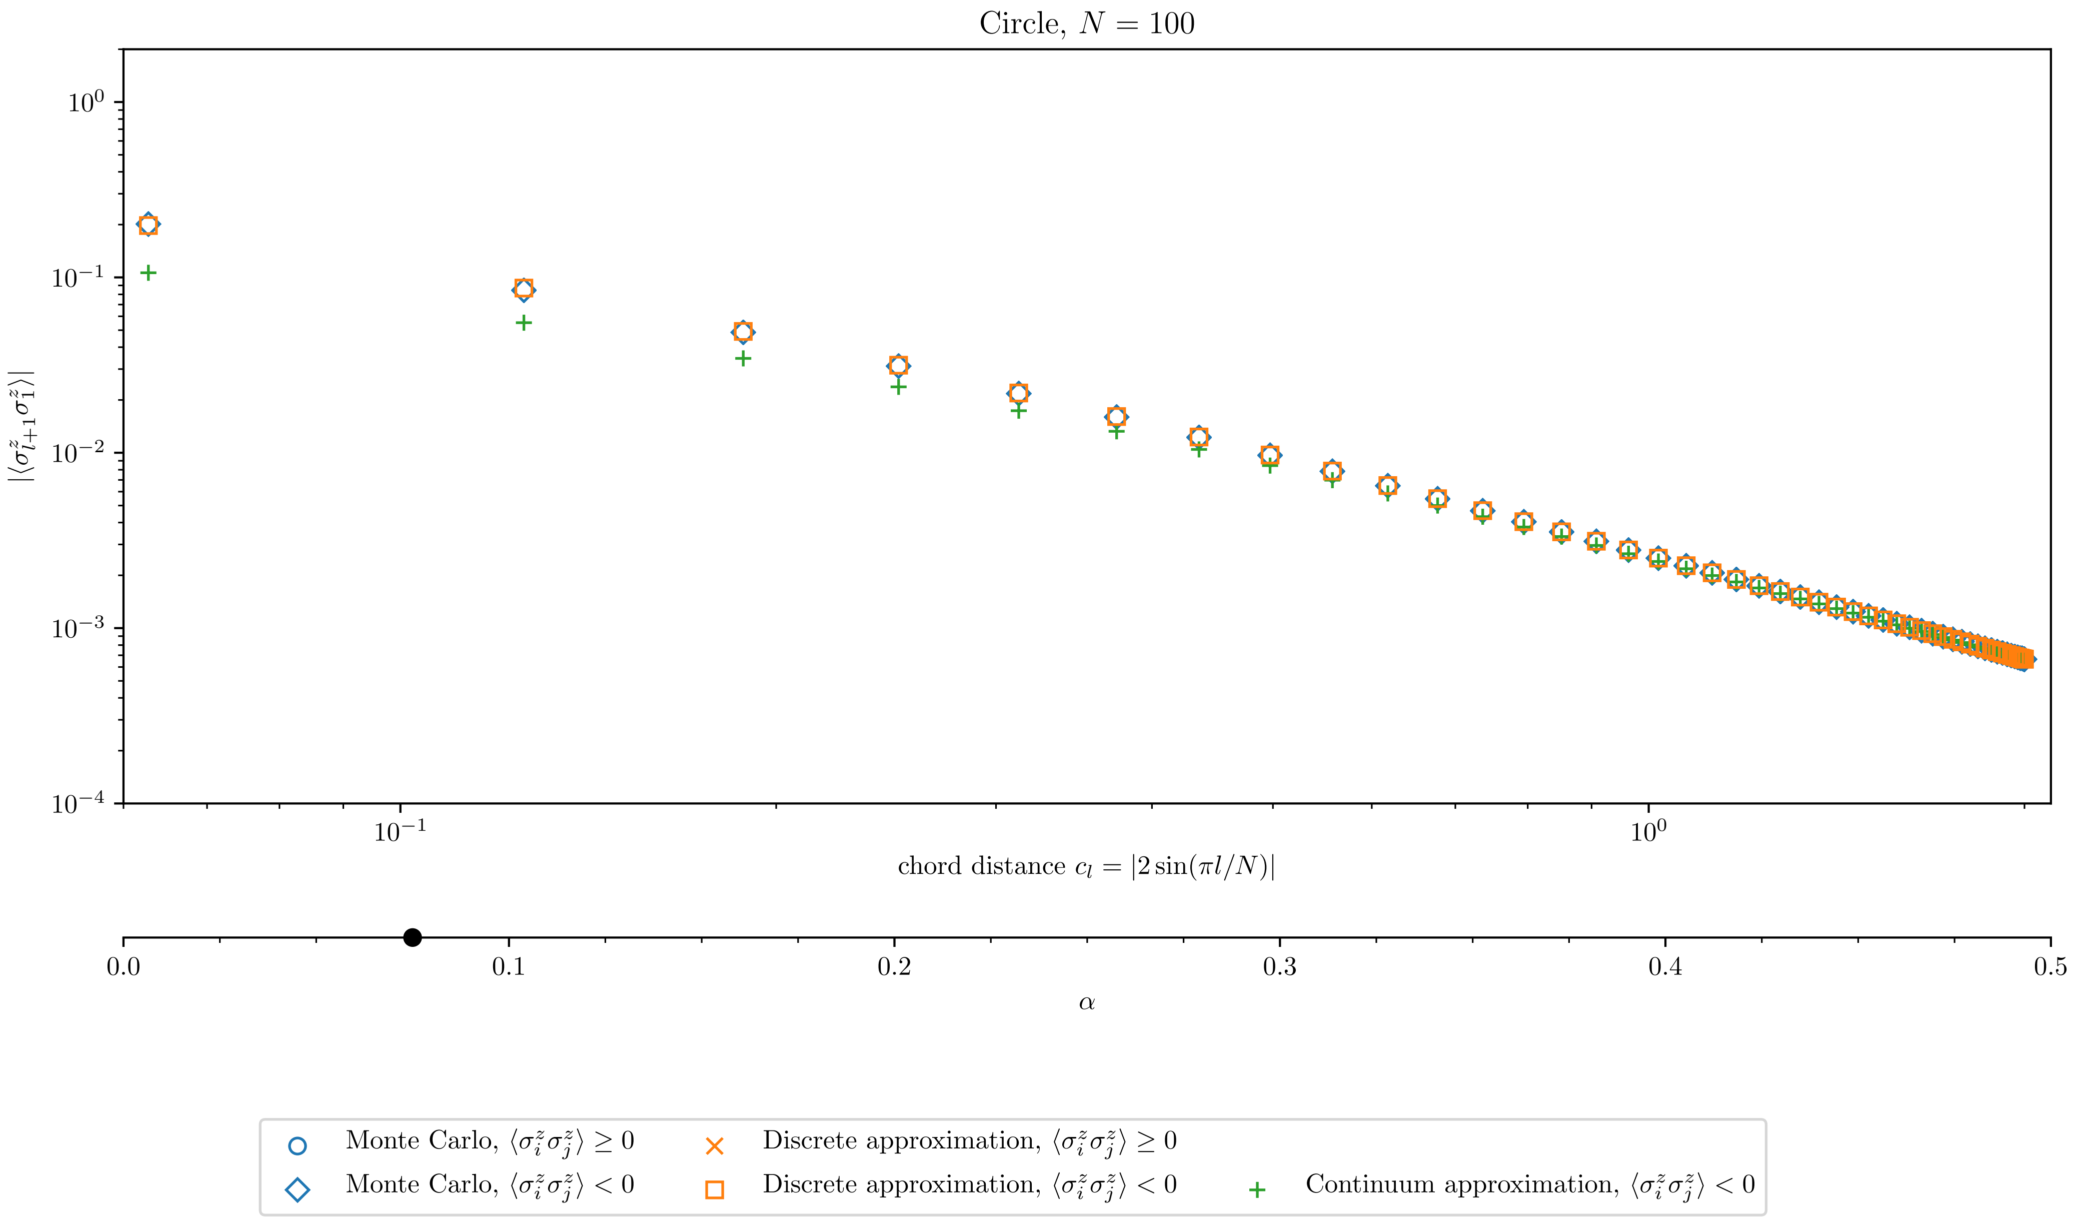
Circle, $N = 100$
$|\langle \sigma^z_{l+1} \sigma^z_1 \rangle|$
$10^0$
$10^{-1}$
$10^{-2}$
$10^{-3}$
$10^{-4}$
chord distance $c_l = |2\sin(\pi l/N)|$
$\alpha$
0.0
0.1
0.2
0.3
0.4
0.5
Monte Carlo, $\langle \sigma^z_i \sigma^z_j \rangle \geq 0$
Monte Carlo, $\langle \sigma^z_i \sigma^z_j \rangle < 0$
Discrete approximation, $\langle \sigma^z_i \sigma^z_j \rangle \geq 0$
Discrete approximation, $\langle \sigma^z_i \sigma^z_j \rangle < 0$
Continuum approximation, $\langle \sigma^z_i \sigma^z_j \rangle < 0$

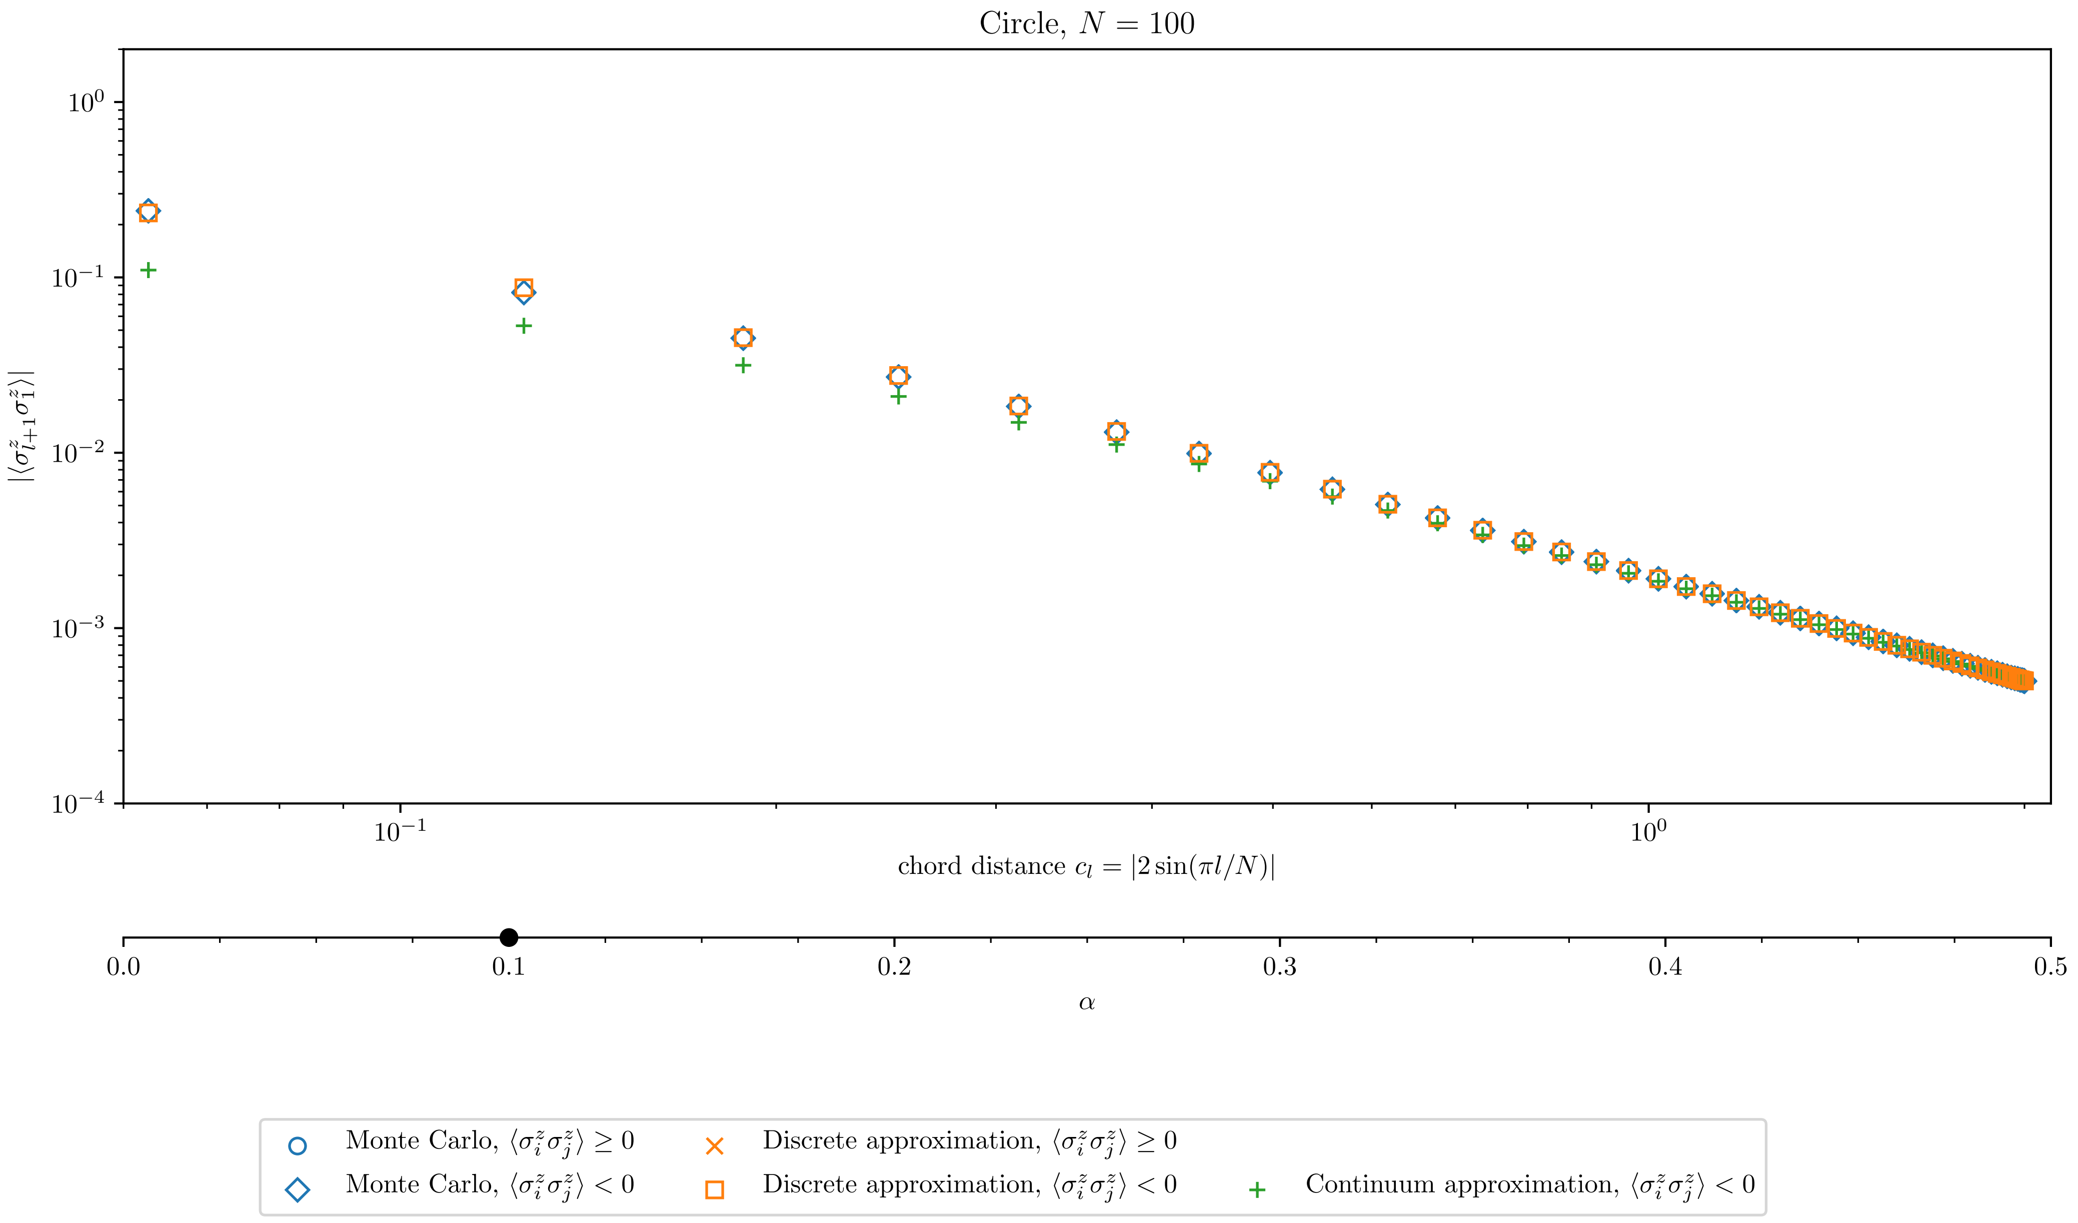

Circle, $N = 100$
$|\langle\sigma^z_{l+1}\sigma^z_1\rangle|$
$10^0$
$10^{-1}$
$10^{-2}$
$10^{-3}$
$10^{-4}$
chord distance $c_l = |2\sin(\pi l/N)|$
0.0
0.1
0.2
0.3
0.4
0.5
$\alpha$
Monte Carlo, $\langle\sigma^z_i\sigma^z_j\rangle \geq 0$
Monte Carlo, $\langle\sigma^z_i\sigma^z_j\rangle < 0$
Discrete approximation, $\langle\sigma^z_i\sigma^z_j\rangle \geq 0$
Discrete approximation, $\langle\sigma^z_i\sigma^z_j\rangle < 0$
Continuum approximation, $\langle\sigma^z_i\sigma^z_j\rangle < 0$

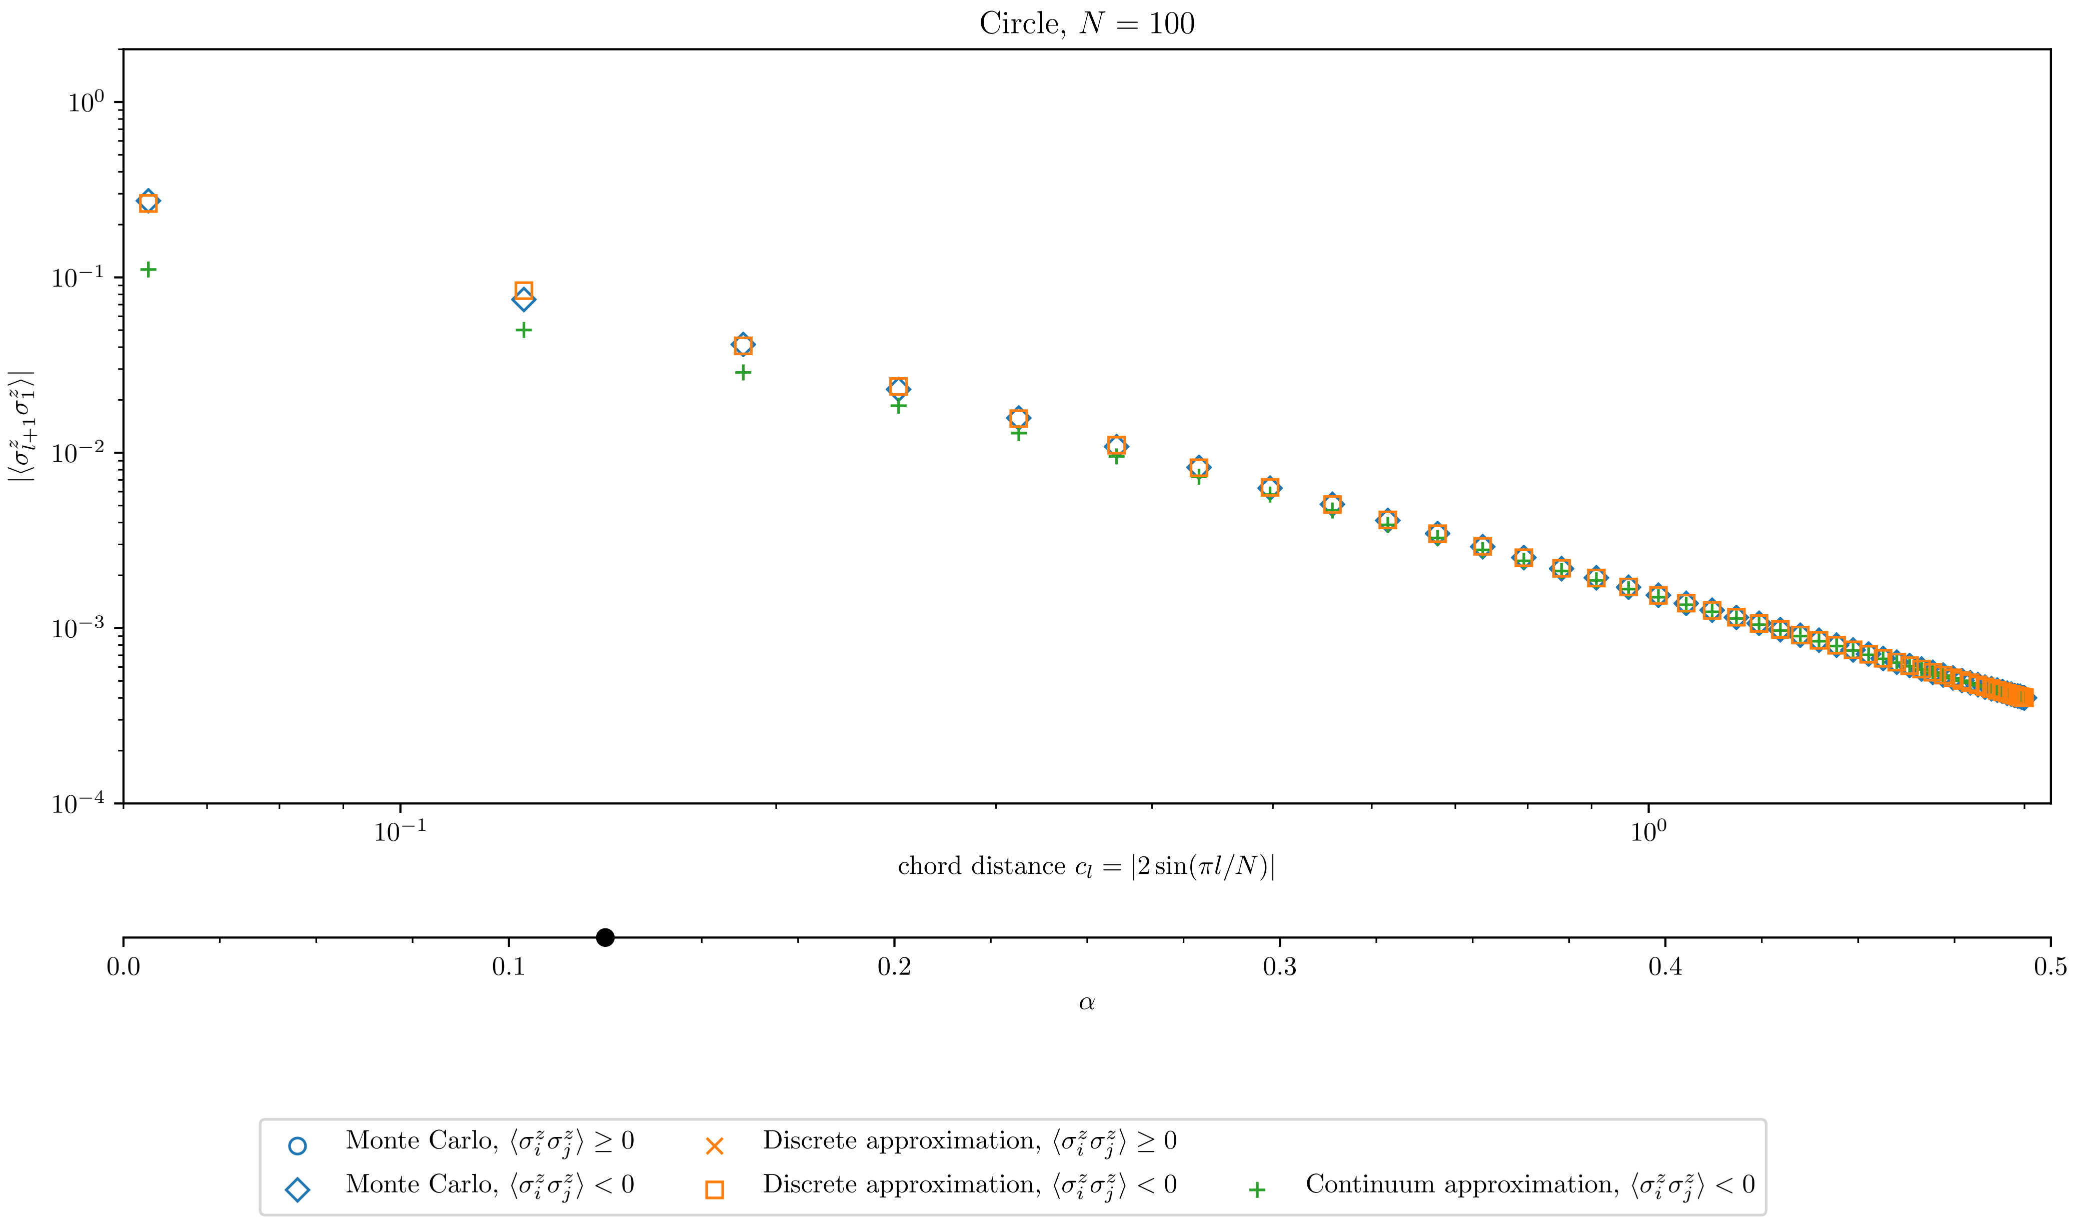

Circle, $N = 100$
$10^0$
$10^{-1}$
$10^{-2}$
$10^{-3}$
$10^{-4}$
$|\langle \sigma^z_{l+1} \sigma^z_1 \rangle|$
$10^{-1}$
$10^0$
chord distance $c_l = |2\sin(\pi l/N)|$
0.0
0.1
0.2
0.3
0.4
0.5
$\alpha$
Monte Carlo, $\langle \sigma^z_i \sigma^z_j \rangle \geq 0$
Monte Carlo, $\langle \sigma^z_i \sigma^z_j \rangle < 0$
Discrete approximation, $\langle \sigma^z_i \sigma^z_j \rangle \geq 0$
Discrete approximation, $\langle \sigma^z_i \sigma^z_j \rangle < 0$
Continuum approximation, $\langle \sigma^z_i \sigma^z_j \rangle < 0$

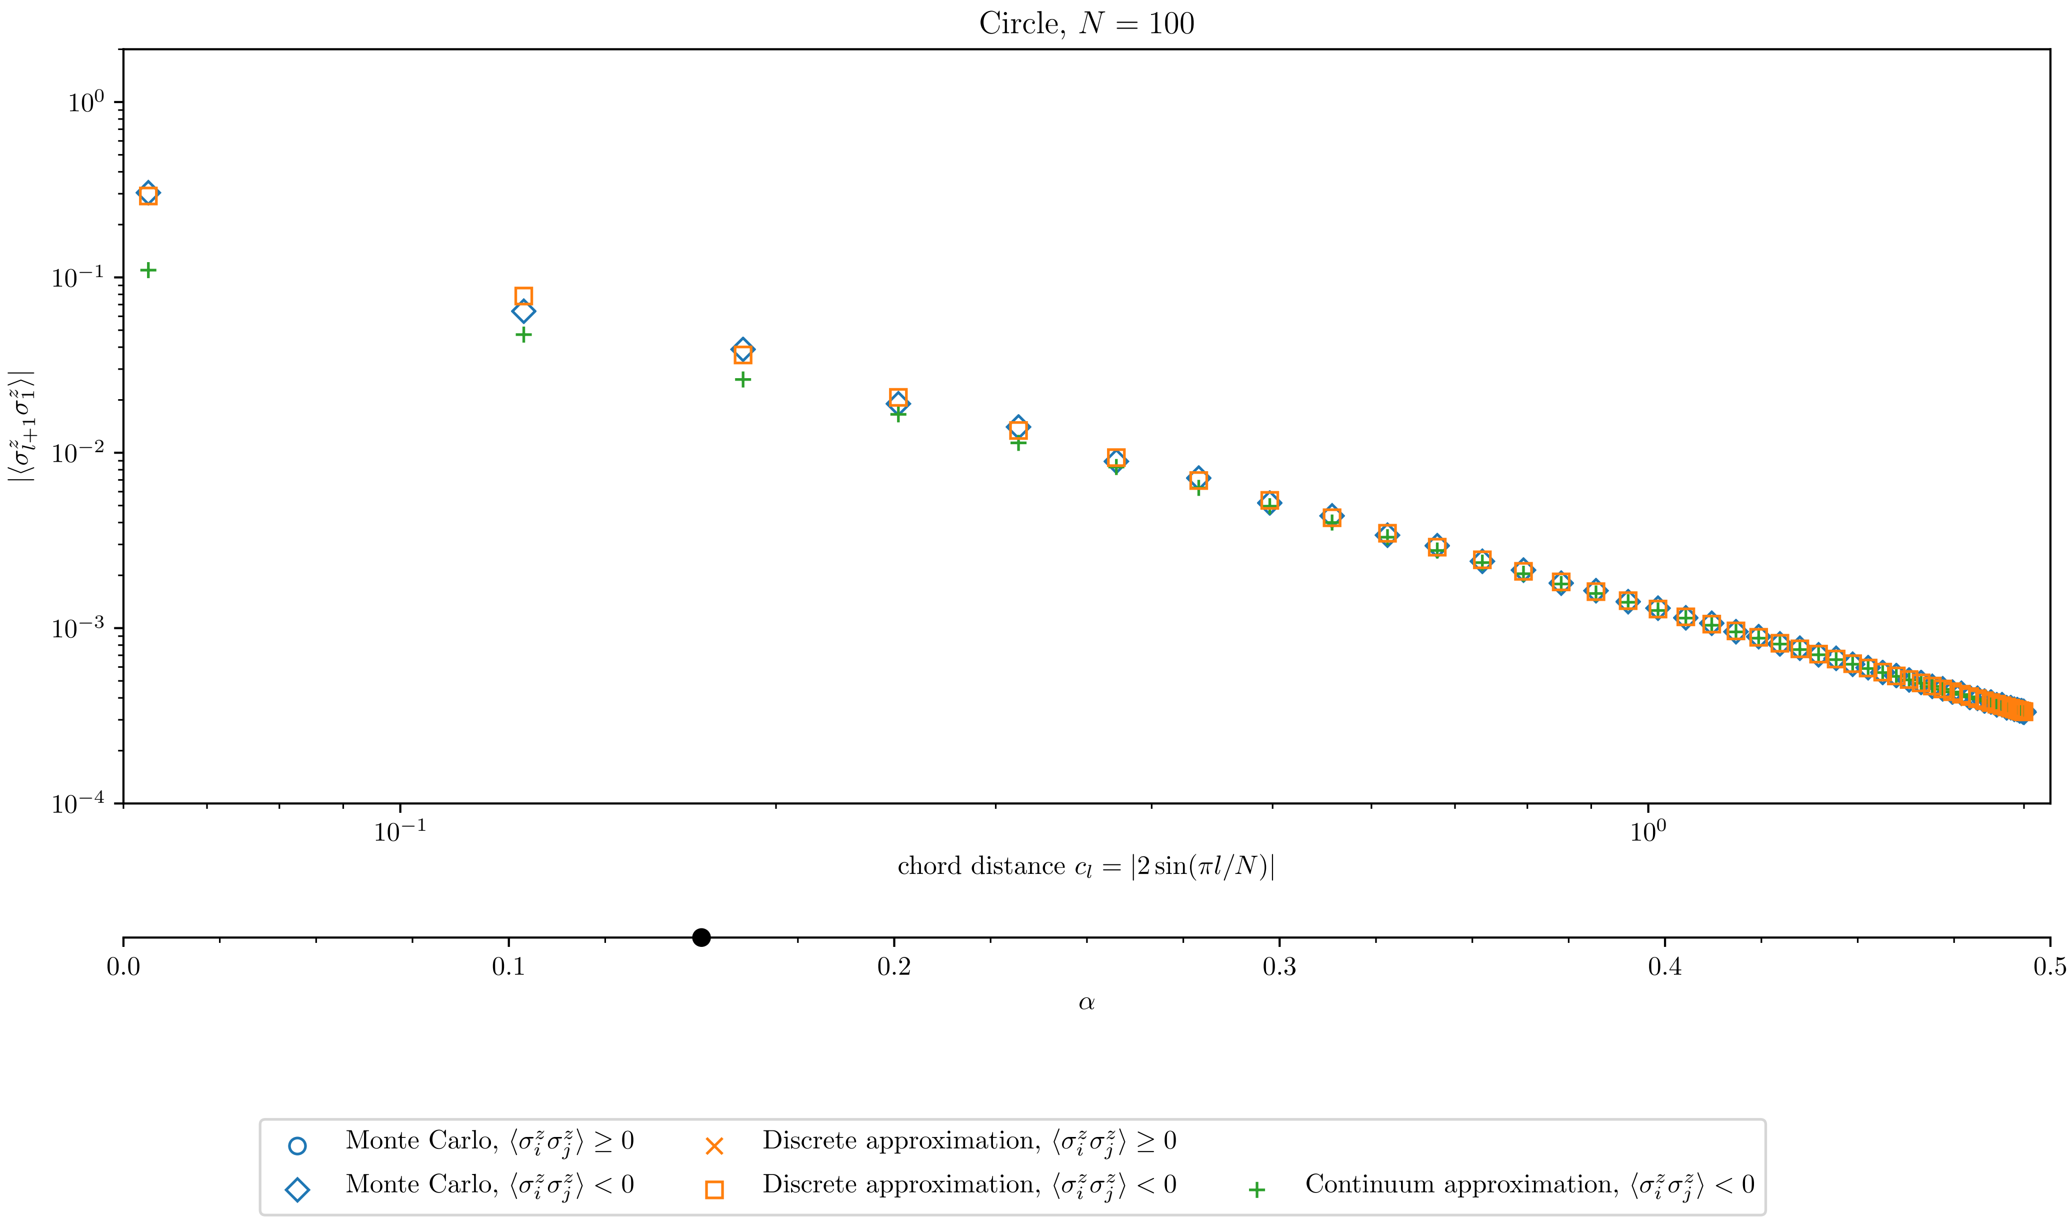

Circle, $N = 100$
$|\langle\sigma^z_{l+1}\sigma^z_1\rangle|$
$10^0$
$10^{-1}$
$10^{-2}$
$10^{-3}$
$10^{-4}$
$10^{-1}$
$10^0$
chord distance $c_l = |2\sin(\pi l/N)|$
0.0
0.1
0.2
0.3
0.4
0.5
$\alpha$
Monte Carlo, $\langle\sigma^z_i\sigma^z_j\rangle \geq 0$
Monte Carlo, $\langle\sigma^z_i\sigma^z_j\rangle < 0$
Discrete approximation, $\langle\sigma^z_i\sigma^z_j\rangle \geq 0$
Discrete approximation, $\langle\sigma^z_i\sigma^z_j\rangle < 0$
Continuum approximation, $\langle\sigma^z_i\sigma^z_j\rangle < 0$

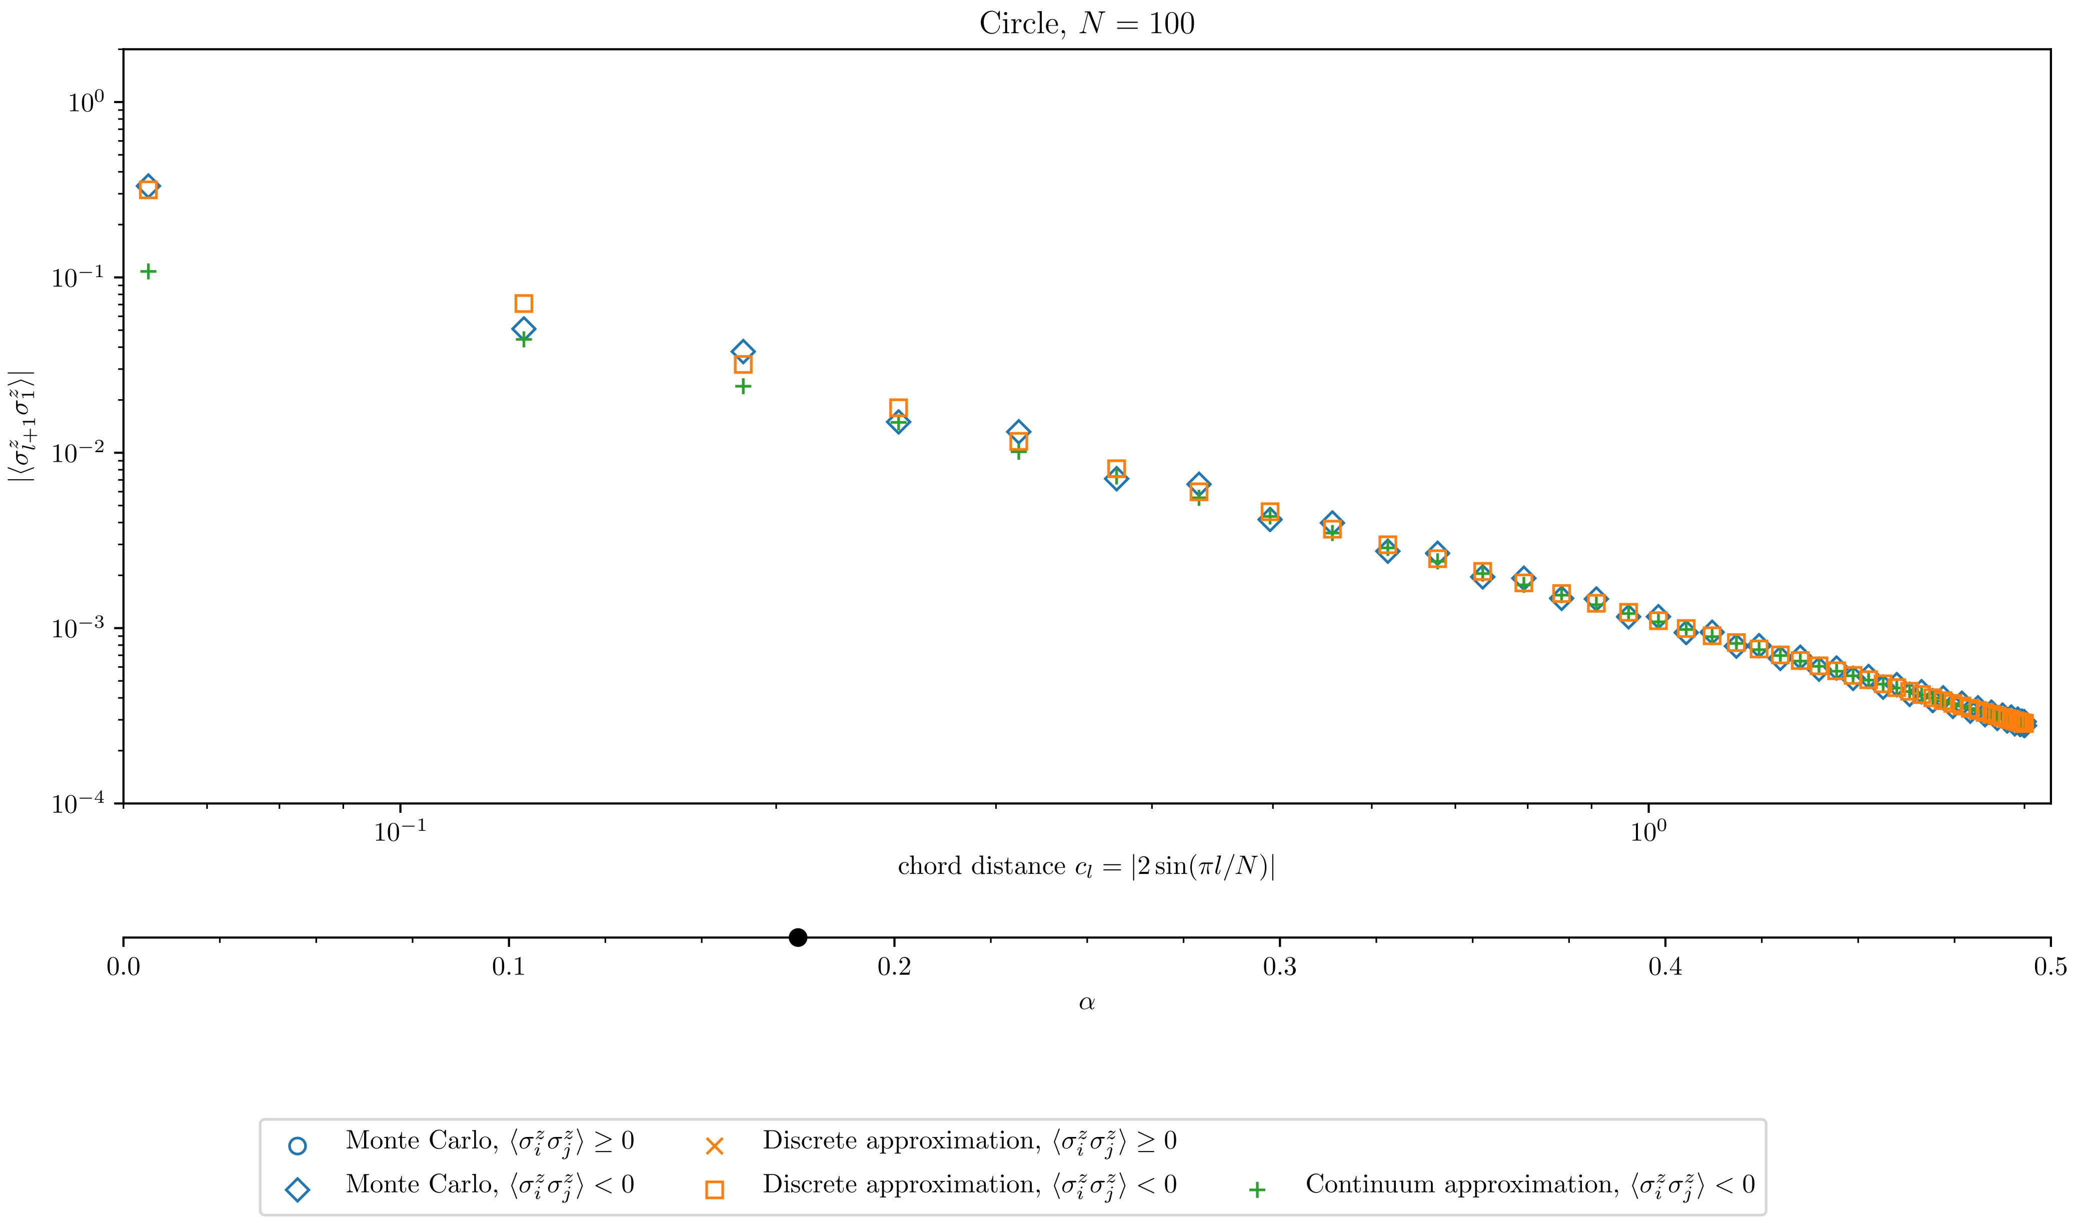

Circle, $N = 100$
$|\langle\sigma^z_{l+1}\sigma^z_1\rangle|$
$10^0$
$10^{-1}$
$10^{-2}$
$10^{-3}$
$10^{-4}$
$10^{-1}$
$10^0$
chord distance $c_l = |2\sin(\pi l/N)|$
0.0
0.1
0.2
0.3
0.4
0.5
$\alpha$
Monte Carlo, $\langle\sigma^z_i\sigma^z_j\rangle \geq 0$
Monte Carlo, $\langle\sigma^z_i\sigma^z_j\rangle < 0$
Discrete approximation, $\langle\sigma^z_i\sigma^z_j\rangle \geq 0$
Discrete approximation, $\langle\sigma^z_i\sigma^z_j\rangle < 0$
Continuum approximation, $\langle\sigma^z_i\sigma^z_j\rangle < 0$

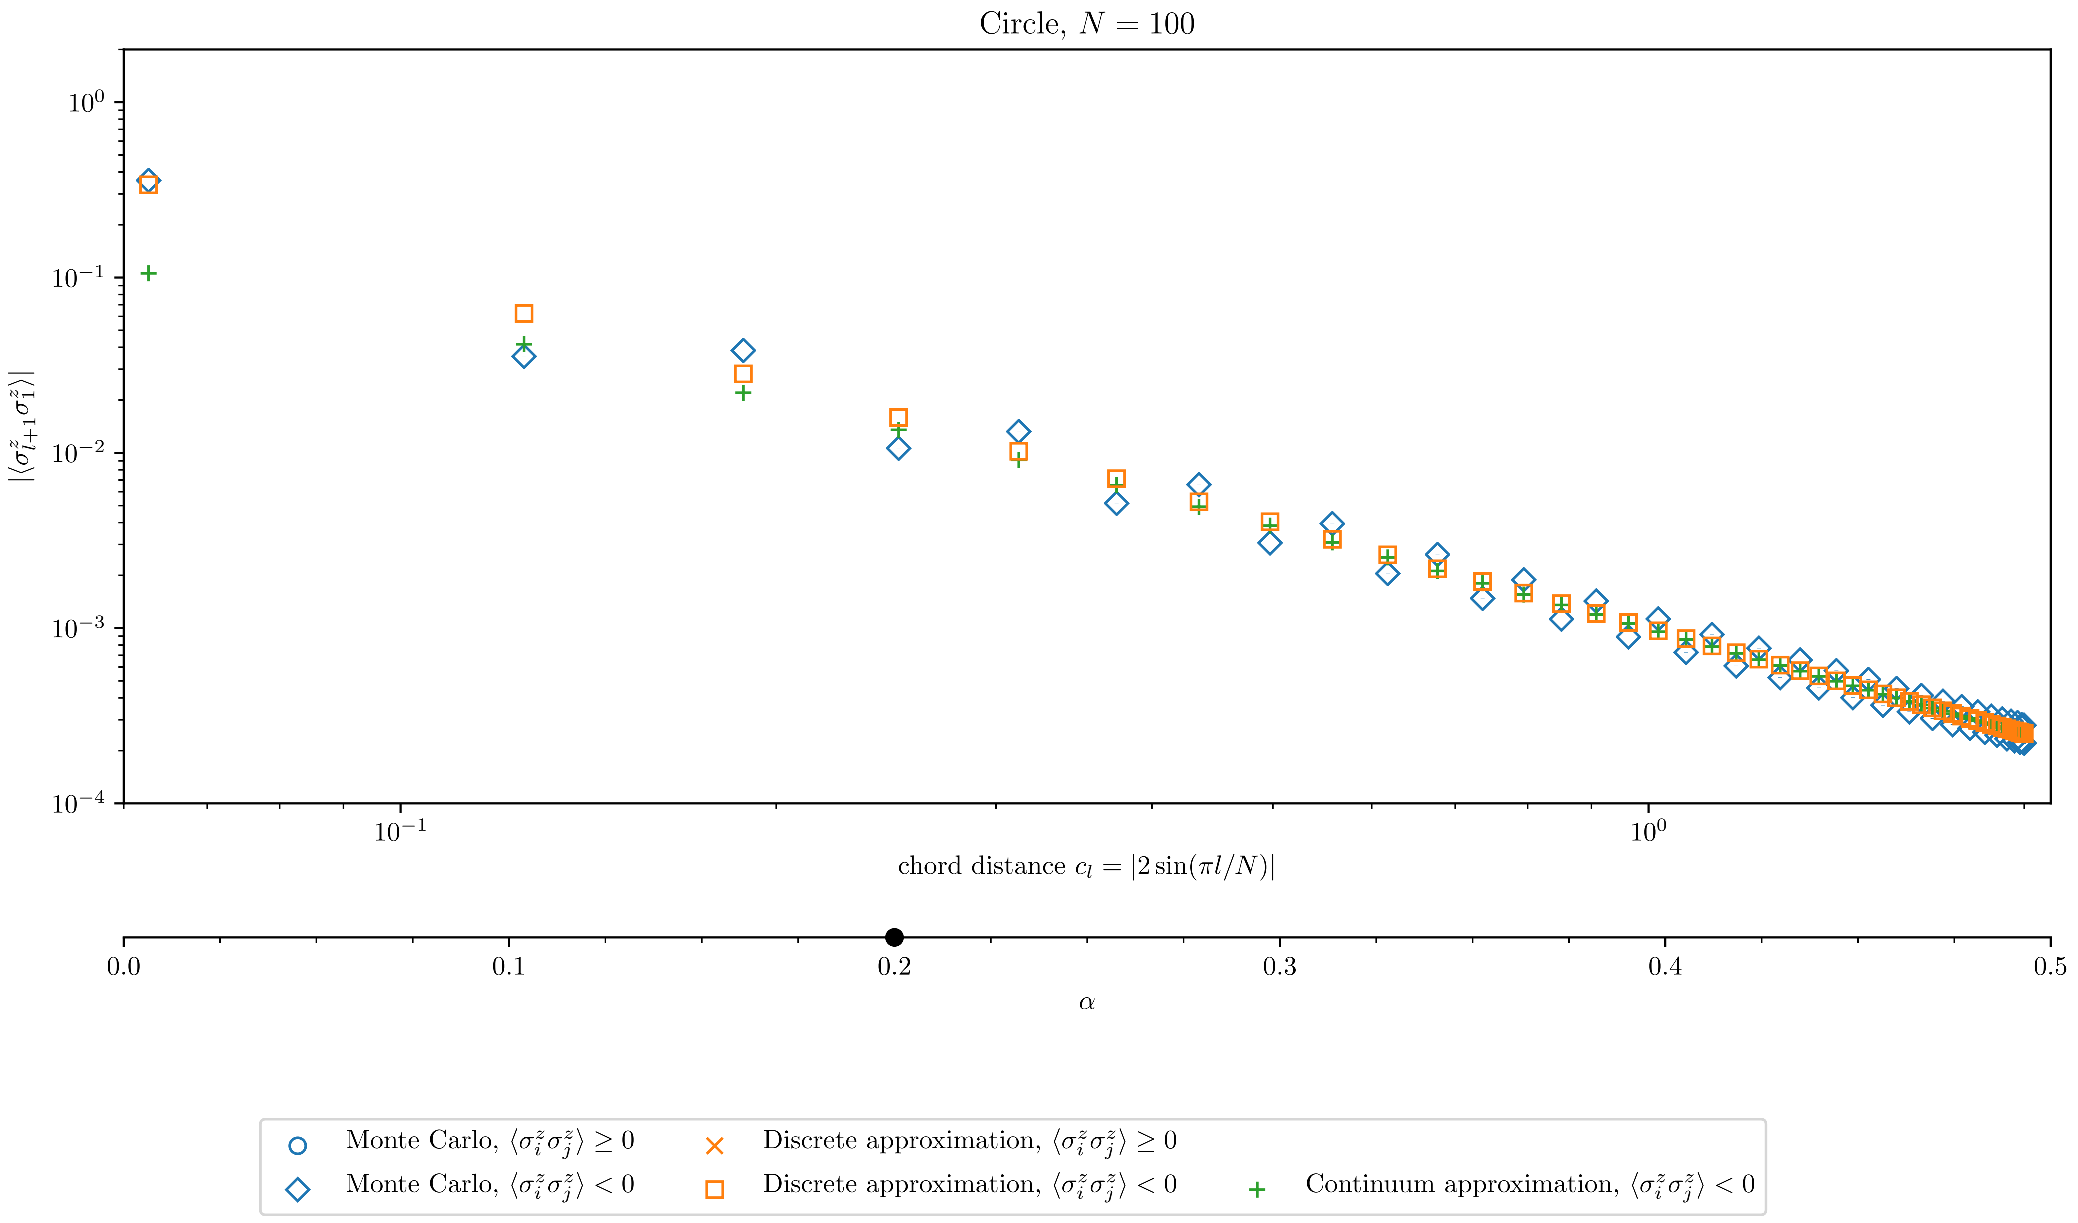
Circle, $N = 100$
$|\langle \sigma^z_{l+1} \sigma^z_1 \rangle|$
chord distance $c_l = |2 \sin(\pi l / N)|$
$\alpha$
Monte Carlo, $\langle \sigma^z_i \sigma^z_j \rangle \geq 0$
Monte Carlo, $\langle \sigma^z_i \sigma^z_j \rangle < 0$
Discrete approximation, $\langle \sigma^z_i \sigma^z_j \rangle \geq 0$
Discrete approximation, $\langle \sigma^z_i \sigma^z_j \rangle < 0$
Continuum approximation, $\langle \sigma^z_i \sigma^z_j \rangle < 0$

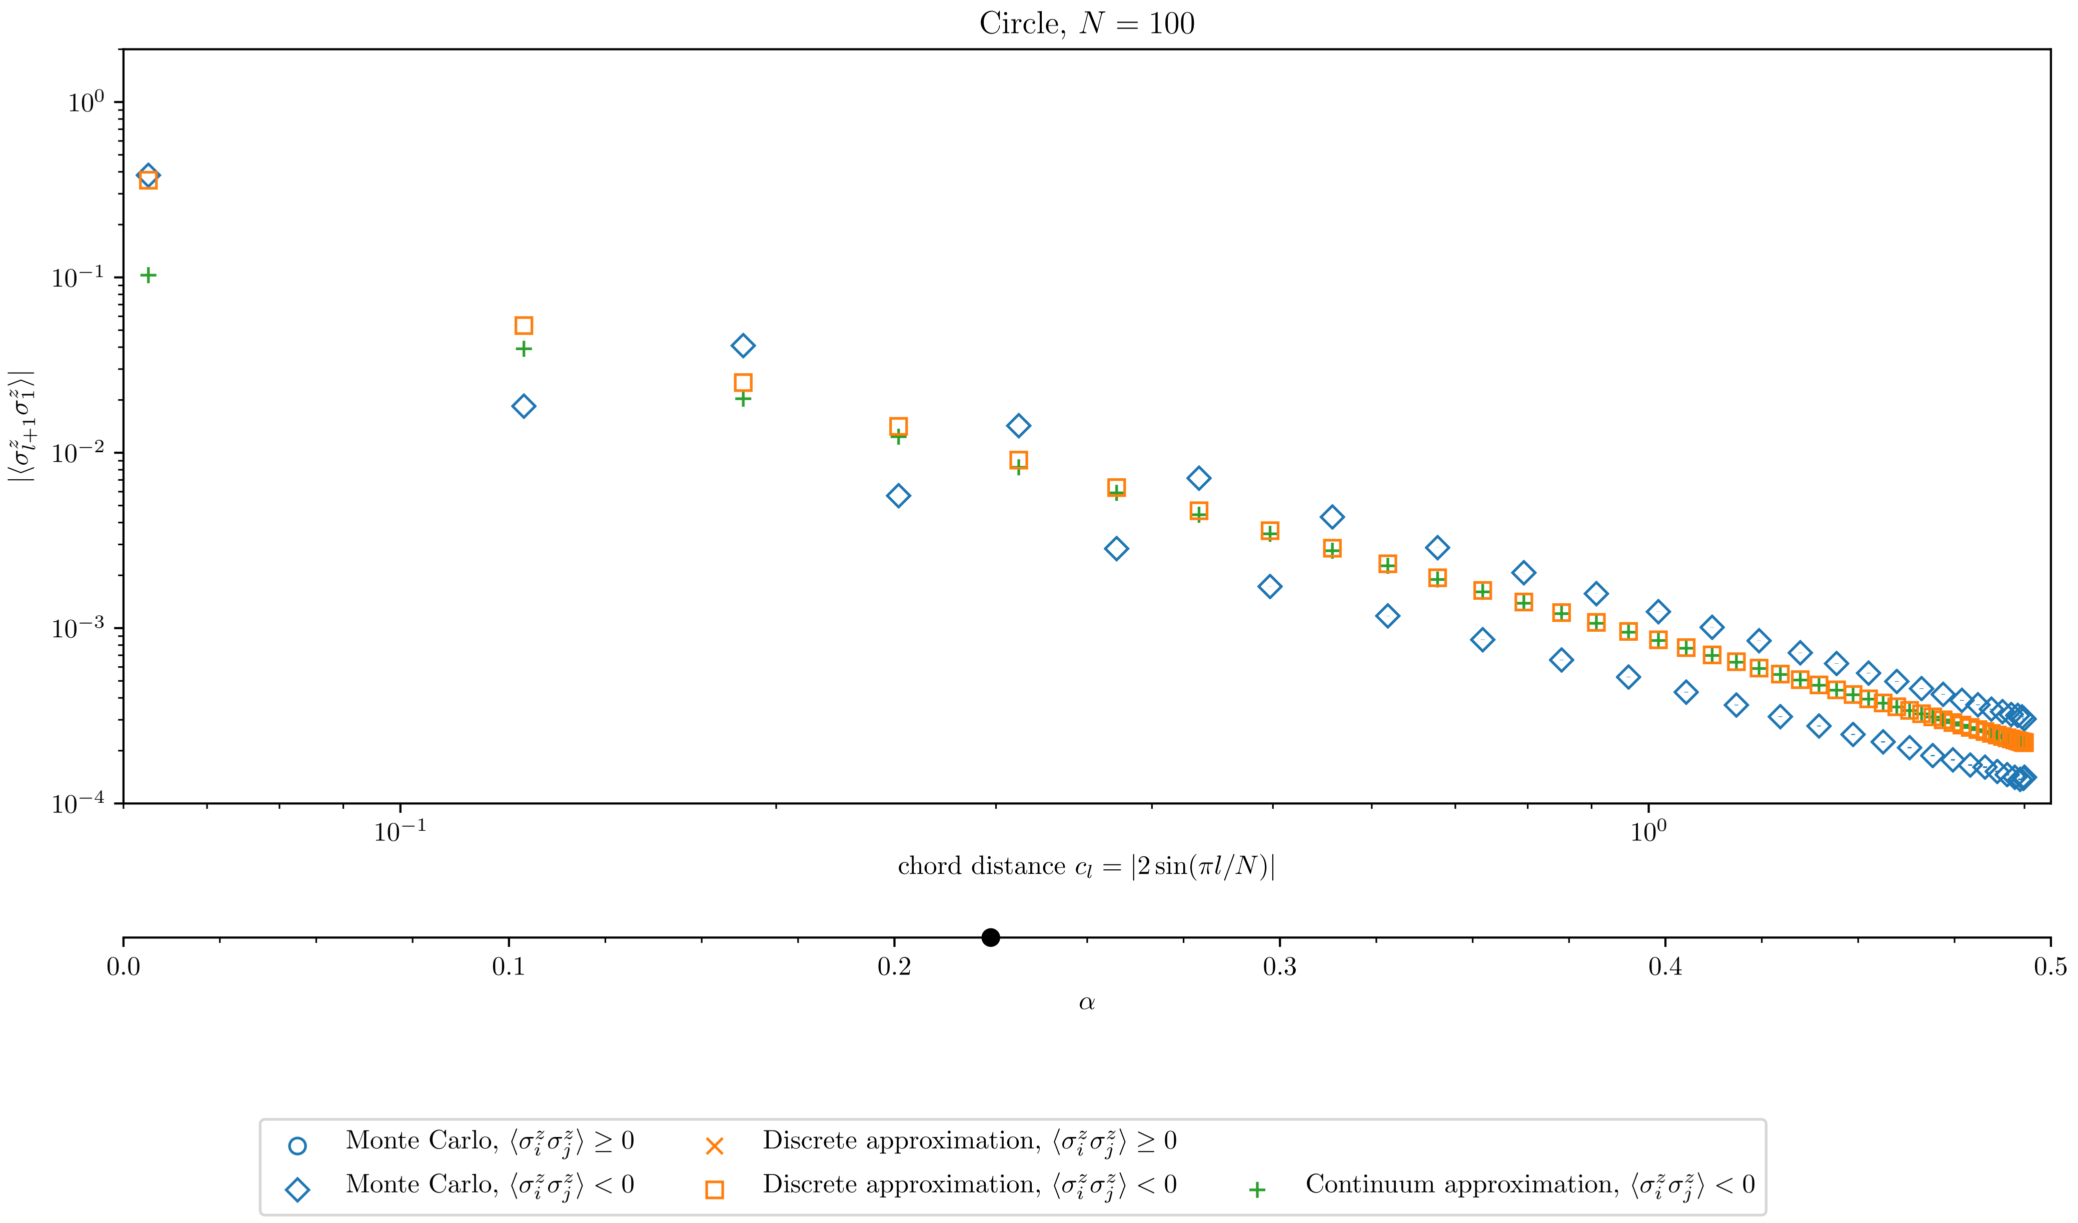

Circle, $N = 100$
$|\langle\sigma^z_{l+1}\sigma^z_1\rangle|$
$10^0$
$10^{-1}$
$10^{-2}$
$10^{-3}$
$10^{-4}$
chord distance $c_l = |2\sin(\pi l/N)|$
0.0
0.1
0.2
0.3
0.4
0.5
$\alpha$
Monte Carlo, $\langle\sigma^z_i\sigma^z_j\rangle \geq 0$
Monte Carlo, $\langle\sigma^z_i\sigma^z_j\rangle < 0$
Discrete approximation, $\langle\sigma^z_i\sigma^z_j\rangle \geq 0$
Discrete approximation, $\langle\sigma^z_i\sigma^z_j\rangle < 0$
Continuum approximation, $\langle\sigma^z_i\sigma^z_j\rangle < 0$

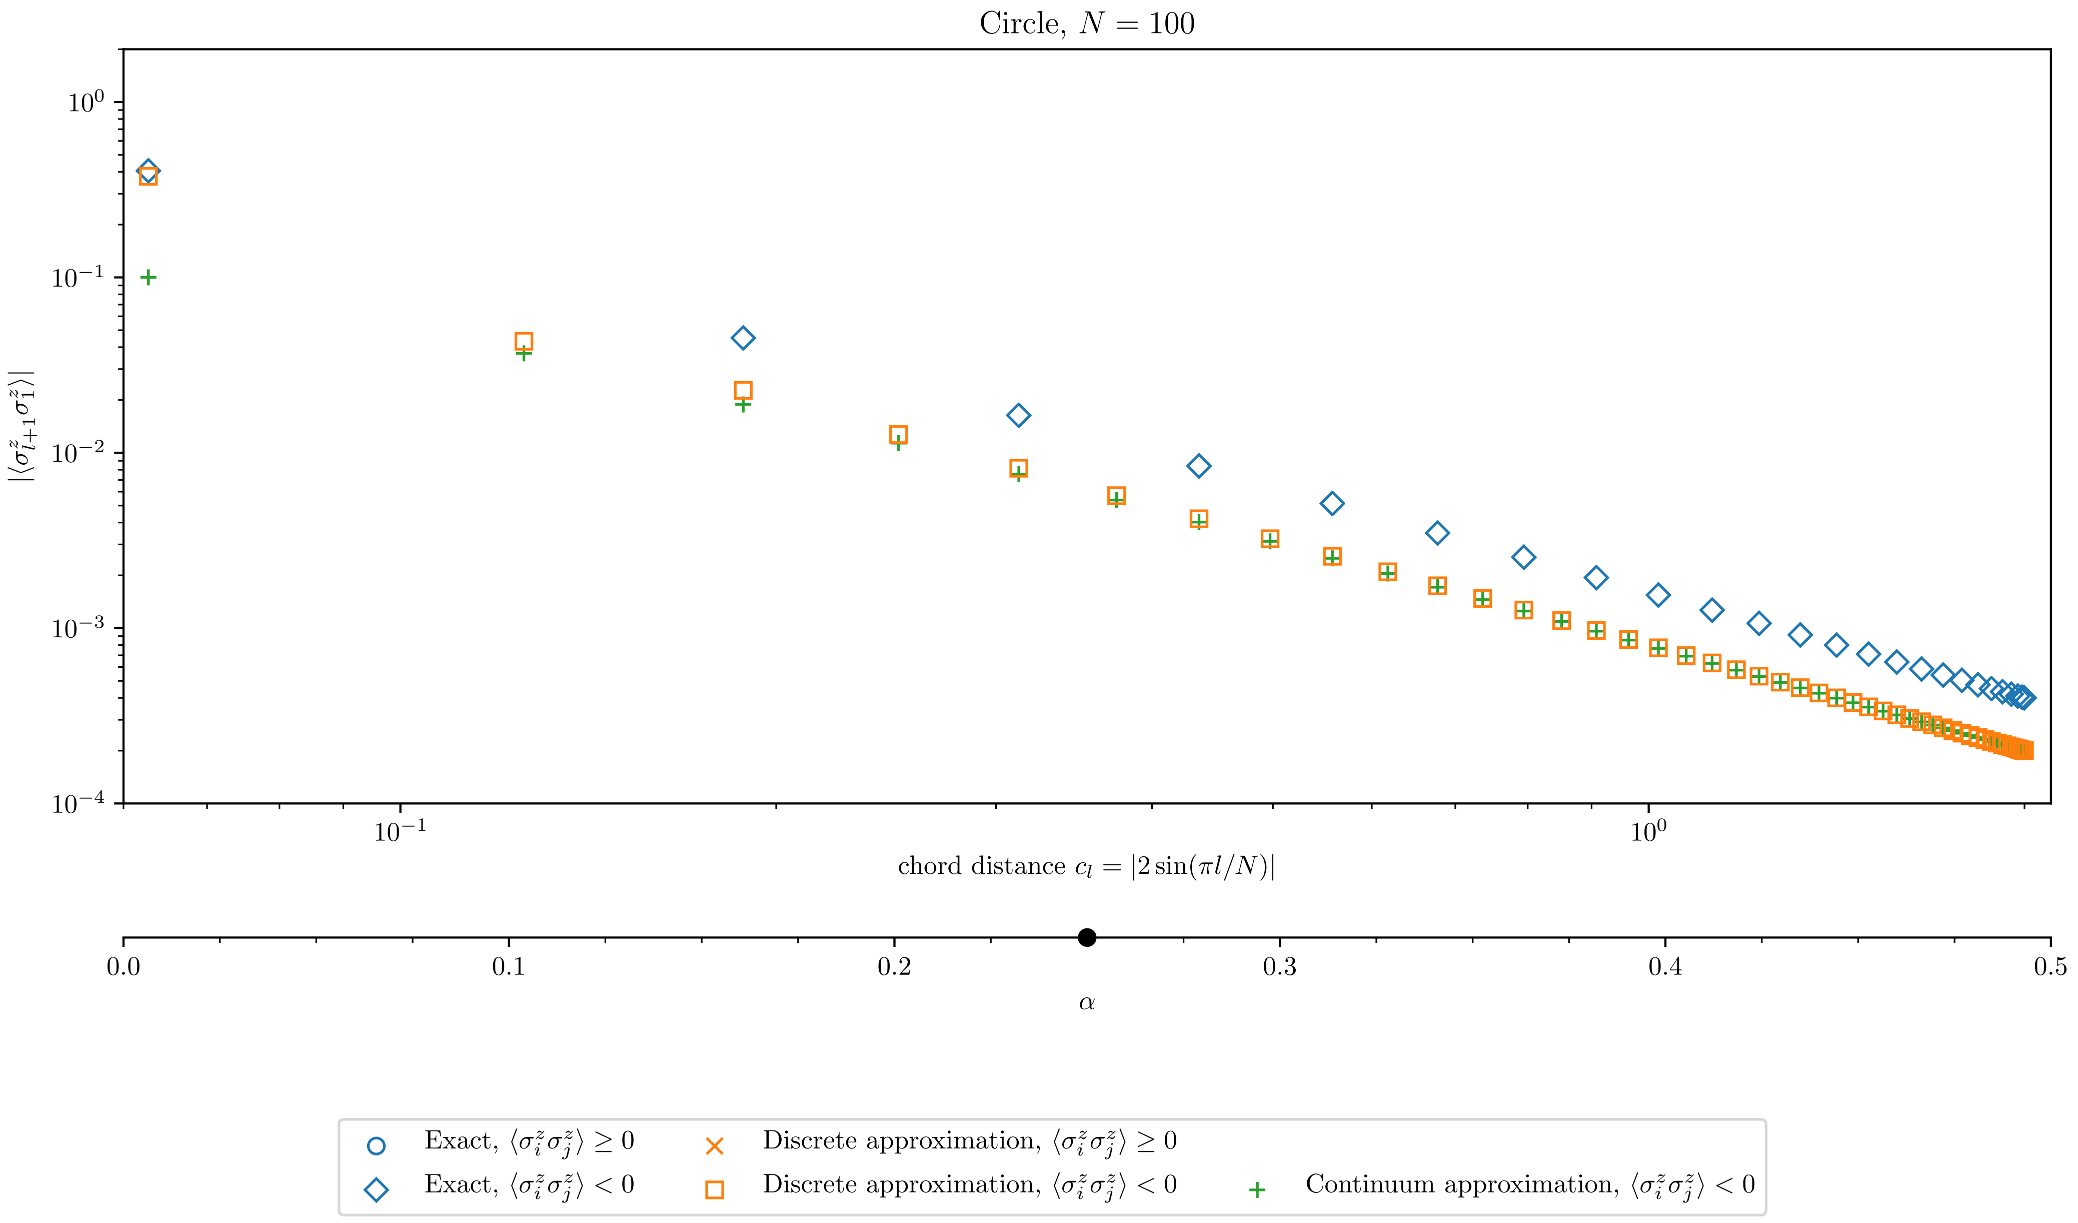

Circle, $N = 100$
$|\langle \sigma^z_{l+1} \sigma^z_1 \rangle|$
chord distance $c_l = |2\sin(\pi l/N)|$
$\alpha$
Exact, $\langle \sigma^z_i \sigma^z_j \rangle \geq 0$
Exact, $\langle \sigma^z_i \sigma^z_j \rangle < 0$
Discrete approximation, $\langle \sigma^z_i \sigma^z_j \rangle \geq 0$
Discrete approximation, $\langle \sigma^z_i \sigma^z_j \rangle < 0$
Continuum approximation, $\langle \sigma^z_i \sigma^z_j \rangle < 0$

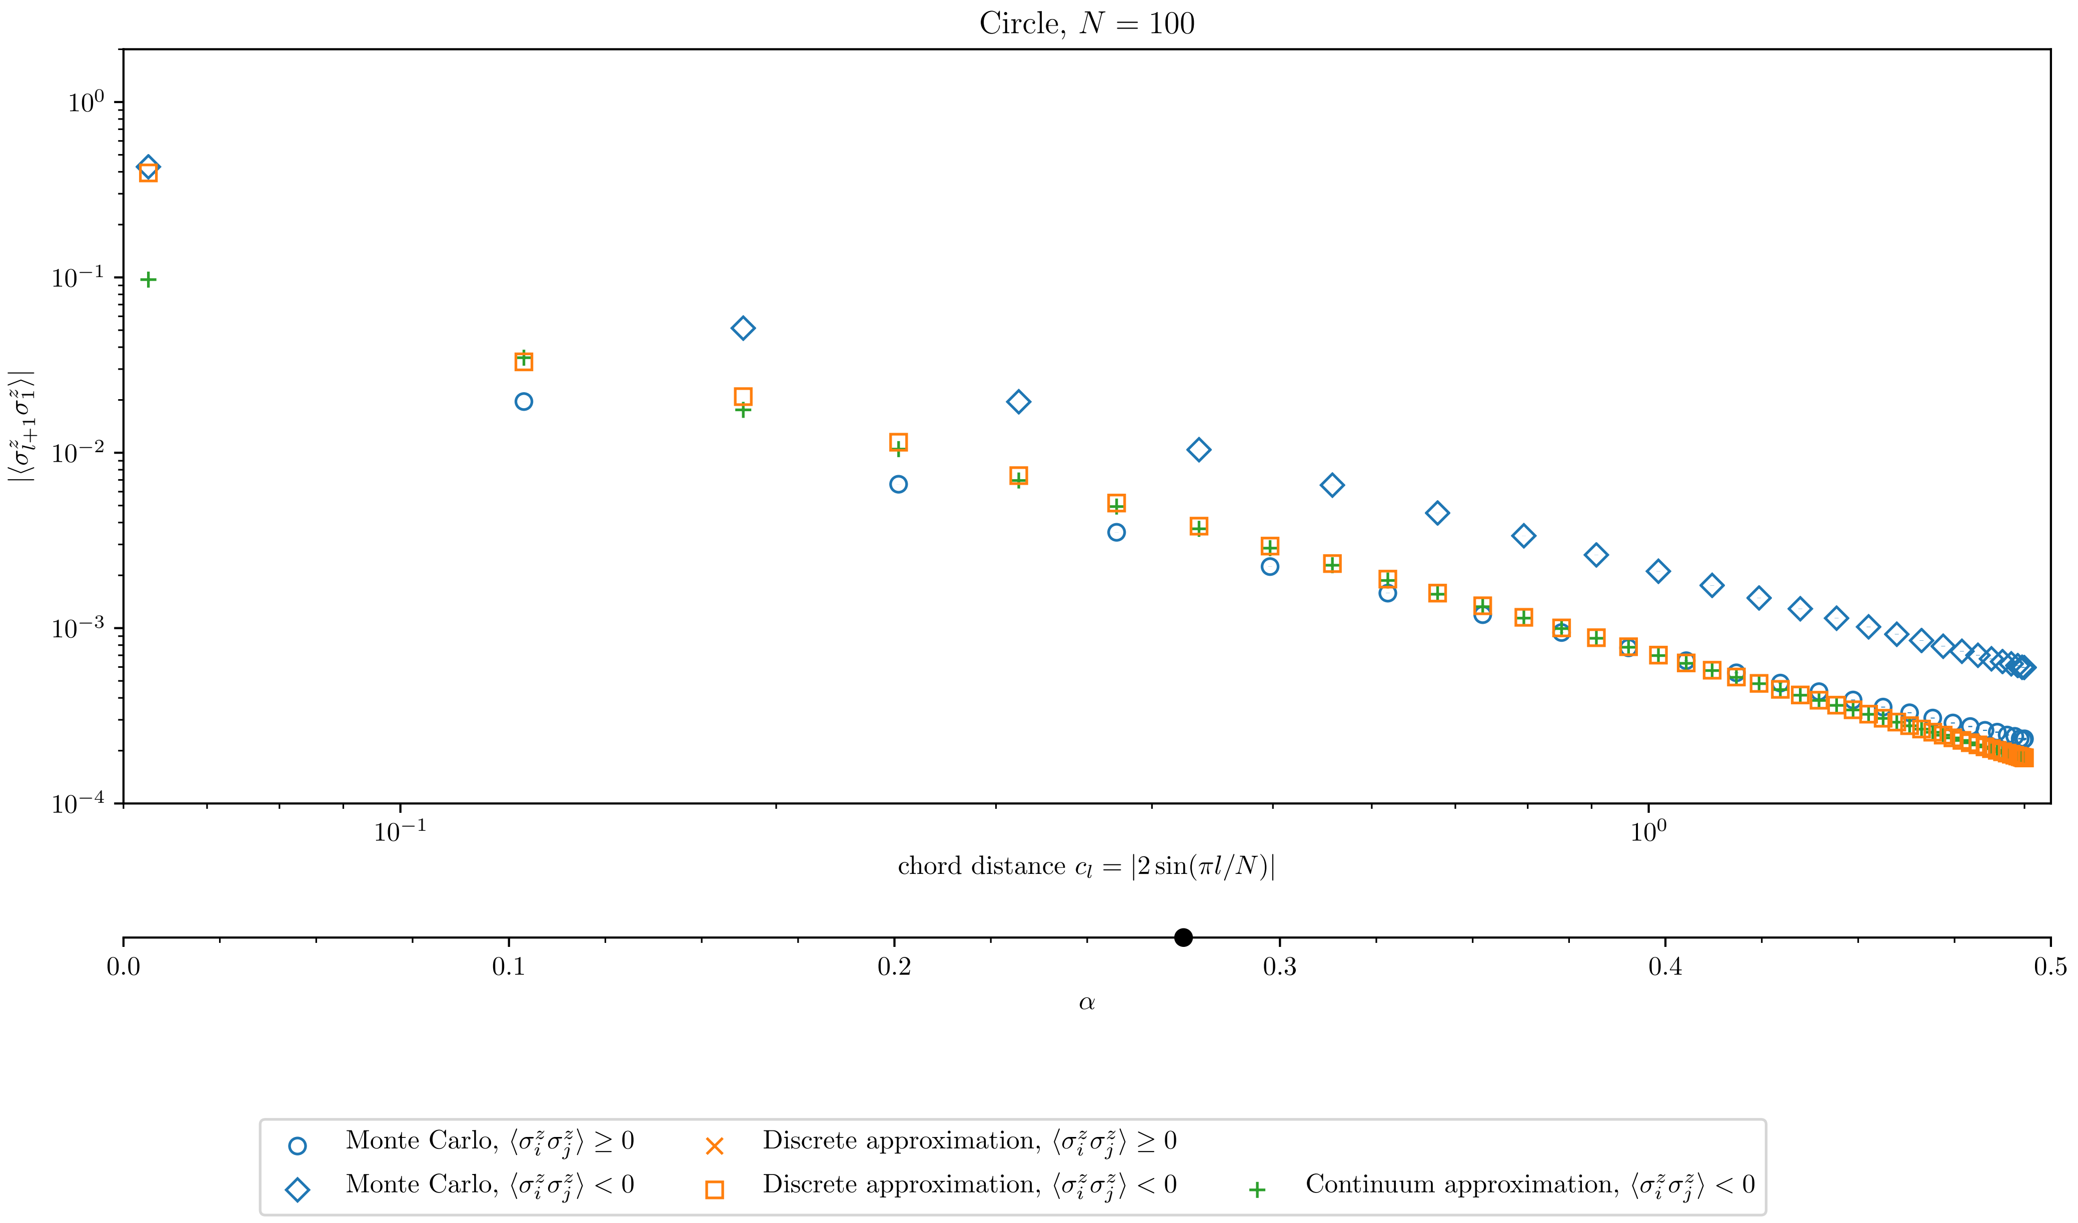
Circle, $N = 100$
$|\langle \sigma^z_{l+1} \sigma^z_1 \rangle|$
chord distance $c_l = |2\sin(\pi l/N)|$
$\alpha$
Monte Carlo, $\langle \sigma^z_i \sigma^z_j \rangle \geq 0$
Monte Carlo, $\langle \sigma^z_i \sigma^z_j \rangle < 0$
Discrete approximation, $\langle \sigma^z_i \sigma^z_j \rangle \geq 0$
Discrete approximation, $\langle \sigma^z_i \sigma^z_j \rangle < 0$
Continuum approximation, $\langle \sigma^z_i \sigma^z_j \rangle < 0$

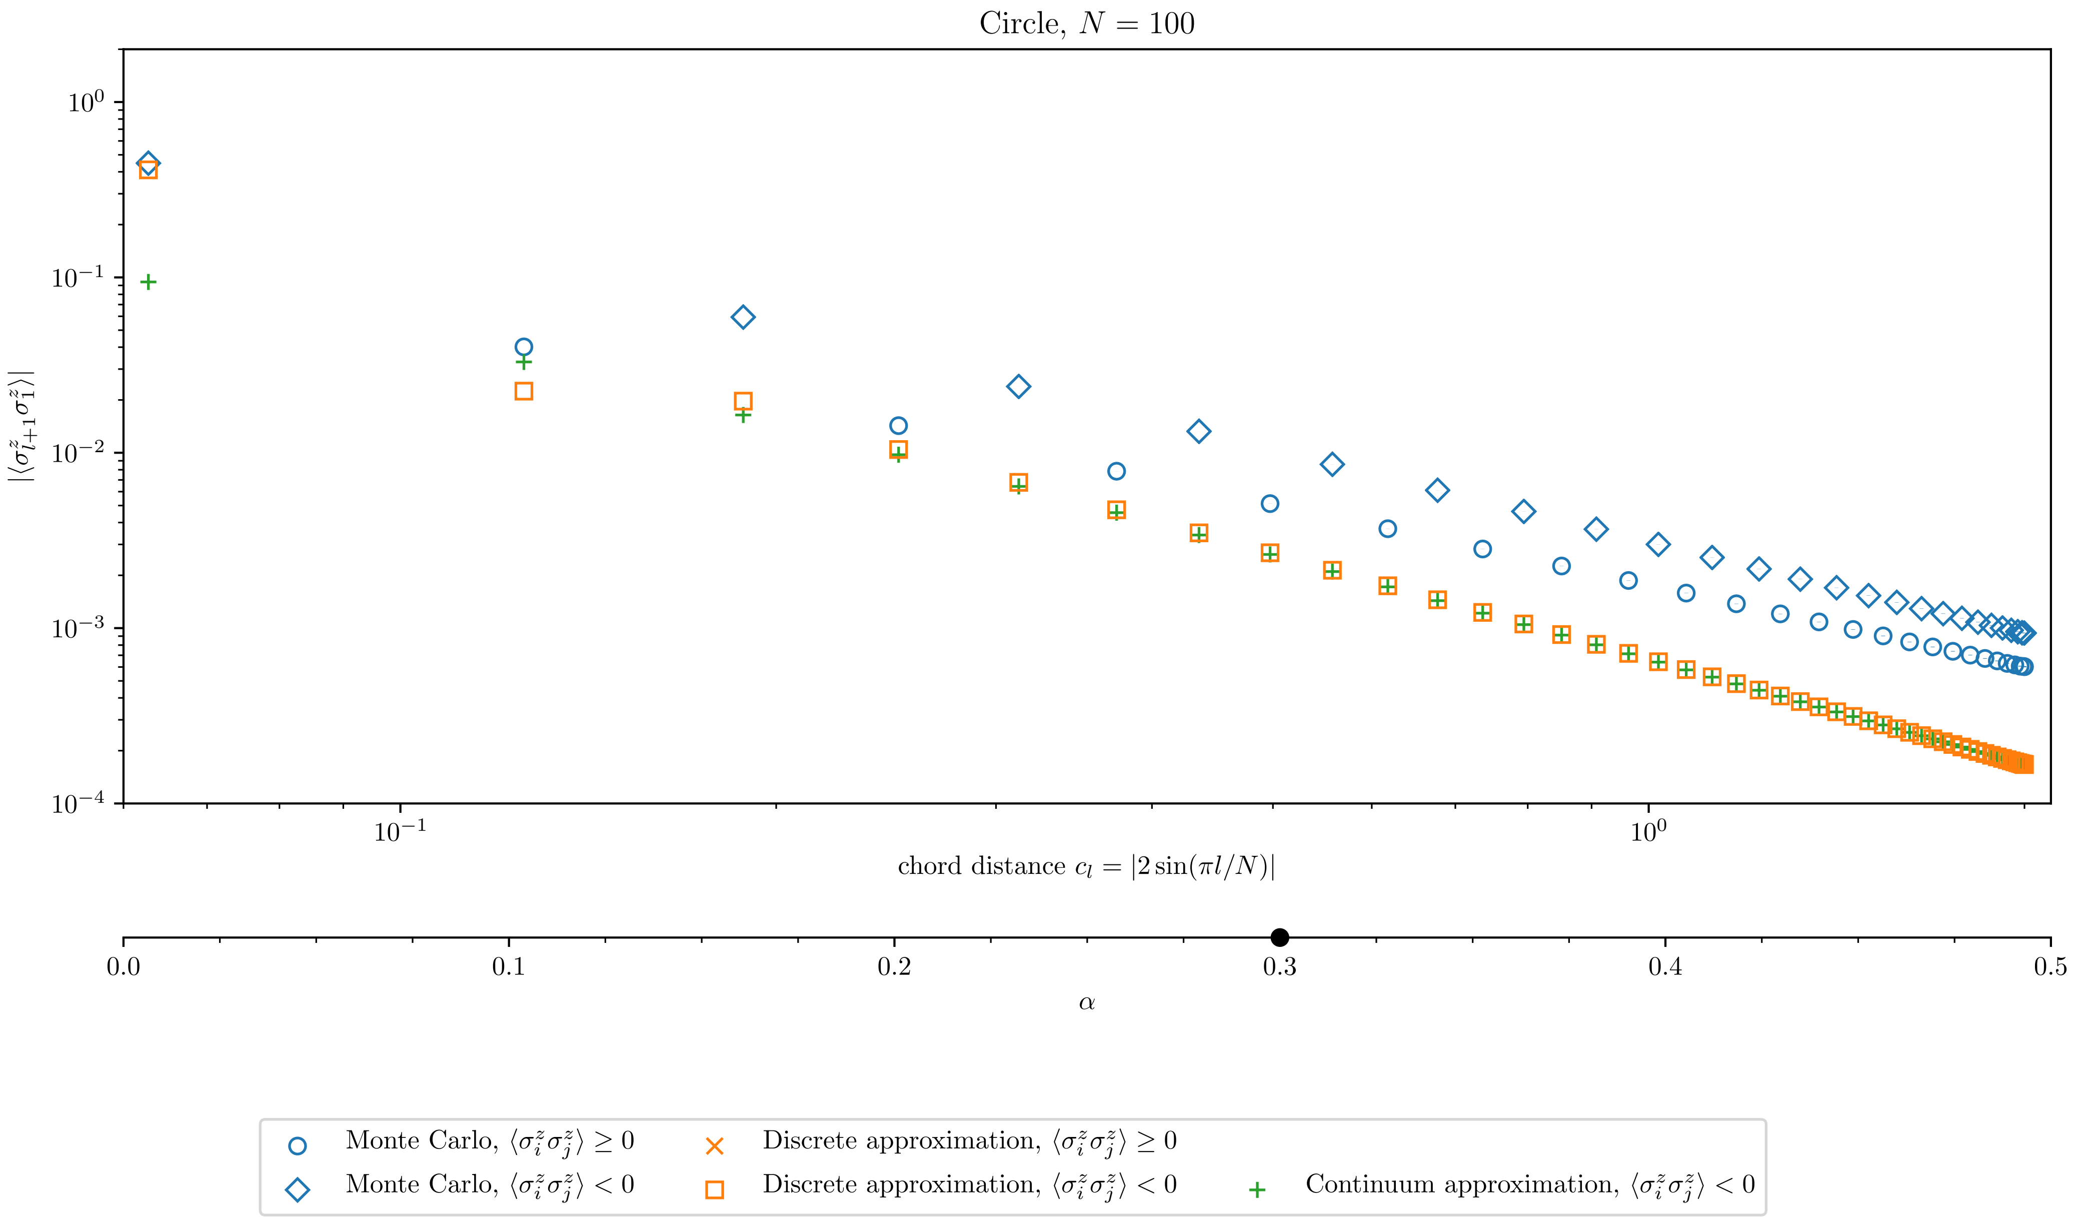

Circle, $N = 100$
$|\langle\sigma^z_{l+1}\sigma^z_1\rangle|$
$10^0$
$10^{-1}$
$10^{-2}$
$10^{-3}$
$10^{-4}$
$10^{-1}$
$10^0$
chord distance $c_l = |2\sin(\pi l/N)|$
0.0
0.1
0.2
0.3
0.4
0.5
$\alpha$
Monte Carlo, $\langle\sigma^z_i\sigma^z_j\rangle \geq 0$
Monte Carlo, $\langle\sigma^z_i\sigma^z_j\rangle < 0$
Discrete approximation, $\langle\sigma^z_i\sigma^z_j\rangle \geq 0$
Discrete approximation, $\langle\sigma^z_i\sigma^z_j\rangle < 0$
Continuum approximation, $\langle\sigma^z_i\sigma^z_j\rangle < 0$

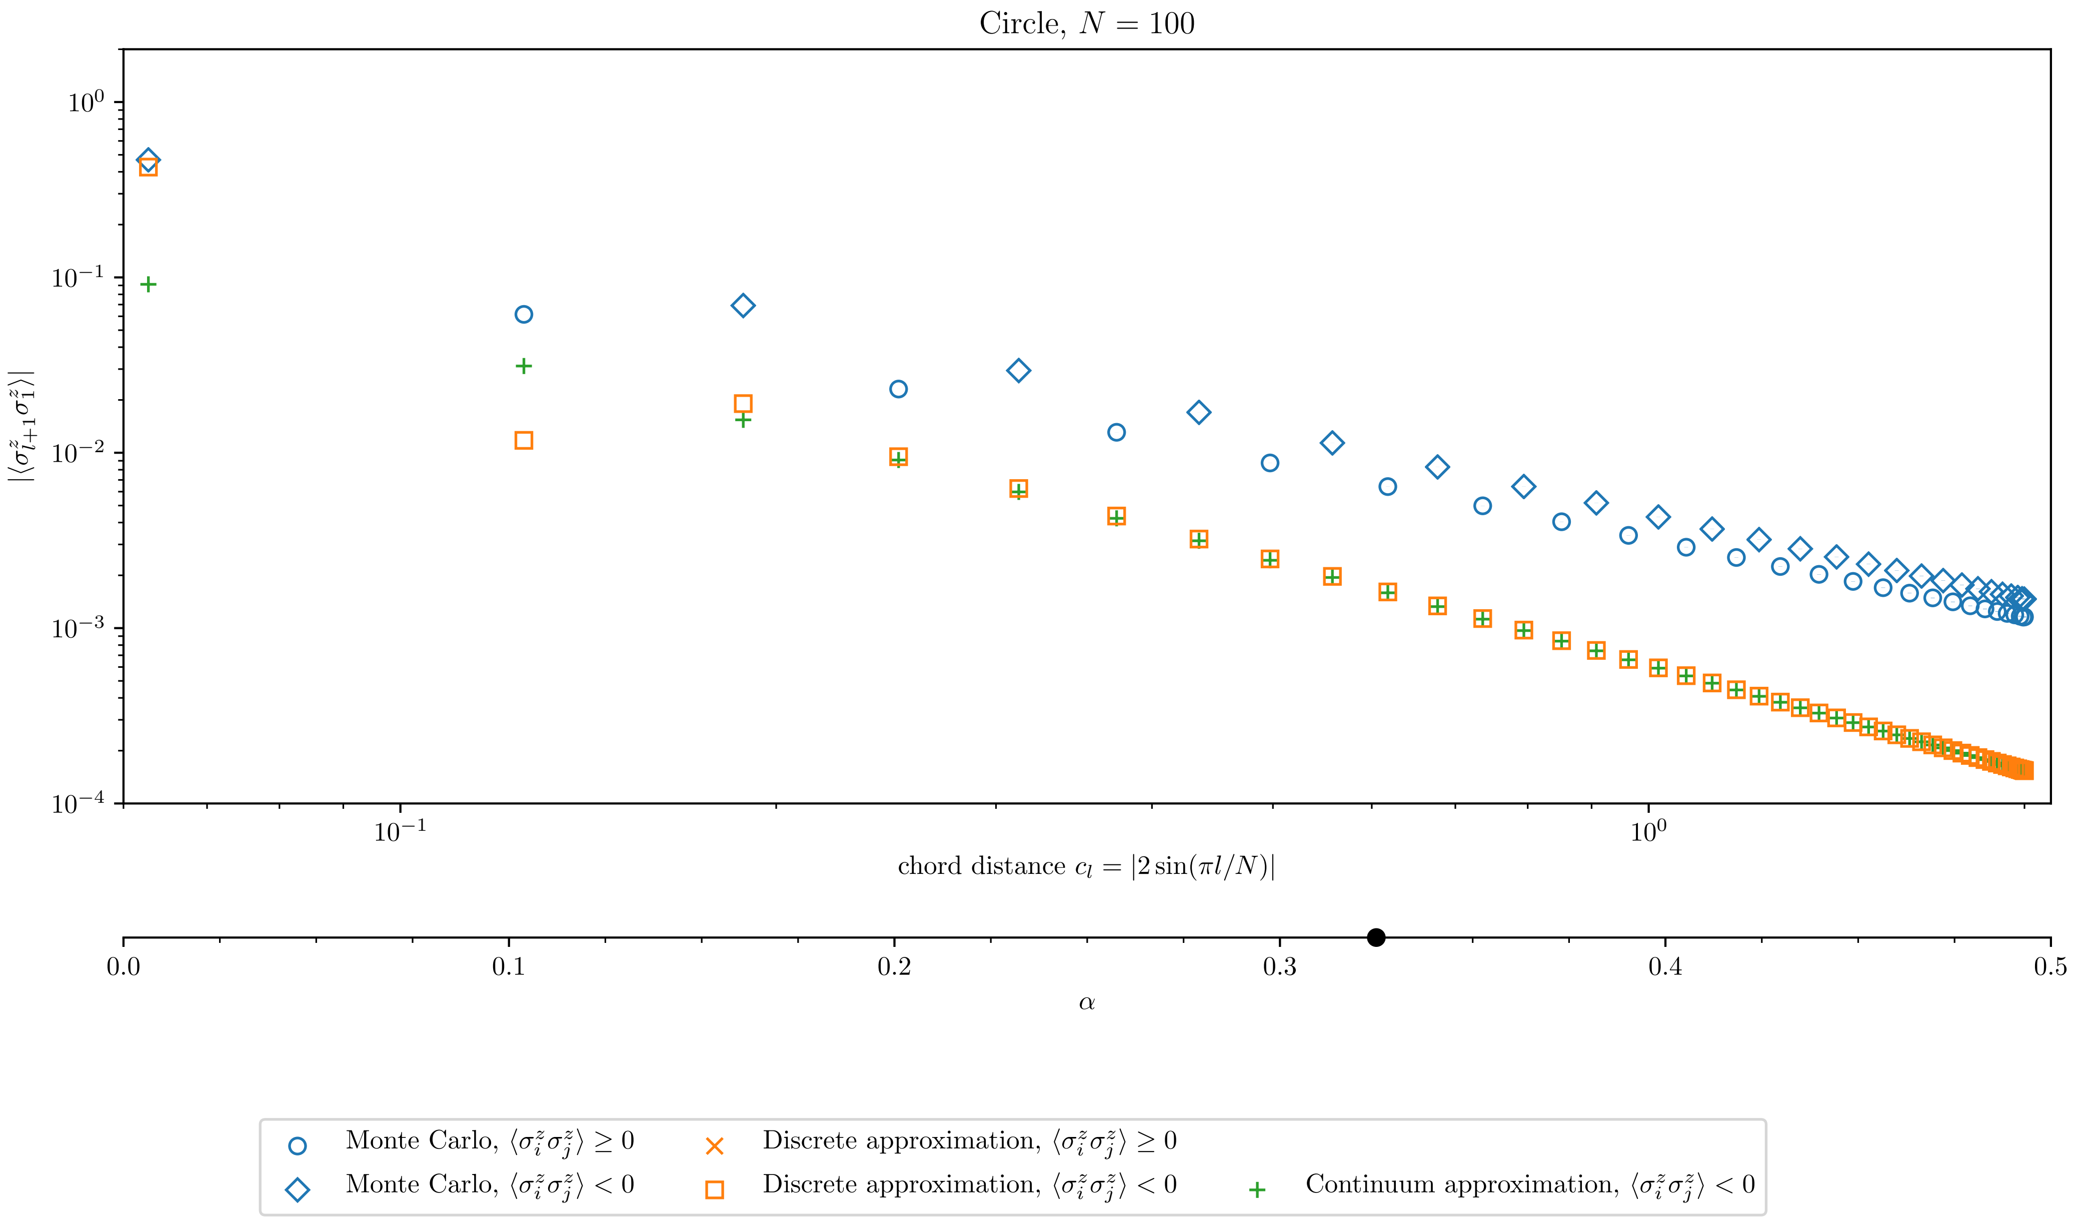

Circle, $N = 100$
$|\langle\sigma^z_{l+1}\sigma^z_1\rangle|$
$10^0$
$10^{-1}$
$10^{-2}$
$10^{-3}$
$10^{-4}$
$10^{-1}$
$10^0$
chord distance $c_l = |2\sin(\pi l/N)|$
0.0
0.1
0.2
0.3
0.4
0.5
$\alpha$
Monte Carlo, $\langle\sigma^z_i\sigma^z_j\rangle \geq 0$
Monte Carlo, $\langle\sigma^z_i\sigma^z_j\rangle < 0$
Discrete approximation, $\langle\sigma^z_i\sigma^z_j\rangle \geq 0$
Discrete approximation, $\langle\sigma^z_i\sigma^z_j\rangle < 0$
Continuum approximation, $\langle\sigma^z_i\sigma^z_j\rangle < 0$

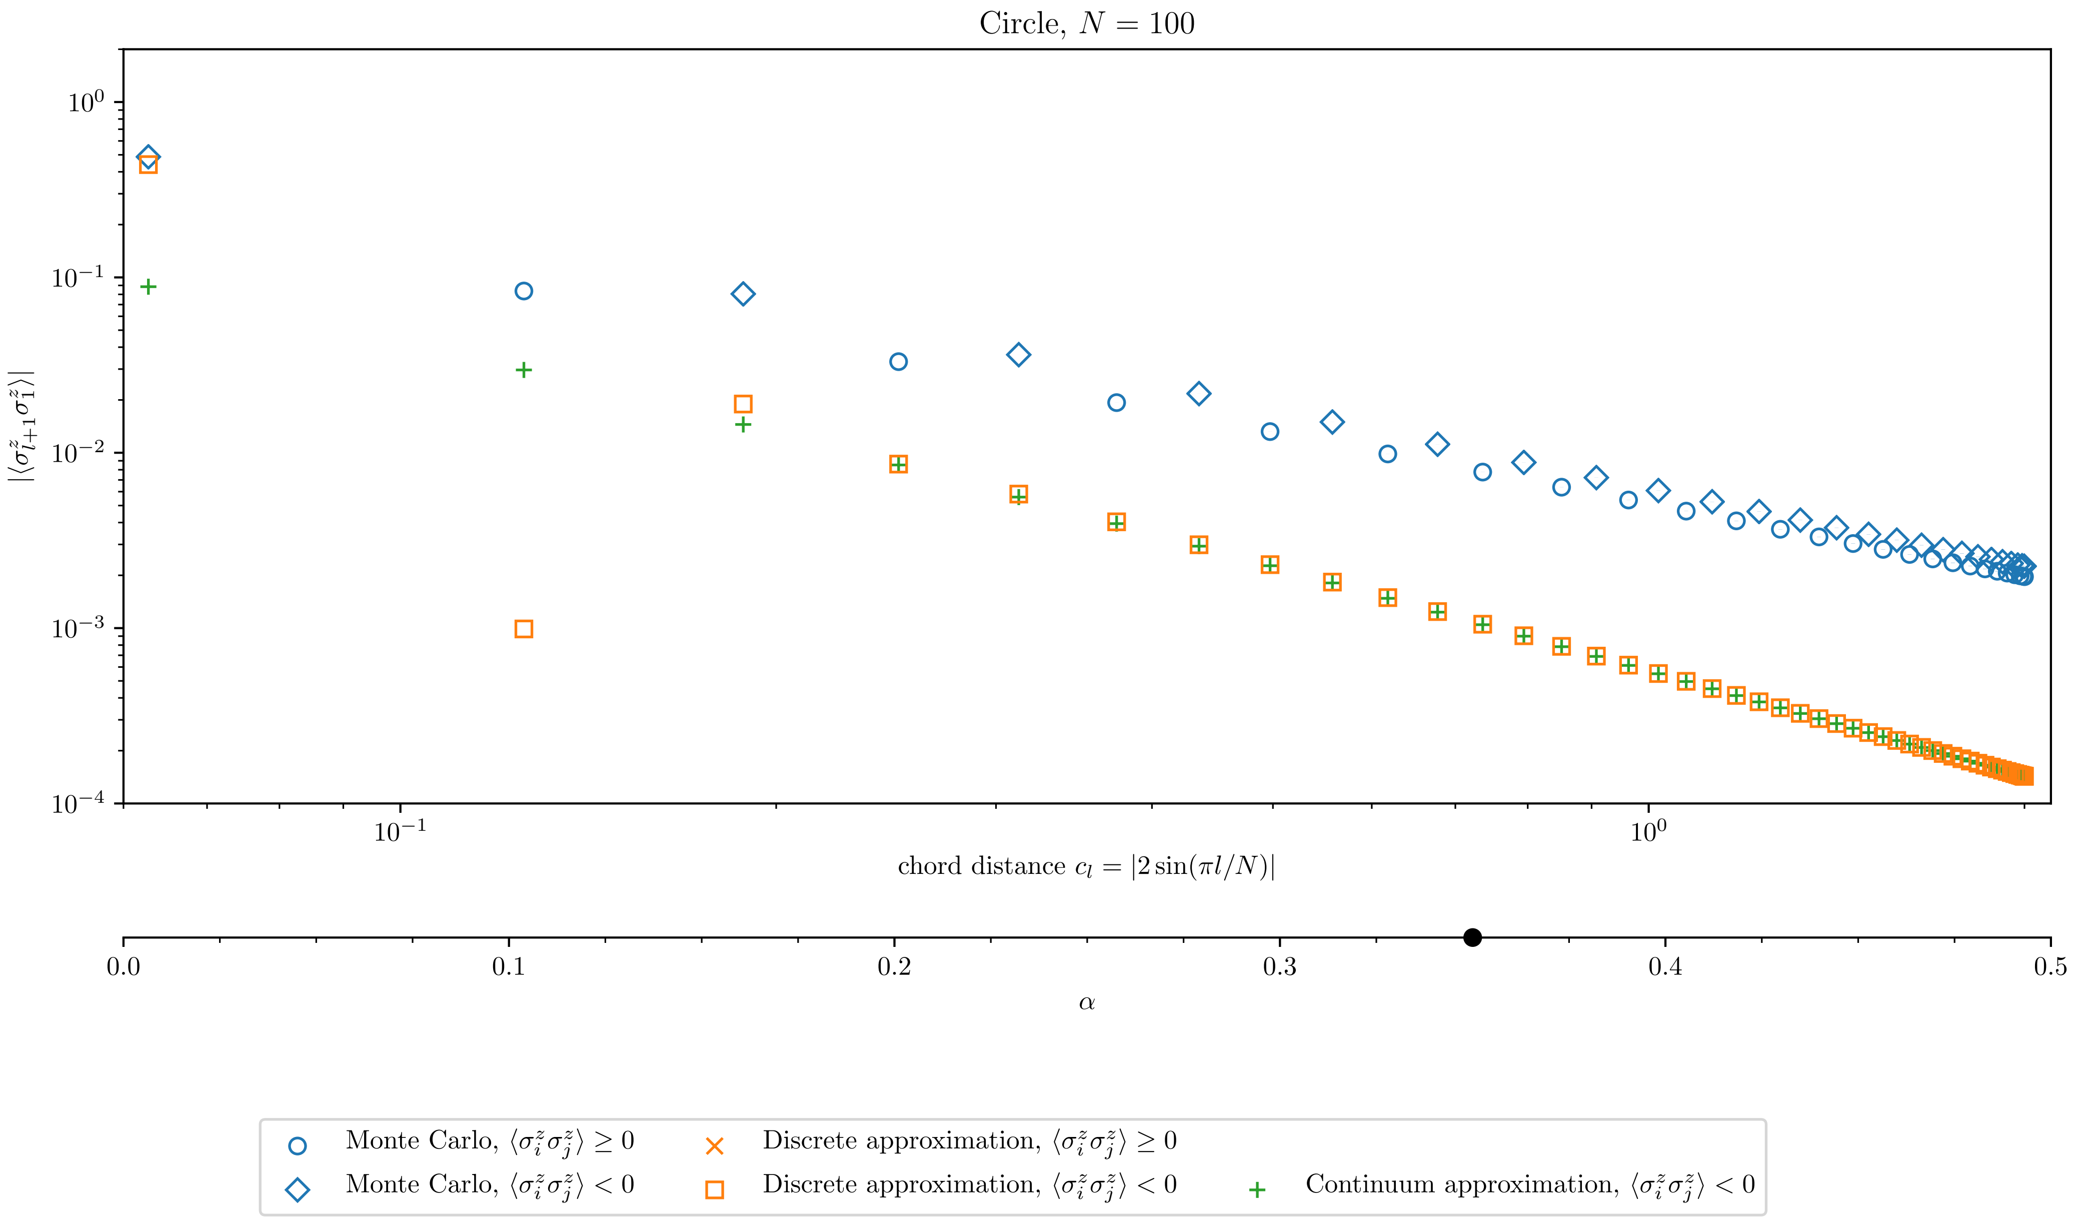

Circle, $N = 100$
$|\langle \sigma^z_{l+1} \sigma^z_1 \rangle|$
$10^0$
$10^{-1}$
$10^{-2}$
$10^{-3}$
$10^{-4}$
$10^{-1}$
$10^0$
chord distance $c_l = |2\sin(\pi l/N)|$
0.0
0.1
0.2
0.3
0.4
0.5
$\alpha$
Monte Carlo, $\langle \sigma^z_i \sigma^z_j \rangle \geq 0$
Monte Carlo, $\langle \sigma^z_i \sigma^z_j \rangle < 0$
Discrete approximation, $\langle \sigma^z_i \sigma^z_j \rangle \geq 0$
Discrete approximation, $\langle \sigma^z_i \sigma^z_j \rangle < 0$
Continuum approximation, $\langle \sigma^z_i \sigma^z_j \rangle < 0$

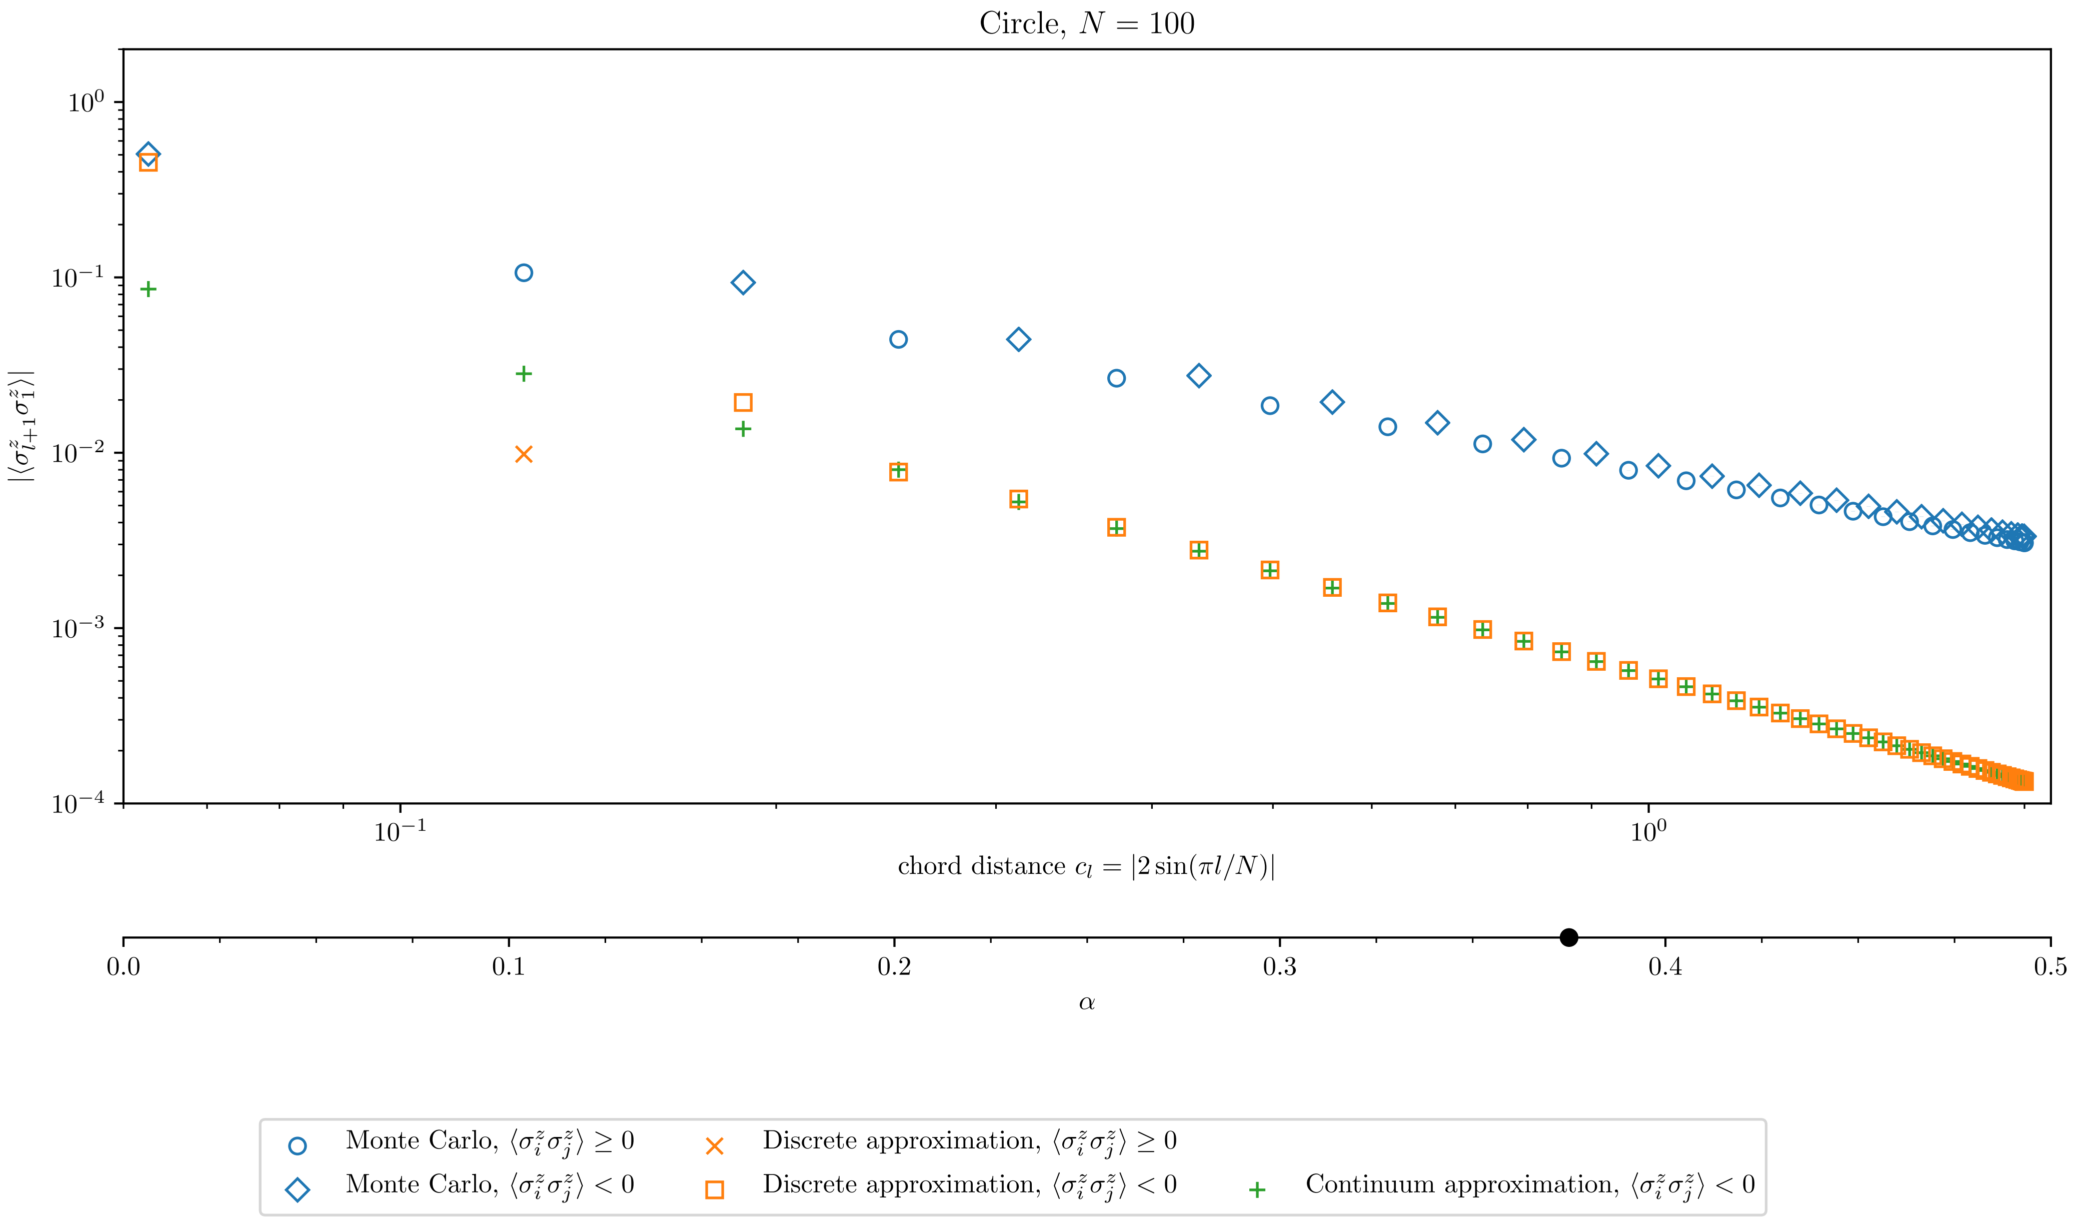
Circle, $N = 100$
$|\langle\sigma^z_{l+1}\sigma^z_1\rangle|$
chord distance $c_l = |2\sin(\pi l/N)|$
$\alpha$
Monte Carlo, $\langle\sigma^z_i\sigma^z_j\rangle \geq 0$
Monte Carlo, $\langle\sigma^z_i\sigma^z_j\rangle < 0$
Discrete approximation, $\langle\sigma^z_i\sigma^z_j\rangle \geq 0$
Discrete approximation, $\langle\sigma^z_i\sigma^z_j\rangle < 0$
Continuum approximation, $\langle\sigma^z_i\sigma^z_j\rangle < 0$

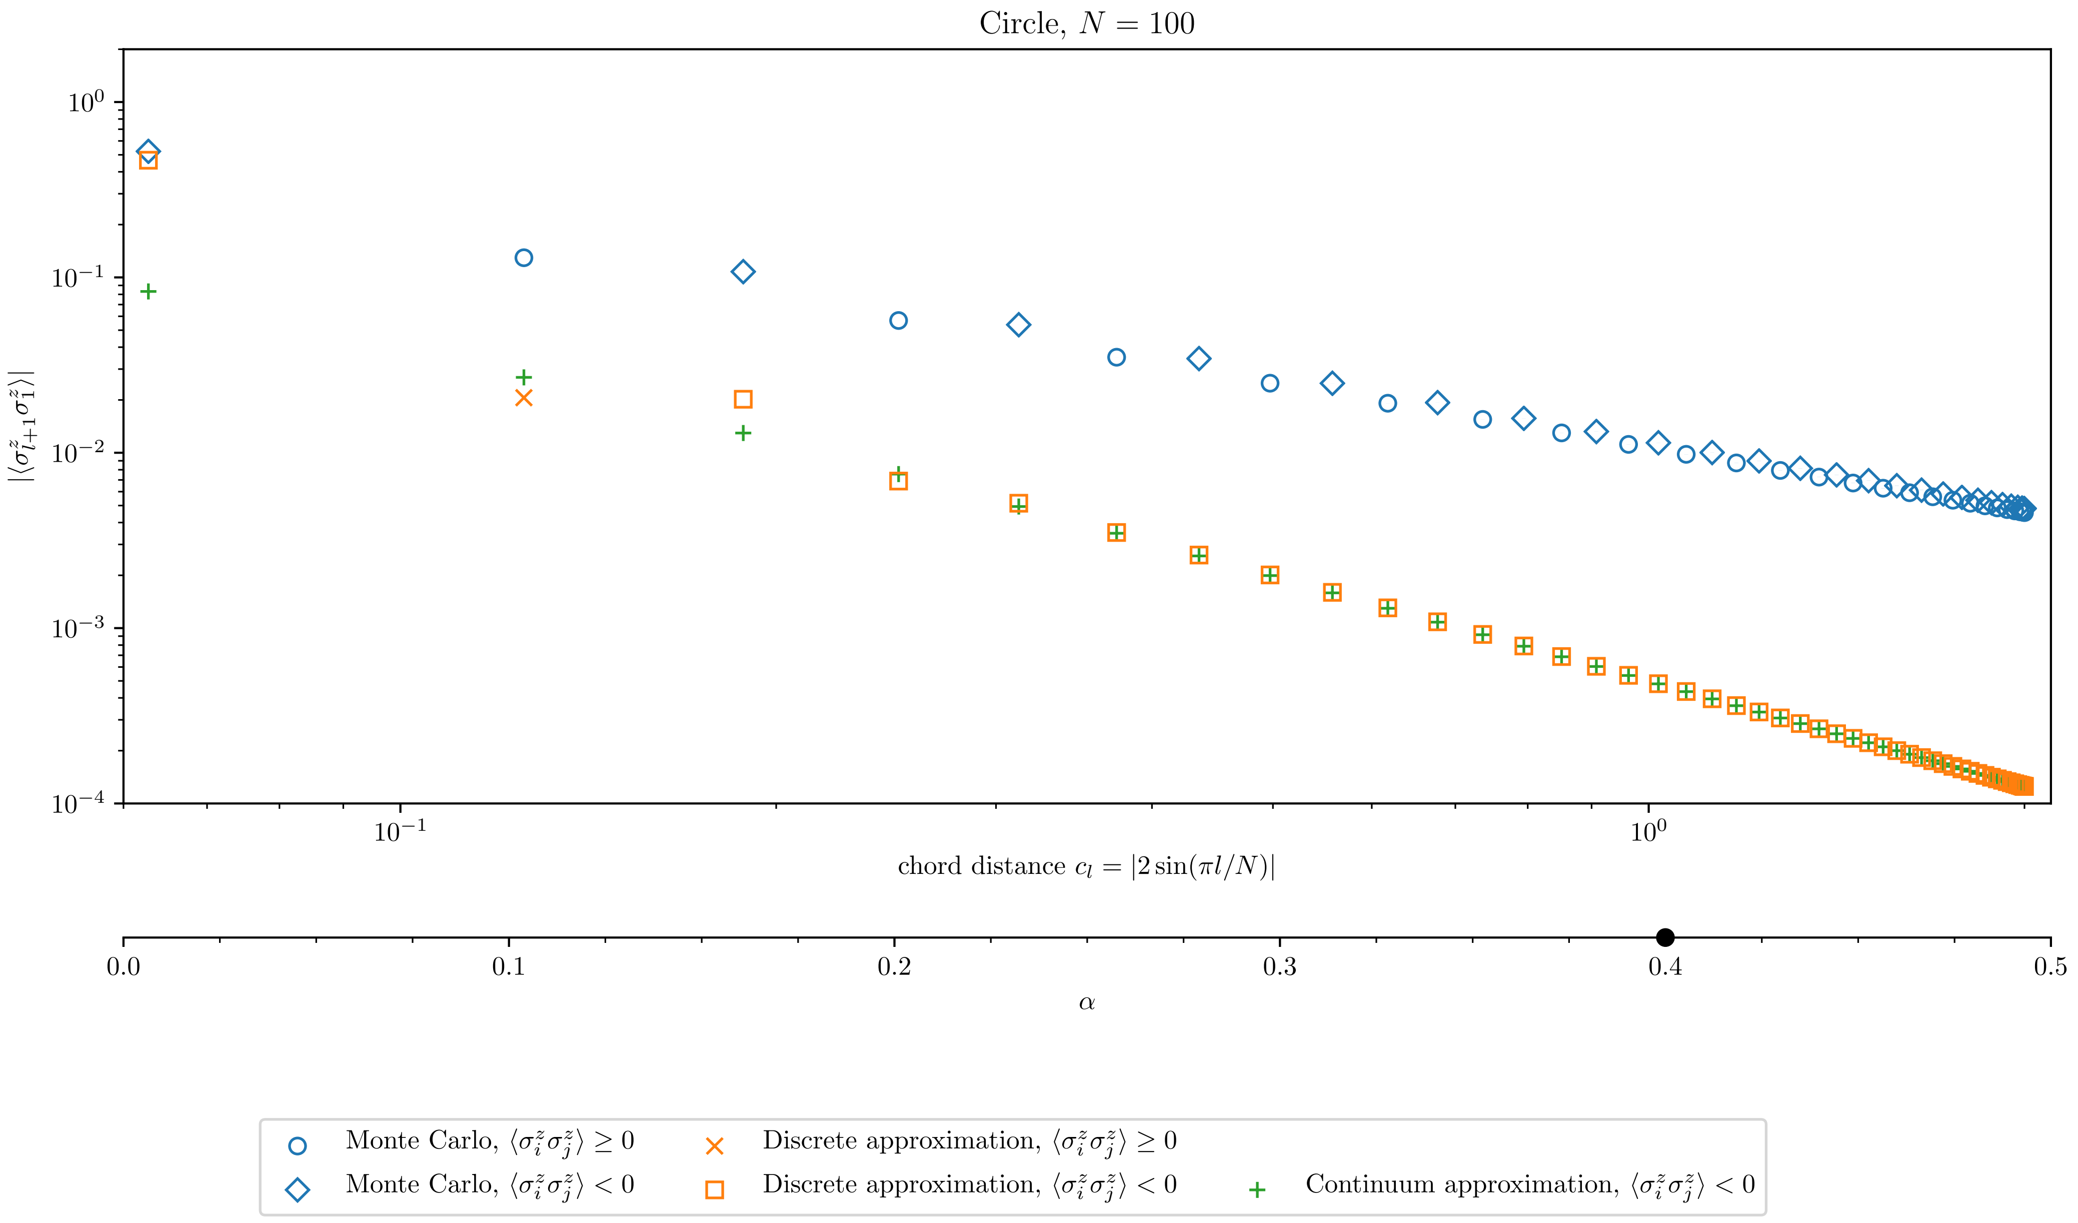
Circle, $N = 100$
$|\langle\sigma^z_{l+1}\sigma^z_1\rangle|$
$10^0$
$10^{-1}$
$10^{-2}$
$10^{-3}$
$10^{-4}$
$10^{-1}$
$10^0$
chord distance $c_l = |2\sin(\pi l/N)|$
0.0
0.1
0.2
0.3
0.4
0.5
$\alpha$
Monte Carlo, $\langle\sigma^z_i\sigma^z_j\rangle \geq 0$
Monte Carlo, $\langle\sigma^z_i\sigma^z_j\rangle < 0$
Discrete approximation, $\langle\sigma^z_i\sigma^z_j\rangle \geq 0$
Discrete approximation, $\langle\sigma^z_i\sigma^z_j\rangle < 0$
Continuum approximation, $\langle\sigma^z_i\sigma^z_j\rangle < 0$

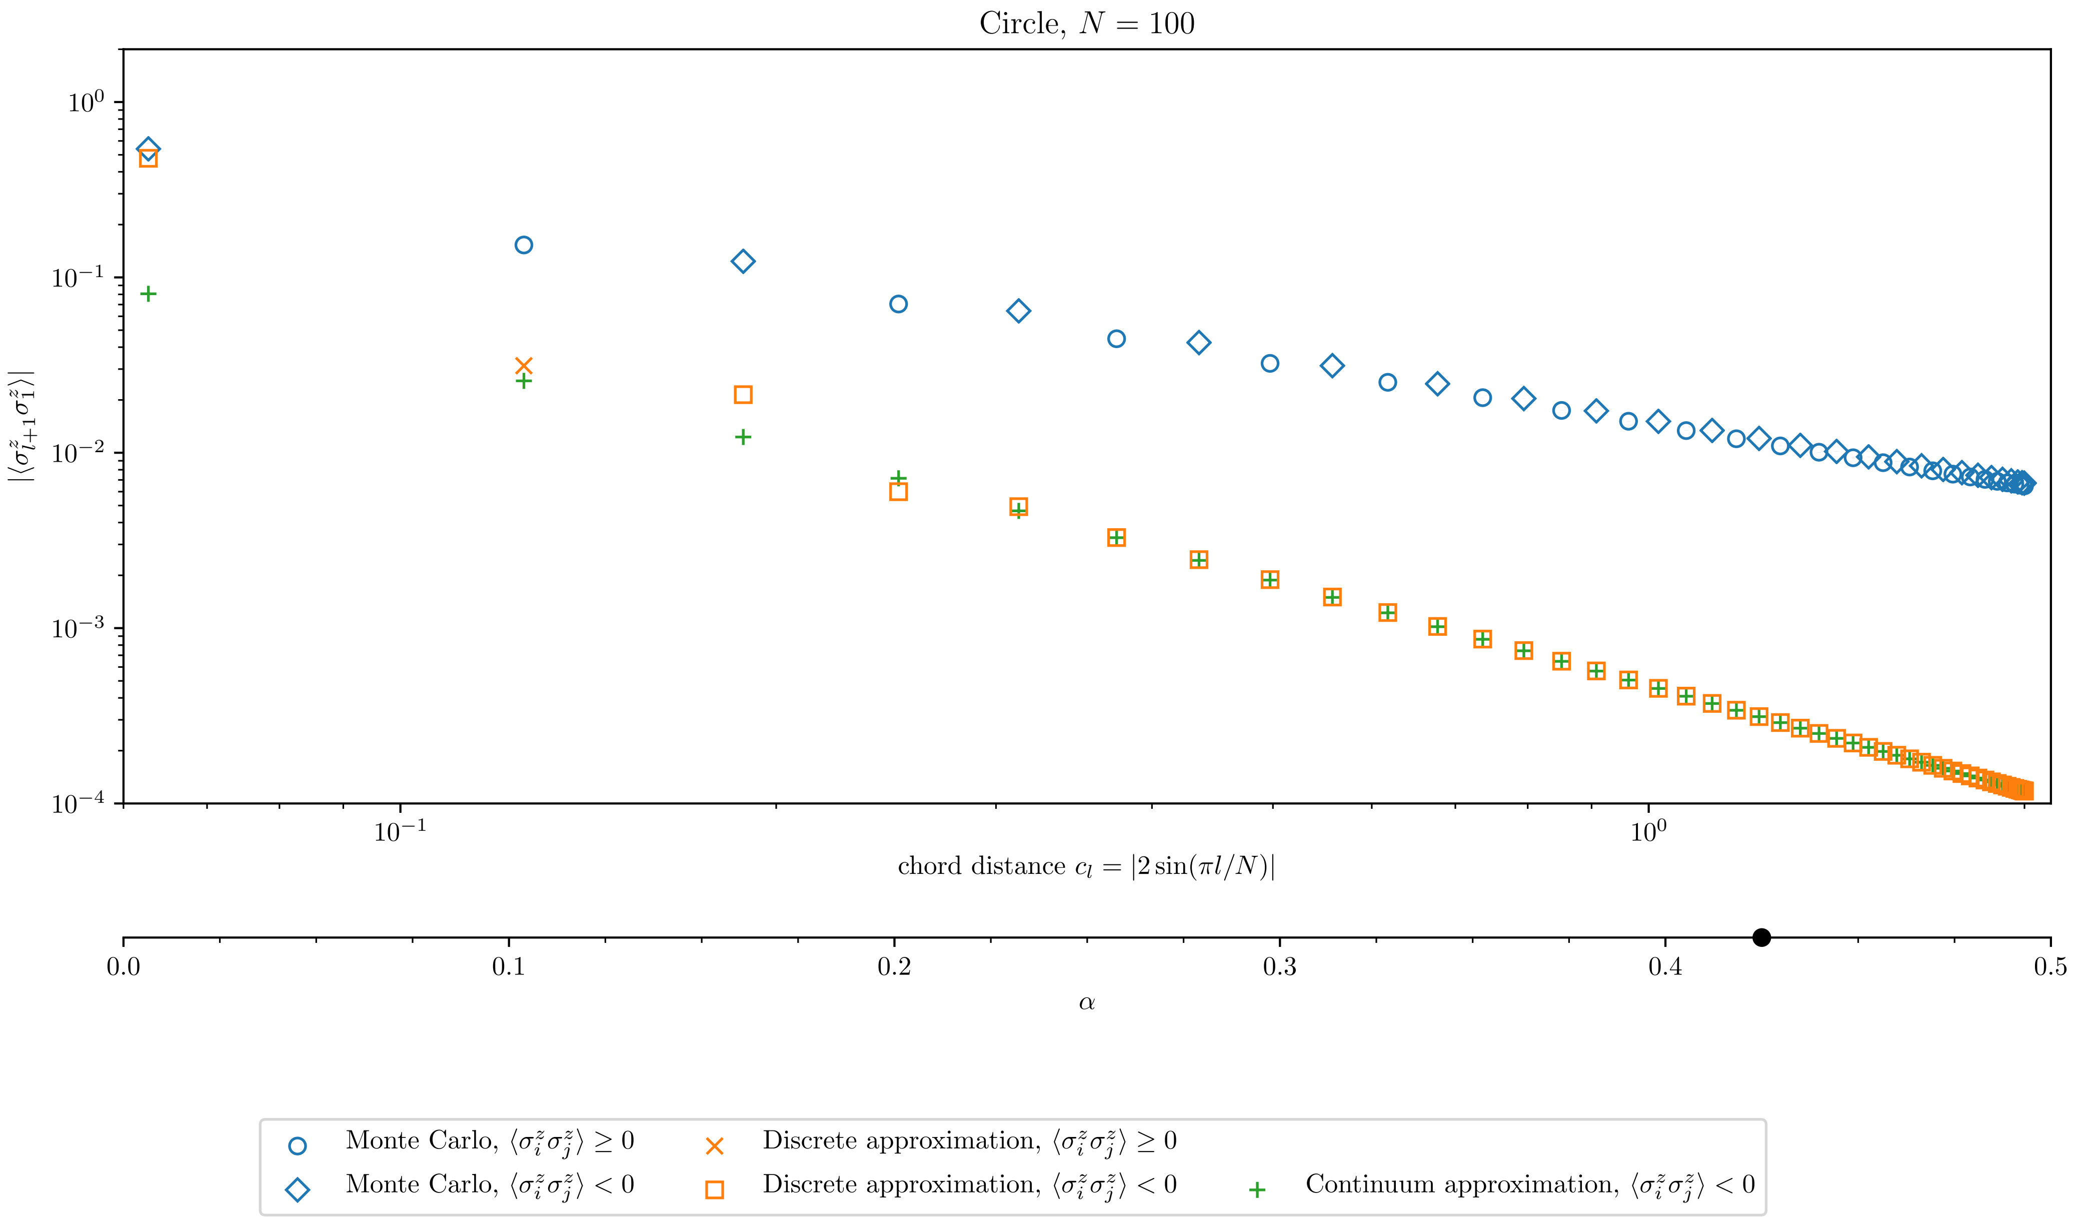

Circle, $N = 100$
$|\langle\sigma^z_{l+1}\sigma^z_1\rangle|$
$10^0$
$10^{-1}$
$10^{-2}$
$10^{-3}$
$10^{-4}$
$10^{-1}$
$10^0$
chord distance $c_l = |2\sin(\pi l/N)|$
0.0
0.1
0.2
0.3
0.4
0.5
$\alpha$
Monte Carlo, $\langle\sigma^z_i\sigma^z_j\rangle \geq 0$
Monte Carlo, $\langle\sigma^z_i\sigma^z_j\rangle < 0$
Discrete approximation, $\langle\sigma^z_i\sigma^z_j\rangle \geq 0$
Discrete approximation, $\langle\sigma^z_i\sigma^z_j\rangle < 0$
Continuum approximation, $\langle\sigma^z_i\sigma^z_j\rangle < 0$

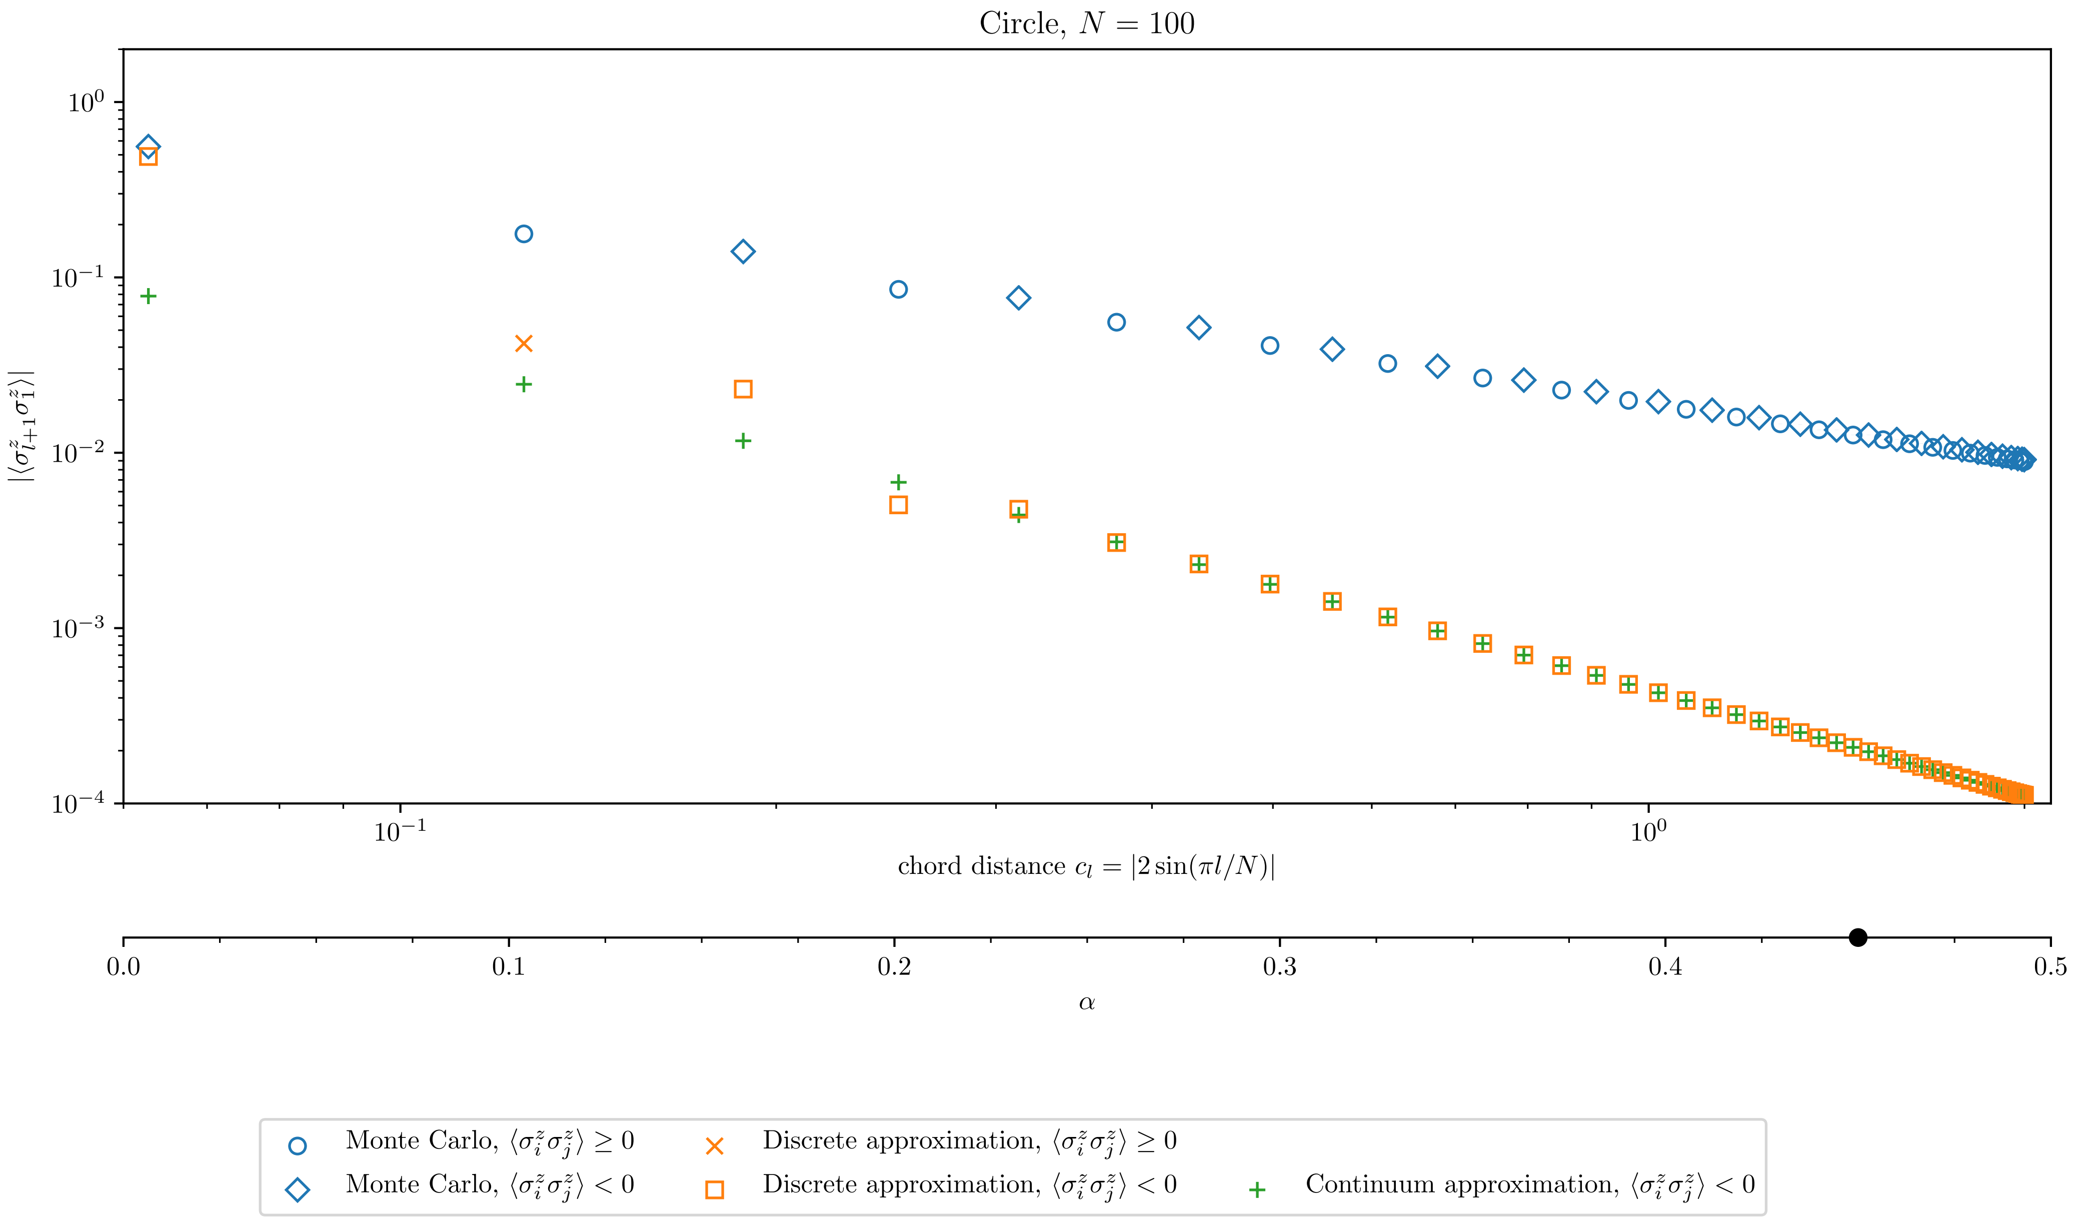
Circle, $N = 100$
$|\langle\sigma^z_{l+1}\sigma^z_1\rangle|$
$10^0$
$10^{-1}$
$10^{-2}$
$10^{-3}$
$10^{-4}$
$10^{-1}$
$10^0$
chord distance $c_l = |2\sin(\pi l/N)|$
0.0
0.1
0.2
0.3
0.4
0.5
$\alpha$
Monte Carlo, $\langle\sigma^z_i\sigma^z_j\rangle \geq 0$
Monte Carlo, $\langle\sigma^z_i\sigma^z_j\rangle < 0$
Discrete approximation, $\langle\sigma^z_i\sigma^z_j\rangle \geq 0$
Discrete approximation, $\langle\sigma^z_i\sigma^z_j\rangle < 0$
Continuum approximation, $\langle\sigma^z_i\sigma^z_j\rangle < 0$

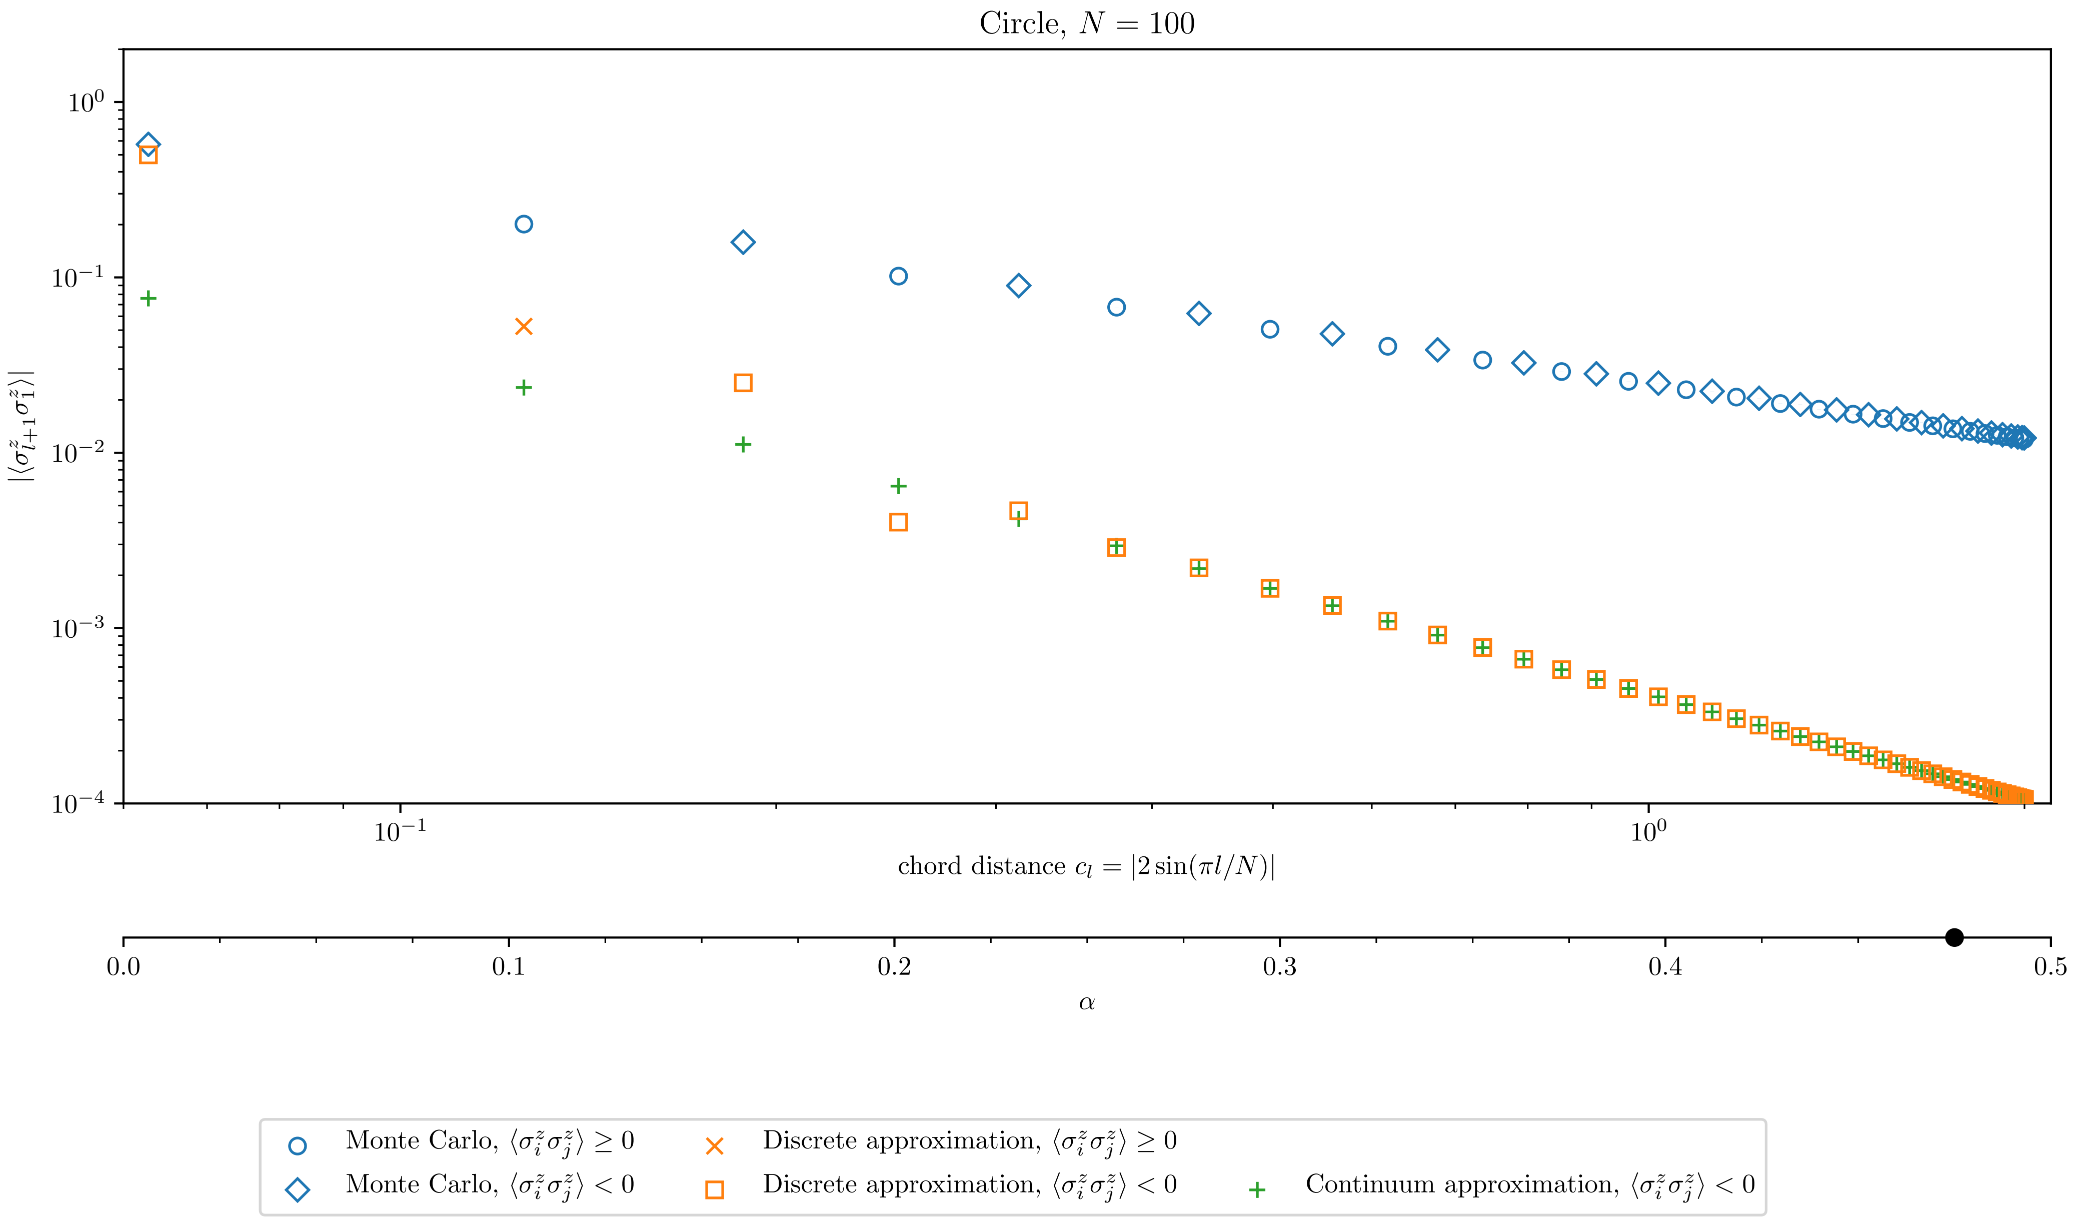

Circle, $N = 100$
$|\langle\sigma^z_{l+1}\sigma^z_1\rangle|$
$10^0$
$10^{-1}$
$10^{-2}$
$10^{-3}$
$10^{-4}$
$10^{-1}$
$10^0$
chord distance $c_l = |2\sin(\pi l/N)|$
0.0
0.1
0.2
0.3
0.4
0.5
$\alpha$
Monte Carlo, $\langle\sigma^z_i\sigma^z_j\rangle \geq 0$
Discrete approximation, $\langle\sigma^z_i\sigma^z_j\rangle \geq 0$
Monte Carlo, $\langle\sigma^z_i\sigma^z_j\rangle < 0$
Discrete approximation, $\langle\sigma^z_i\sigma^z_j\rangle < 0$
Continuum approximation, $\langle\sigma^z_i\sigma^z_j\rangle < 0$

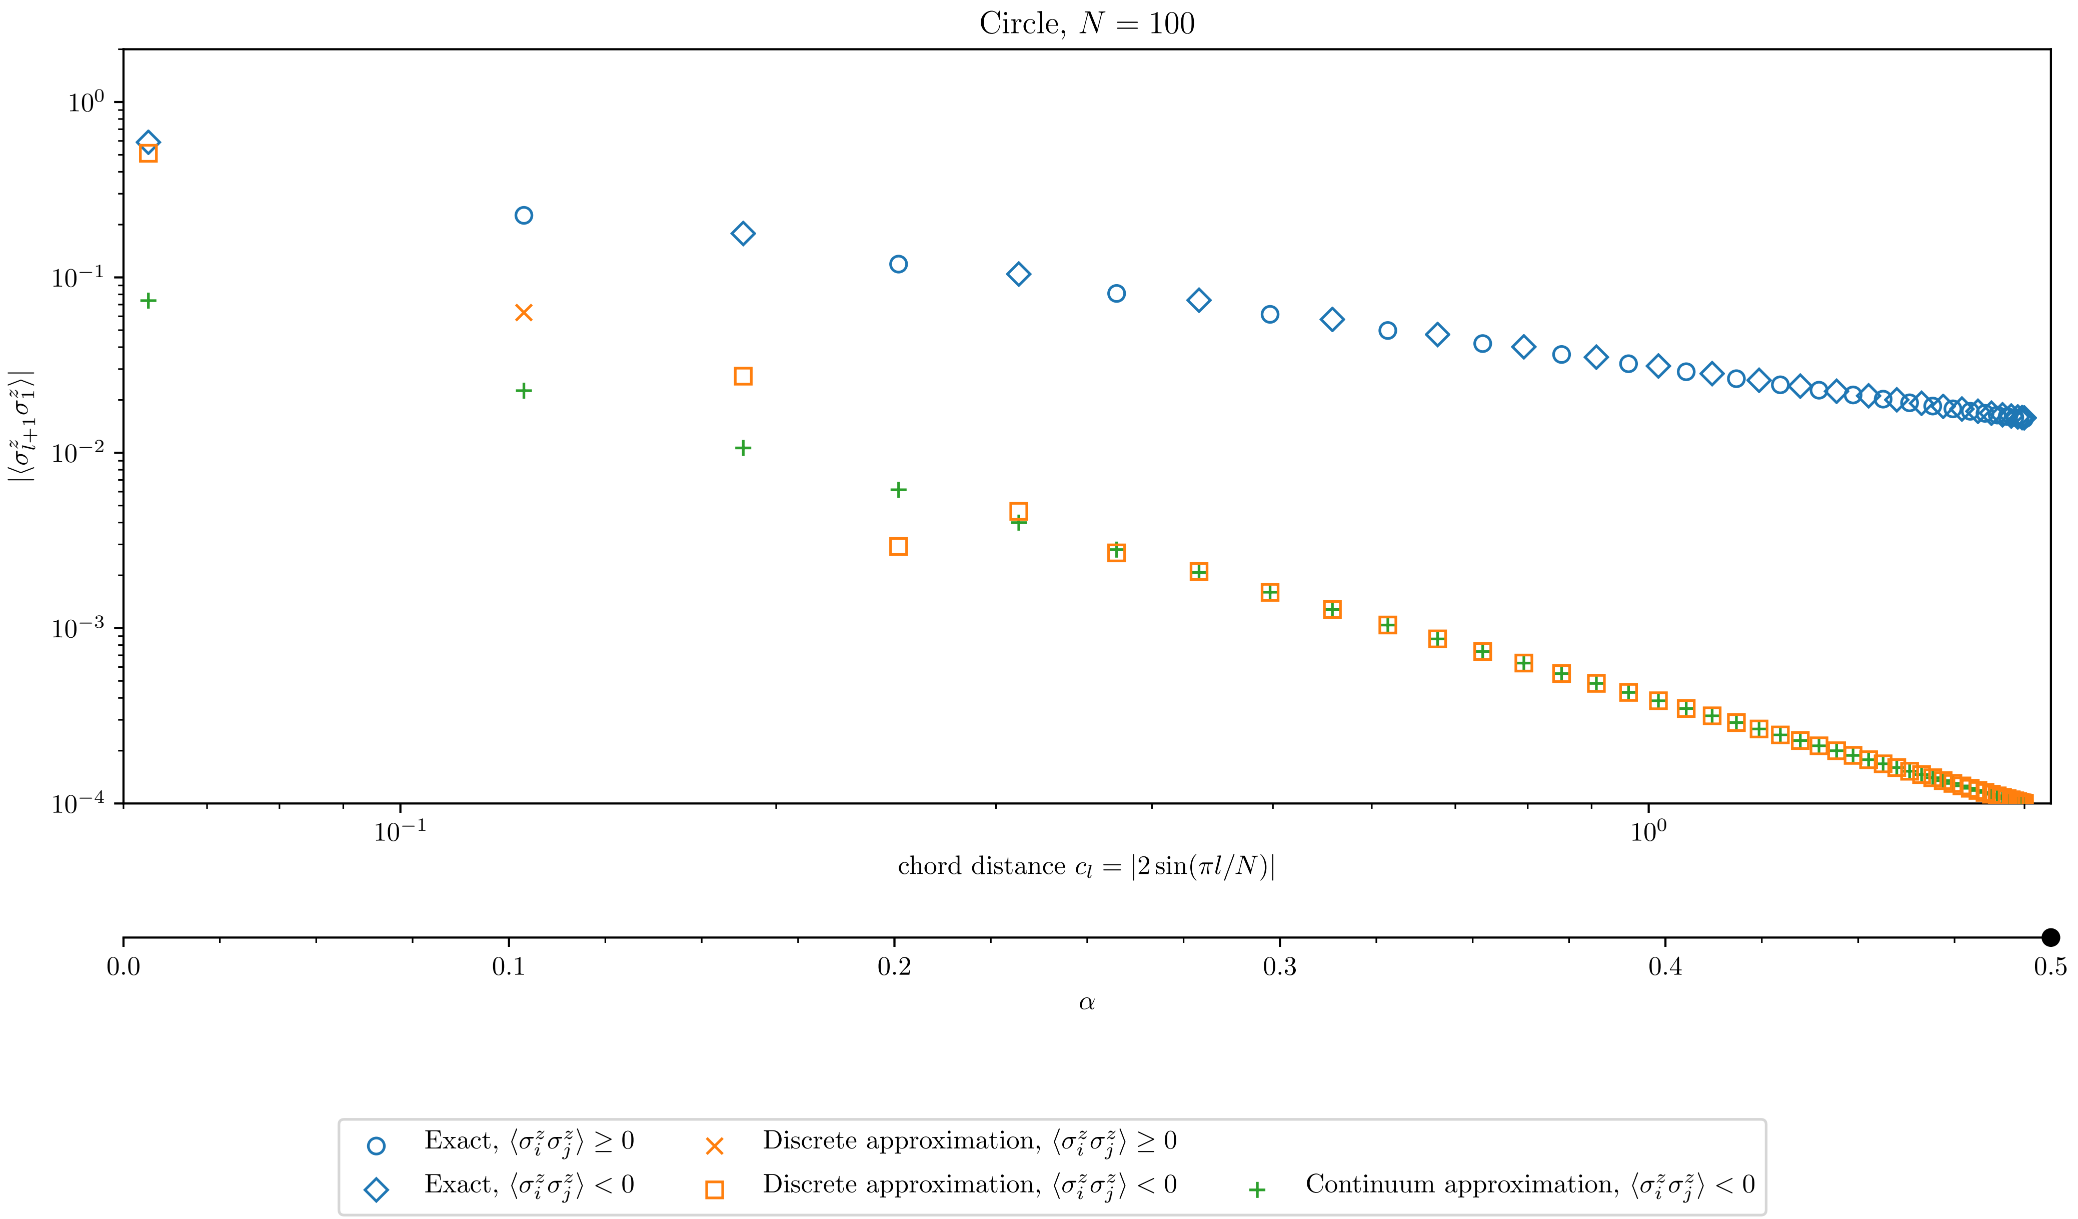

Circle, $N = 100$
$|\langle\sigma^z_{l+1}\sigma^z_1\rangle|$
$10^0$
$10^{-1}$
$10^{-2}$
$10^{-3}$
$10^{-4}$
chord distance $c_l = |2\sin(\pi l/N)|$
0.0
0.1
0.2
0.3
0.4
0.5
$\alpha$
Exact, $\langle\sigma^z_i\sigma^z_j\rangle \geq 0$
Exact, $\langle\sigma^z_i\sigma^z_j\rangle < 0$
Discrete approximation, $\langle\sigma^z_i\sigma^z_j\rangle \geq 0$
Discrete approximation, $\langle\sigma^z_i\sigma^z_j\rangle < 0$
Continuum approximation, $\langle\sigma^z_i\sigma^z_j\rangle < 0$

I. Circle

II. Sphere

III. Cylinder (edge)

IV. Cylinder (bulk)

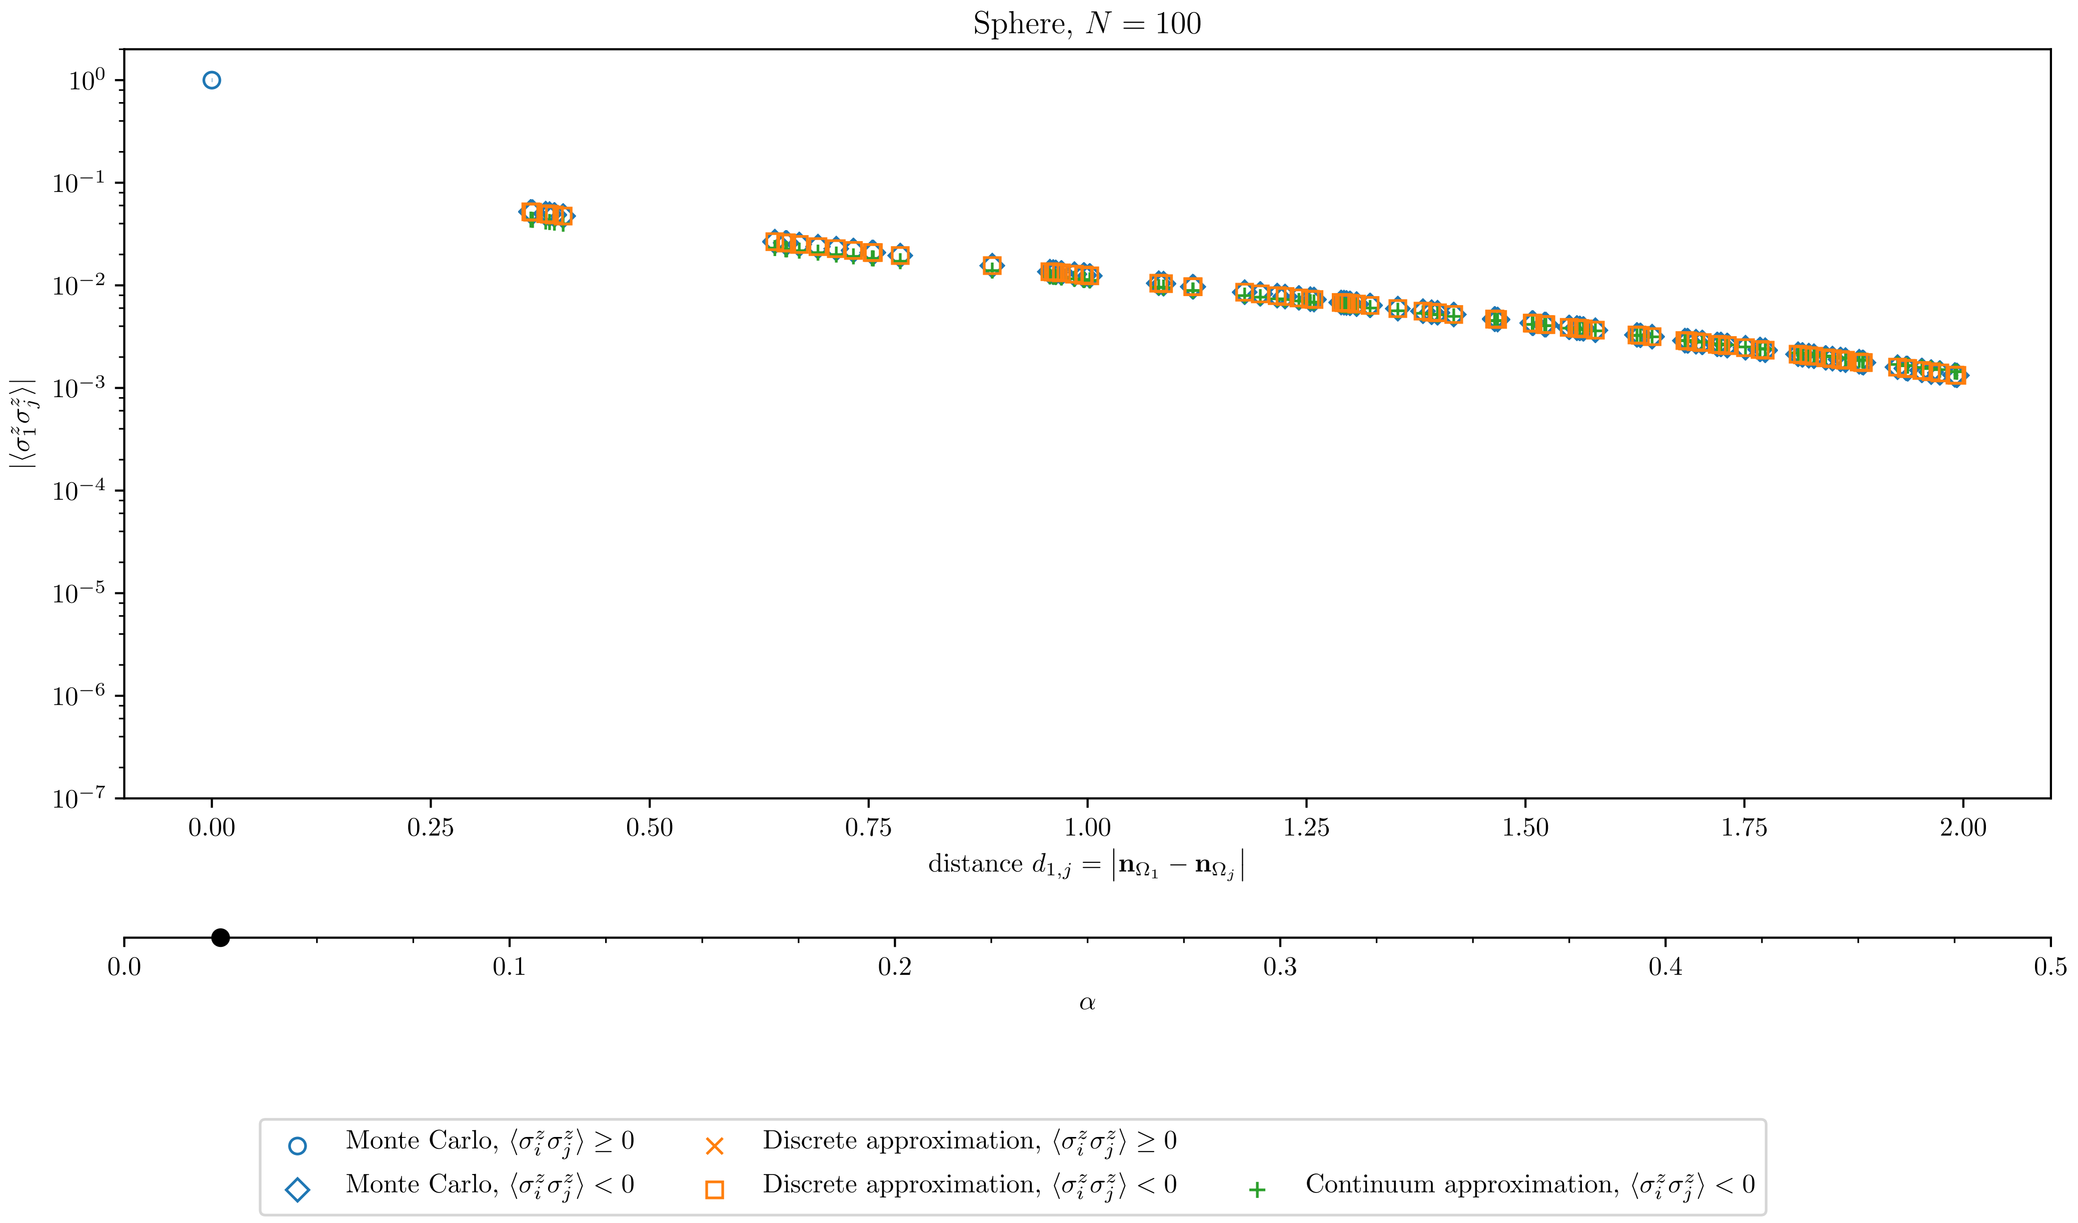

Sphere, $N = 100$
$|\langle\sigma_1^z\sigma_j^z\rangle|$
$10^0$
$10^{-1}$
$10^{-2}$
$10^{-3}$
$10^{-4}$
$10^{-5}$
$10^{-6}$
$10^{-7}$
0.00
0.25
0.50
0.75
1.00
1.25
1.50
1.75
2.00
distance $d_{1,j} = |\mathbf{n}_{\Omega_1} - \mathbf{n}_{\Omega_j}|$
0.0
0.1
0.2
0.3
0.4
0.5
$\alpha$
Monte Carlo, $\langle\sigma_i^z\sigma_j^z\rangle \geq 0$
Discrete approximation, $\langle\sigma_i^z\sigma_j^z\rangle \geq 0$
Monte Carlo, $\langle\sigma_i^z\sigma_j^z\rangle < 0$
Discrete approximation, $\langle\sigma_i^z\sigma_j^z\rangle < 0$
Continuum approximation, $\langle\sigma_i^z\sigma_j^z\rangle < 0$

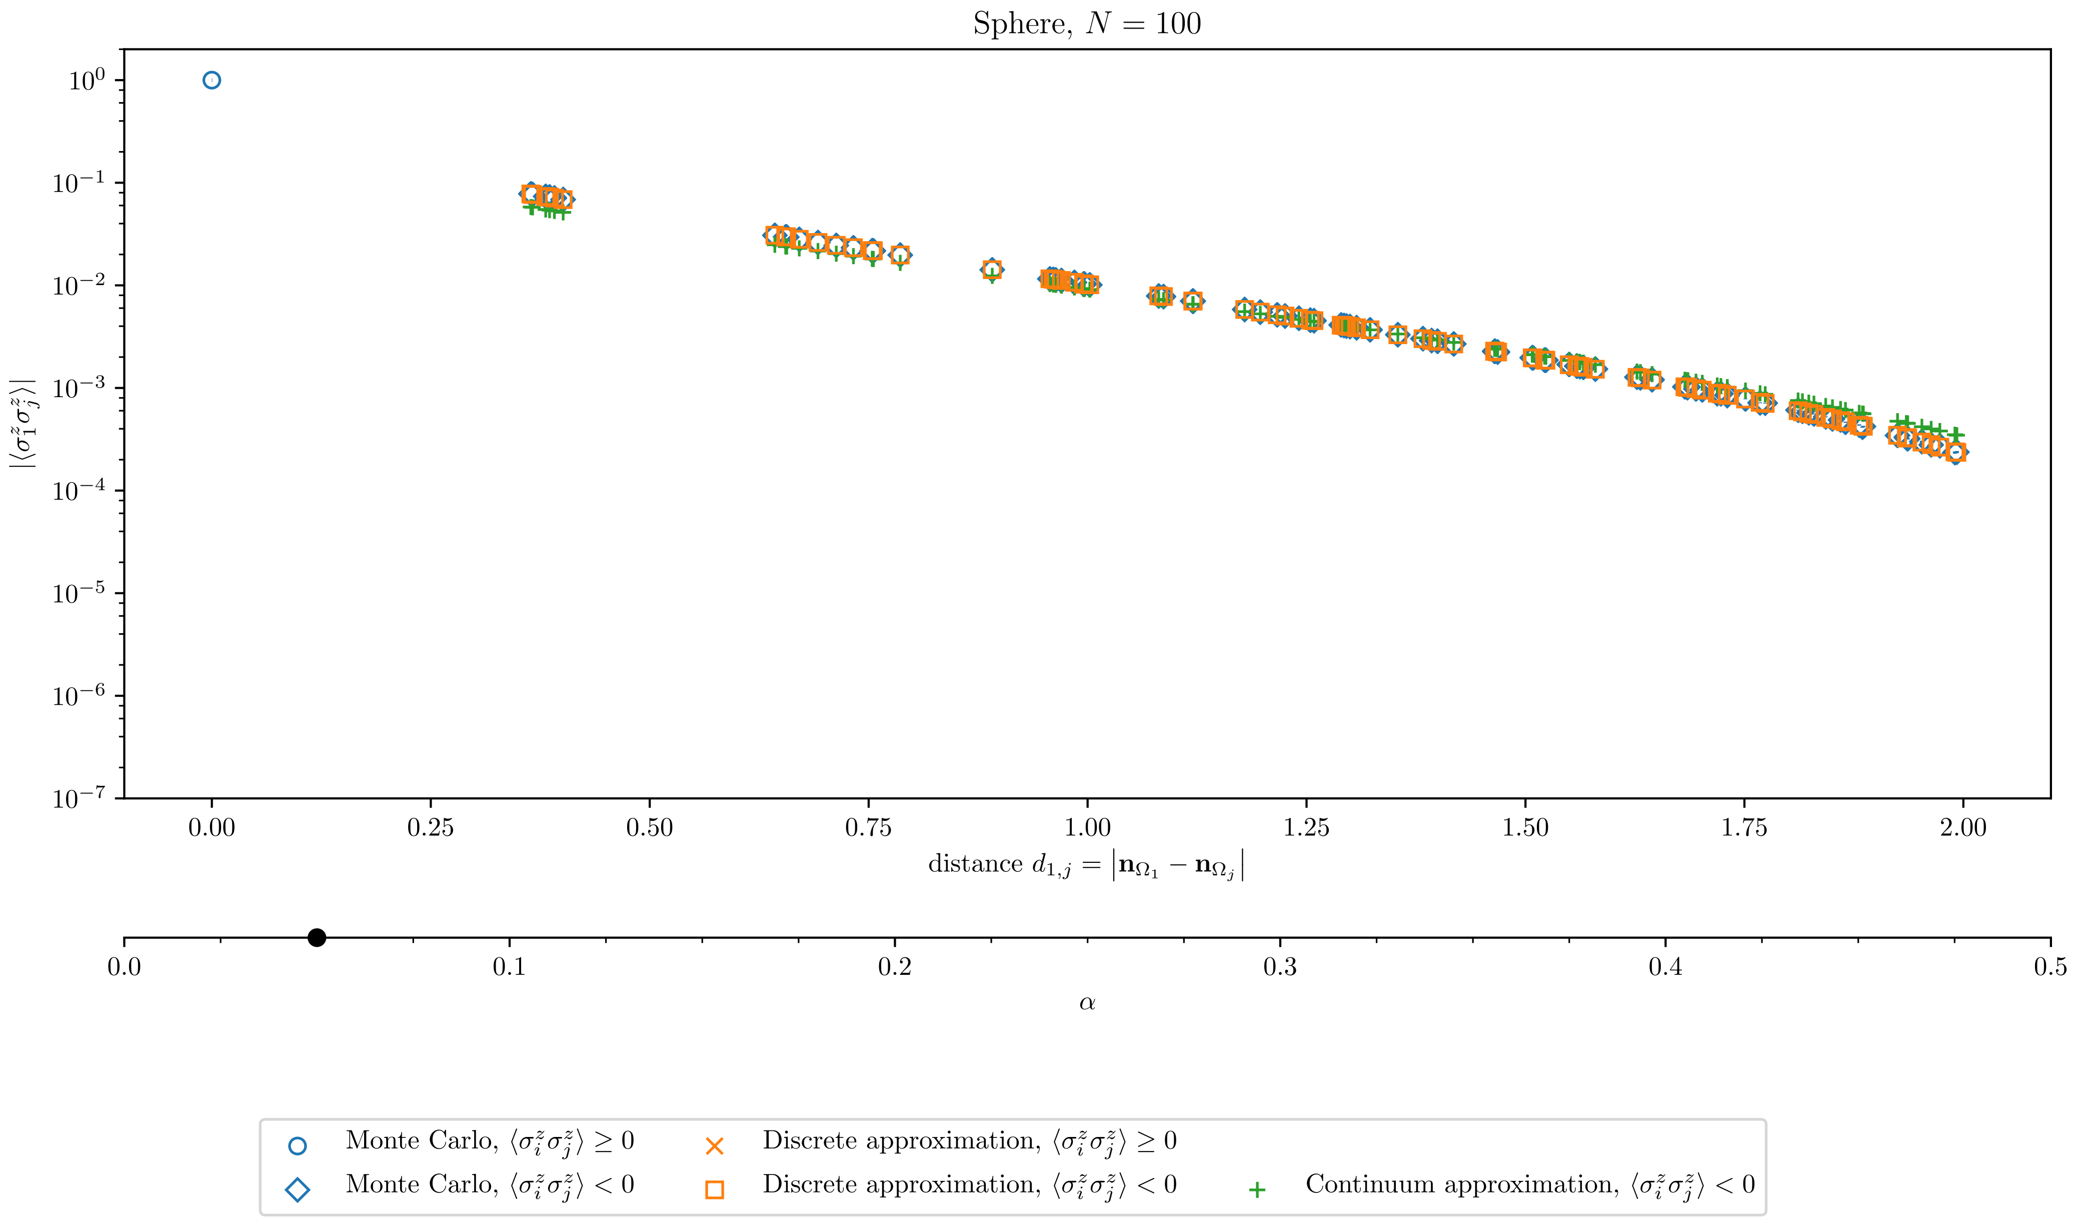

Sphere, $N = 100$
$10^0$
$10^{-1}$
$10^{-2}$
$10^{-3}$
$10^{-4}$
$10^{-5}$
$10^{-6}$
$10^{-7}$
$|\langle \sigma_1^z \sigma_j^z \rangle|$
0.00
0.25
0.50
0.75
1.00
1.25
1.50
1.75
2.00
distance $d_{1,j} = |\mathbf{n}_{\Omega_1} - \mathbf{n}_{\Omega_j}|$
0.0
0.1
0.2
0.3
0.4
0.5
$\alpha$
Monte Carlo, $\langle \sigma_i^z \sigma_j^z \rangle \geq 0$
Monte Carlo, $\langle \sigma_i^z \sigma_j^z \rangle < 0$
Discrete approximation, $\langle \sigma_i^z \sigma_j^z \rangle \geq 0$
Discrete approximation, $\langle \sigma_i^z \sigma_j^z \rangle < 0$
Continuum approximation, $\langle \sigma_i^z \sigma_j^z \rangle < 0$

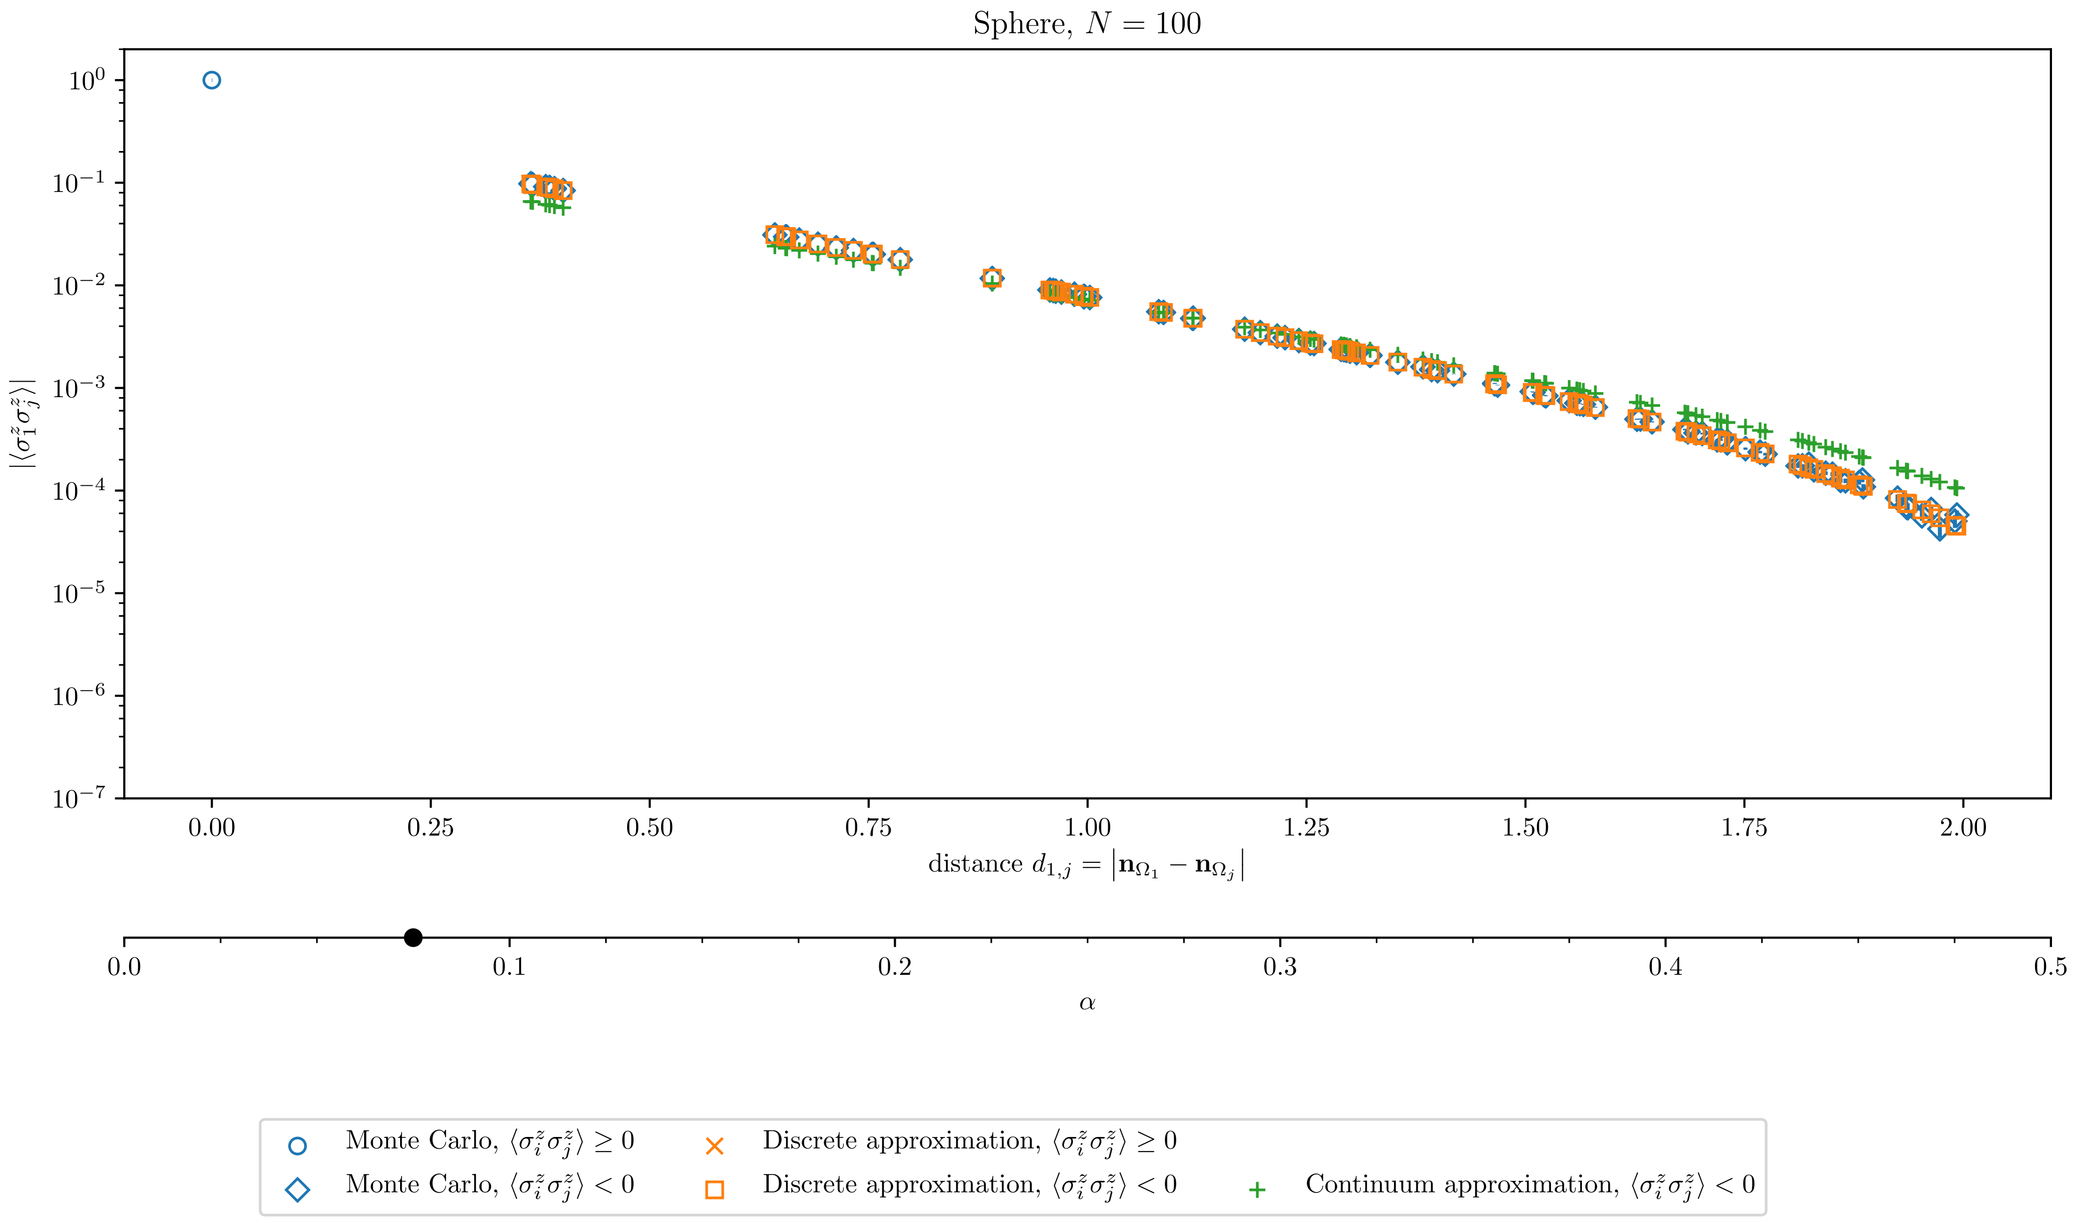

Sphere, $N = 100$
$|\langle\sigma_1^z\sigma_j^z\rangle|$
$10^0$
$10^{-1}$
$10^{-2}$
$10^{-3}$
$10^{-4}$
$10^{-5}$
$10^{-6}$
$10^{-7}$
0.00
0.25
0.50
0.75
1.00
1.25
1.50
1.75
2.00
distance $d_{1,j} = |\mathbf{n}_{\Omega_1} - \mathbf{n}_{\Omega_j}|$
0.0
0.1
0.2
0.3
0.4
0.5
$\alpha$
Monte Carlo, $\langle\sigma_i^z\sigma_j^z\rangle \geq 0$
Monte Carlo, $\langle\sigma_i^z\sigma_j^z\rangle < 0$
Discrete approximation, $\langle\sigma_i^z\sigma_j^z\rangle \geq 0$
Discrete approximation, $\langle\sigma_i^z\sigma_j^z\rangle < 0$
Continuum approximation, $\langle\sigma_i^z\sigma_j^z\rangle < 0$

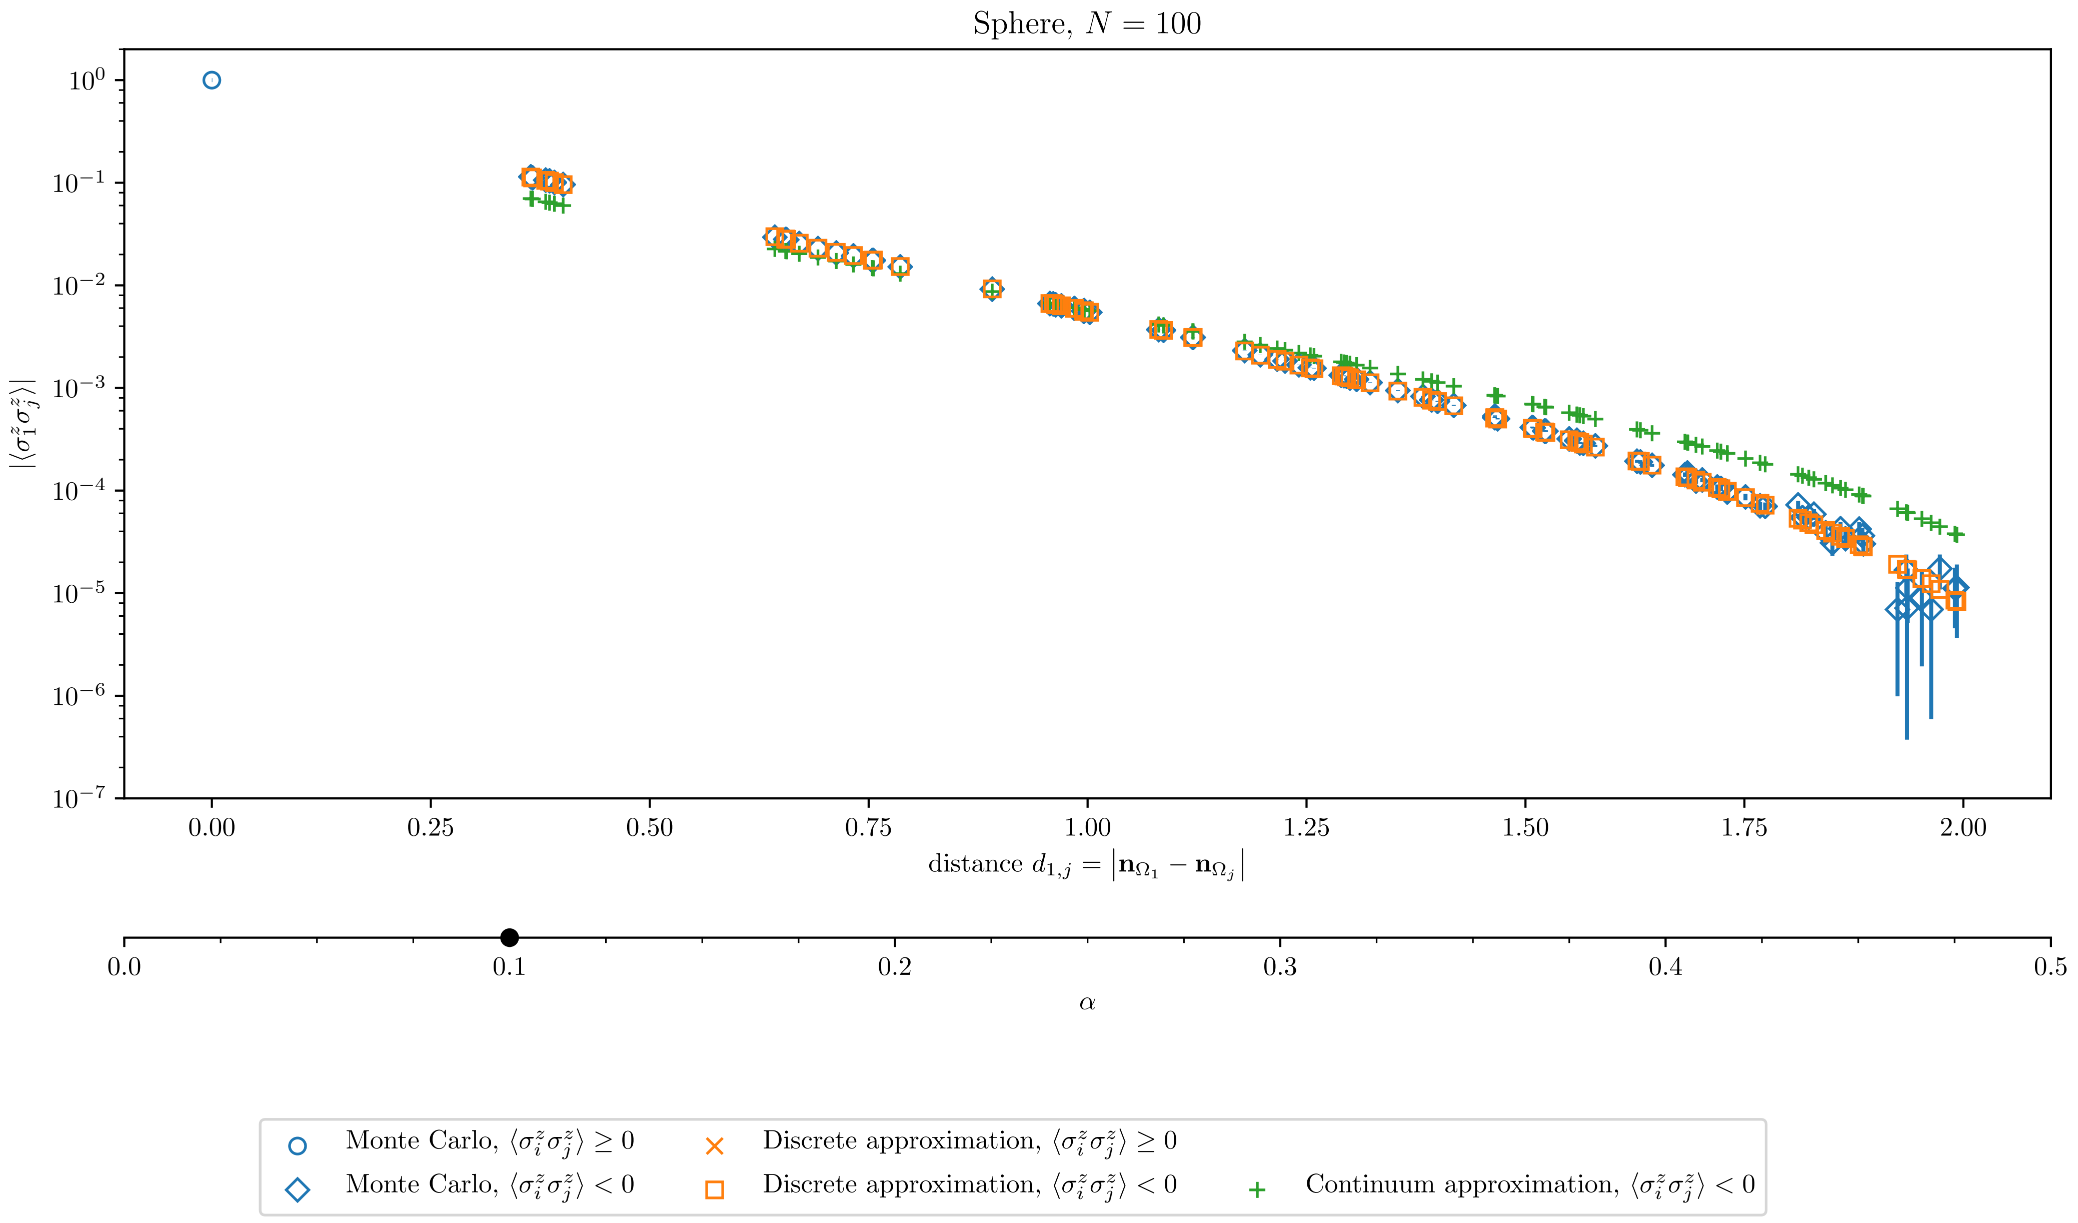

Sphere, $N = 100$
$|\langle\sigma_1^z\sigma_j^z\rangle|$
$10^0$
$10^{-1}$
$10^{-2}$
$10^{-3}$
$10^{-4}$
$10^{-5}$
$10^{-6}$
$10^{-7}$
0.00
0.25
0.50
0.75
1.00
1.25
1.50
1.75
2.00
distance $d_{1,j} = |\mathbf{n}_{\Omega_1} - \mathbf{n}_{\Omega_j}|$
0.0
0.1
0.2
0.3
0.4
0.5
$\alpha$
Monte Carlo, $\langle\sigma_i^z\sigma_j^z\rangle \geq 0$
Monte Carlo, $\langle\sigma_i^z\sigma_j^z\rangle < 0$
Discrete approximation, $\langle\sigma_i^z\sigma_j^z\rangle \geq 0$
Discrete approximation, $\langle\sigma_i^z\sigma_j^z\rangle < 0$
Continuum approximation, $\langle\sigma_i^z\sigma_j^z\rangle < 0$

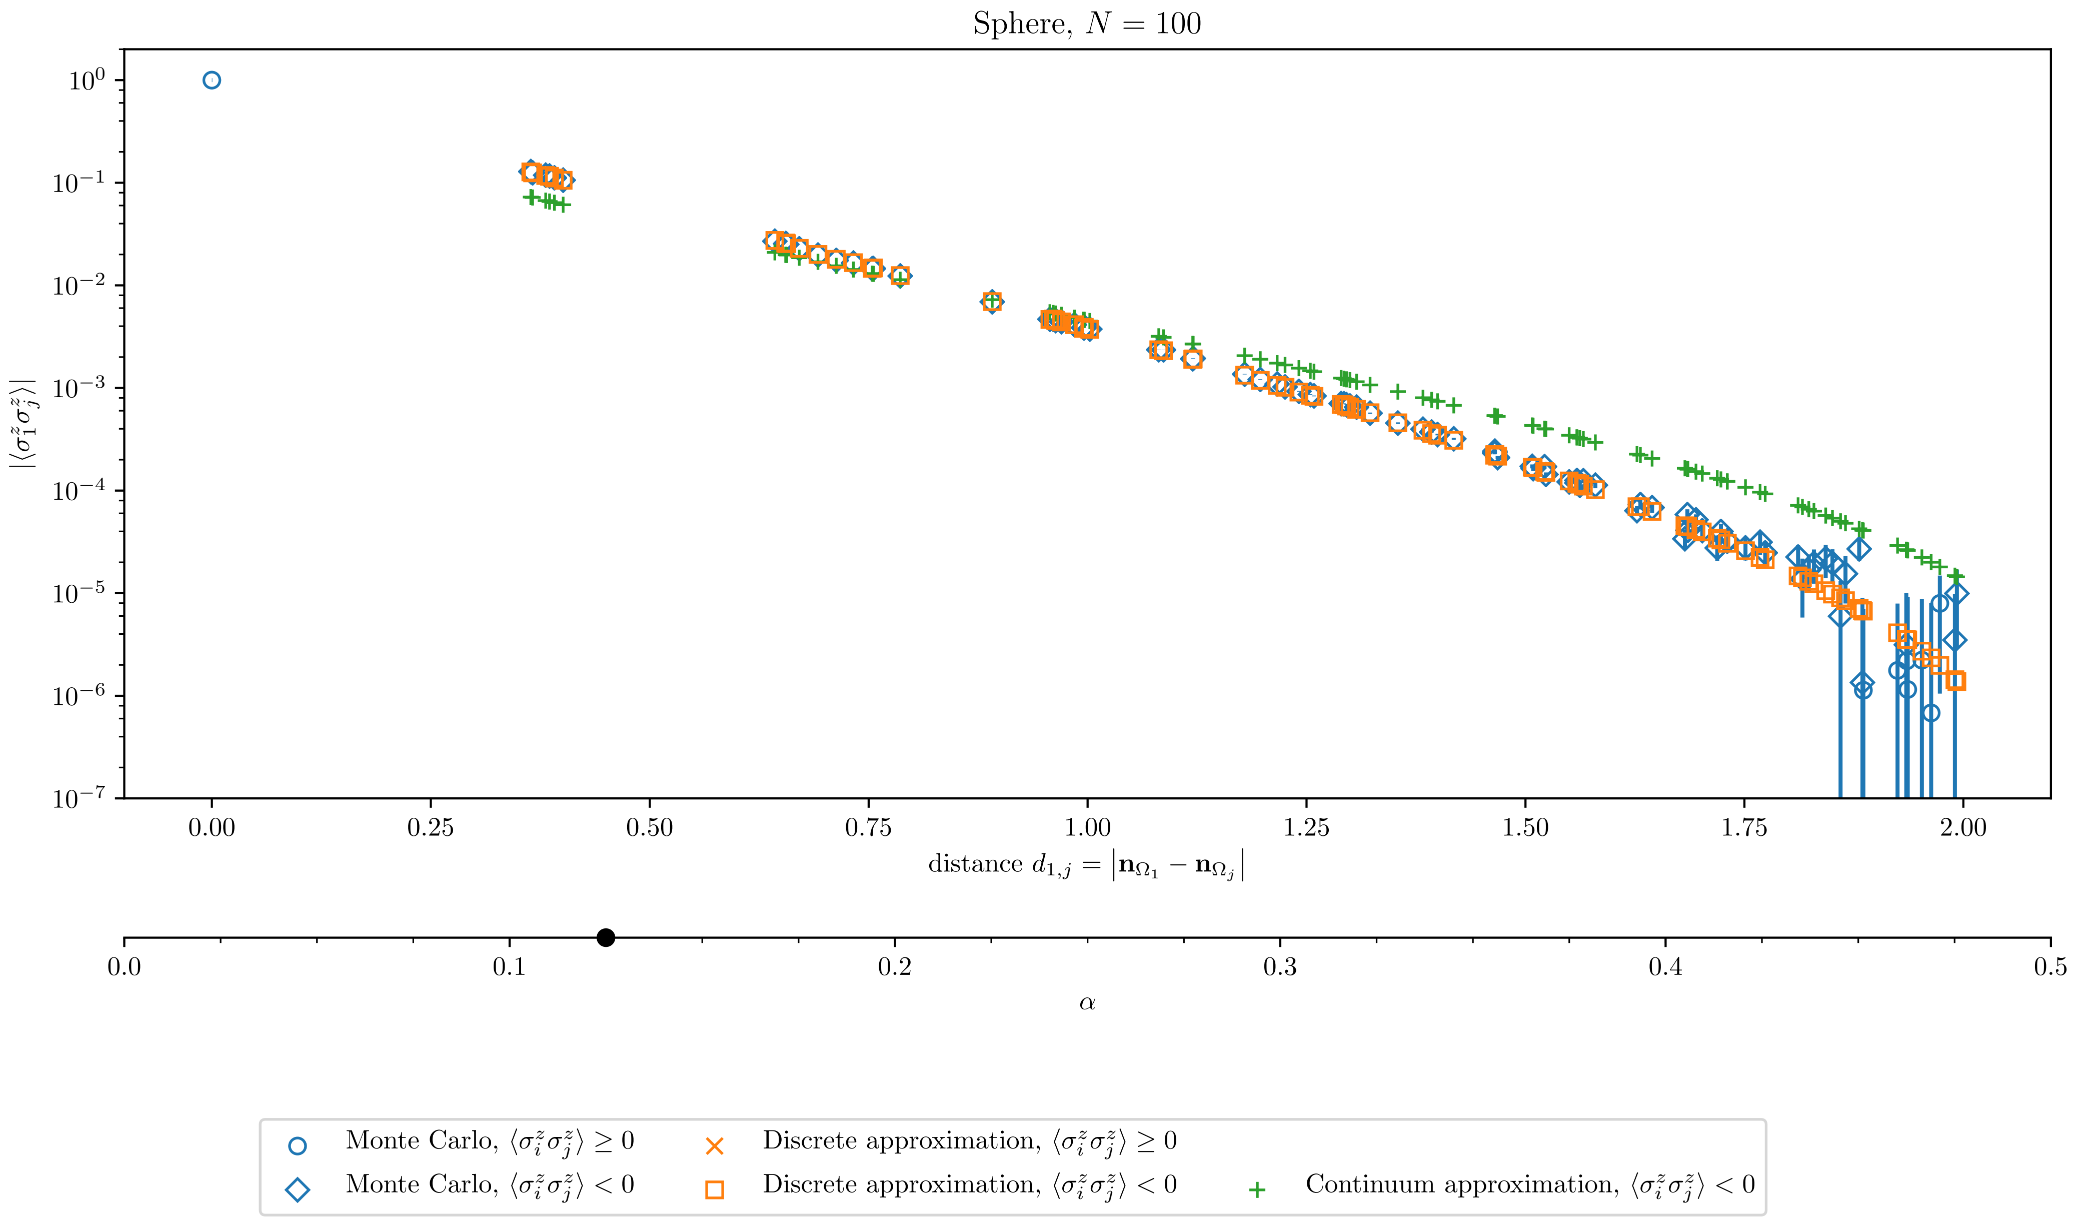

Sphere, $N = 100$
$10^{0}$
$10^{-1}$
$10^{-2}$
$10^{-3}$
$10^{-4}$
$10^{-5}$
$10^{-6}$
$10^{-7}$
$|\langle\sigma_1^z\sigma_j^z\rangle|$
0.00
0.25
0.50
0.75
1.00
1.25
1.50
1.75
2.00
distance $d_{1,j} = |\mathbf{n}_{\Omega_1} - \mathbf{n}_{\Omega_j}|$
0.0
0.1
0.2
0.3
0.4
0.5
$\alpha$
Monte Carlo, $\langle\sigma_i^z\sigma_j^z\rangle \geq 0$
Monte Carlo, $\langle\sigma_i^z\sigma_j^z\rangle < 0$
Discrete approximation, $\langle\sigma_i^z\sigma_j^z\rangle \geq 0$
Discrete approximation, $\langle\sigma_i^z\sigma_j^z\rangle < 0$
Continuum approximation, $\langle\sigma_i^z\sigma_j^z\rangle < 0$

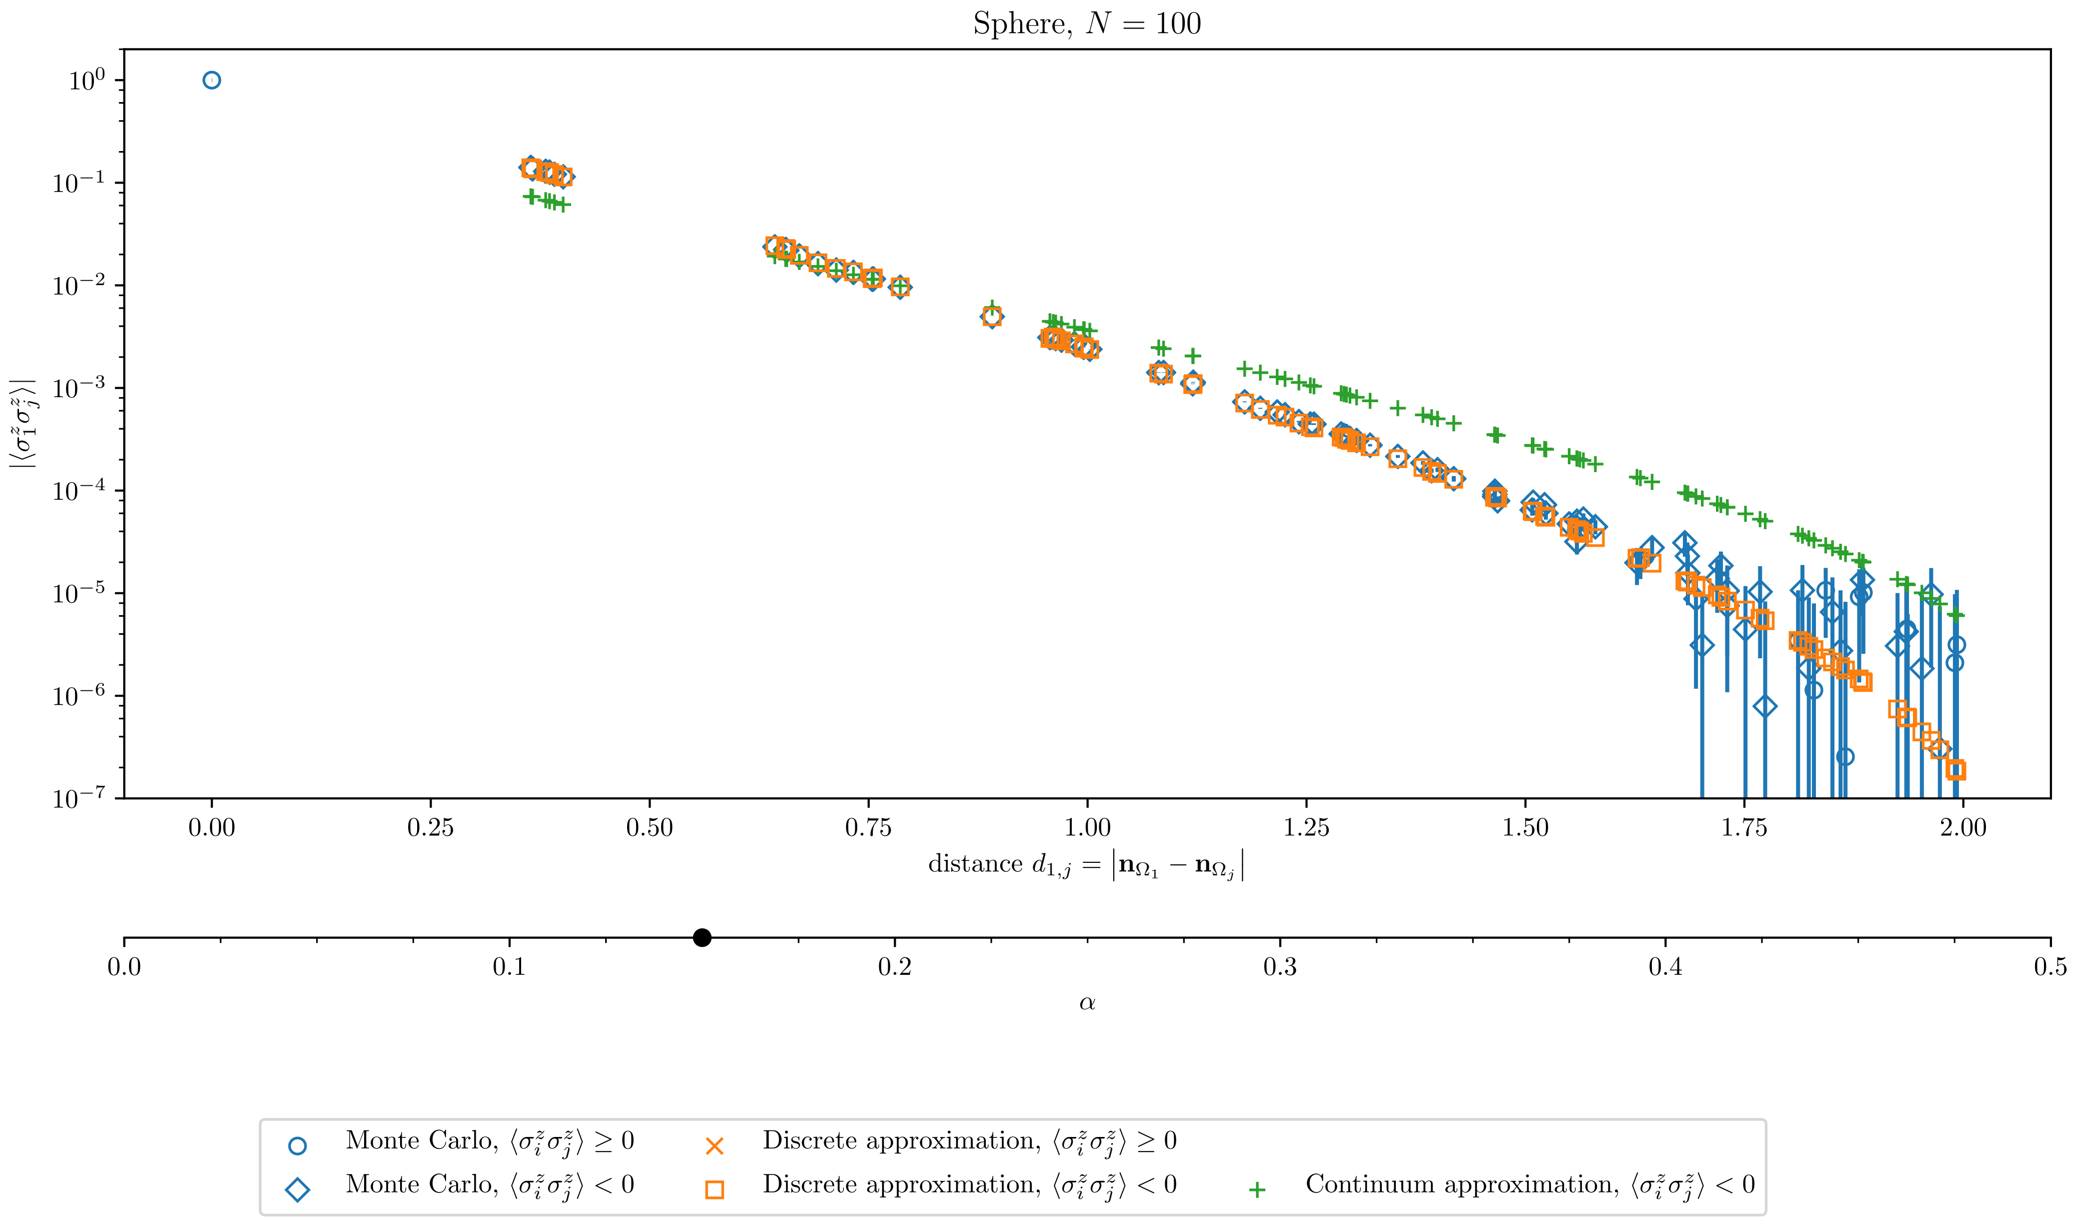

Sphere, $N = 100$
$10^{0}$
$10^{-1}$
$10^{-2}$
$10^{-3}$
$10^{-4}$
$10^{-5}$
$10^{-6}$
$10^{-7}$
$|\langle \sigma_1^z \sigma_j^z \rangle|$
0.00
0.25
0.50
0.75
1.00
1.25
1.50
1.75
2.00
distance $d_{1,j} = |\mathbf{n}_{\Omega_1} - \mathbf{n}_{\Omega_j}|$
0.0
0.1
0.2
0.3
0.4
0.5
$\alpha$
Monte Carlo, $\langle \sigma_i^z \sigma_j^z \rangle \geq 0$
Monte Carlo, $\langle \sigma_i^z \sigma_j^z \rangle < 0$
Discrete approximation, $\langle \sigma_i^z \sigma_j^z \rangle \geq 0$
Discrete approximation, $\langle \sigma_i^z \sigma_j^z \rangle < 0$
Continuum approximation, $\langle \sigma_i^z \sigma_j^z \rangle < 0$

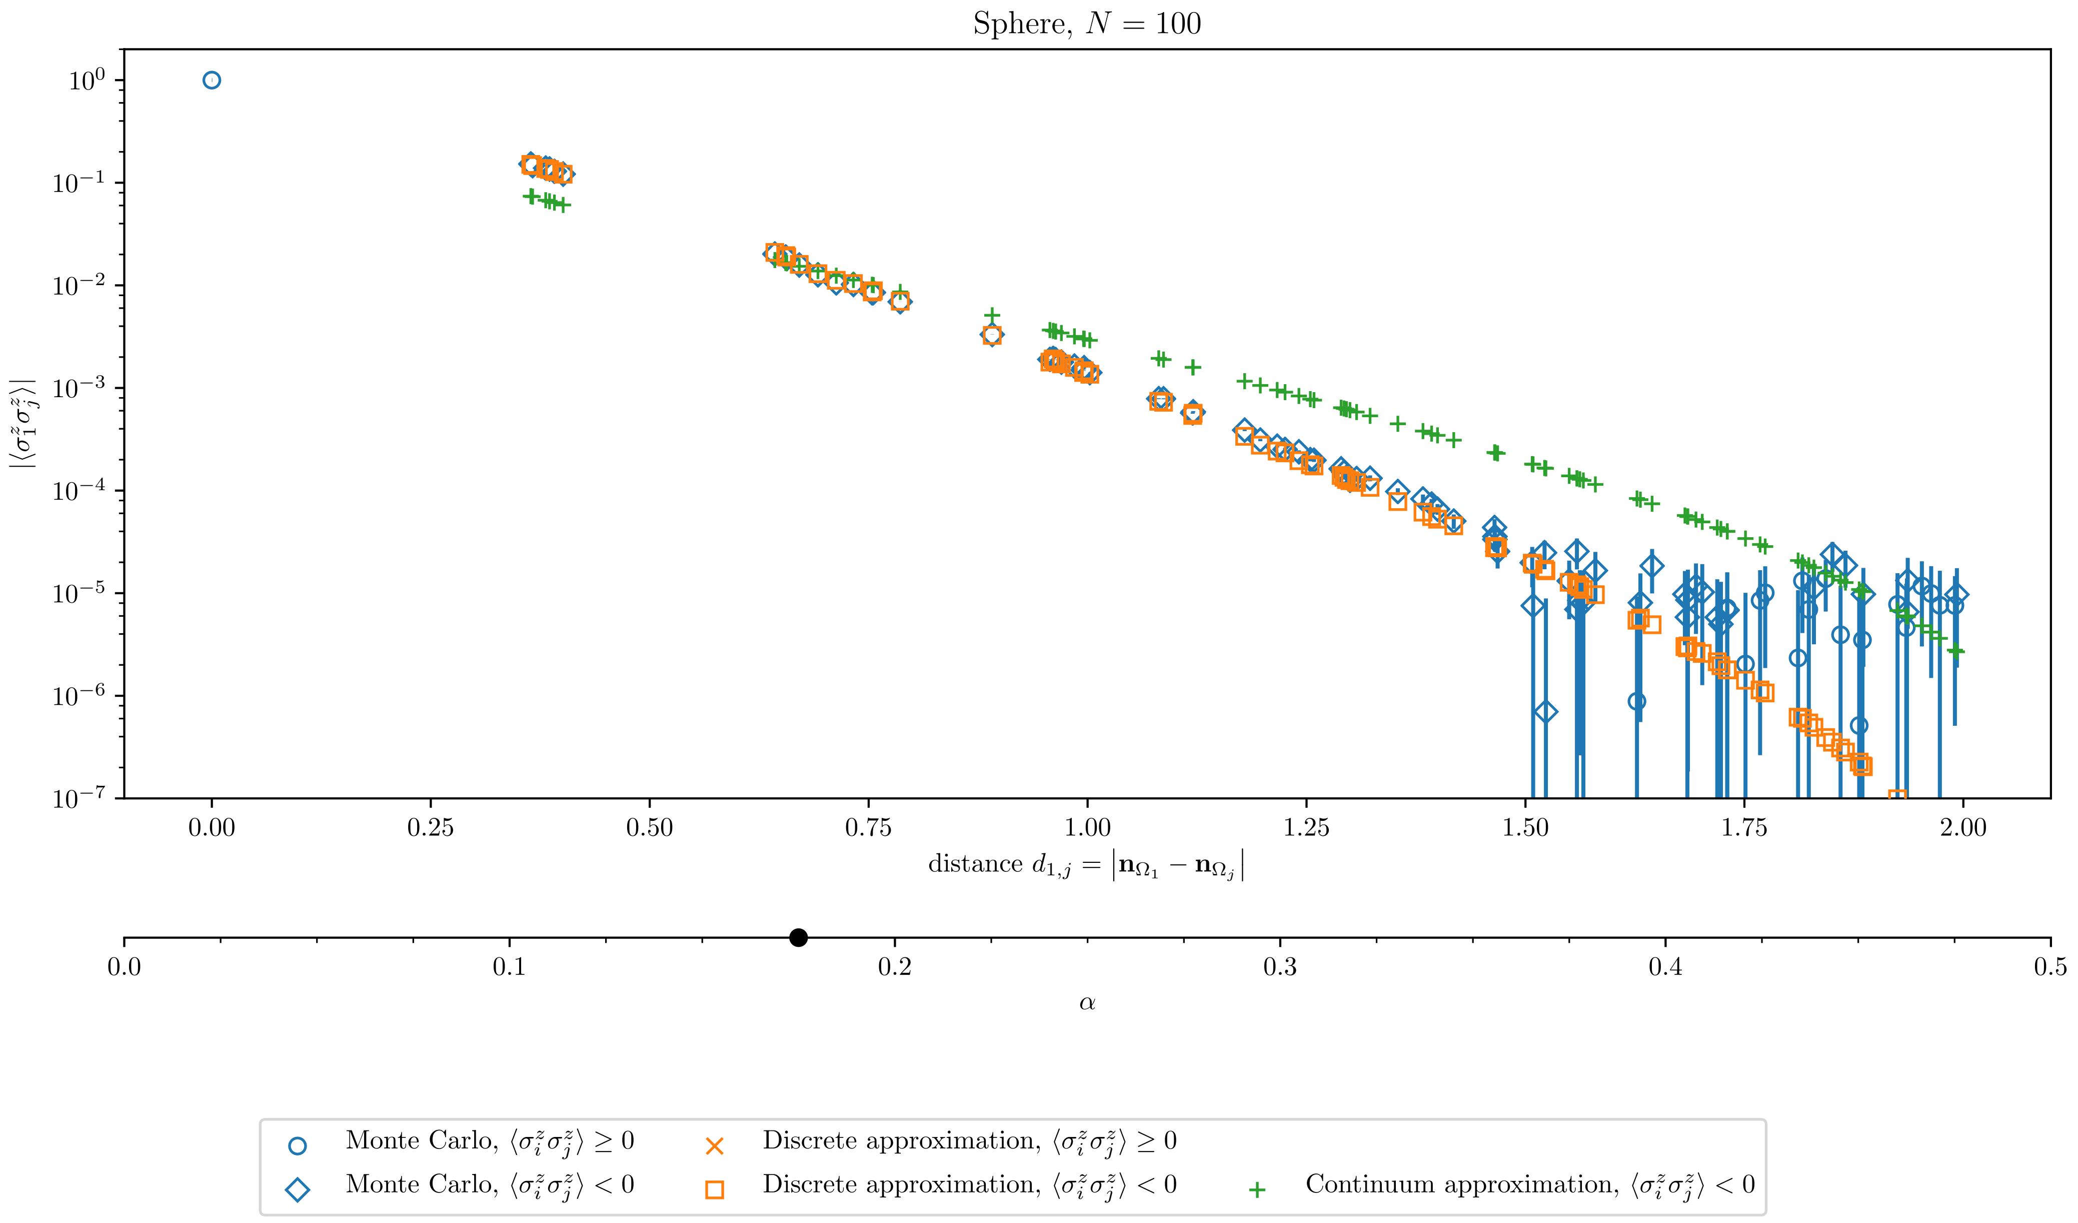

Sphere, $N = 100$
$10^{0}$
$10^{-1}$
$10^{-2}$
$10^{-3}$
$10^{-4}$
$10^{-5}$
$10^{-6}$
$10^{-7}$
$|\langle \sigma_1^z \sigma_j^z \rangle|$
0.00
0.25
0.50
0.75
1.00
1.25
1.50
1.75
2.00
distance $d_{1,j} = |\mathbf{n}_{\Omega_1} - \mathbf{n}_{\Omega_j}|$
0.0
0.1
0.2
0.3
0.4
0.5
$\alpha$
Monte Carlo, $\langle \sigma_i^z \sigma_j^z \rangle \geq 0$
Monte Carlo, $\langle \sigma_i^z \sigma_j^z \rangle < 0$
Discrete approximation, $\langle \sigma_i^z \sigma_j^z \rangle \geq 0$
Discrete approximation, $\langle \sigma_i^z \sigma_j^z \rangle < 0$
Continuum approximation, $\langle \sigma_i^z \sigma_j^z \rangle < 0$

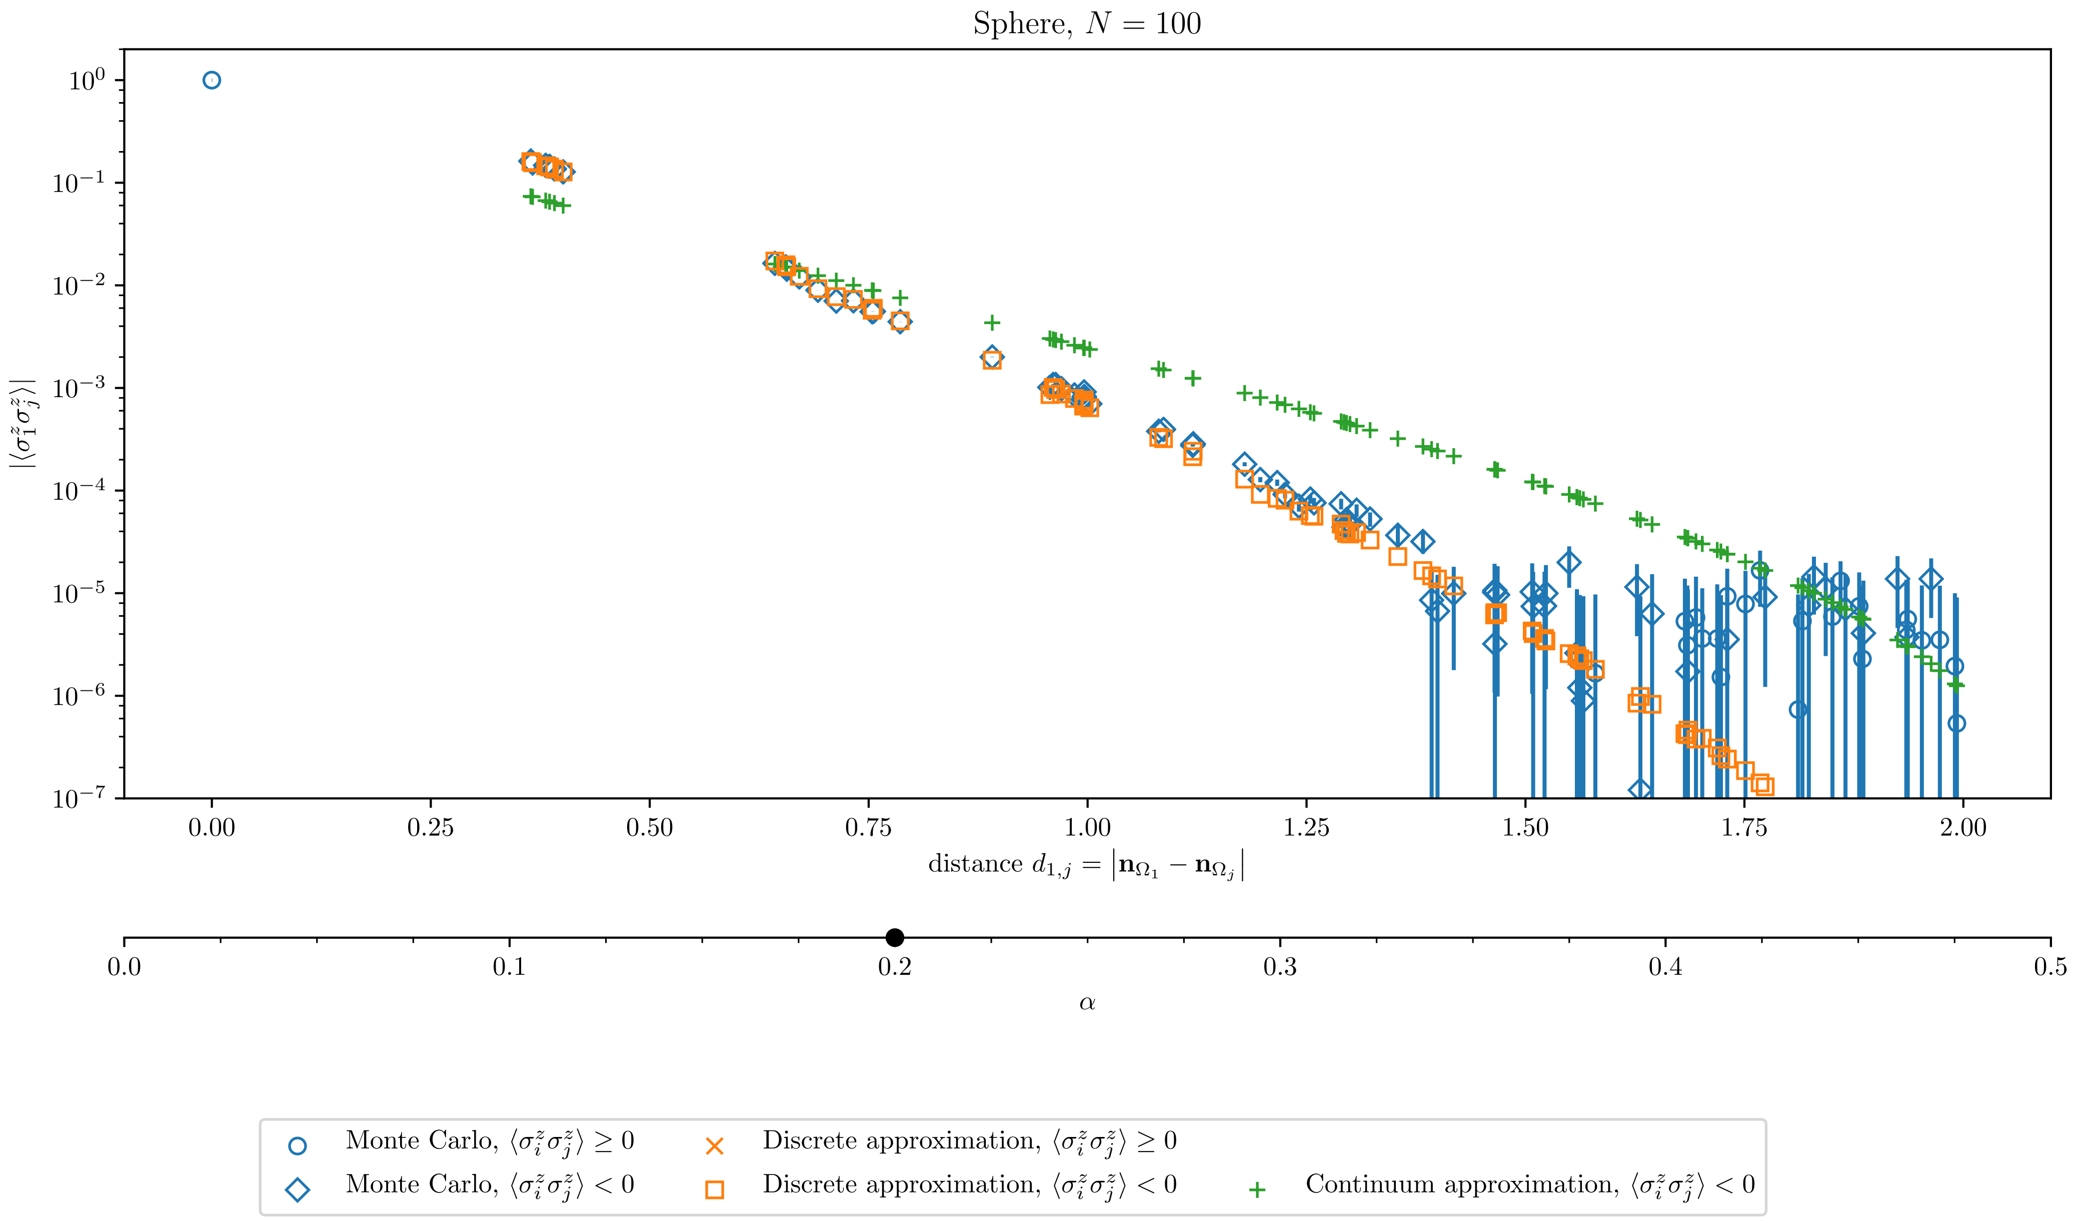

Sphere, $N = 100$
$|\langle\sigma_1^z\sigma_j^z\rangle|$
$10^0$
$10^{-1}$
$10^{-2}$
$10^{-3}$
$10^{-4}$
$10^{-5}$
$10^{-6}$
$10^{-7}$
0.00 0.25 0.50 0.75 1.00 1.25 1.50 1.75 2.00
distance $d_{1,j} = |\mathbf{n}_{\Omega_1} - \mathbf{n}_{\Omega_j}|$
0.0 0.1 0.2 0.3 0.4 0.5
$\alpha$
Monte Carlo, $\langle\sigma_i^z\sigma_j^z\rangle \geq 0$
Monte Carlo, $\langle\sigma_i^z\sigma_j^z\rangle < 0$
Discrete approximation, $\langle\sigma_i^z\sigma_j^z\rangle \geq 0$
Discrete approximation, $\langle\sigma_i^z\sigma_j^z\rangle < 0$
Continuum approximation, $\langle\sigma_i^z\sigma_j^z\rangle < 0$

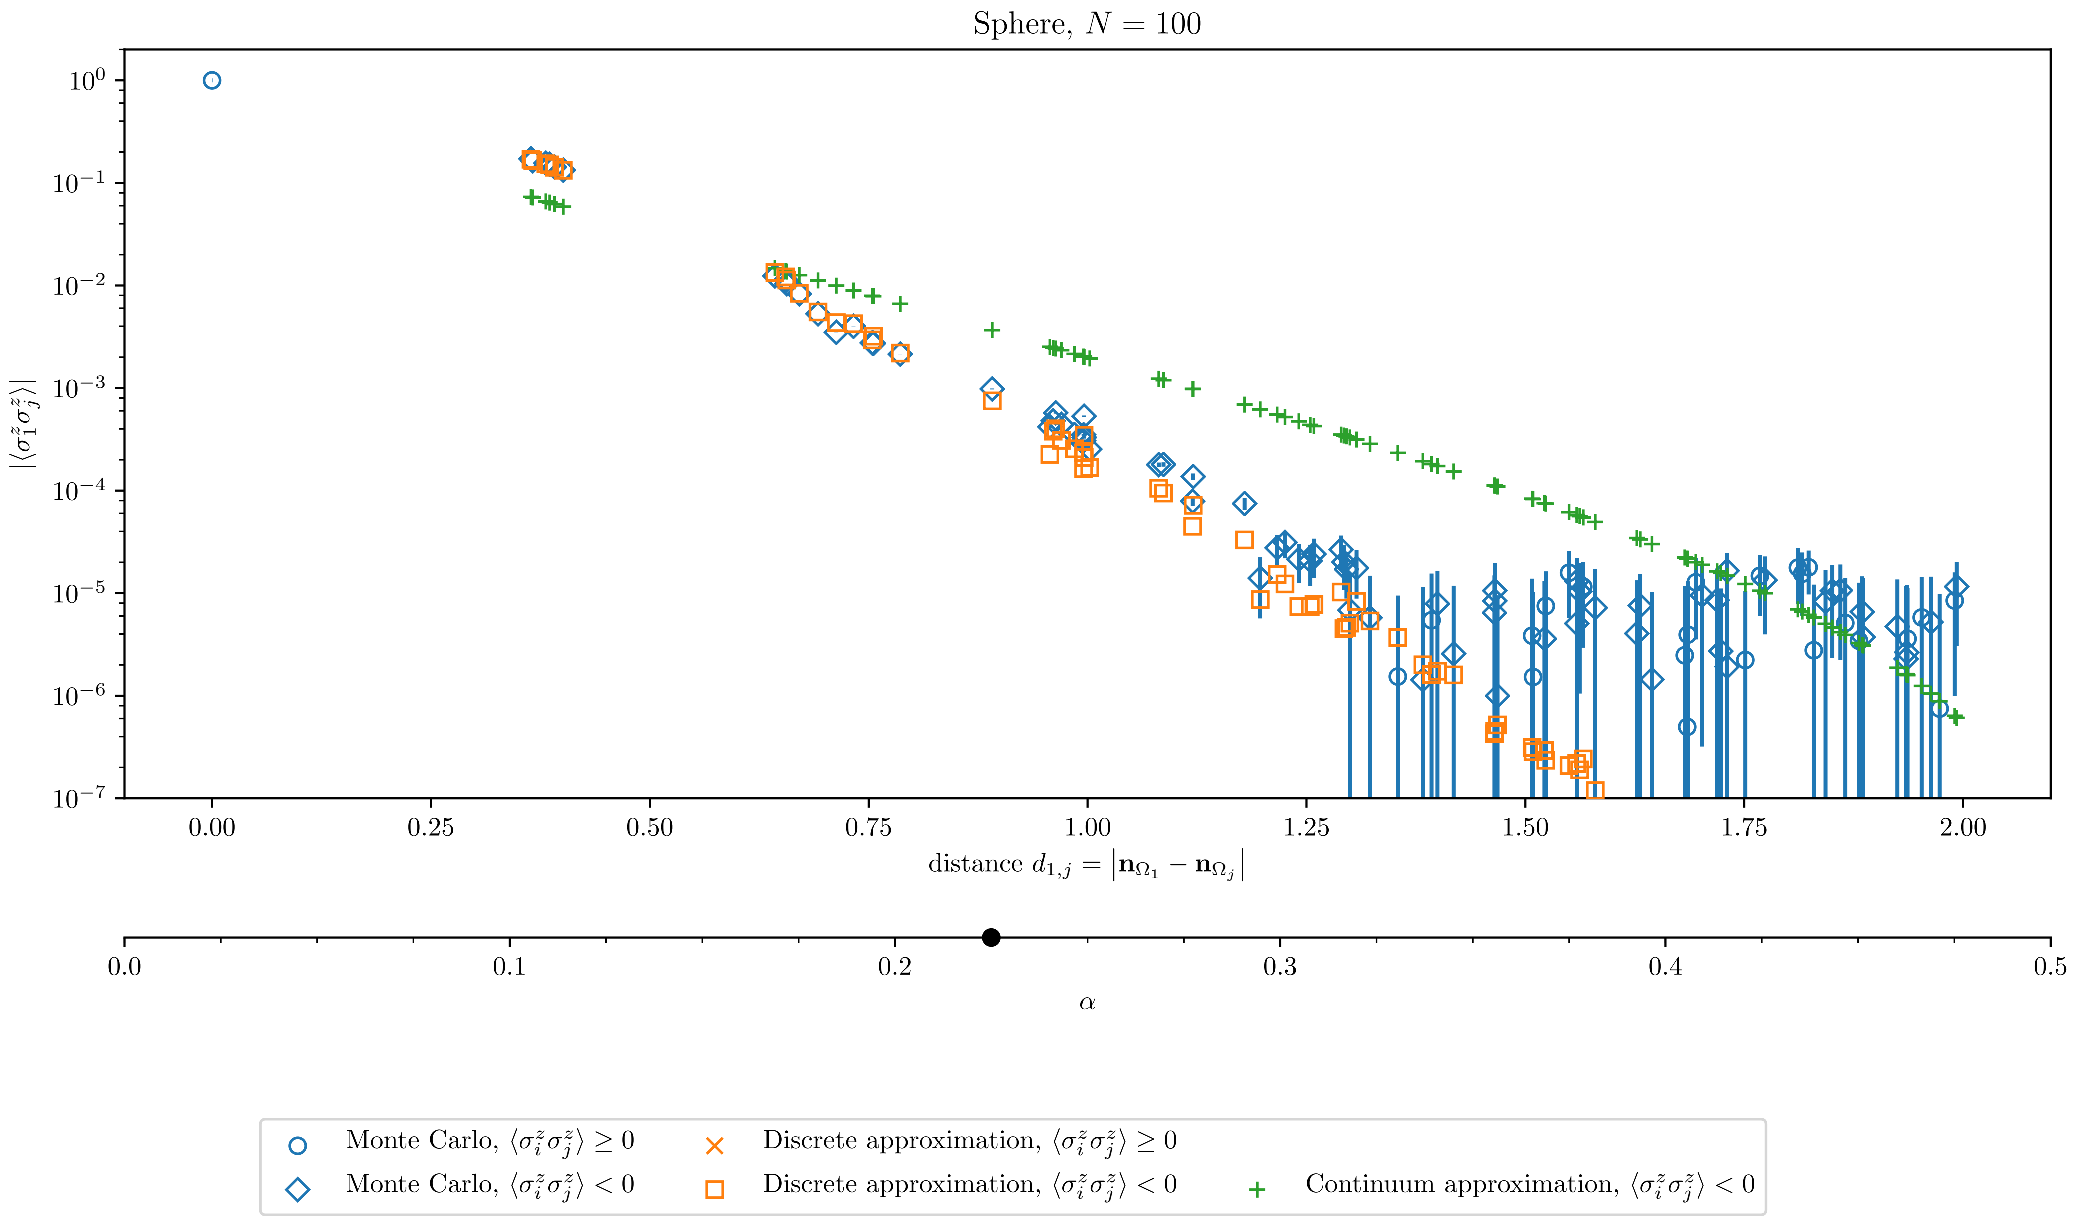

Sphere, $N = 100$
$|\langle\sigma_1^z\sigma_j^z\rangle|$
$10^0$
$10^{-1}$
$10^{-2}$
$10^{-3}$
$10^{-4}$
$10^{-5}$
$10^{-6}$
$10^{-7}$
0.00
0.25
0.50
0.75
1.00
1.25
1.50
1.75
2.00
distance $d_{1,j} = |\mathbf{n}_{\Omega_1} - \mathbf{n}_{\Omega_j}|$
0.0
0.1
0.2
0.3
0.4
0.5
$\alpha$
Monte Carlo, $\langle\sigma_i^z\sigma_j^z\rangle \geq 0$
Monte Carlo, $\langle\sigma_i^z\sigma_j^z\rangle < 0$
Discrete approximation, $\langle\sigma_i^z\sigma_j^z\rangle \geq 0$
Discrete approximation, $\langle\sigma_i^z\sigma_j^z\rangle < 0$
Continuum approximation, $\langle\sigma_i^z\sigma_j^z\rangle < 0$

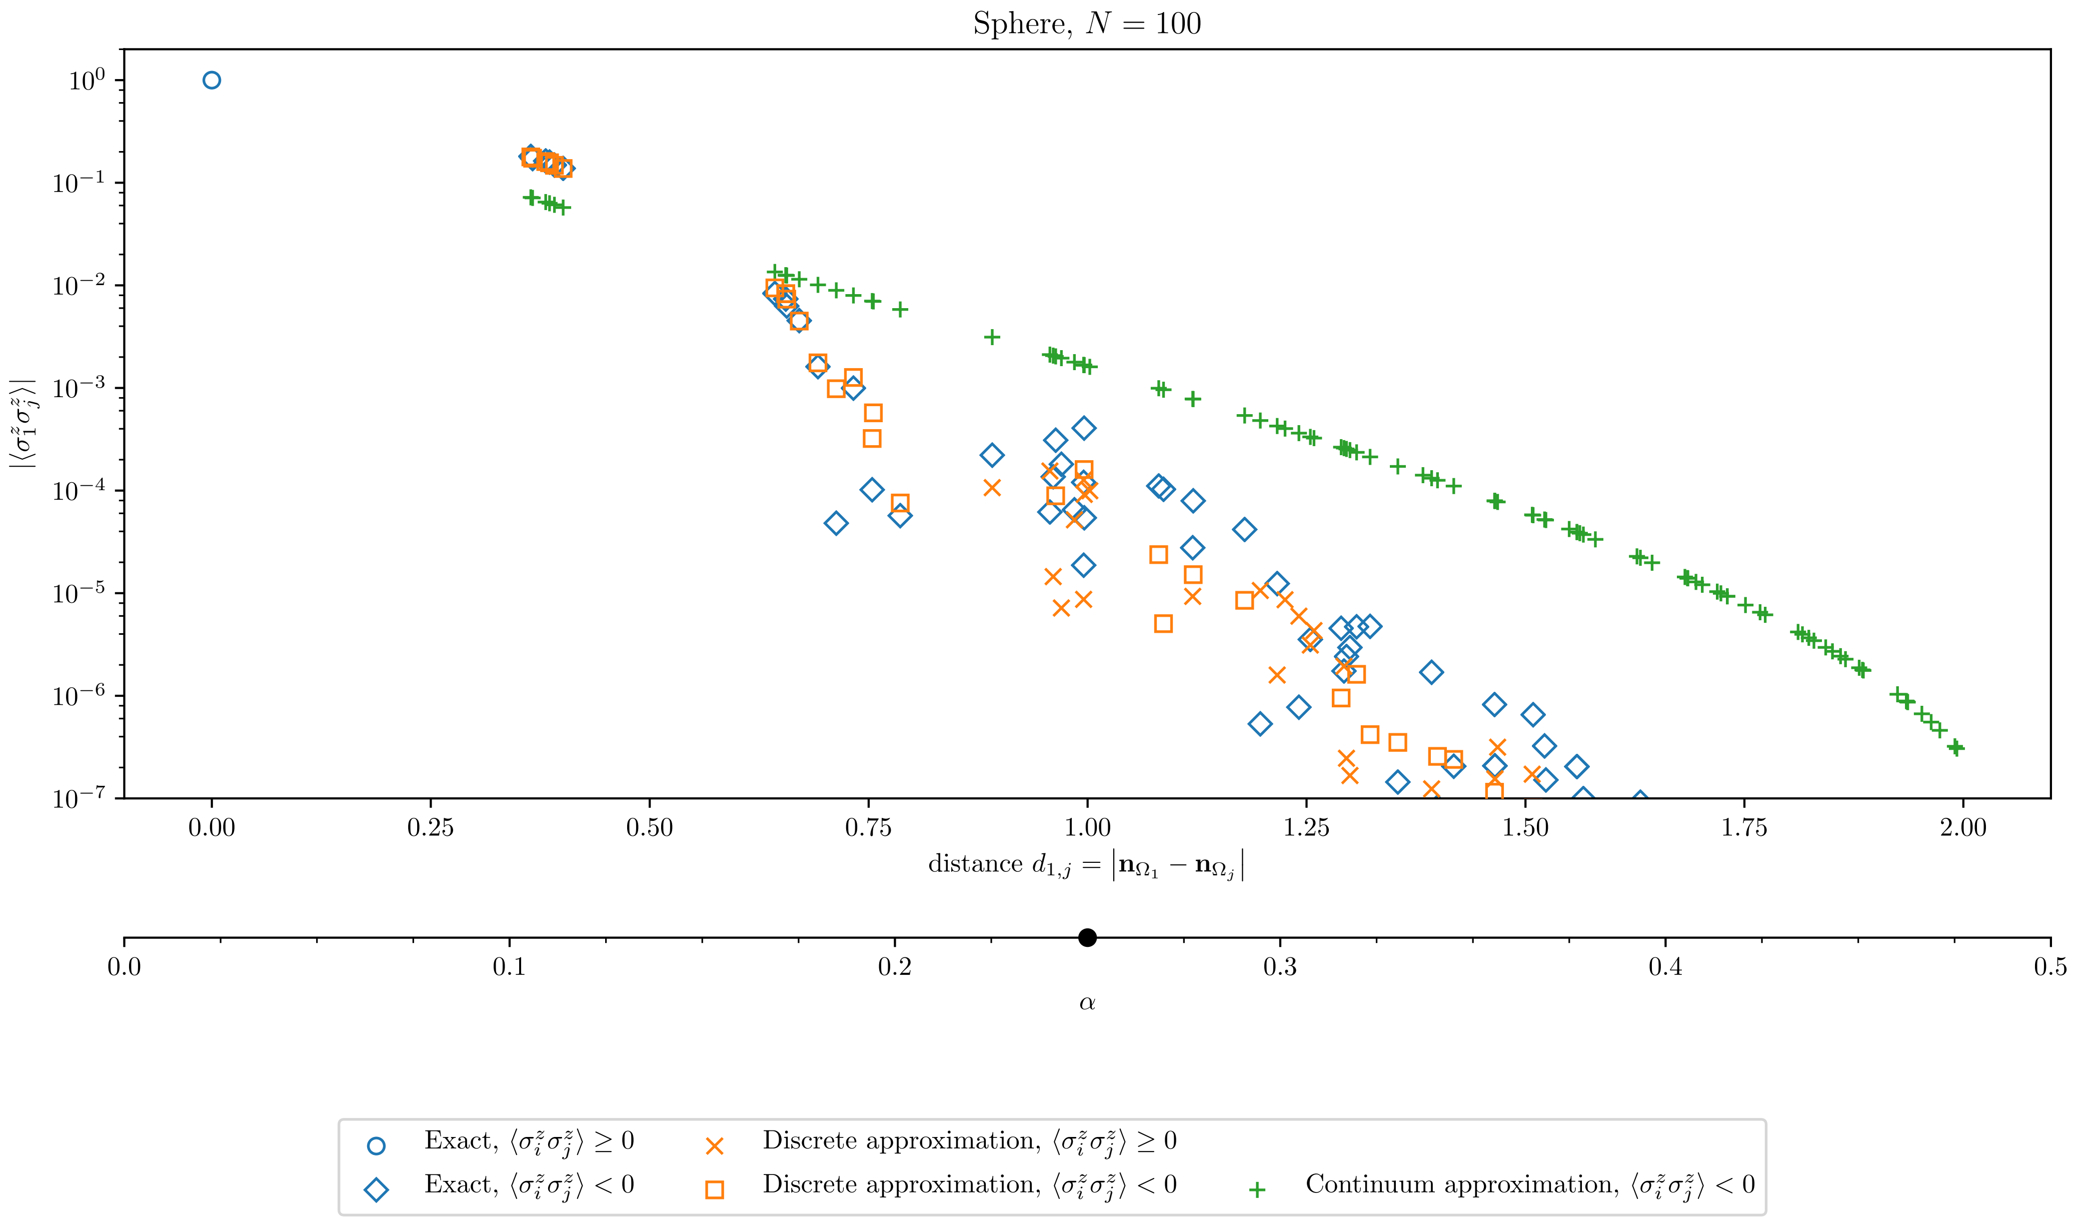

Sphere, $N = 100$
$|\langle\sigma_1^z\sigma_j^z\rangle|$
distance $d_{1,j} = |\mathbf{n}_{\Omega_1} - \mathbf{n}_{\Omega_j}|$
$\alpha$
Exact, $\langle\sigma_i^z\sigma_j^z\rangle \geq 0$
Exact, $\langle\sigma_i^z\sigma_j^z\rangle < 0$
Discrete approximation, $\langle\sigma_i^z\sigma_j^z\rangle \geq 0$
Discrete approximation, $\langle\sigma_i^z\sigma_j^z\rangle < 0$
Continuum approximation, $\langle\sigma_i^z\sigma_j^z\rangle < 0$

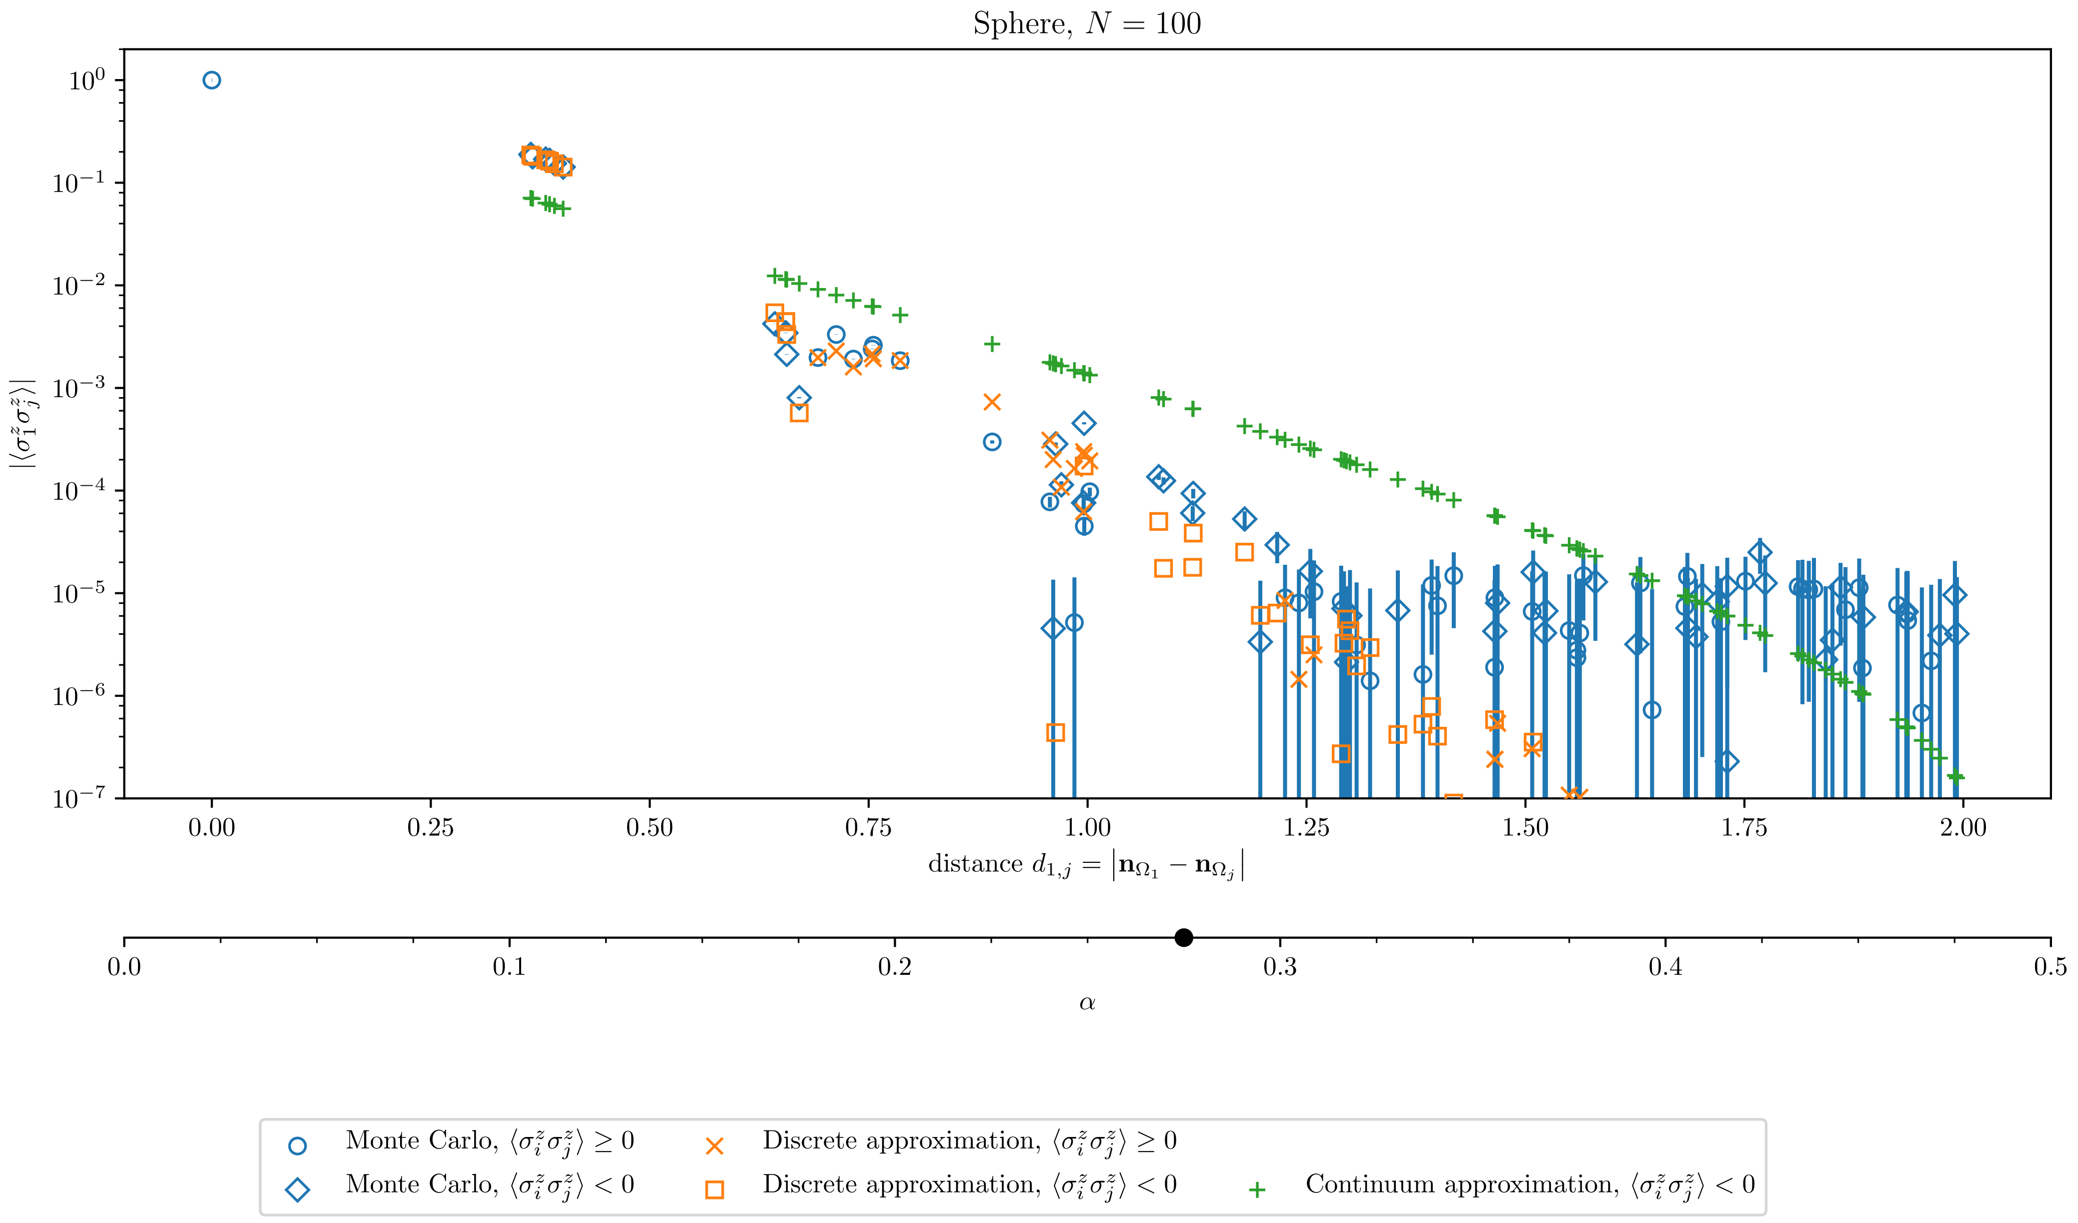

Sphere, $N = 100$
$|\langle\sigma_1^z\sigma_j^z\rangle|$
$10^0$
$10^{-1}$
$10^{-2}$
$10^{-3}$
$10^{-4}$
$10^{-5}$
$10^{-6}$
$10^{-7}$
0.00
0.25
0.50
0.75
1.00
1.25
1.50
1.75
2.00
distance $d_{1,j} = |\mathbf{n}_{\Omega_1} - \mathbf{n}_{\Omega_j}|$
0.0
0.1
0.2
0.3
0.4
0.5
$\alpha$
Monte Carlo, $\langle\sigma_i^z\sigma_j^z\rangle \geq 0$
Monte Carlo, $\langle\sigma_i^z\sigma_j^z\rangle < 0$
Discrete approximation, $\langle\sigma_i^z\sigma_j^z\rangle \geq 0$
Discrete approximation, $\langle\sigma_i^z\sigma_j^z\rangle < 0$
Continuum approximation, $\langle\sigma_i^z\sigma_j^z\rangle < 0$

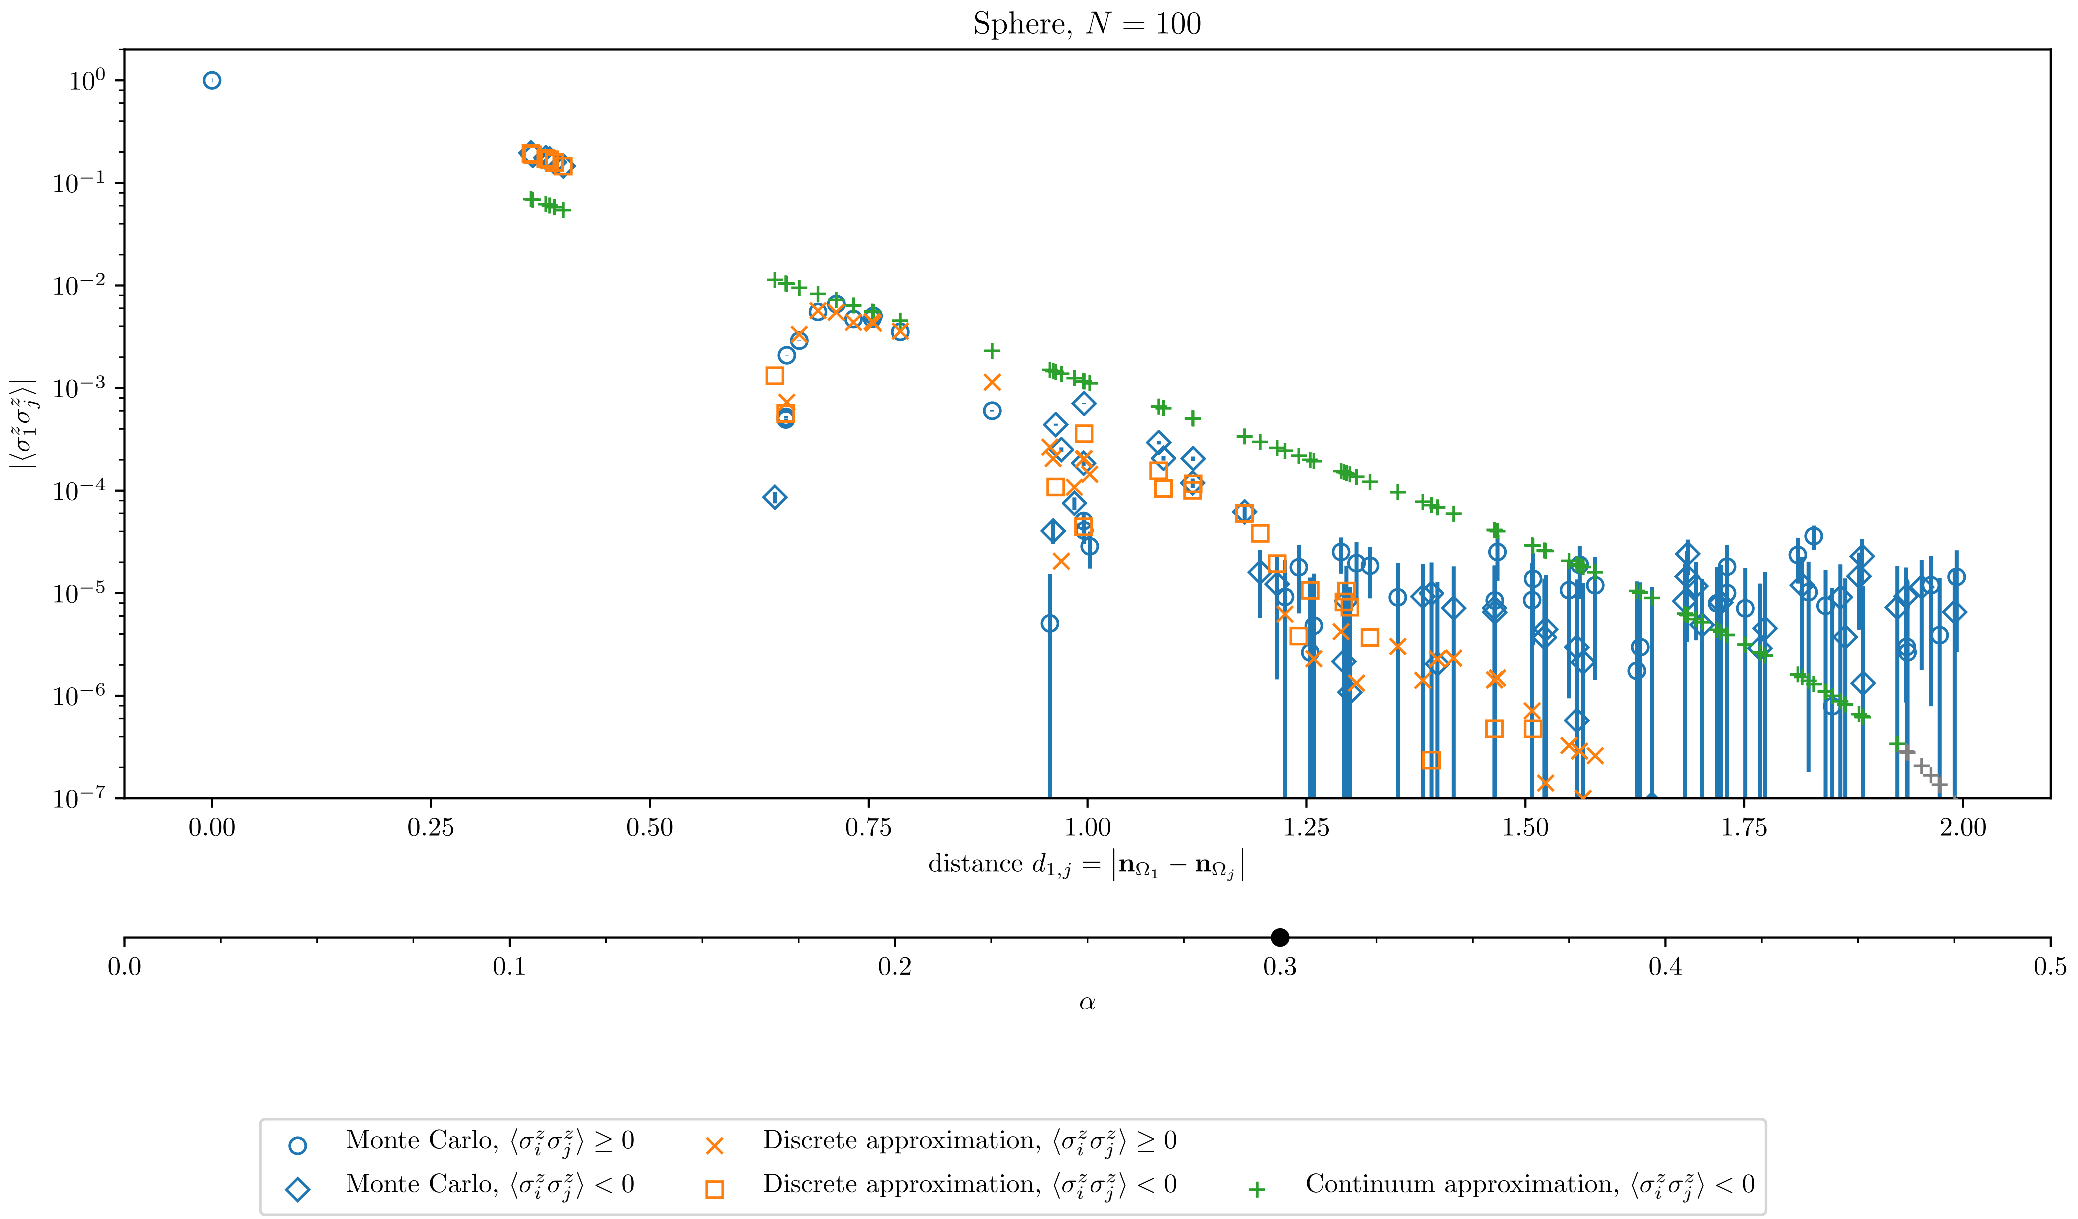

Sphere, $N = 100$
$|\langle \sigma_1^z \sigma_j^z \rangle|$
$10^0$
$10^{-1}$
$10^{-2}$
$10^{-3}$
$10^{-4}$
$10^{-5}$
$10^{-6}$
$10^{-7}$
0.00
0.25
0.50
0.75
1.00
1.25
1.50
1.75
2.00
distance $d_{1,j} = |\mathbf{n}_{\Omega_1} - \mathbf{n}_{\Omega_j}|$
0.0
0.1
0.2
0.3
0.4
0.5
$\alpha$
Monte Carlo, $\langle \sigma_i^z \sigma_j^z \rangle \geq 0$
Monte Carlo, $\langle \sigma_i^z \sigma_j^z \rangle < 0$
Discrete approximation, $\langle \sigma_i^z \sigma_j^z \rangle \geq 0$
Discrete approximation, $\langle \sigma_i^z \sigma_j^z \rangle < 0$
Continuum approximation, $\langle \sigma_i^z \sigma_j^z \rangle < 0$

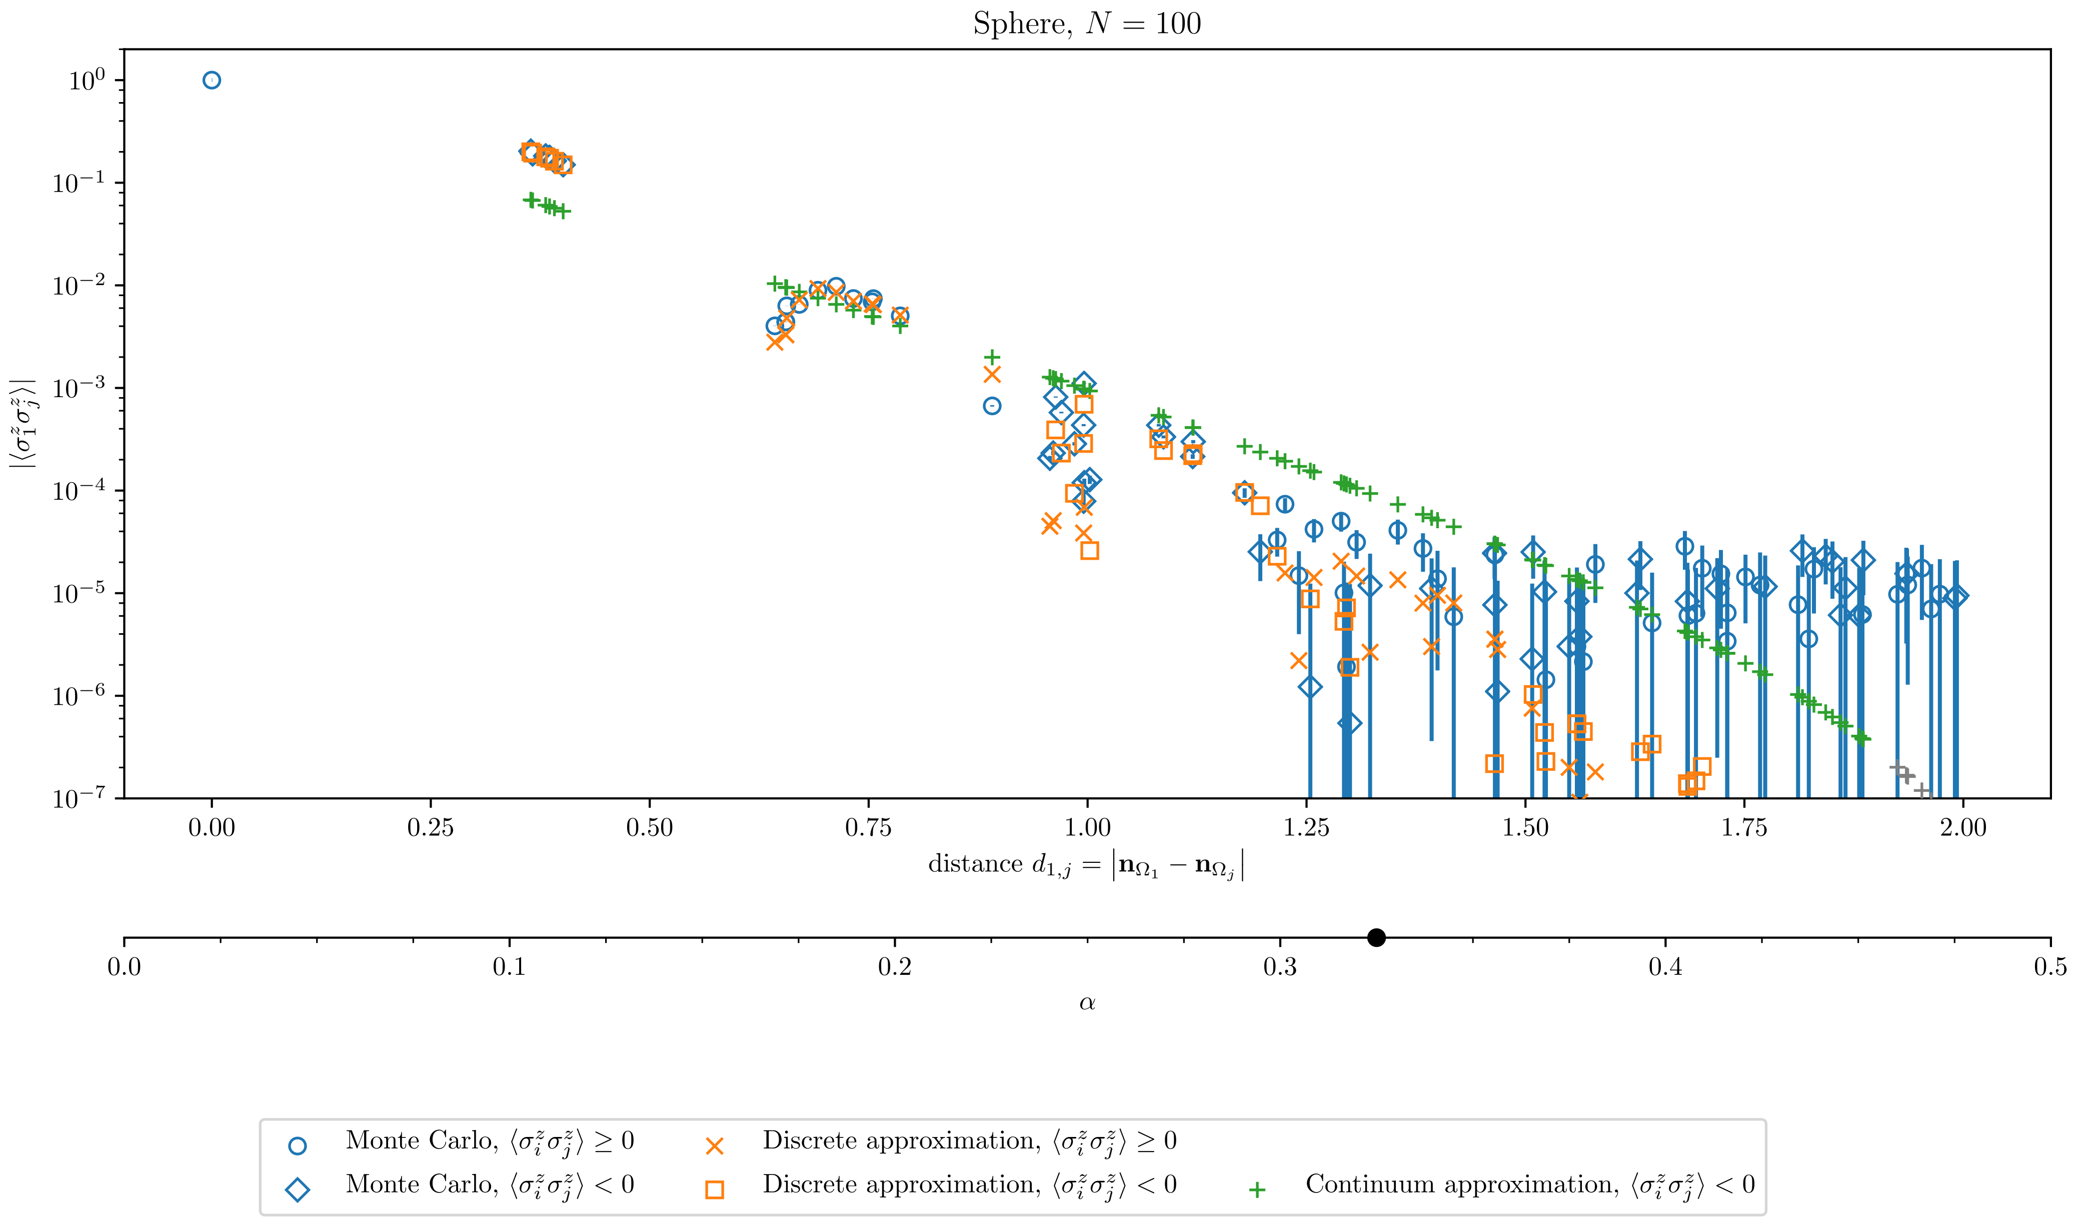

Sphere, $N = 100$
$10^0$
$10^{-1}$
$10^{-2}$
$10^{-3}$
$10^{-4}$
$10^{-5}$
$10^{-6}$
$10^{-7}$
$|\langle \sigma_1^z \sigma_j^z \rangle|$
0.00
0.25
0.50
0.75
1.00
1.25
1.50
1.75
2.00
distance $d_{1,j} = |\mathbf{n}_{\Omega_1} - \mathbf{n}_{\Omega_j}|$
0.0
0.1
0.2
0.3
0.4
0.5
$\alpha$
Monte Carlo, $\langle \sigma_i^z \sigma_j^z \rangle \geq 0$
Monte Carlo, $\langle \sigma_i^z \sigma_j^z \rangle < 0$
Discrete approximation, $\langle \sigma_i^z \sigma_j^z \rangle \geq 0$
Discrete approximation, $\langle \sigma_i^z \sigma_j^z \rangle < 0$
Continuum approximation, $\langle \sigma_i^z \sigma_j^z \rangle < 0$

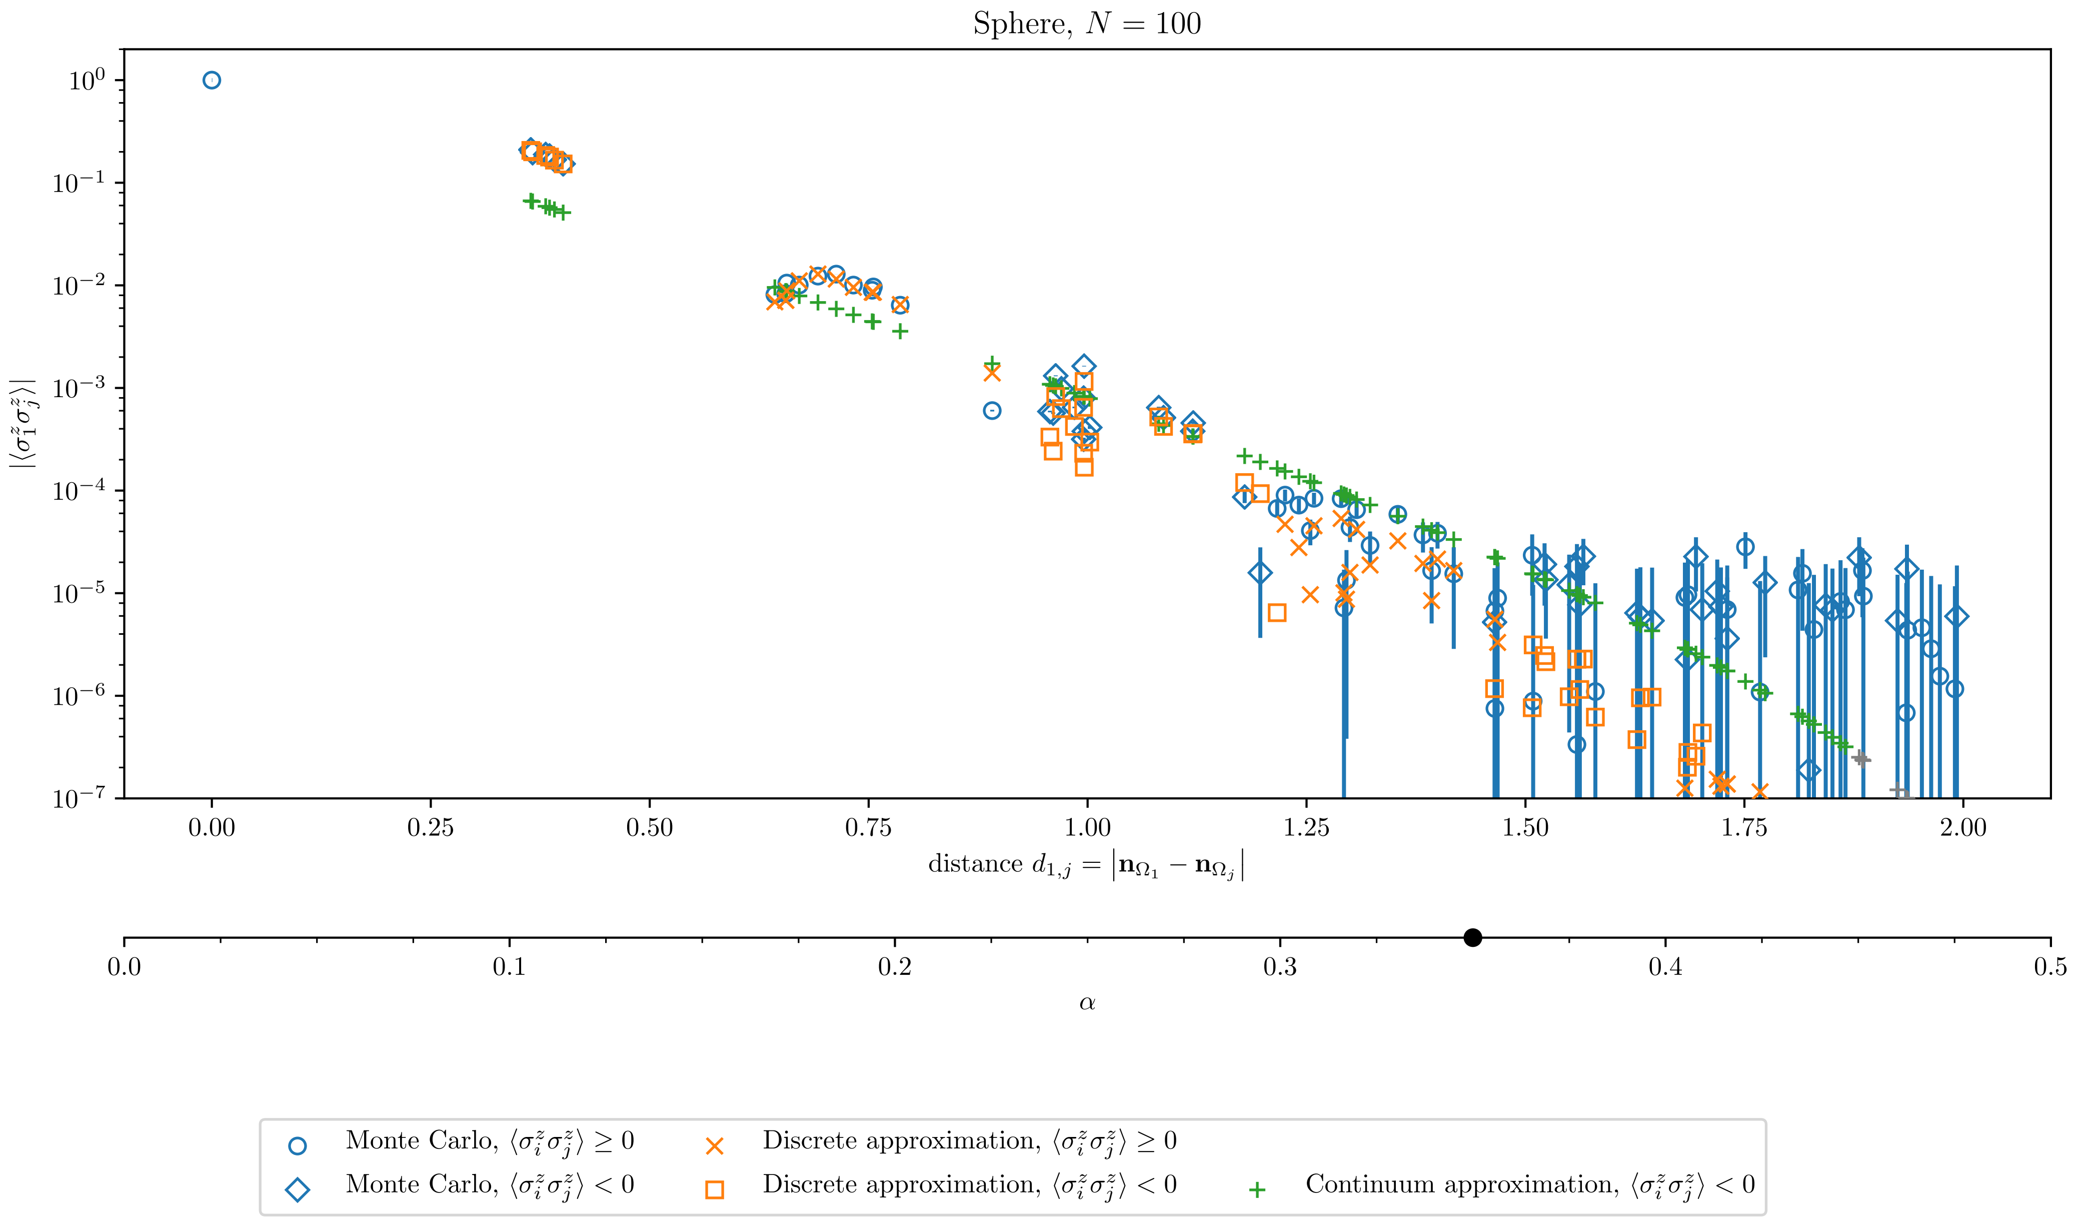

Sphere, $N = 100$
$|\langle\sigma_1^z\sigma_j^z\rangle|$
$10^0$
$10^{-1}$
$10^{-2}$
$10^{-3}$
$10^{-4}$
$10^{-5}$
$10^{-6}$
$10^{-7}$
0.00
0.25
0.50
0.75
1.00
1.25
1.50
1.75
2.00
distance $d_{1,j} = |\mathbf{n}_{\Omega_1} - \mathbf{n}_{\Omega_j}|$
0.0
0.1
0.2
0.3
0.4
0.5
$\alpha$
Monte Carlo, $\langle\sigma_i^z\sigma_j^z\rangle \geq 0$
Monte Carlo, $\langle\sigma_i^z\sigma_j^z\rangle < 0$
Discrete approximation, $\langle\sigma_i^z\sigma_j^z\rangle \geq 0$
Discrete approximation, $\langle\sigma_i^z\sigma_j^z\rangle < 0$
Continuum approximation, $\langle\sigma_i^z\sigma_j^z\rangle < 0$

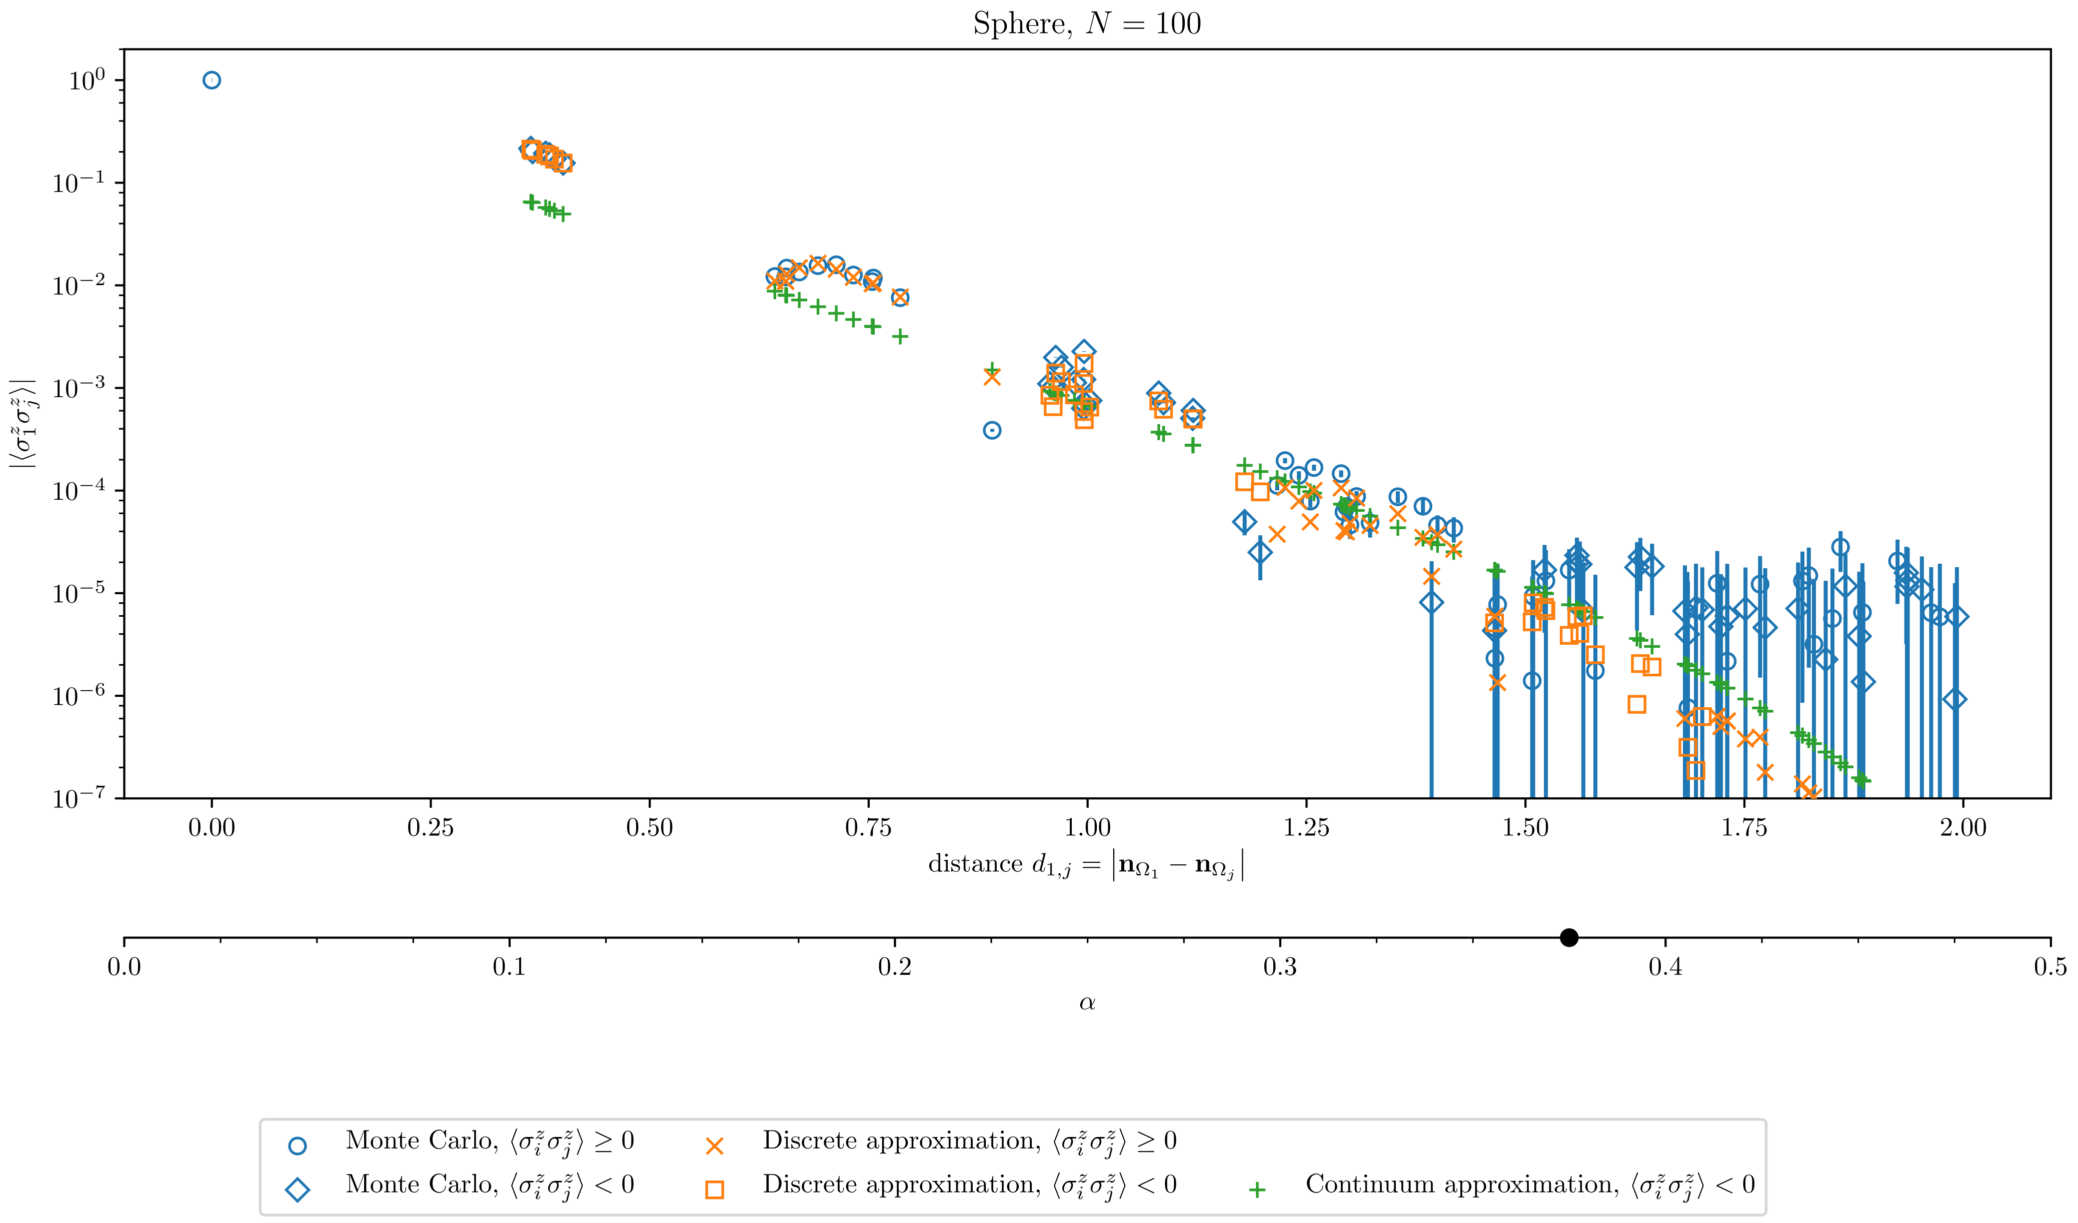

Sphere, $N = 100$
$|\langle\sigma_1^z\sigma_j^z\rangle|$
$10^0$
$10^{-1}$
$10^{-2}$
$10^{-3}$
$10^{-4}$
$10^{-5}$
$10^{-6}$
$10^{-7}$
0.00
0.25
0.50
0.75
1.00
1.25
1.50
1.75
2.00
distance $d_{1,j} = |\mathbf{n}_{\Omega_1} - \mathbf{n}_{\Omega_j}|$
0.0
0.1
0.2
0.3
0.4
0.5
$\alpha$
Monte Carlo, $\langle\sigma_i^z\sigma_j^z\rangle \geq 0$
Monte Carlo, $\langle\sigma_i^z\sigma_j^z\rangle < 0$
Discrete approximation, $\langle\sigma_i^z\sigma_j^z\rangle \geq 0$
Discrete approximation, $\langle\sigma_i^z\sigma_j^z\rangle < 0$
Continuum approximation, $\langle\sigma_i^z\sigma_j^z\rangle < 0$

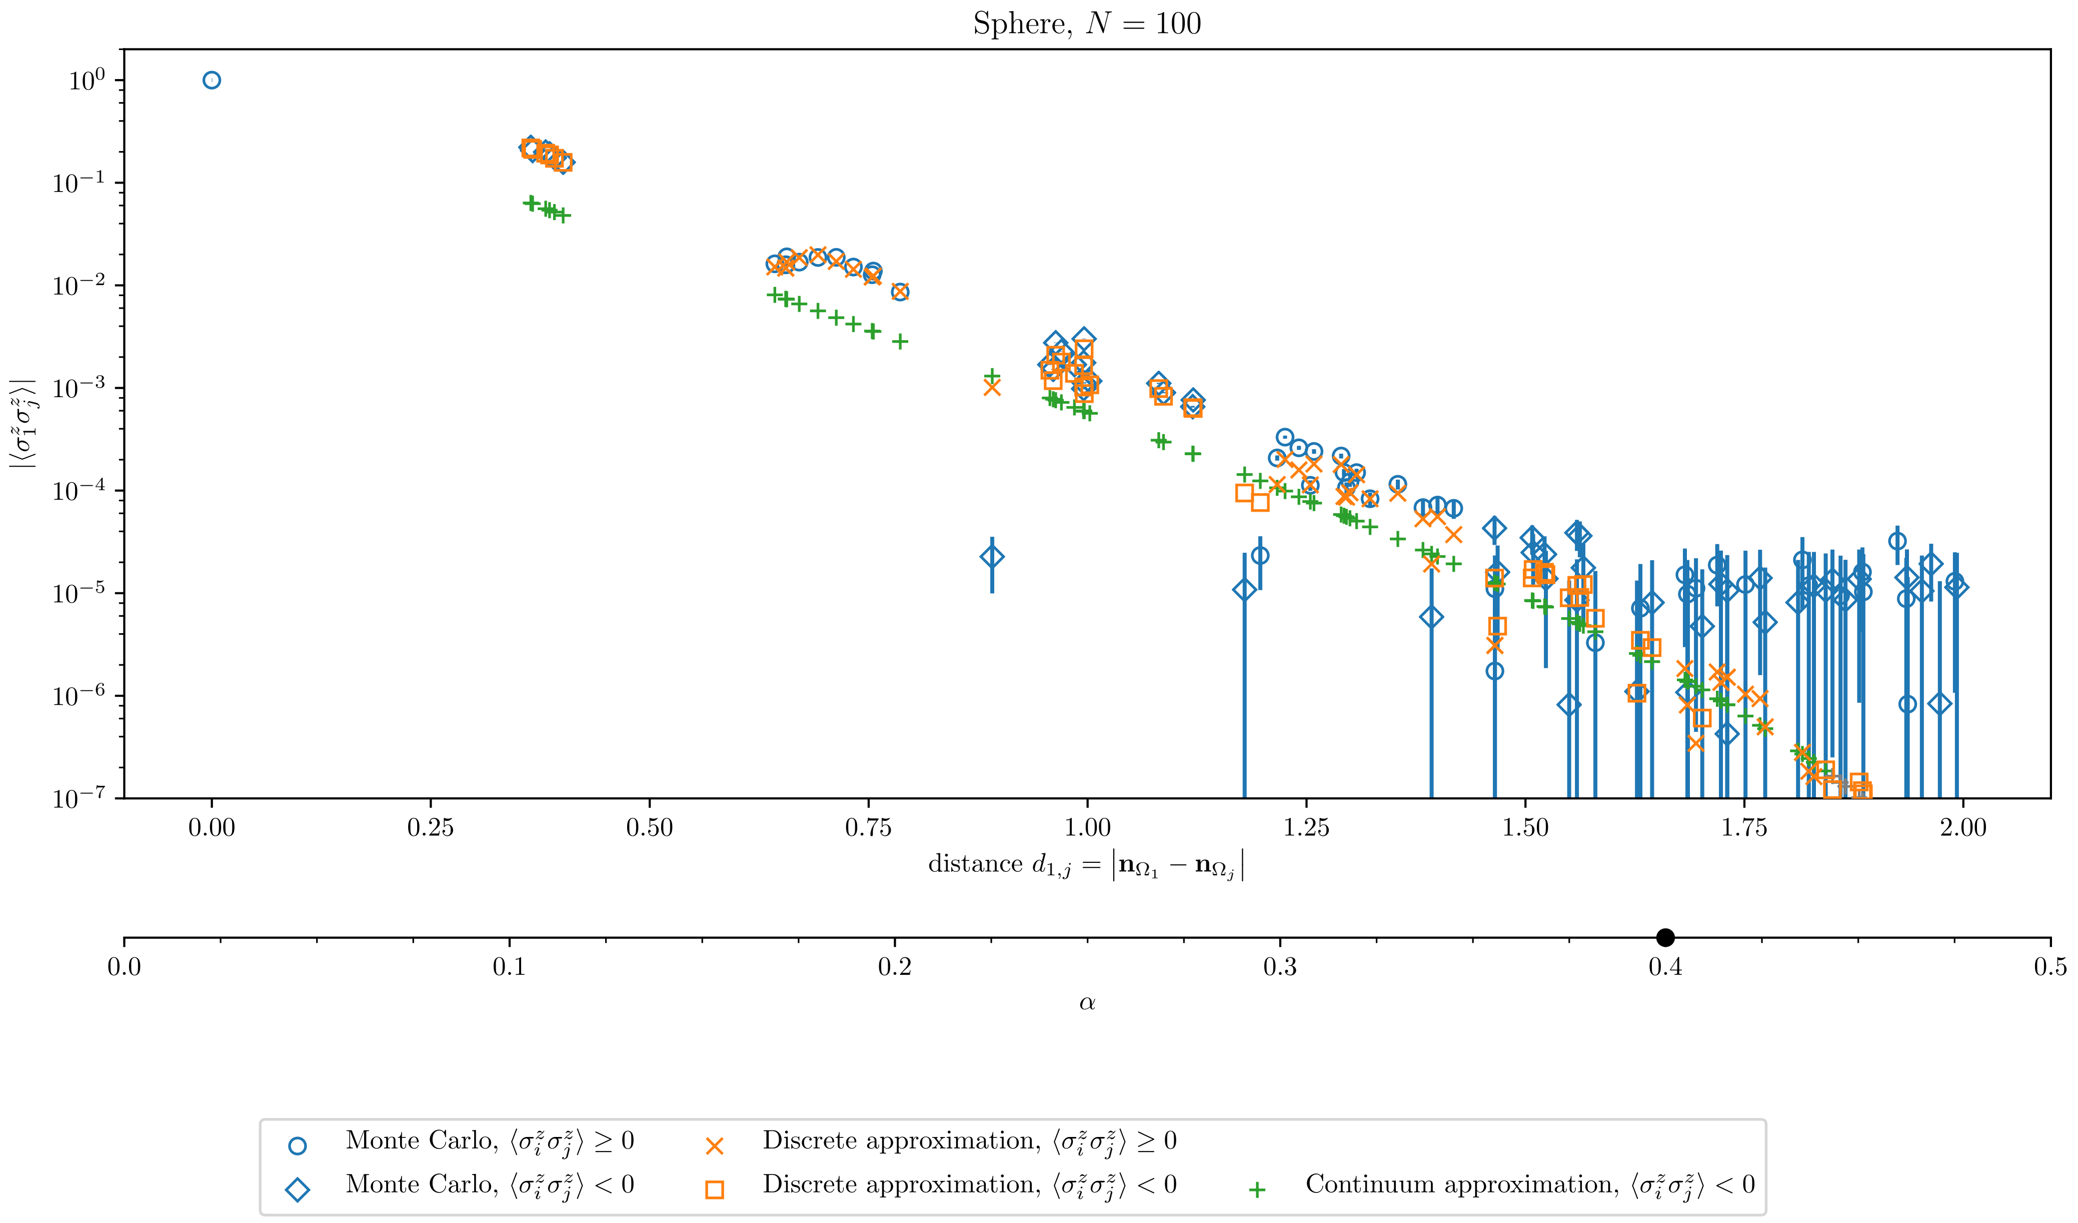

Sphere, $N = 100$
$|\langle\sigma_1^z\sigma_j^z\rangle|$
$10^0$
$10^{-1}$
$10^{-2}$
$10^{-3}$
$10^{-4}$
$10^{-5}$
$10^{-6}$
$10^{-7}$
0.00
0.25
0.50
0.75
1.00
1.25
1.50
1.75
2.00
distance $d_{1,j} = |\mathbf{n}_{\Omega_1} - \mathbf{n}_{\Omega_j}|$
0.0
0.1
0.2
0.3
0.4
0.5
$\alpha$
Monte Carlo, $\langle\sigma_i^z\sigma_j^z\rangle \geq 0$
Monte Carlo, $\langle\sigma_i^z\sigma_j^z\rangle < 0$
Discrete approximation, $\langle\sigma_i^z\sigma_j^z\rangle \geq 0$
Discrete approximation, $\langle\sigma_i^z\sigma_j^z\rangle < 0$
Continuum approximation, $\langle\sigma_i^z\sigma_j^z\rangle < 0$

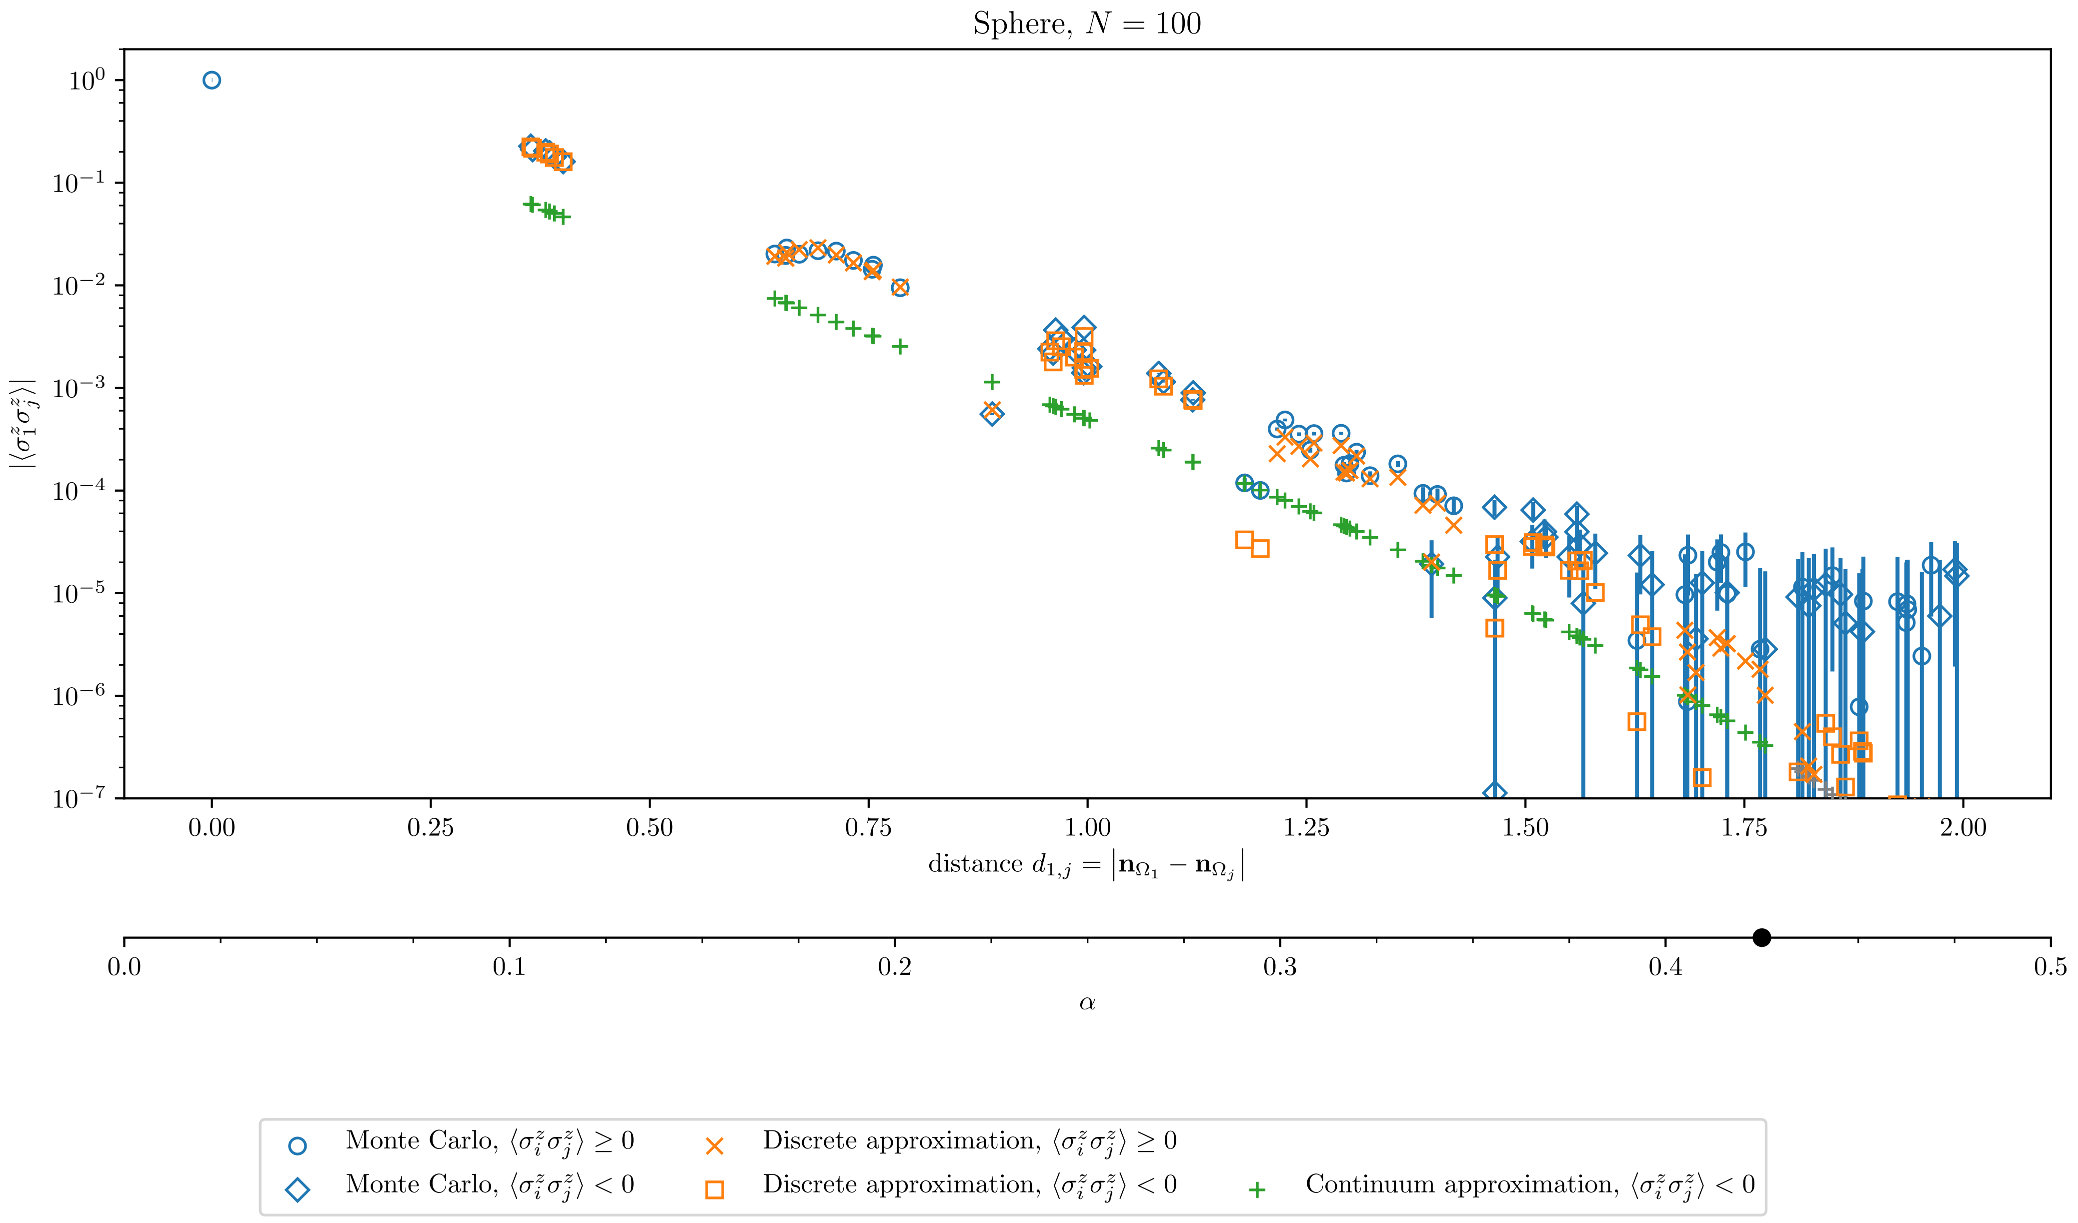

Sphere, $N = 100$
$|\langle\sigma_1^z\sigma_j^z\rangle|$
$10^0$
$10^{-1}$
$10^{-2}$
$10^{-3}$
$10^{-4}$
$10^{-5}$
$10^{-6}$
$10^{-7}$
0.00
0.25
0.50
0.75
1.00
1.25
1.50
1.75
2.00
distance $d_{1,j} = |\mathbf{n}_{\Omega_1} - \mathbf{n}_{\Omega_j}|$
0.0
0.1
0.2
0.3
0.4
0.5
$\alpha$
Monte Carlo, $\langle\sigma_i^z\sigma_j^z\rangle \geq 0$
Monte Carlo, $\langle\sigma_i^z\sigma_j^z\rangle < 0$
Discrete approximation, $\langle\sigma_i^z\sigma_j^z\rangle \geq 0$
Discrete approximation, $\langle\sigma_i^z\sigma_j^z\rangle < 0$
Continuum approximation, $\langle\sigma_i^z\sigma_j^z\rangle < 0$

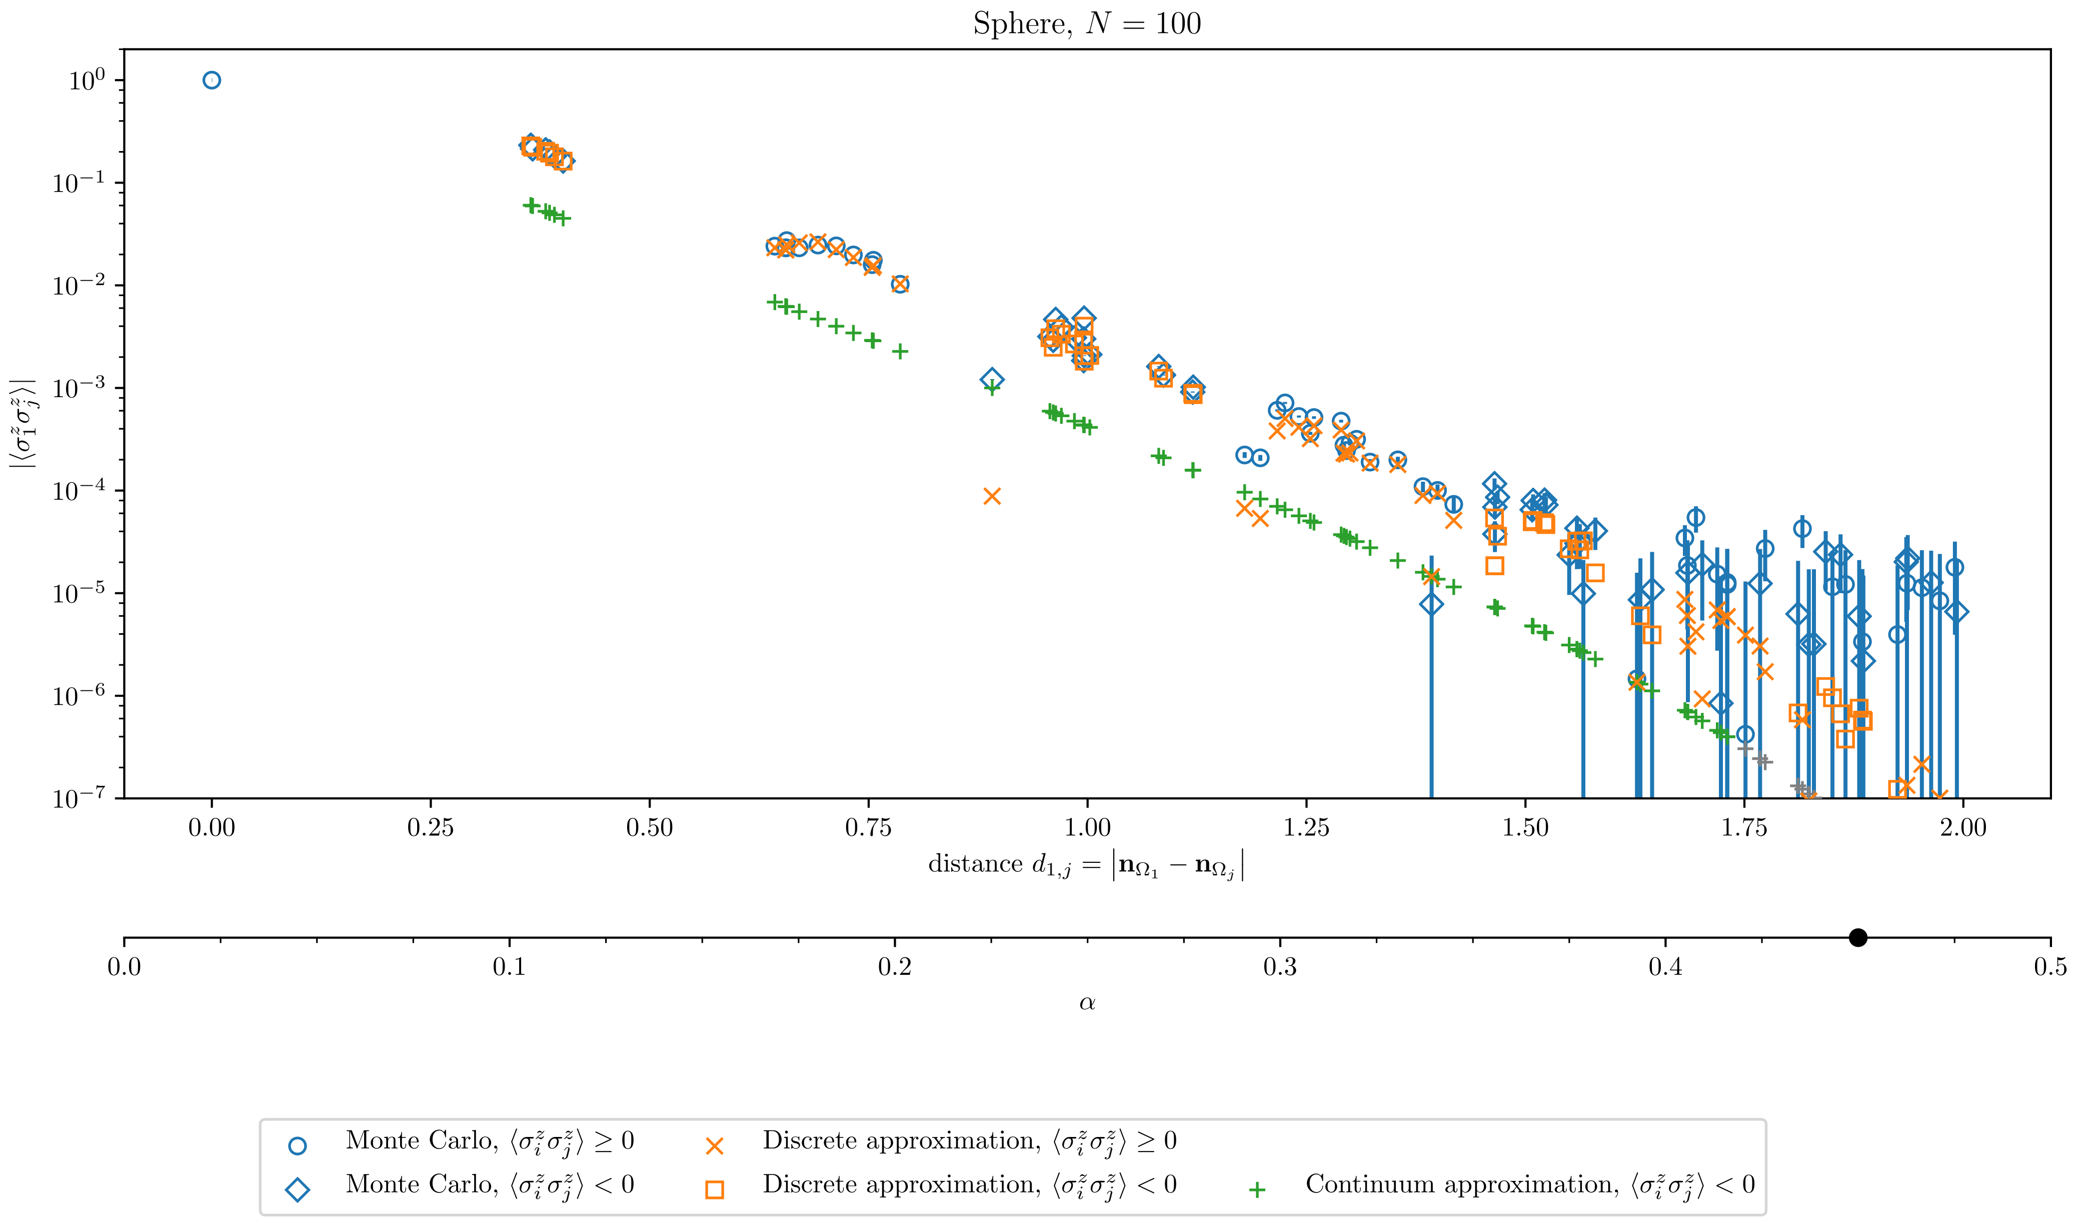

Sphere, $N = 100$
$|\langle \sigma_1^z \sigma_j^z \rangle|$
distance $d_{1,j} = |\mathbf{n}_{\Omega_1} - \mathbf{n}_{\Omega_j}|$
$\alpha$
Monte Carlo, $\langle \sigma_i^z \sigma_j^z \rangle \geq 0$
Monte Carlo, $\langle \sigma_i^z \sigma_j^z \rangle < 0$
Discrete approximation, $\langle \sigma_i^z \sigma_j^z \rangle \geq 0$
Discrete approximation, $\langle \sigma_i^z \sigma_j^z \rangle < 0$
Continuum approximation, $\langle \sigma_i^z \sigma_j^z \rangle < 0$

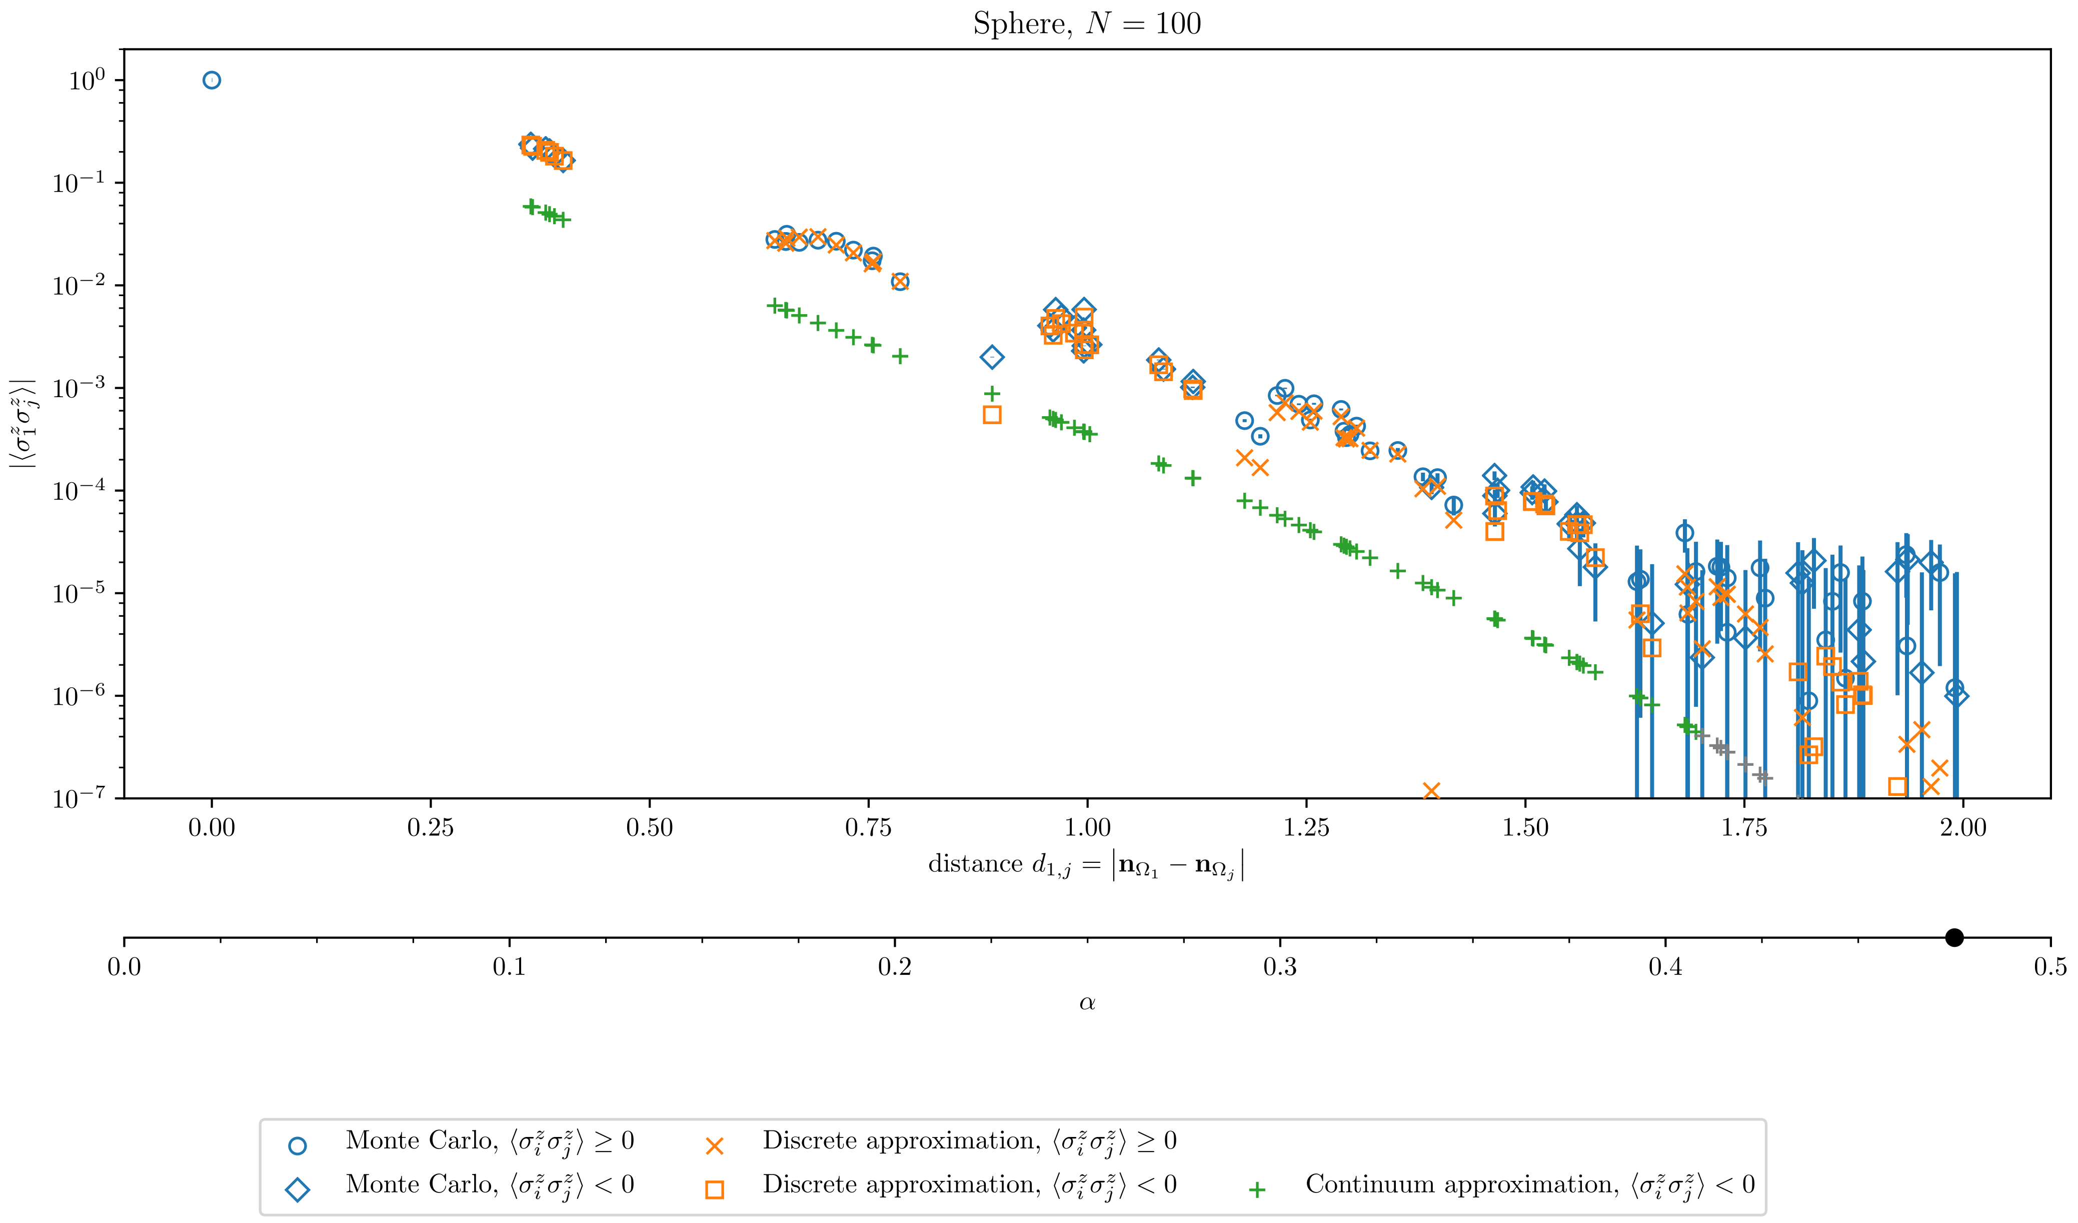

Sphere, $N = 100$
$|\langle \sigma_1^z \sigma_j^z \rangle|$
$10^0$
$10^{-1}$
$10^{-2}$
$10^{-3}$
$10^{-4}$
$10^{-5}$
$10^{-6}$
$10^{-7}$
0.00
0.25
0.50
0.75
1.00
1.25
1.50
1.75
2.00
distance $d_{1,j} = |\mathbf{n}_{\Omega_1} - \mathbf{n}_{\Omega_j}|$
0.0
0.1
0.2
0.3
0.4
0.5
$\alpha$
Monte Carlo, $\langle \sigma_i^z \sigma_j^z \rangle \geq 0$
Monte Carlo, $\langle \sigma_i^z \sigma_j^z \rangle < 0$
Discrete approximation, $\langle \sigma_i^z \sigma_j^z \rangle \geq 0$
Discrete approximation, $\langle \sigma_i^z \sigma_j^z \rangle < 0$
Continuum approximation, $\langle \sigma_i^z \sigma_j^z \rangle < 0$

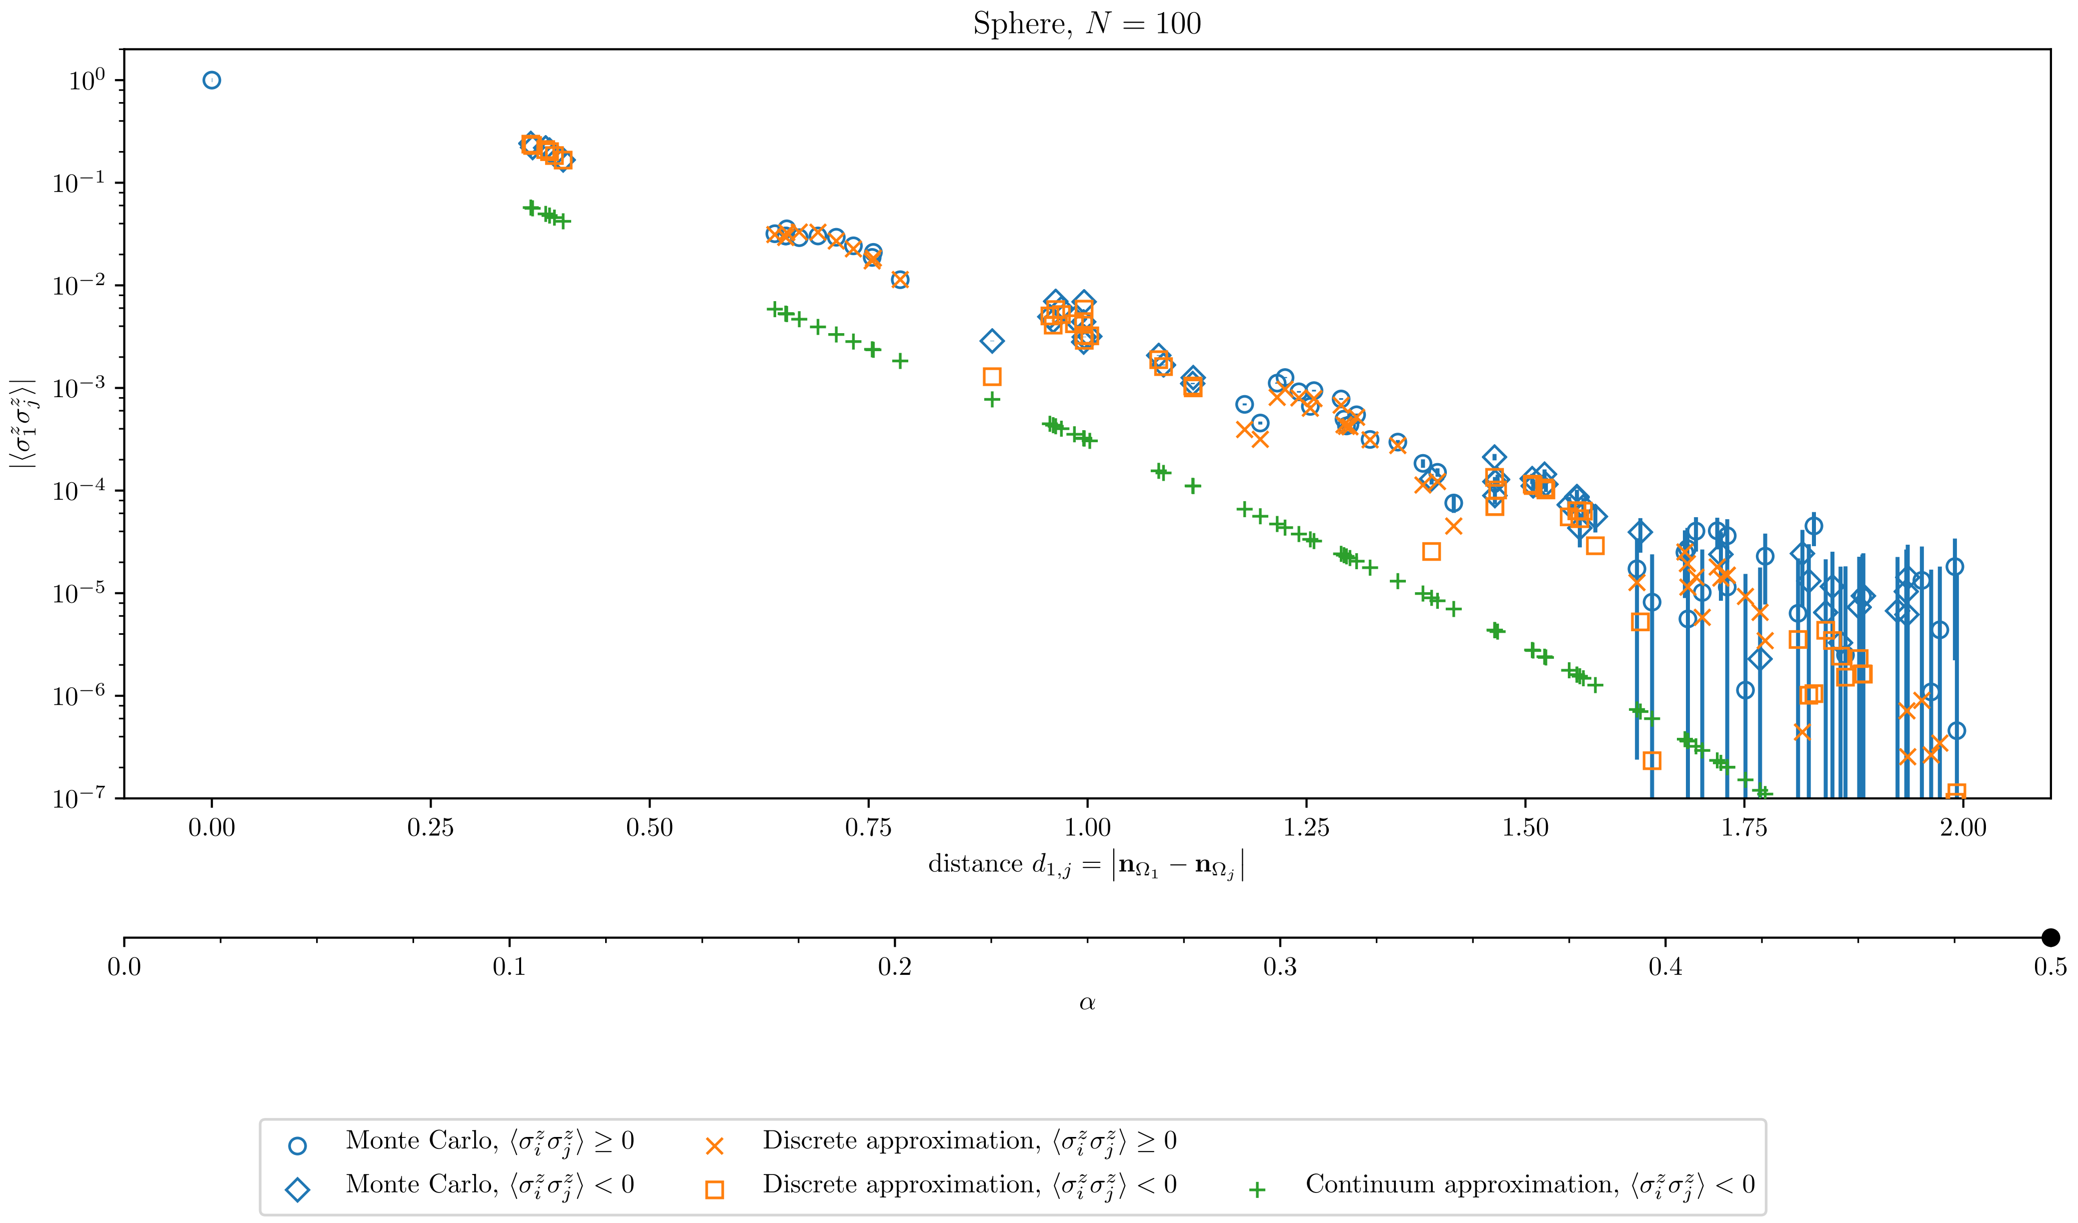

Sphere, $N = 100$
$|\langle\sigma_1^z\sigma_j^z\rangle|$
$10^0$
$10^{-1}$
$10^{-2}$
$10^{-3}$
$10^{-4}$
$10^{-5}$
$10^{-6}$
$10^{-7}$
0.00 0.25 0.50 0.75 1.00 1.25 1.50 1.75 2.00
distance $d_{1,j} = |\mathbf{n}_{\Omega_1} - \mathbf{n}_{\Omega_j}|$
0.0 0.1 0.2 0.3 0.4 0.5
$\alpha$
Monte Carlo, $\langle\sigma_i^z\sigma_j^z\rangle \geq 0$
Monte Carlo, $\langle\sigma_i^z\sigma_j^z\rangle < 0$
Discrete approximation, $\langle\sigma_i^z\sigma_j^z\rangle \geq 0$
Discrete approximation, $\langle\sigma_i^z\sigma_j^z\rangle < 0$
Continuum approximation, $\langle\sigma_i^z\sigma_j^z\rangle < 0$

I. Circle

II. Sphere

III. Cylinder (edge)

IV. Cylinder (bulk)

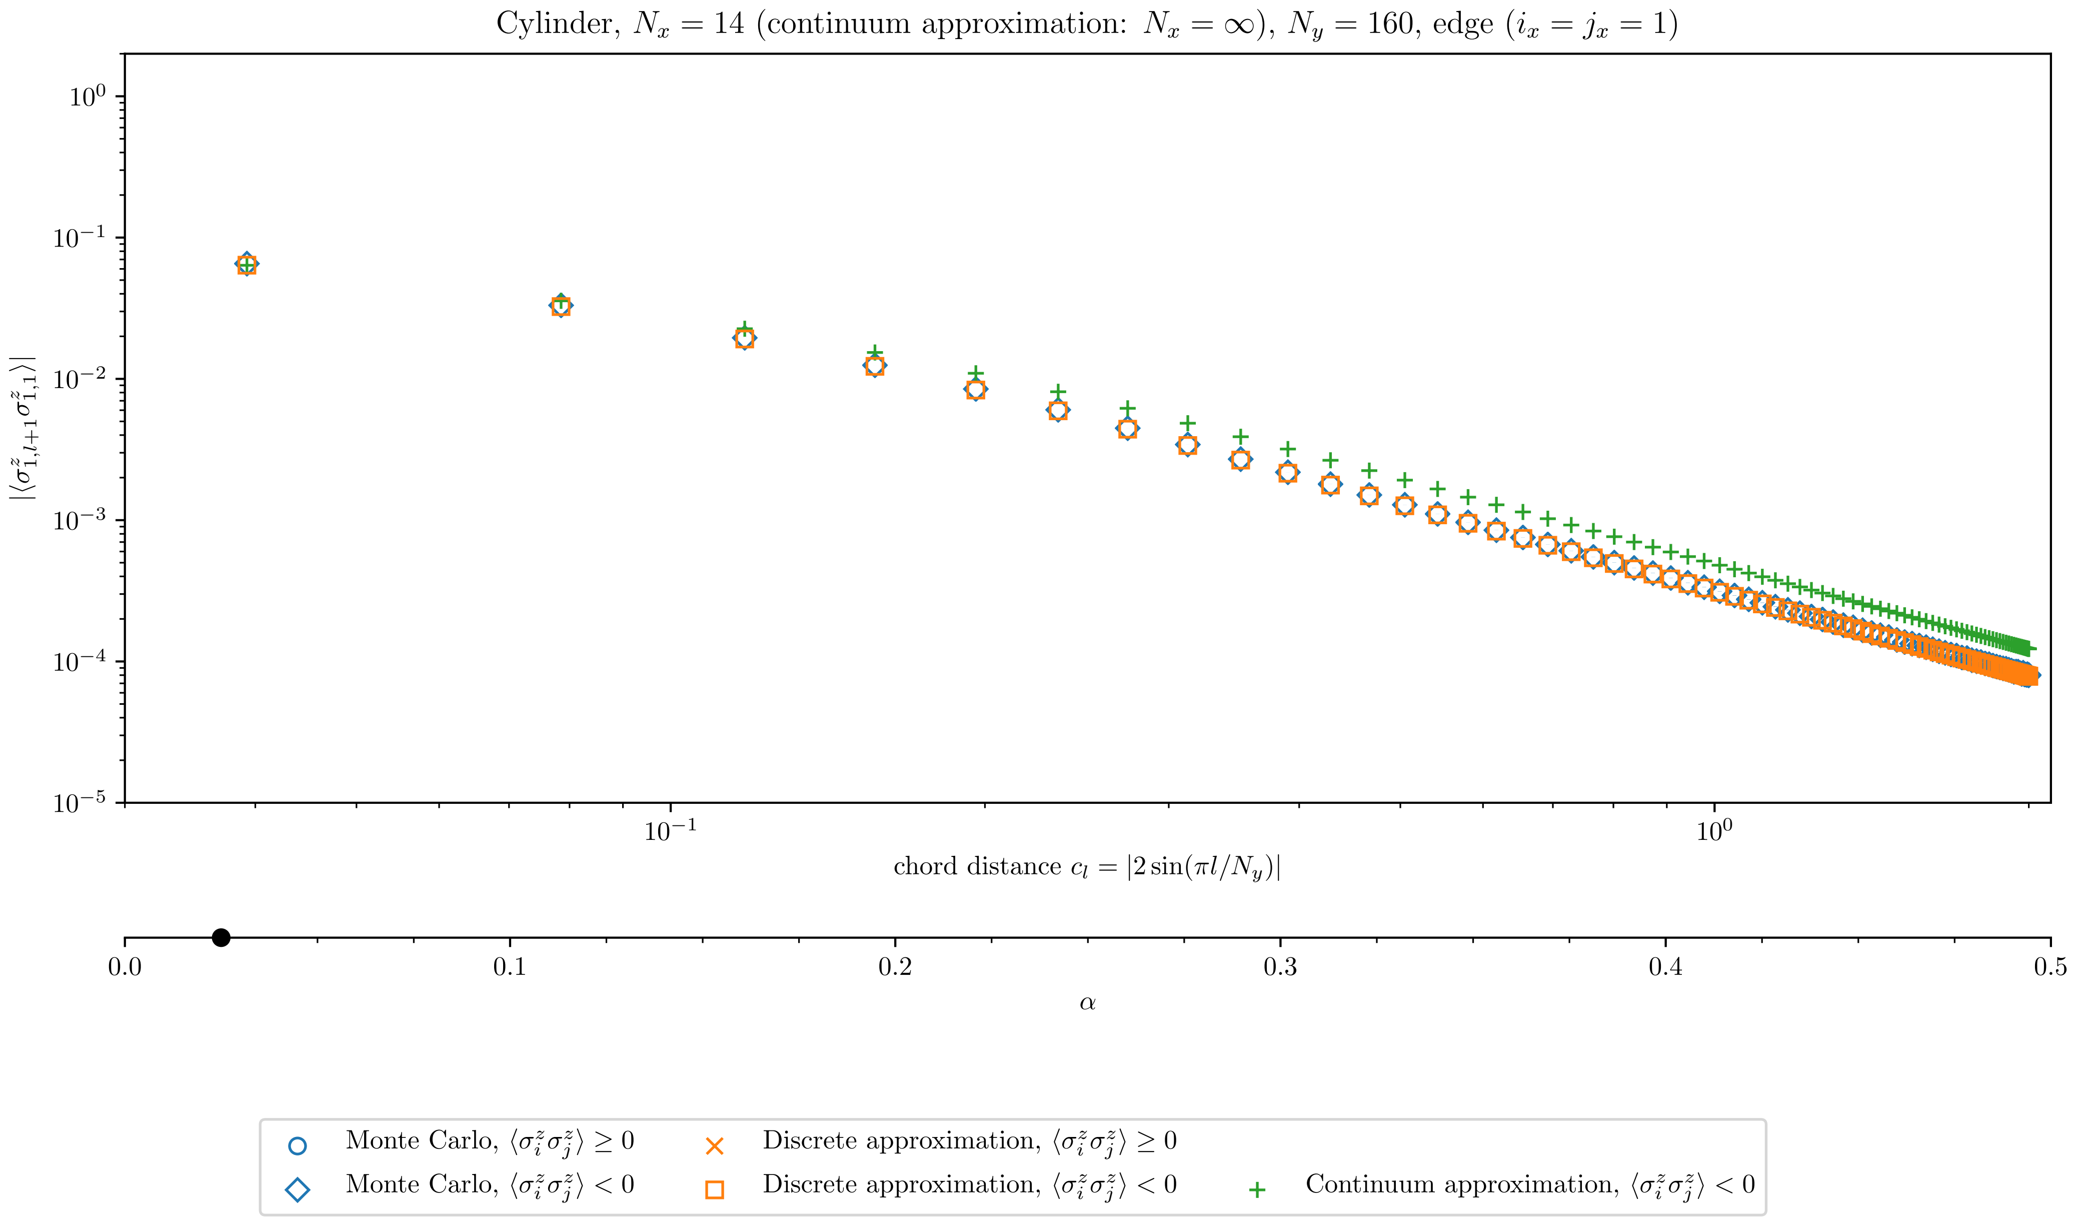

Cylinder, $N_x = 14$ (continuum approximation: $N_x = \infty$), $N_y = 160$, edge ($i_x = j_x = 1$)
$|\langle \sigma^z_{1,l+1} \sigma^z_{1,1} \rangle|$
$10^0$
$10^{-1}$
$10^{-2}$
$10^{-3}$
$10^{-4}$
$10^{-5}$
$10^{-1}$
$10^0$
chord distance $c_l = |2\sin(\pi l/N_y)|$
0.0
0.1
0.2
0.3
0.4
0.5
$\alpha$
Monte Carlo, $\langle \sigma^z_i \sigma^z_j \rangle \geq 0$
Monte Carlo, $\langle \sigma^z_i \sigma^z_j \rangle < 0$
Discrete approximation, $\langle \sigma^z_i \sigma^z_j \rangle \geq 0$
Discrete approximation, $\langle \sigma^z_i \sigma^z_j \rangle < 0$
Continuum approximation, $\langle \sigma^z_i \sigma^z_j \rangle < 0$

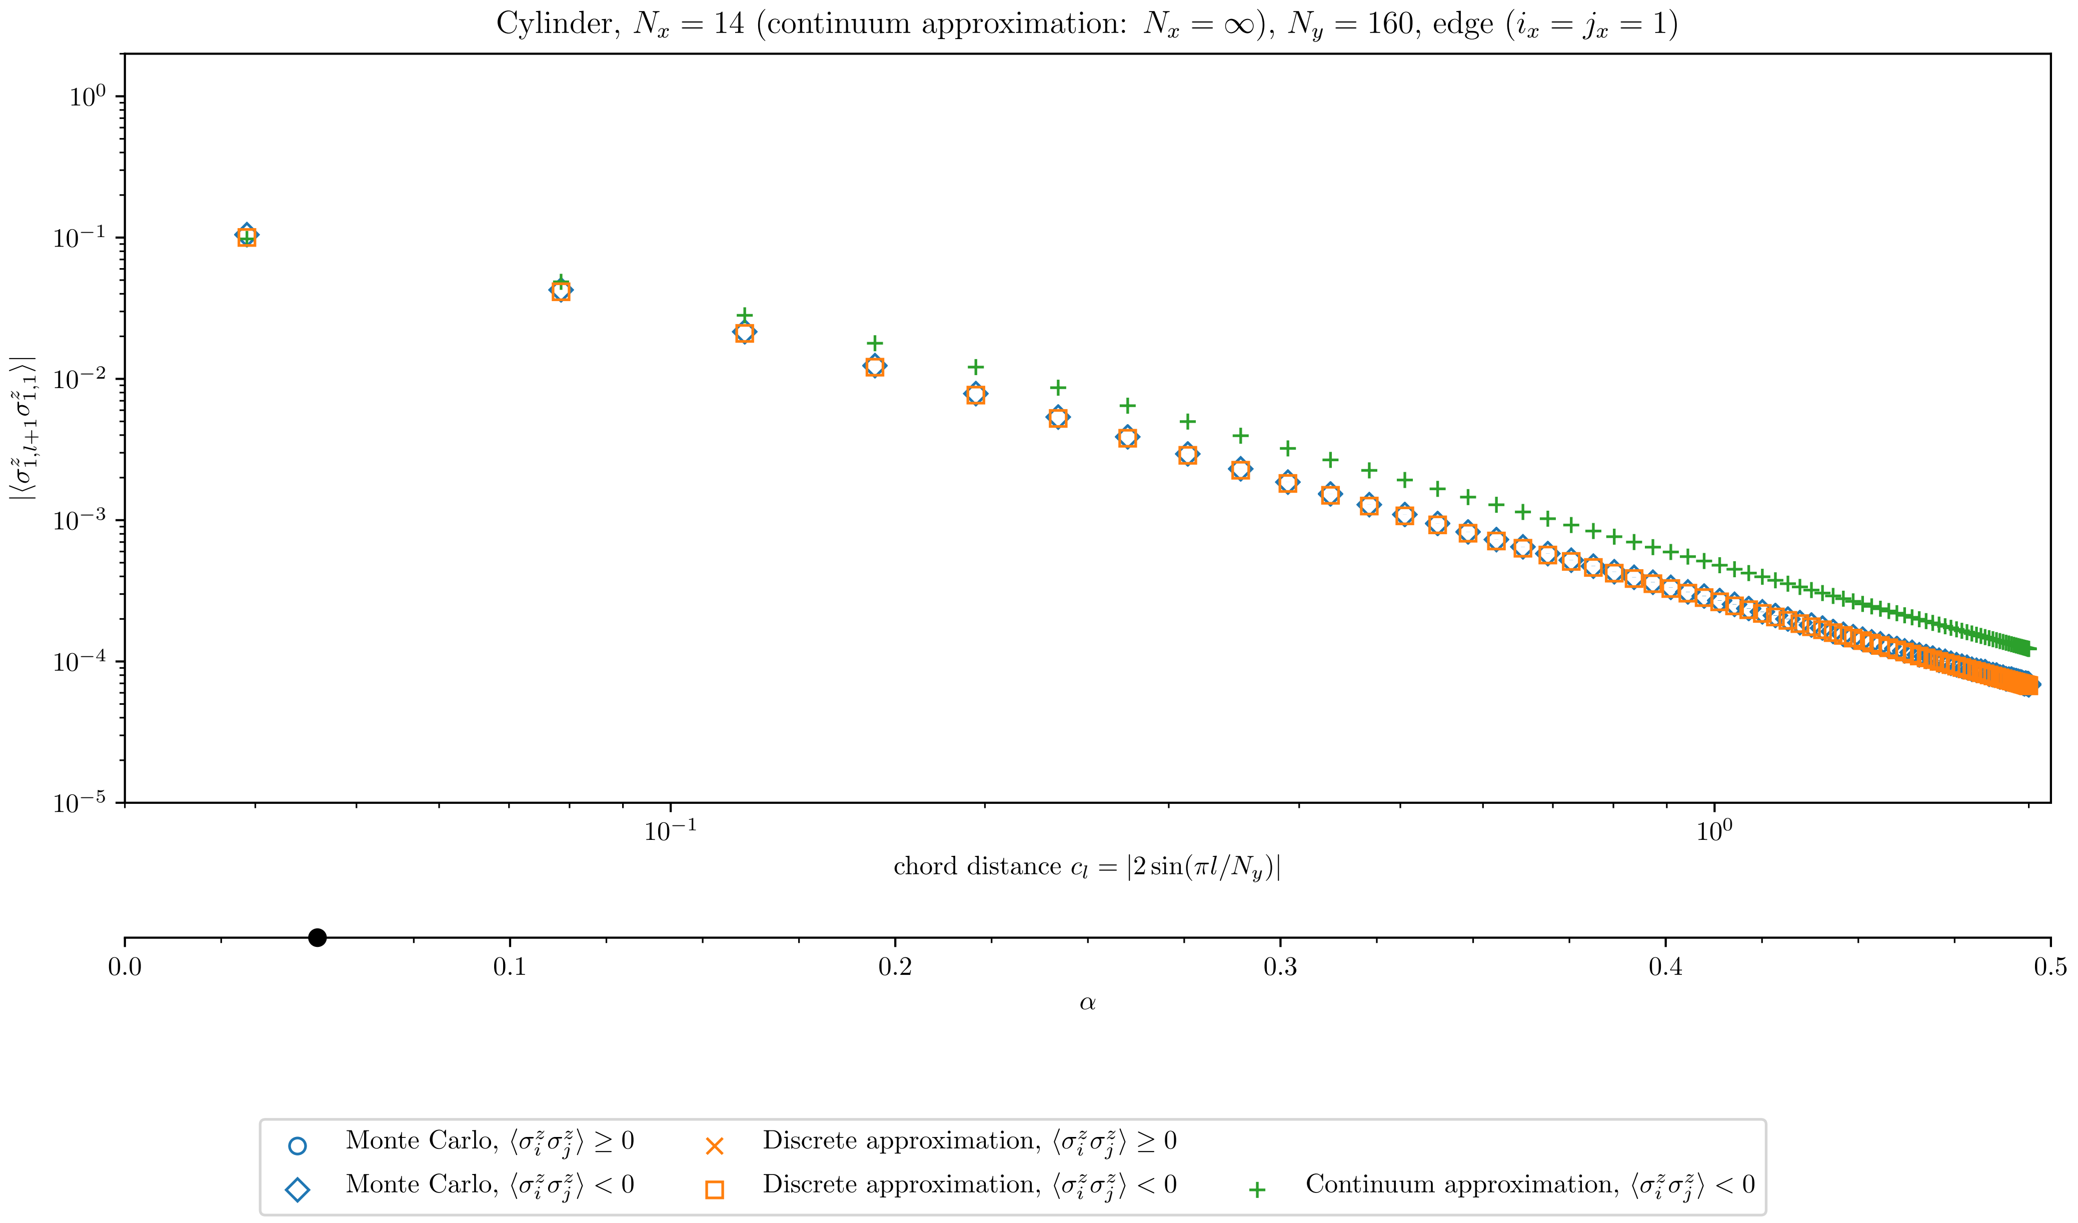

Cylinder, $N_x = 14$ (continuum approximation: $N_x = \infty$), $N_y = 160$, edge ($i_x = j_x = 1$)
$|\langle \sigma^z_{1,l+1} \sigma^z_{1,1} \rangle|$
$10^0$
$10^{-1}$
$10^{-2}$
$10^{-3}$
$10^{-4}$
$10^{-5}$
$10^{-1}$
$10^0$
chord distance $c_l = |2\sin(\pi l/N_y)|$
0.0
0.1
0.2
0.3
0.4
0.5
$\alpha$
Monte Carlo, $\langle \sigma^z_i \sigma^z_j \rangle \geq 0$
Monte Carlo, $\langle \sigma^z_i \sigma^z_j \rangle < 0$
Discrete approximation, $\langle \sigma^z_i \sigma^z_j \rangle \geq 0$
Discrete approximation, $\langle \sigma^z_i \sigma^z_j \rangle < 0$
Continuum approximation, $\langle \sigma^z_i \sigma^z_j \rangle < 0$

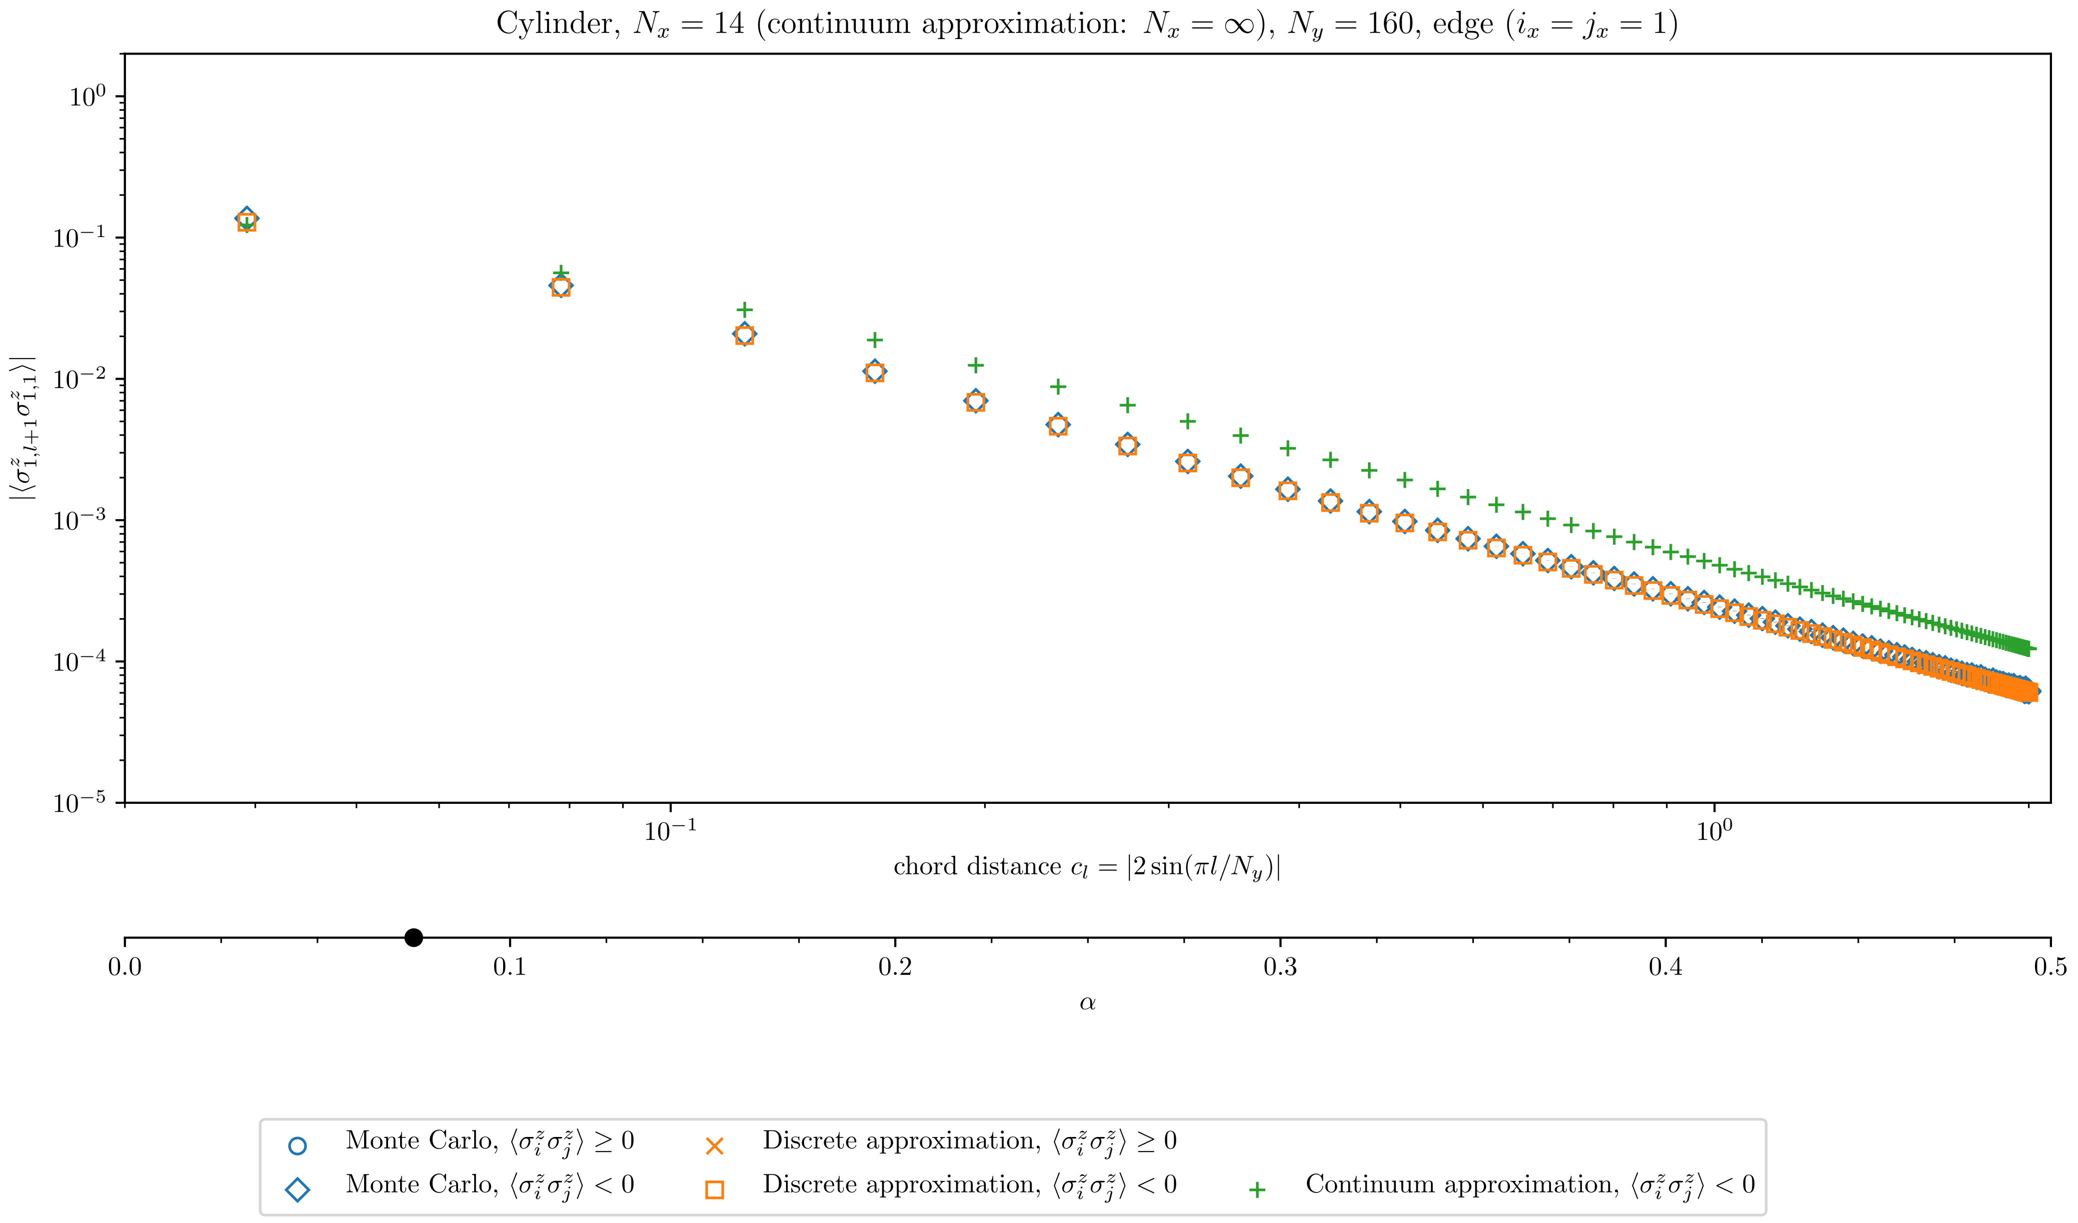

Cylinder, $N_x = 14$ (continuum approximation: $N_x = \infty$), $N_y = 160$, edge ($i_x = j_x = 1$)
$|\langle \sigma^z_{1,l+1} \sigma^z_{1,1} \rangle|$
$10^0$
$10^{-1}$
$10^{-2}$
$10^{-3}$
$10^{-4}$
$10^{-5}$
$10^{-1}$
$10^0$
chord distance $c_l = |2\sin(\pi l/N_y)|$
0.0
0.1
0.2
0.3
0.4
0.5
$\alpha$
Monte Carlo, $\langle \sigma^z_i \sigma^z_j \rangle \geq 0$
Monte Carlo, $\langle \sigma^z_i \sigma^z_j \rangle < 0$
Discrete approximation, $\langle \sigma^z_i \sigma^z_j \rangle \geq 0$
Discrete approximation, $\langle \sigma^z_i \sigma^z_j \rangle < 0$
Continuum approximation, $\langle \sigma^z_i \sigma^z_j \rangle < 0$

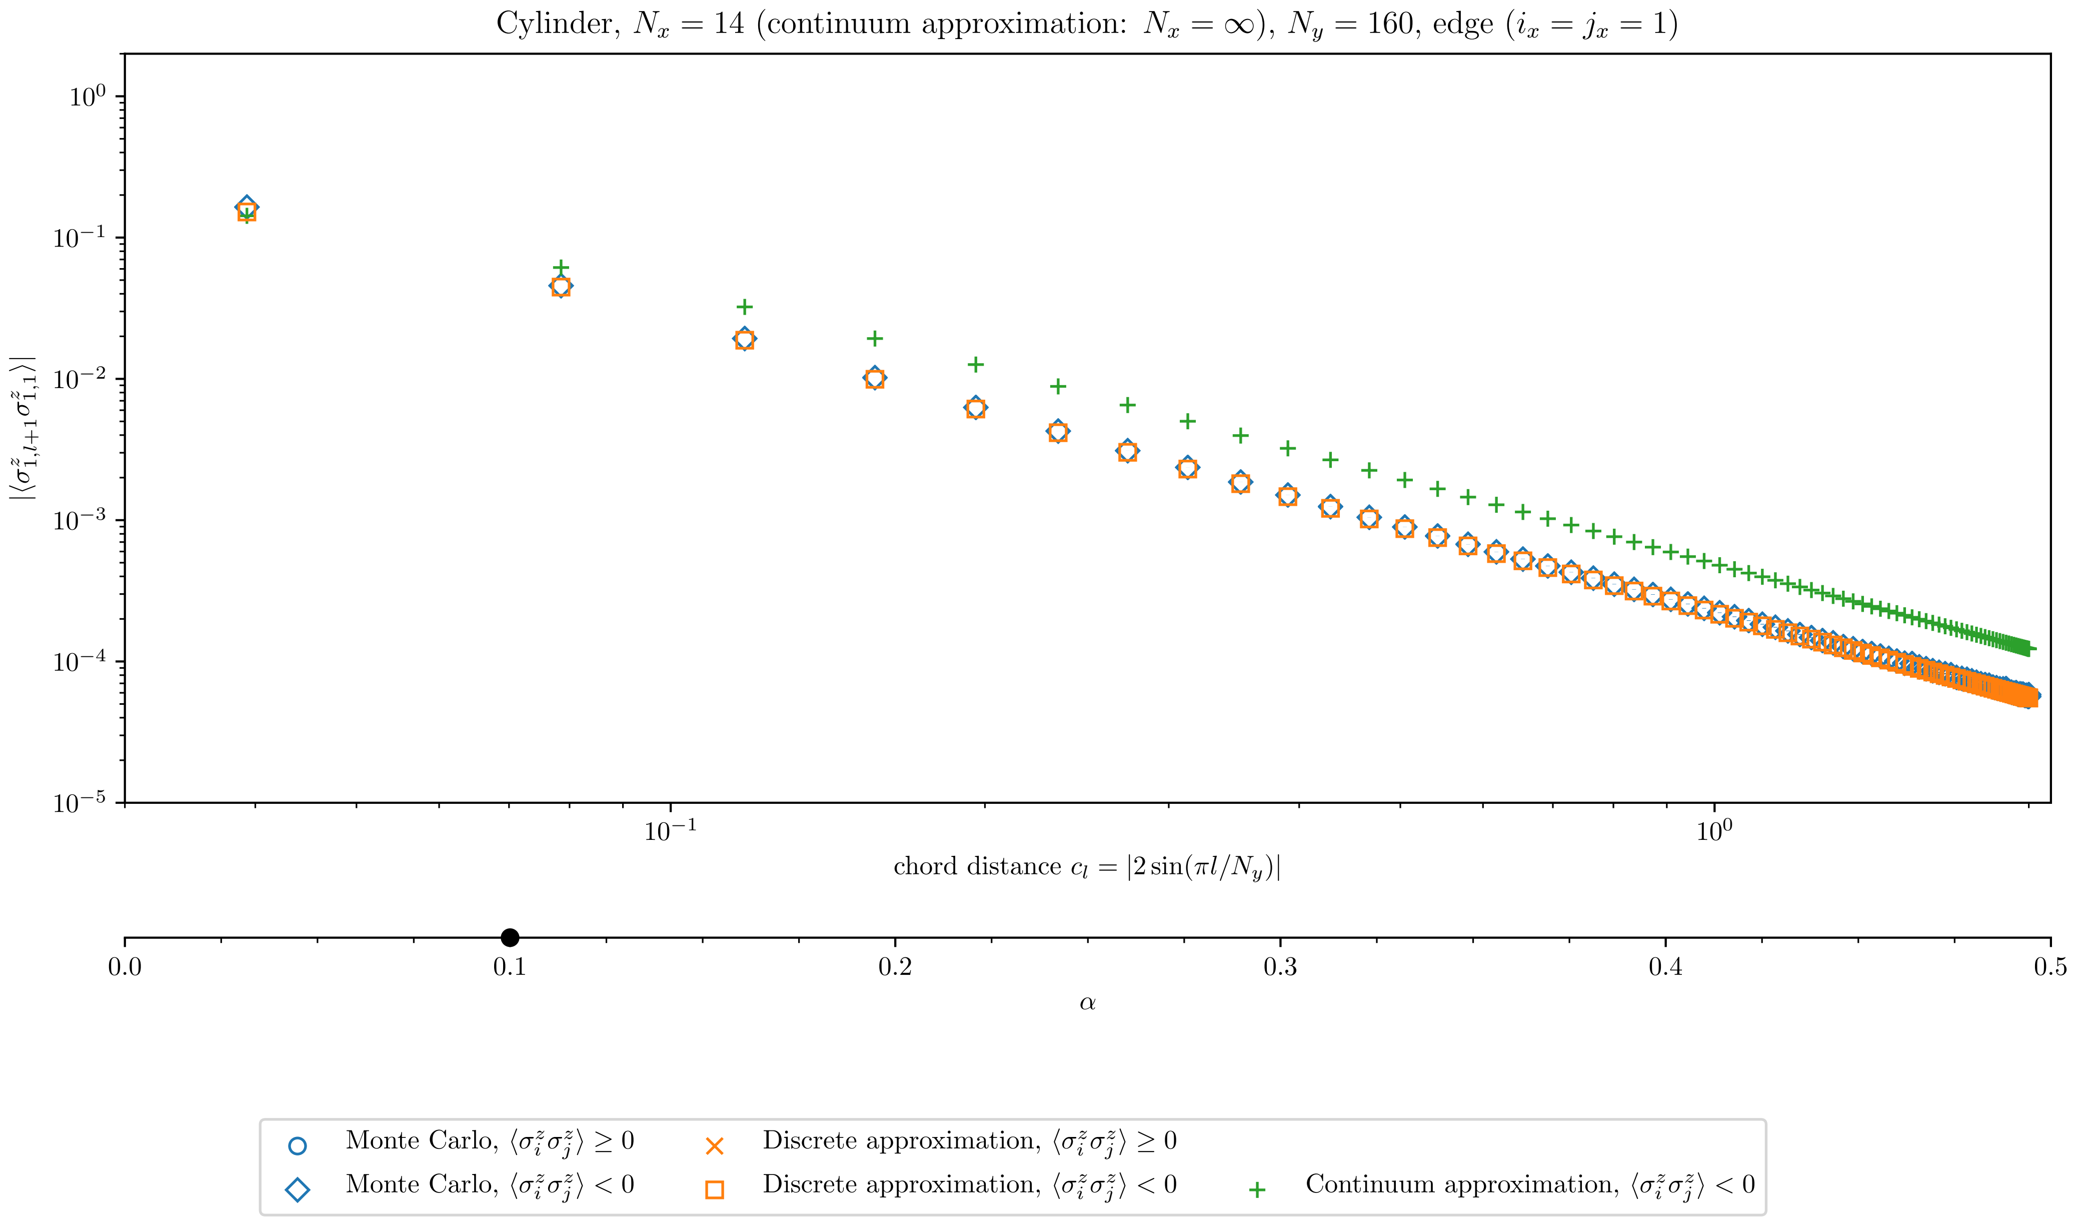

Cylinder, $N_x = 14$ (continuum approximation: $N_x = \infty$), $N_y = 160$, edge ($i_x = j_x = 1$)
$|\langle \sigma^z_{1,l+1} \sigma^z_{1,1} \rangle|$
$10^0$
$10^{-1}$
$10^{-2}$
$10^{-3}$
$10^{-4}$
$10^{-5}$
$10^{-1}$
$10^0$
chord distance $c_l = |2\sin(\pi l/N_y)|$
0.0
0.1
0.2
0.3
0.4
0.5
$\alpha$
Monte Carlo, $\langle \sigma^z_i \sigma^z_j \rangle \geq 0$
Monte Carlo, $\langle \sigma^z_i \sigma^z_j \rangle < 0$
Discrete approximation, $\langle \sigma^z_i \sigma^z_j \rangle \geq 0$
Discrete approximation, $\langle \sigma^z_i \sigma^z_j \rangle < 0$
Continuum approximation, $\langle \sigma^z_i \sigma^z_j \rangle < 0$

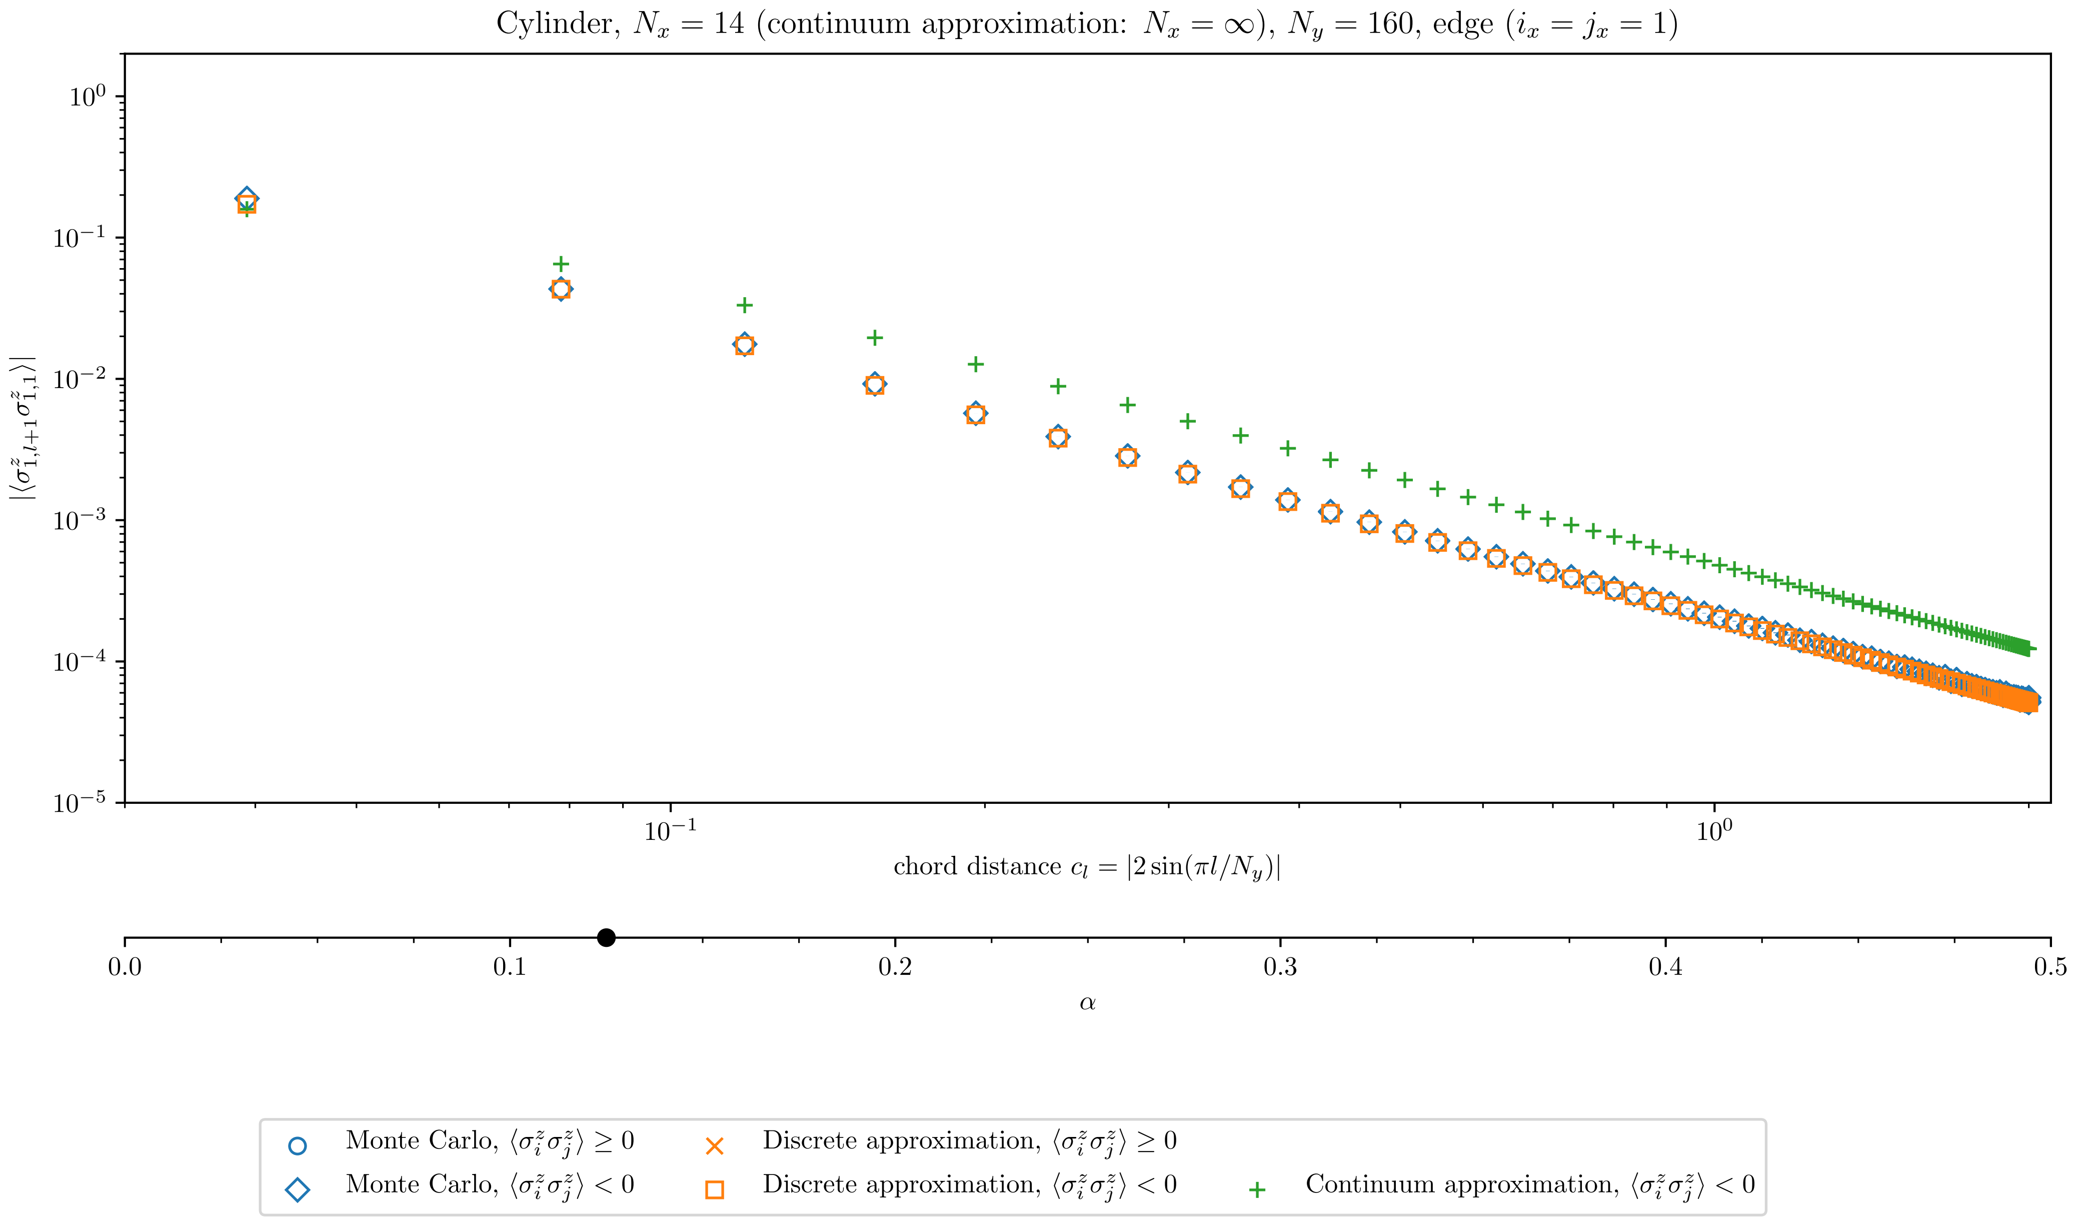

Cylinder, $N_x = 14$ (continuum approximation: $N_x = \infty$), $N_y = 160$, edge ($i_x = j_x = 1$)
$|\langle \sigma^z_{1,l+1} \sigma^z_{1,1} \rangle|$
$10^0$
$10^{-1}$
$10^{-2}$
$10^{-3}$
$10^{-4}$
$10^{-5}$
$10^{-1}$
$10^0$
chord distance $c_l = |2\sin(\pi l/N_y)|$
0.0
0.1
0.2
0.3
0.4
0.5
$\alpha$
Monte Carlo, $\langle \sigma^z_i \sigma^z_j \rangle \geq 0$
Monte Carlo, $\langle \sigma^z_i \sigma^z_j \rangle < 0$
Discrete approximation, $\langle \sigma^z_i \sigma^z_j \rangle \geq 0$
Discrete approximation, $\langle \sigma^z_i \sigma^z_j \rangle < 0$
Continuum approximation, $\langle \sigma^z_i \sigma^z_j \rangle < 0$

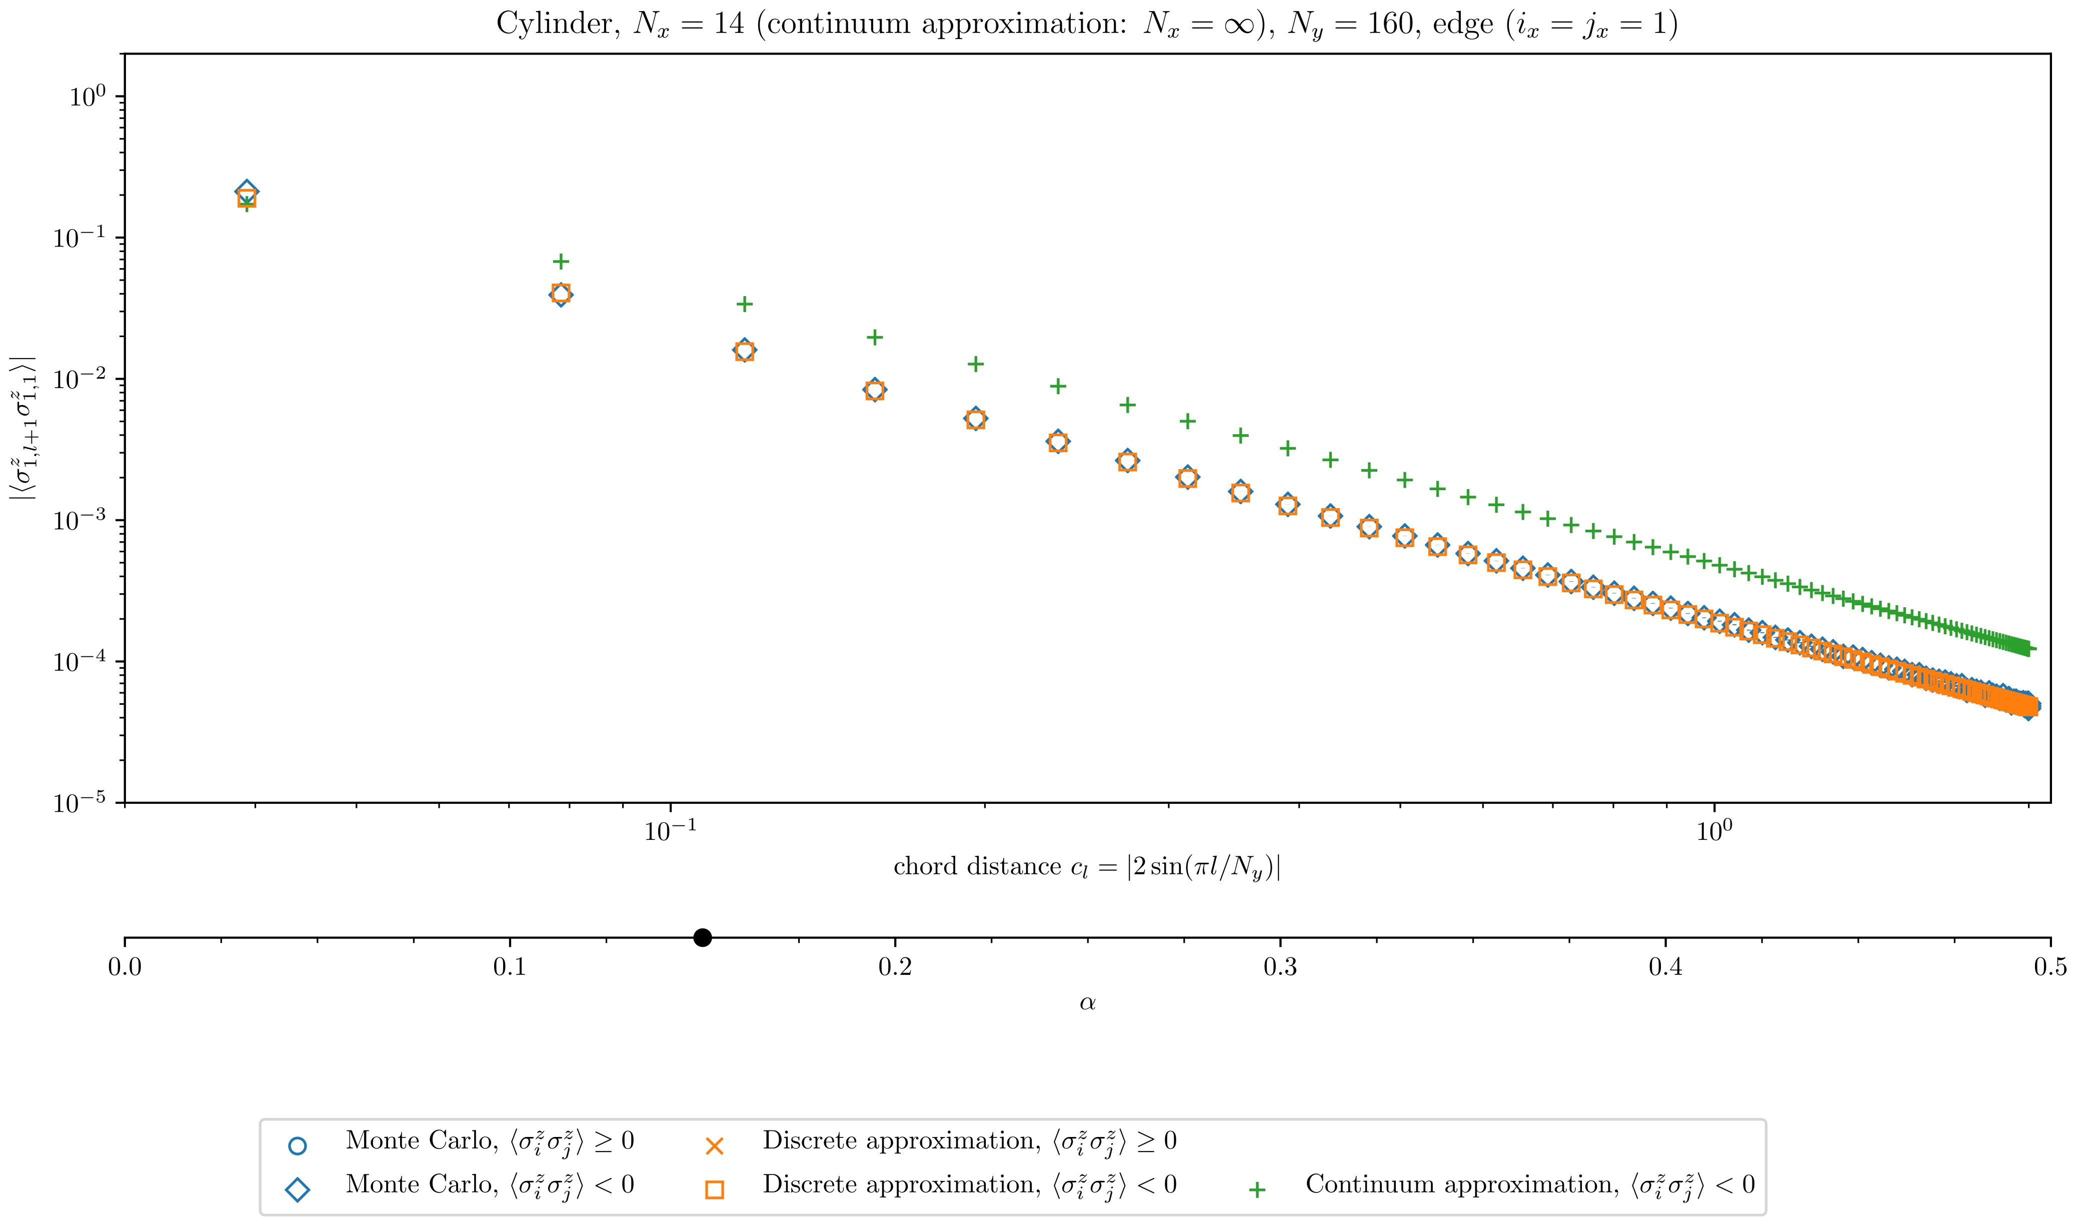

Cylinder, $N_x = 14$ (continuum approximation: $N_x = \infty$), $N_y = 160$, edge ($i_x = j_x = 1$)
$|\langle \sigma^z_{1,l+1} \sigma^z_{1,1} \rangle|$
$10^0$
$10^{-1}$
$10^{-2}$
$10^{-3}$
$10^{-4}$
$10^{-5}$
$10^{-1}$
$10^0$
chord distance $c_l = |2\sin(\pi l/N_y)|$
0.0
0.1
0.2
0.3
0.4
0.5
$\alpha$
Monte Carlo, $\langle \sigma^z_i \sigma^z_j \rangle \geq 0$
Monte Carlo, $\langle \sigma^z_i \sigma^z_j \rangle < 0$
Discrete approximation, $\langle \sigma^z_i \sigma^z_j \rangle \geq 0$
Discrete approximation, $\langle \sigma^z_i \sigma^z_j \rangle < 0$
Continuum approximation, $\langle \sigma^z_i \sigma^z_j \rangle < 0$

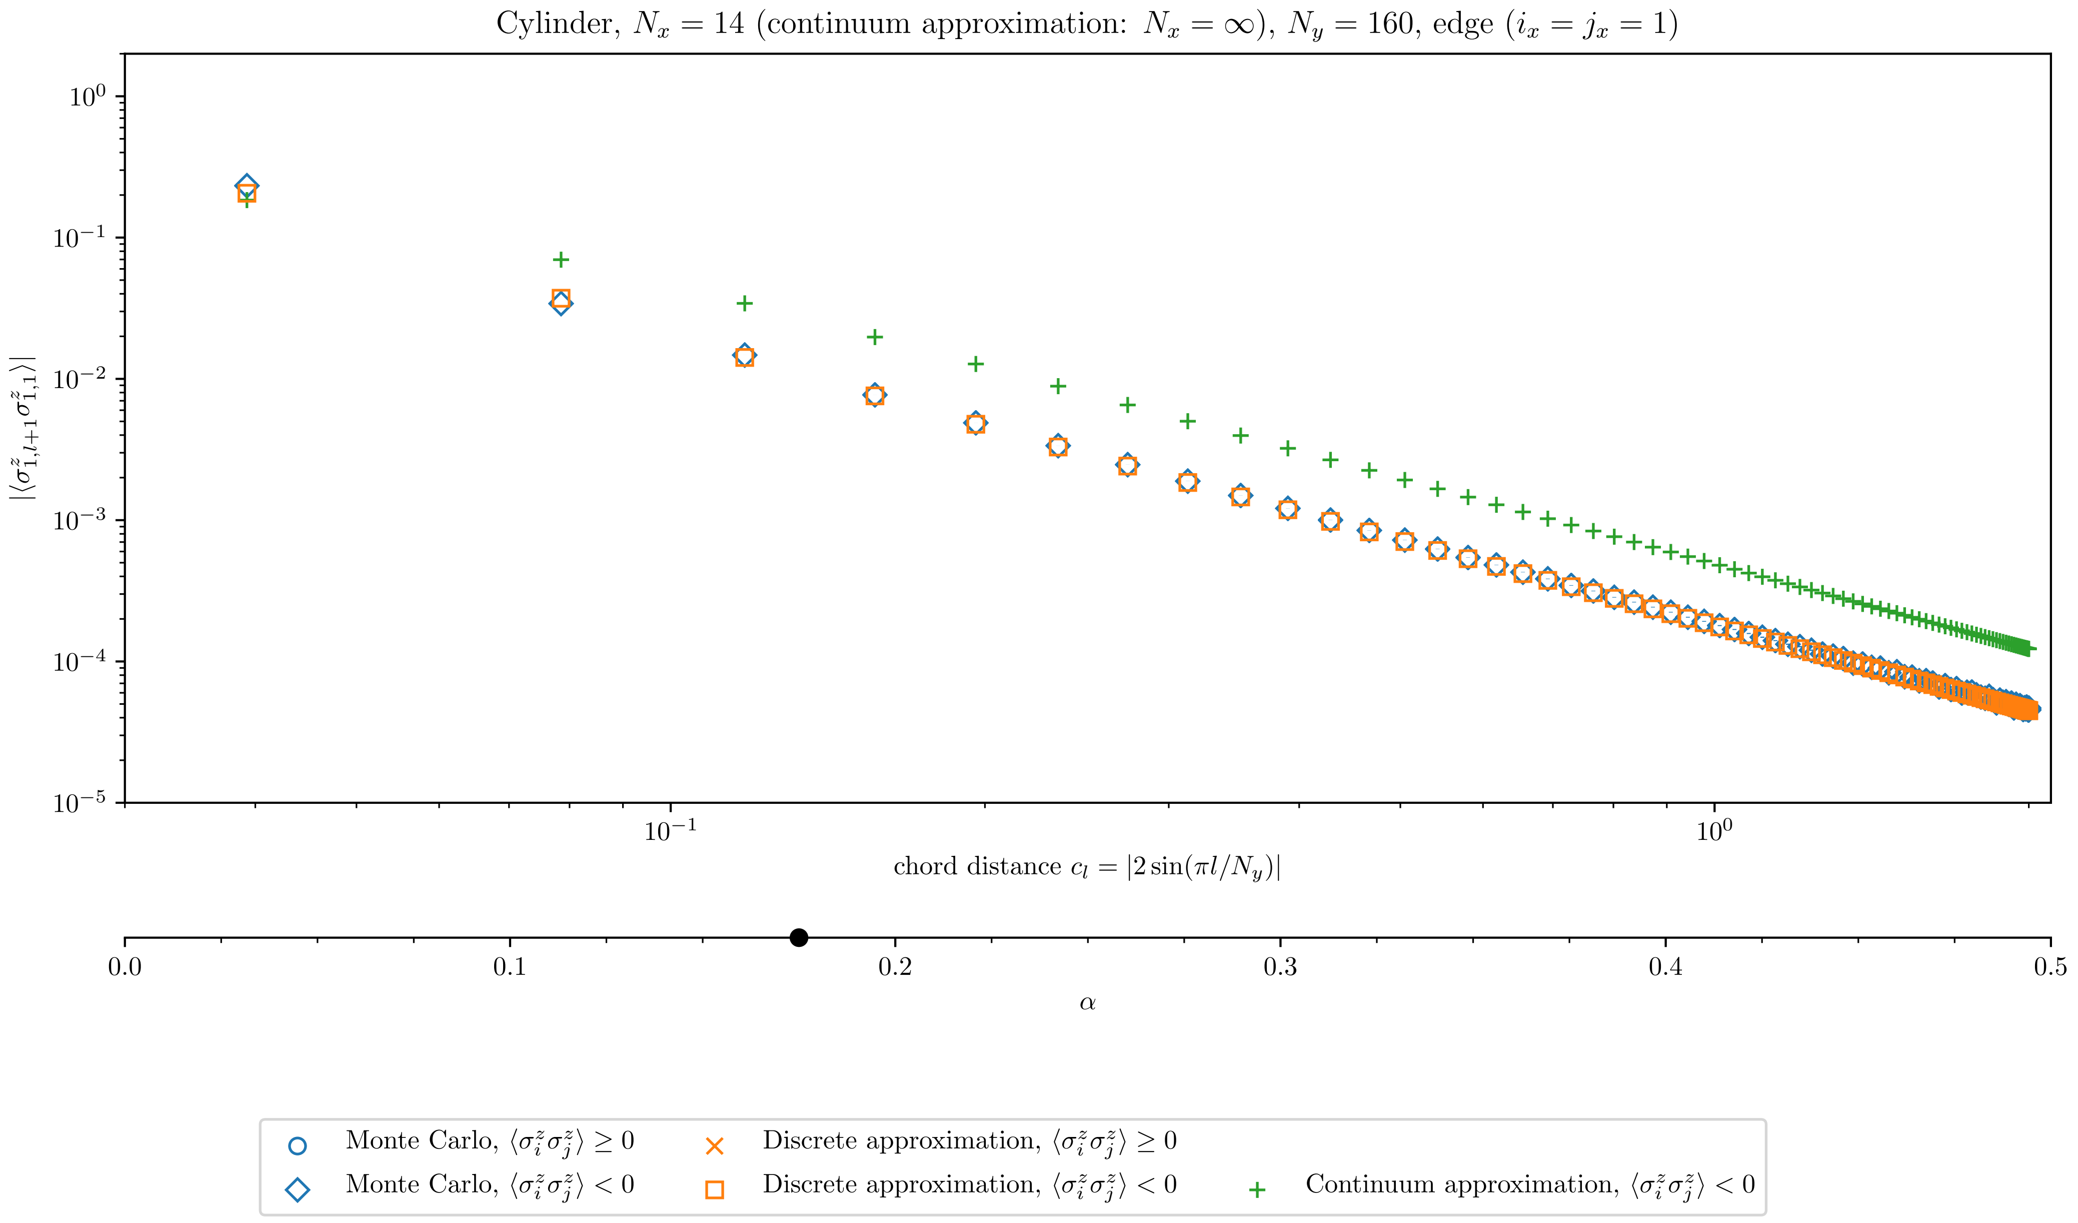

Cylinder, $N_x = 14$ (continuum approximation: $N_x = \infty$), $N_y = 160$, edge ($i_x = j_x = 1$)
$|\langle \sigma^z_{1,l+1}\sigma^z_{1,1}\rangle|$
$10^0$
$10^{-1}$
$10^{-2}$
$10^{-3}$
$10^{-4}$
$10^{-5}$
$10^{-1}$
$10^0$
chord distance $c_l = |2\sin(\pi l/N_y)|$
0.0
0.1
0.2
0.3
0.4
0.5
$\alpha$
Monte Carlo, $\langle \sigma^z_i \sigma^z_j\rangle \geq 0$
Monte Carlo, $\langle \sigma^z_i \sigma^z_j\rangle < 0$
Discrete approximation, $\langle \sigma^z_i \sigma^z_j\rangle \geq 0$
Discrete approximation, $\langle \sigma^z_i \sigma^z_j\rangle < 0$
Continuum approximation, $\langle \sigma^z_i \sigma^z_j\rangle < 0$

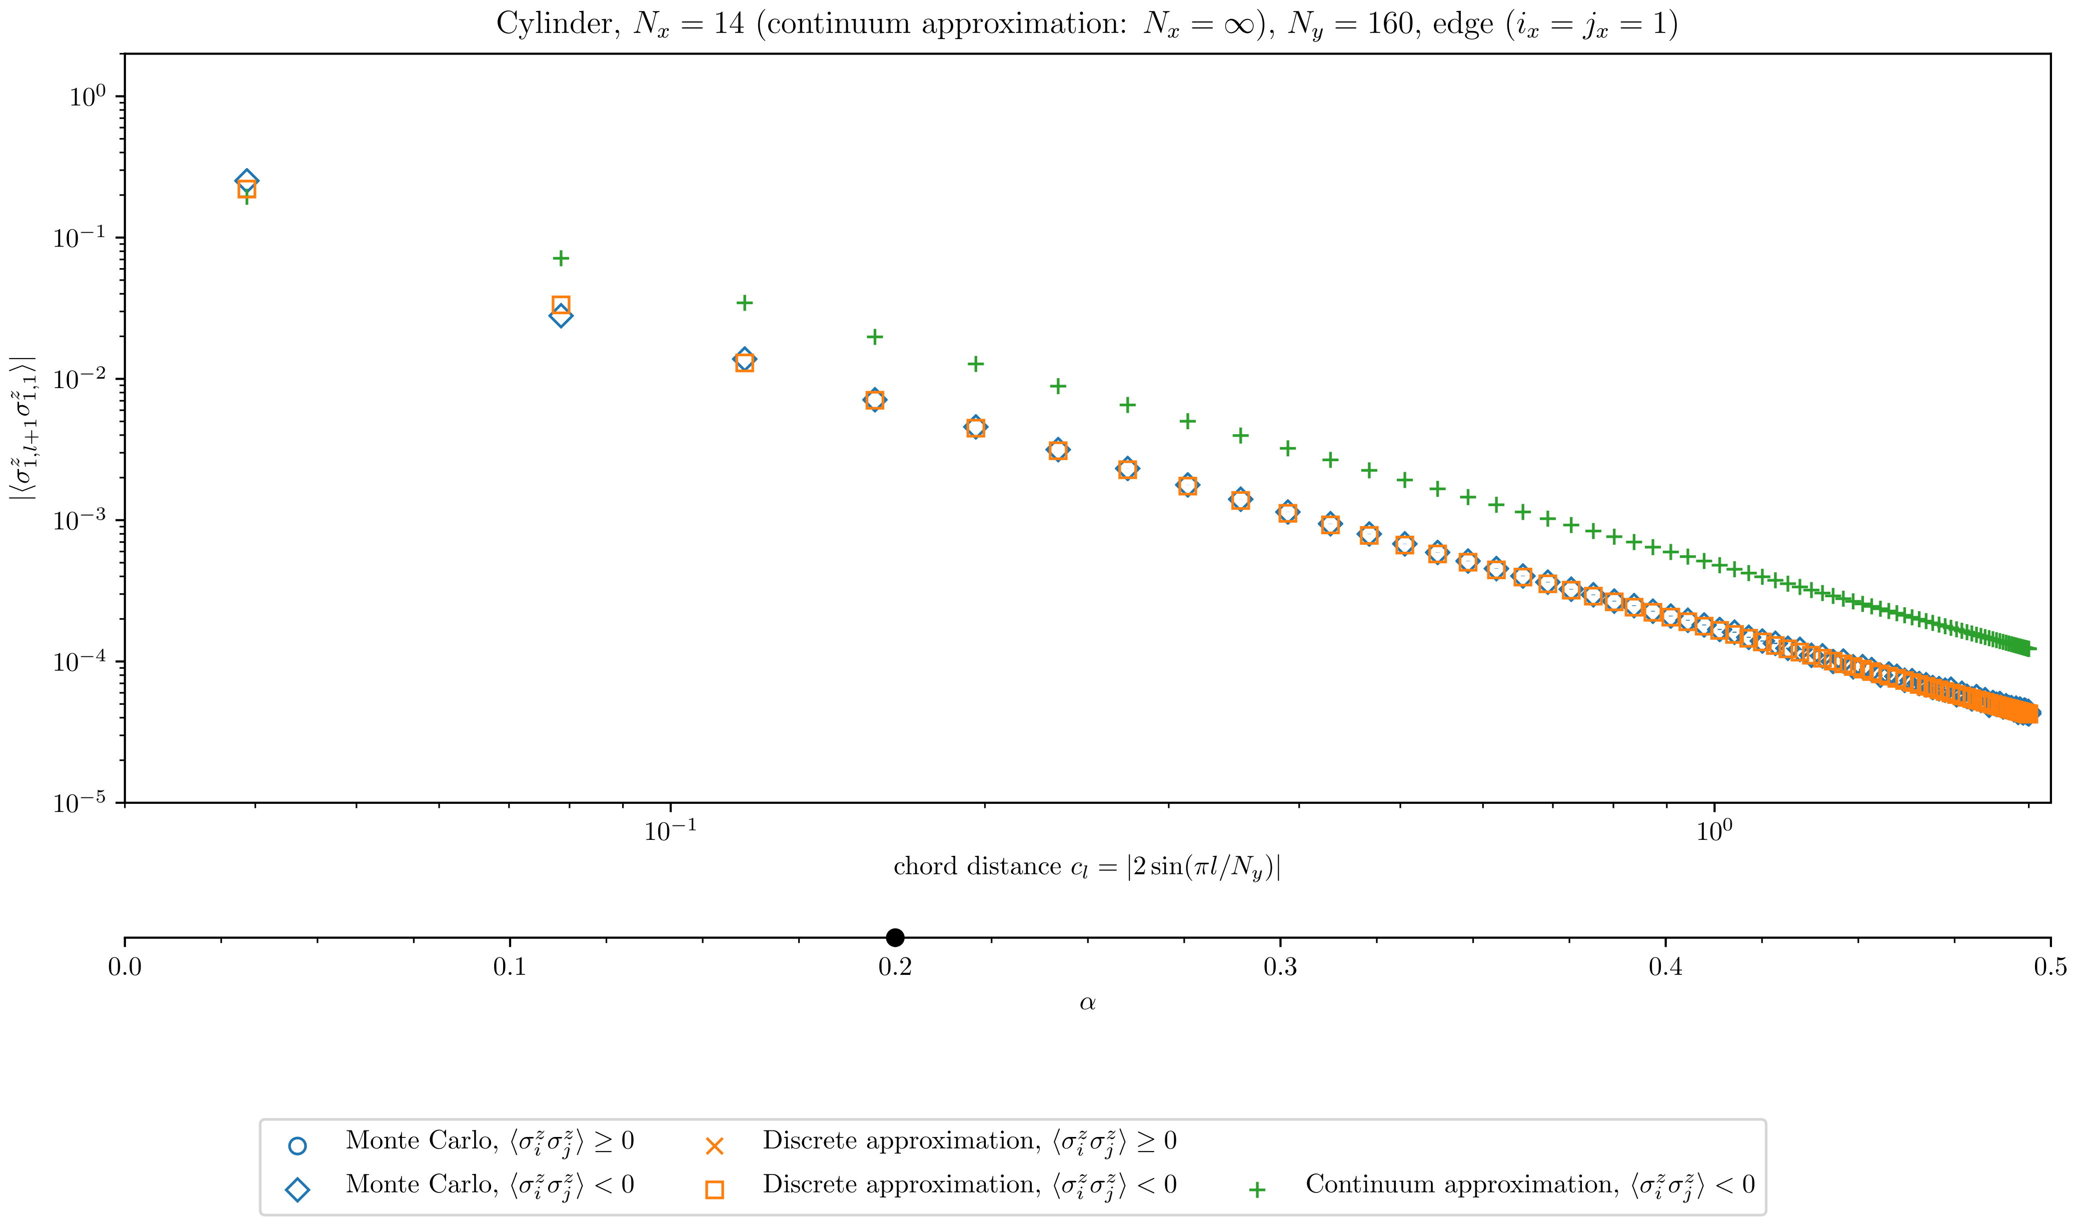

Cylinder, $N_x = 14$ (continuum approximation: $N_x = \infty$), $N_y = 160$, edge ($i_x = j_x = 1$)
$|\langle \sigma^z_{1,l+1} \sigma^z_{1,1} \rangle|$
$10^0$
$10^{-1}$
$10^{-2}$
$10^{-3}$
$10^{-4}$
$10^{-5}$
$10^{-1}$
$10^{0}$
chord distance $c_l = |2 \sin(\pi l / N_y)|$
0.0
0.1
0.2
0.3
0.4
0.5
$\alpha$
Monte Carlo, $\langle \sigma^z_i \sigma^z_j \rangle \geq 0$
Monte Carlo, $\langle \sigma^z_i \sigma^z_j \rangle < 0$
Discrete approximation, $\langle \sigma^z_i \sigma^z_j \rangle \geq 0$
Discrete approximation, $\langle \sigma^z_i \sigma^z_j \rangle < 0$
Continuum approximation, $\langle \sigma^z_i \sigma^z_j \rangle < 0$

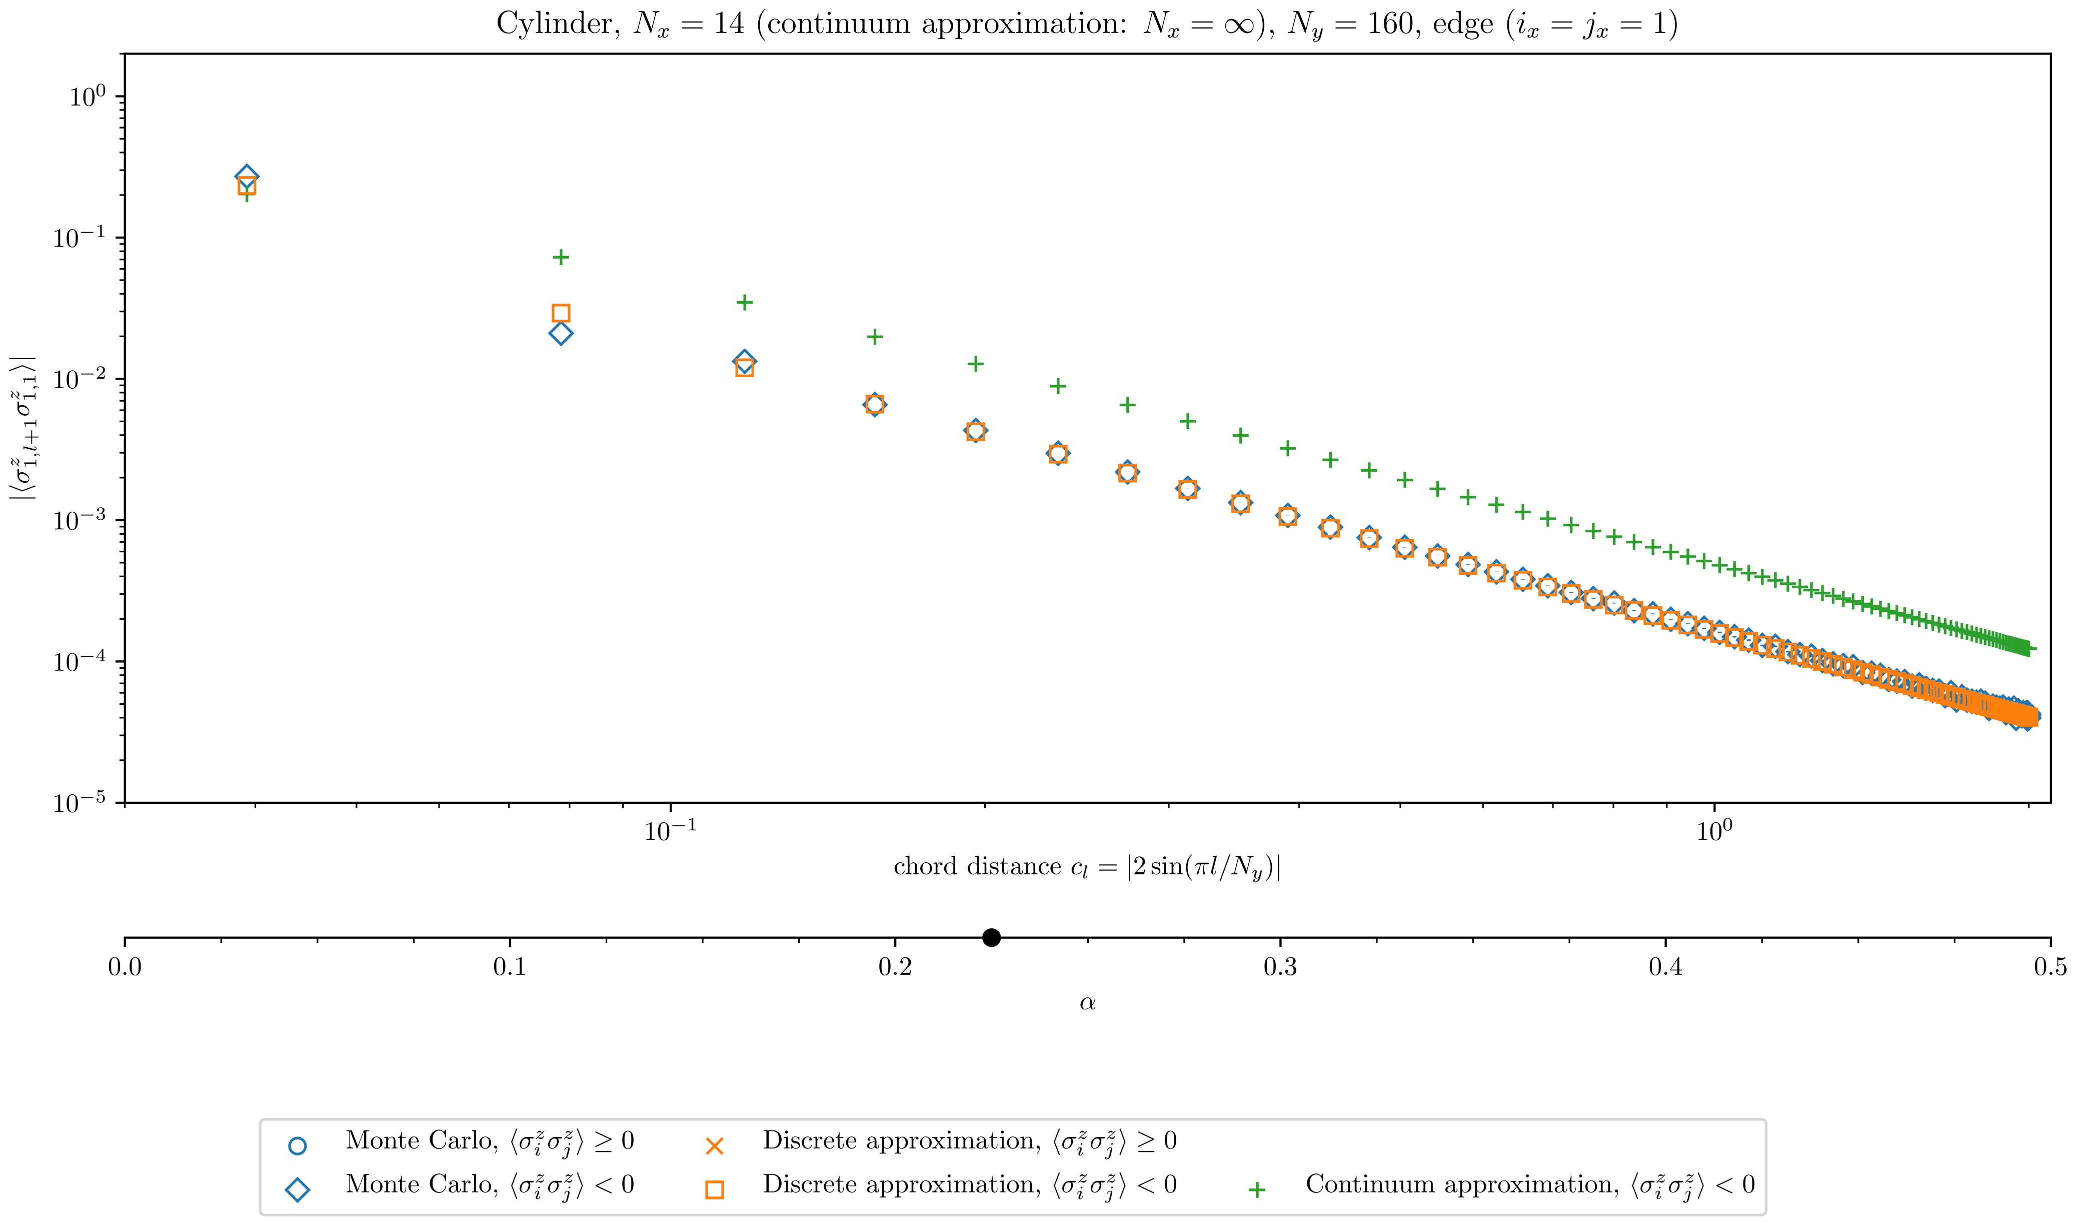

Cylinder, $N_x = 14$ (continuum approximation: $N_x = \infty$), $N_y = 160$, edge ($i_x = j_x = 1$)
$|\langle \sigma^z_{1,l+1} \sigma^z_{1,1} \rangle|$
$10^0$
$10^{-1}$
$10^{-2}$
$10^{-3}$
$10^{-4}$
$10^{-5}$
$10^{-1}$
$10^0$
chord distance $c_l = |2 \sin(\pi l / N_y)|$
0.0
0.1
0.2
0.3
0.4
0.5
$\alpha$
Monte Carlo, $\langle \sigma^z_i \sigma^z_j \rangle \geq 0$
Monte Carlo, $\langle \sigma^z_i \sigma^z_j \rangle < 0$
Discrete approximation, $\langle \sigma^z_i \sigma^z_j \rangle \geq 0$
Discrete approximation, $\langle \sigma^z_i \sigma^z_j \rangle < 0$
Continuum approximation, $\langle \sigma^z_i \sigma^z_j \rangle < 0$

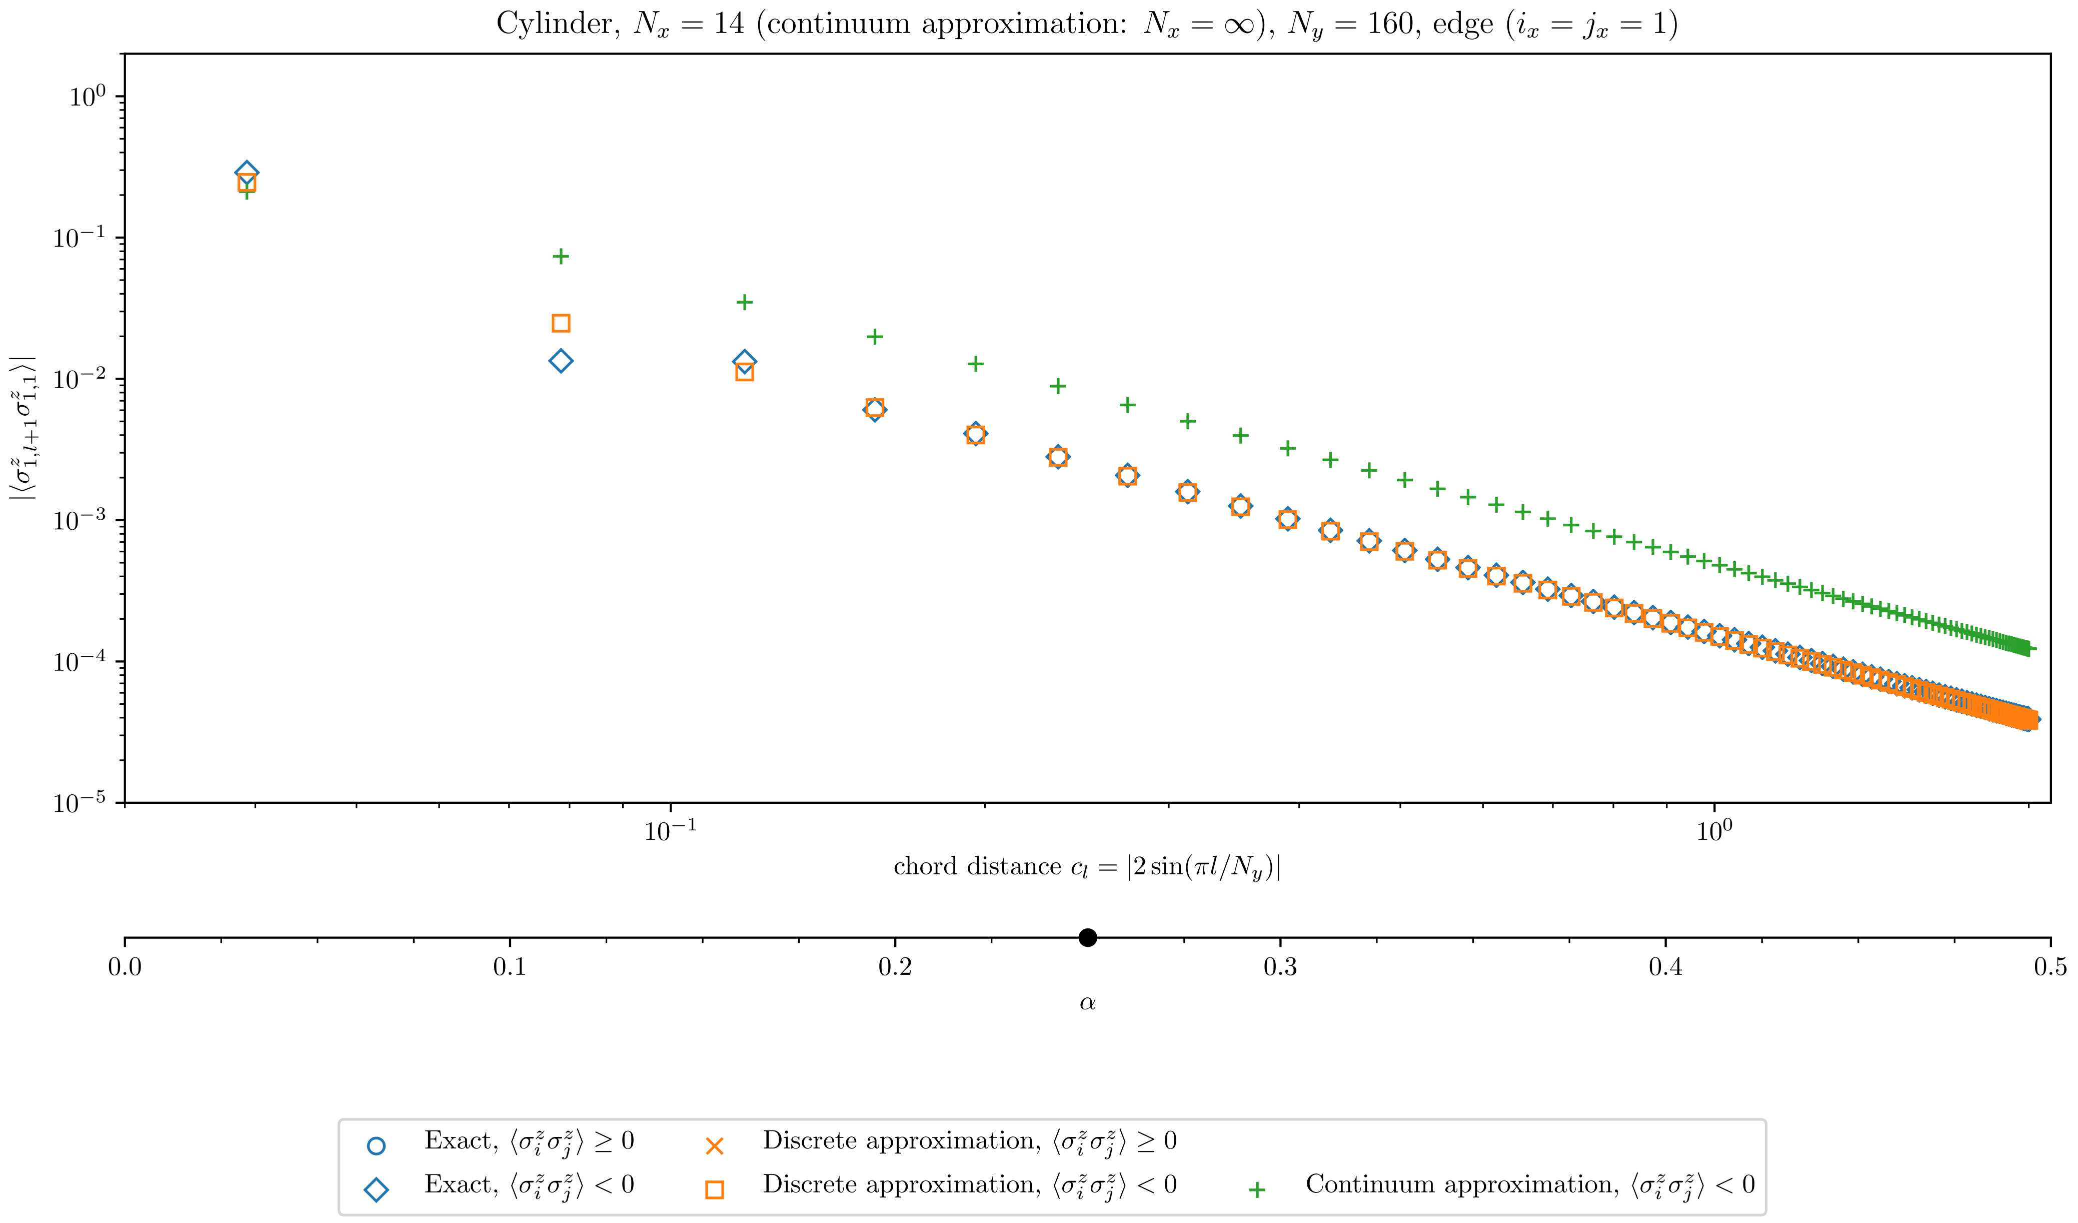

Cylinder, $N_x = 14$ (continuum approximation: $N_x = \infty$), $N_y = 160$, edge ($i_x = j_x = 1$)
$|\langle \sigma^z_{1,l+1} \sigma^z_{1,1} \rangle|$
$10^0$
$10^{-1}$
$10^{-2}$
$10^{-3}$
$10^{-4}$
$10^{-5}$
$10^{-1}$
$10^0$
chord distance $c_l = |2 \sin(\pi l / N_y)|$
0.0
0.1
0.2
0.3
0.4
0.5
$\alpha$
Exact, $\langle \sigma^z_i \sigma^z_j \rangle \geq 0$
Exact, $\langle \sigma^z_i \sigma^z_j \rangle < 0$
Discrete approximation, $\langle \sigma^z_i \sigma^z_j \rangle \geq 0$
Discrete approximation, $\langle \sigma^z_i \sigma^z_j \rangle < 0$
Continuum approximation, $\langle \sigma^z_i \sigma^z_j \rangle < 0$

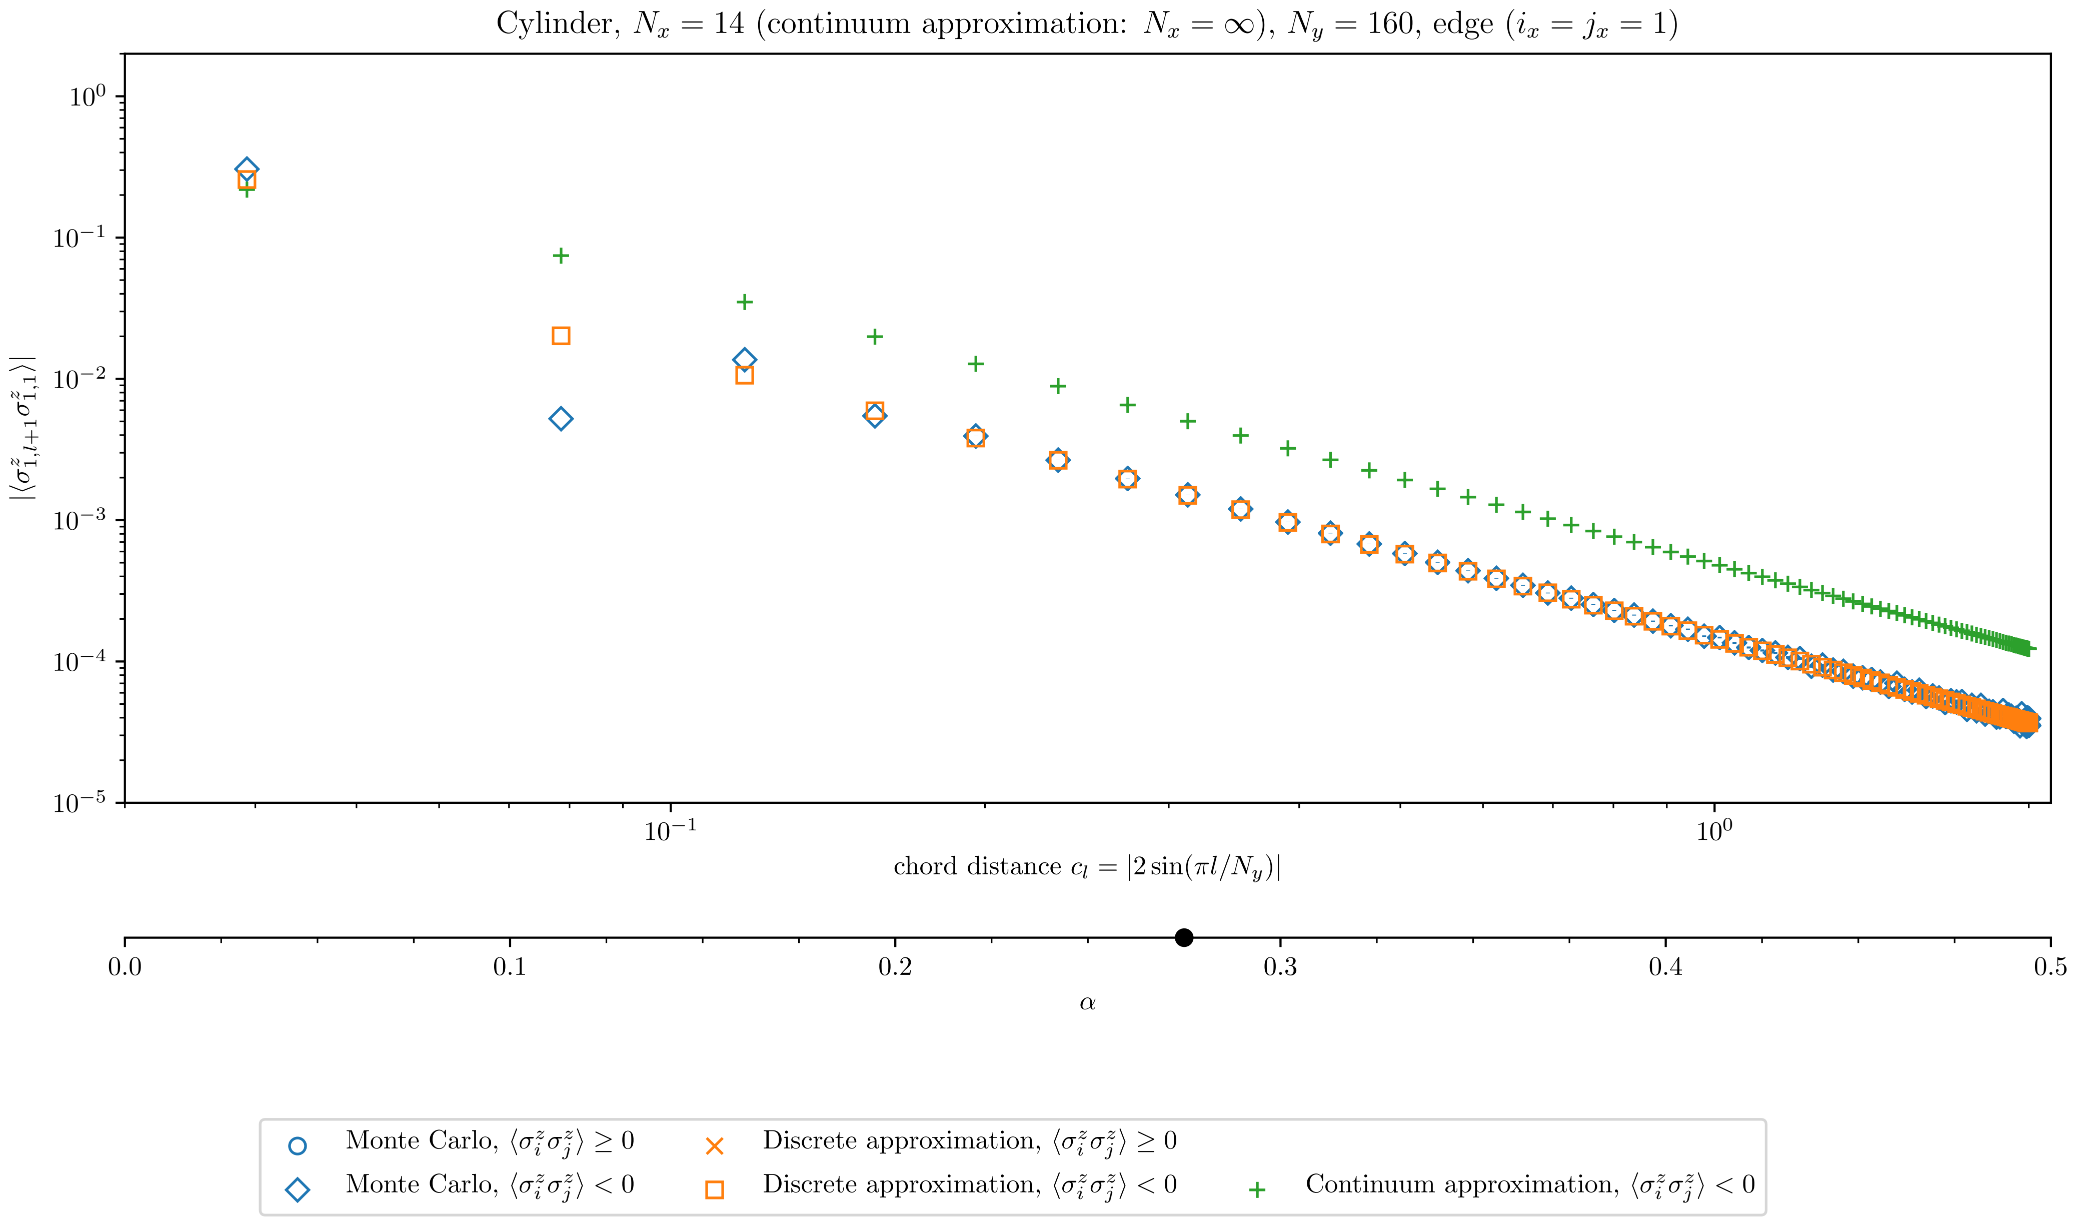

Cylinder, $N_x = 14$ (continuum approximation: $N_x = \infty$), $N_y = 160$, edge ($i_x = j_x = 1$)
$|\langle \sigma^z_{1,l+1} \sigma^z_{1,1} \rangle|$
$10^0$
$10^{-1}$
$10^{-2}$
$10^{-3}$
$10^{-4}$
$10^{-5}$
$10^{-1}$
$10^0$
chord distance $c_l = |2 \sin(\pi l / N_y)|$
0.0
0.1
0.2
0.3
0.4
0.5
$\alpha$
Monte Carlo, $\langle \sigma^z_i \sigma^z_j \rangle \geq 0$
Monte Carlo, $\langle \sigma^z_i \sigma^z_j \rangle < 0$
Discrete approximation, $\langle \sigma^z_i \sigma^z_j \rangle \geq 0$
Discrete approximation, $\langle \sigma^z_i \sigma^z_j \rangle < 0$
Continuum approximation, $\langle \sigma^z_i \sigma^z_j \rangle < 0$

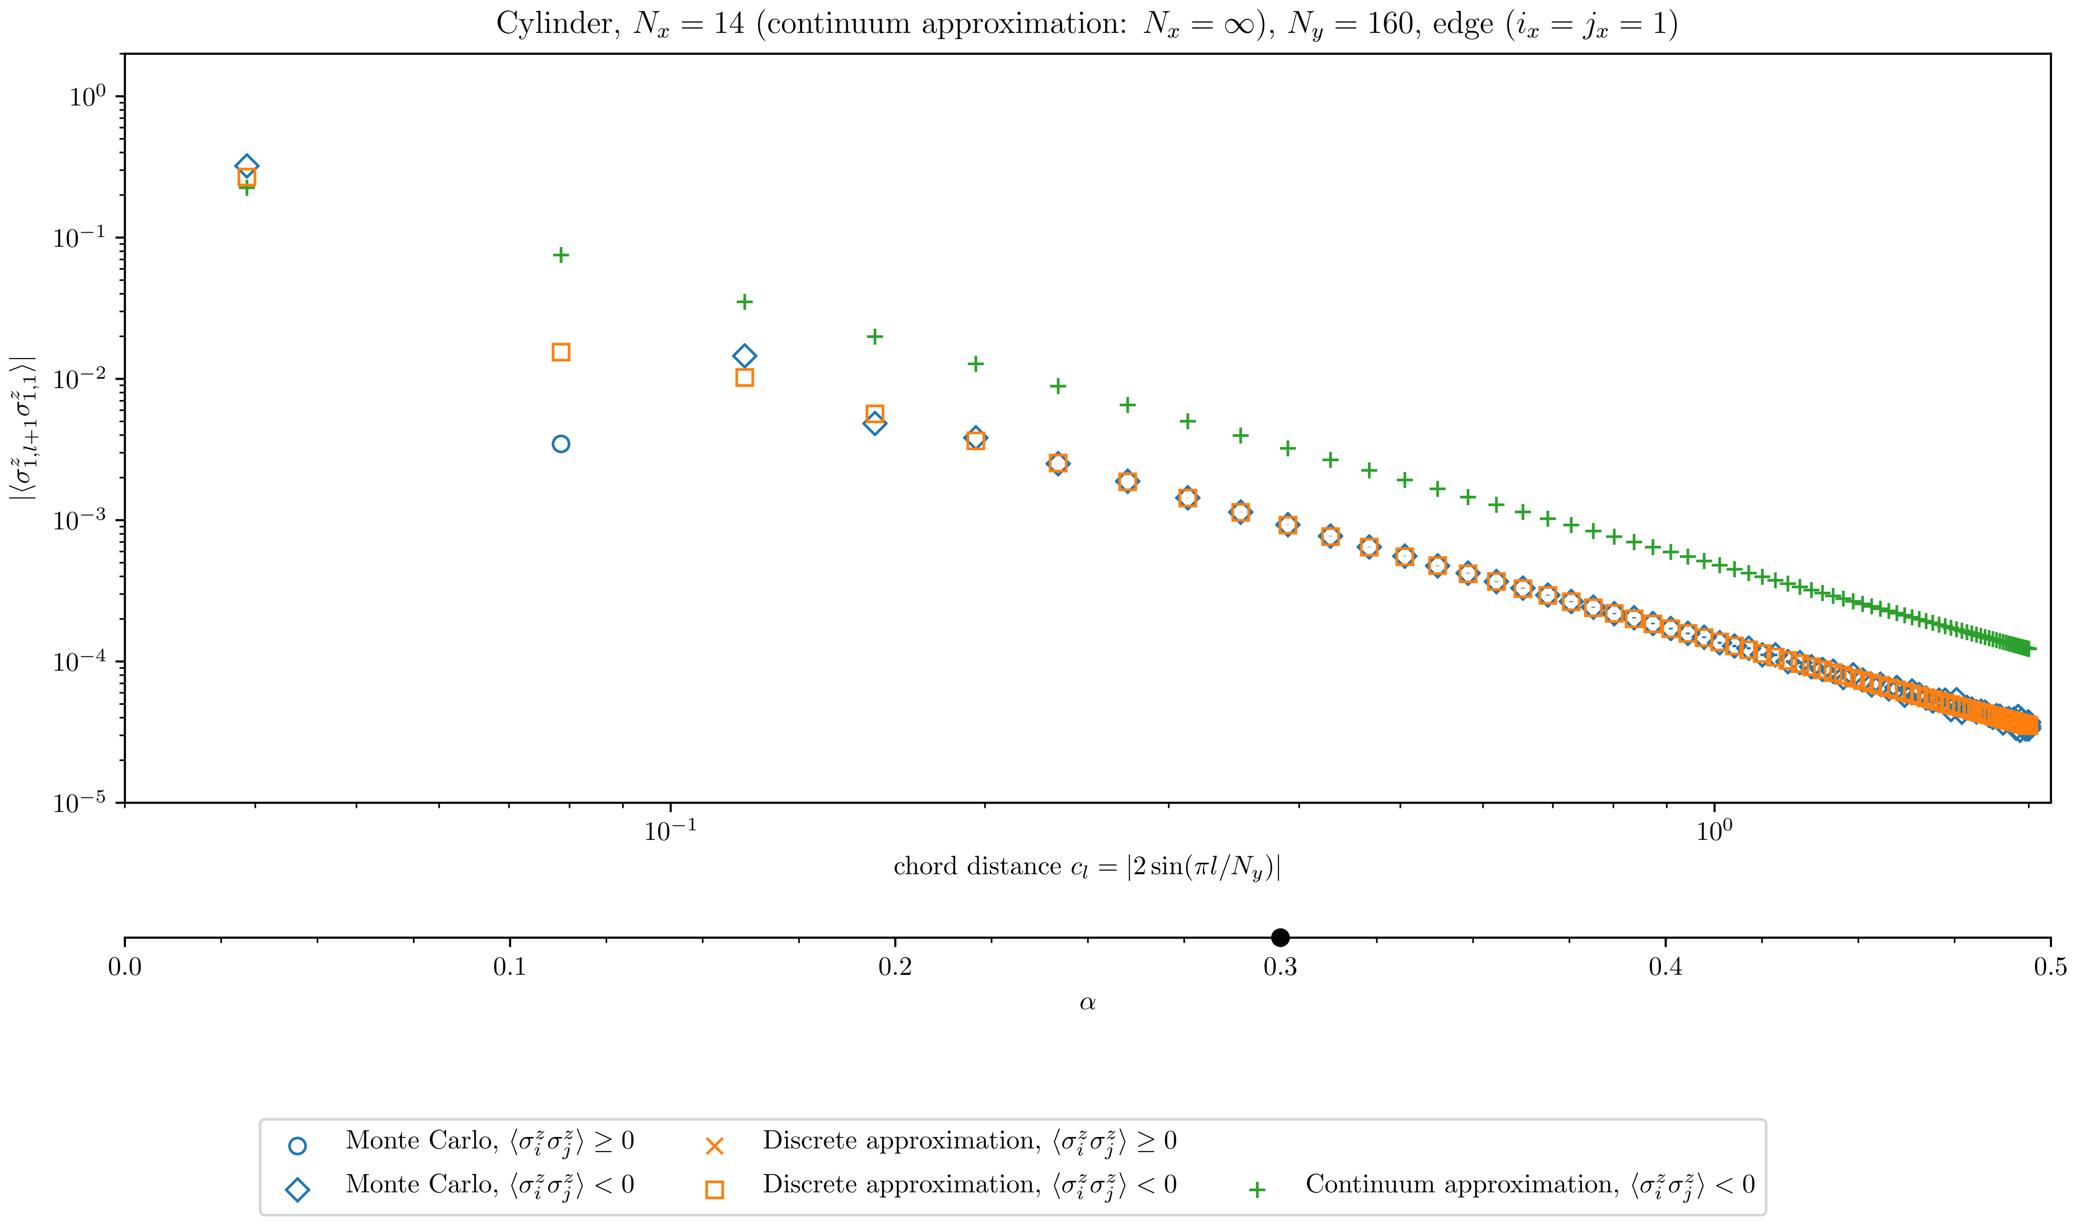

Cylinder, $N_x = 14$ (continuum approximation: $N_x = \infty$), $N_y = 160$, edge ($i_x = j_x = 1$)
$|\langle \sigma^z_{1,l+1} \sigma^z_{1,1} \rangle|$
$10^0$
$10^{-1}$
$10^{-2}$
$10^{-3}$
$10^{-4}$
$10^{-5}$
$10^{-1}$
$10^0$
chord distance $c_l = |2 \sin(\pi l / N_y)|$
0.0
0.1
0.2
0.3
0.4
0.5
$\alpha$
Monte Carlo, $\langle \sigma^z_i \sigma^z_j \rangle \geq 0$
Monte Carlo, $\langle \sigma^z_i \sigma^z_j \rangle < 0$
Discrete approximation, $\langle \sigma^z_i \sigma^z_j \rangle \geq 0$
Discrete approximation, $\langle \sigma^z_i \sigma^z_j \rangle < 0$
Continuum approximation, $\langle \sigma^z_i \sigma^z_j \rangle < 0$

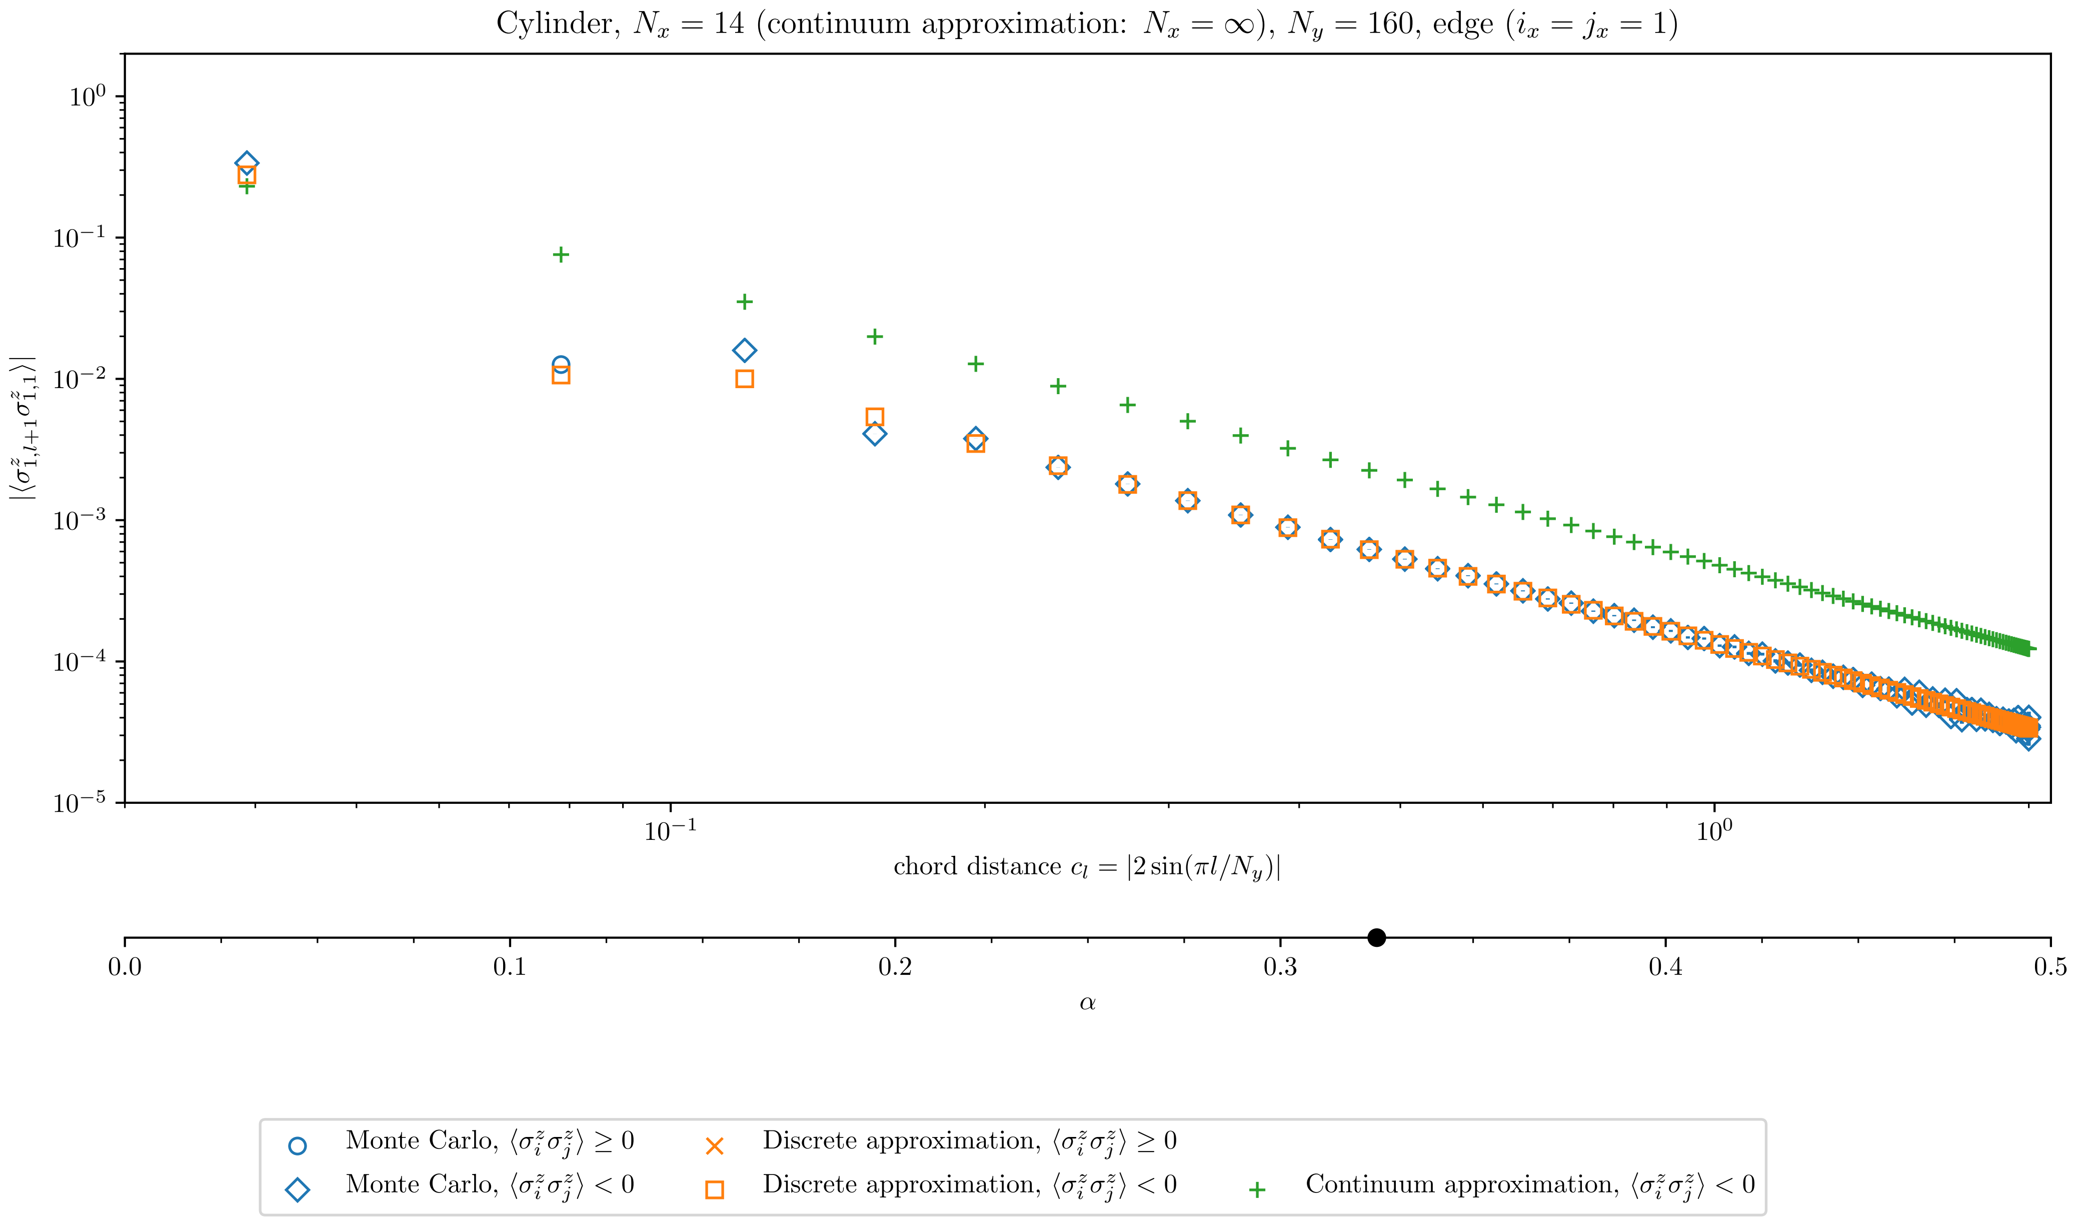
Cylinder, $N_x = 14$ (continuum approximation: $N_x = \infty$), $N_y = 160$, edge ($i_x = j_x = 1$)
$|\langle \sigma^z_{1,l+1} \sigma^z_{1,1} \rangle|$
$10^0$
$10^{-1}$
$10^{-2}$
$10^{-3}$
$10^{-4}$
$10^{-5}$
$10^{-1}$
$10^0$
chord distance $c_l = |2 \sin(\pi l / N_y)|$
0.0
0.1
0.2
0.3
0.4
0.5
$\alpha$
Monte Carlo, $\langle \sigma^z_i \sigma^z_j \rangle \geq 0$
Monte Carlo, $\langle \sigma^z_i \sigma^z_j \rangle < 0$
Discrete approximation, $\langle \sigma^z_i \sigma^z_j \rangle \geq 0$
Discrete approximation, $\langle \sigma^z_i \sigma^z_j \rangle < 0$
Continuum approximation, $\langle \sigma^z_i \sigma^z_j \rangle < 0$

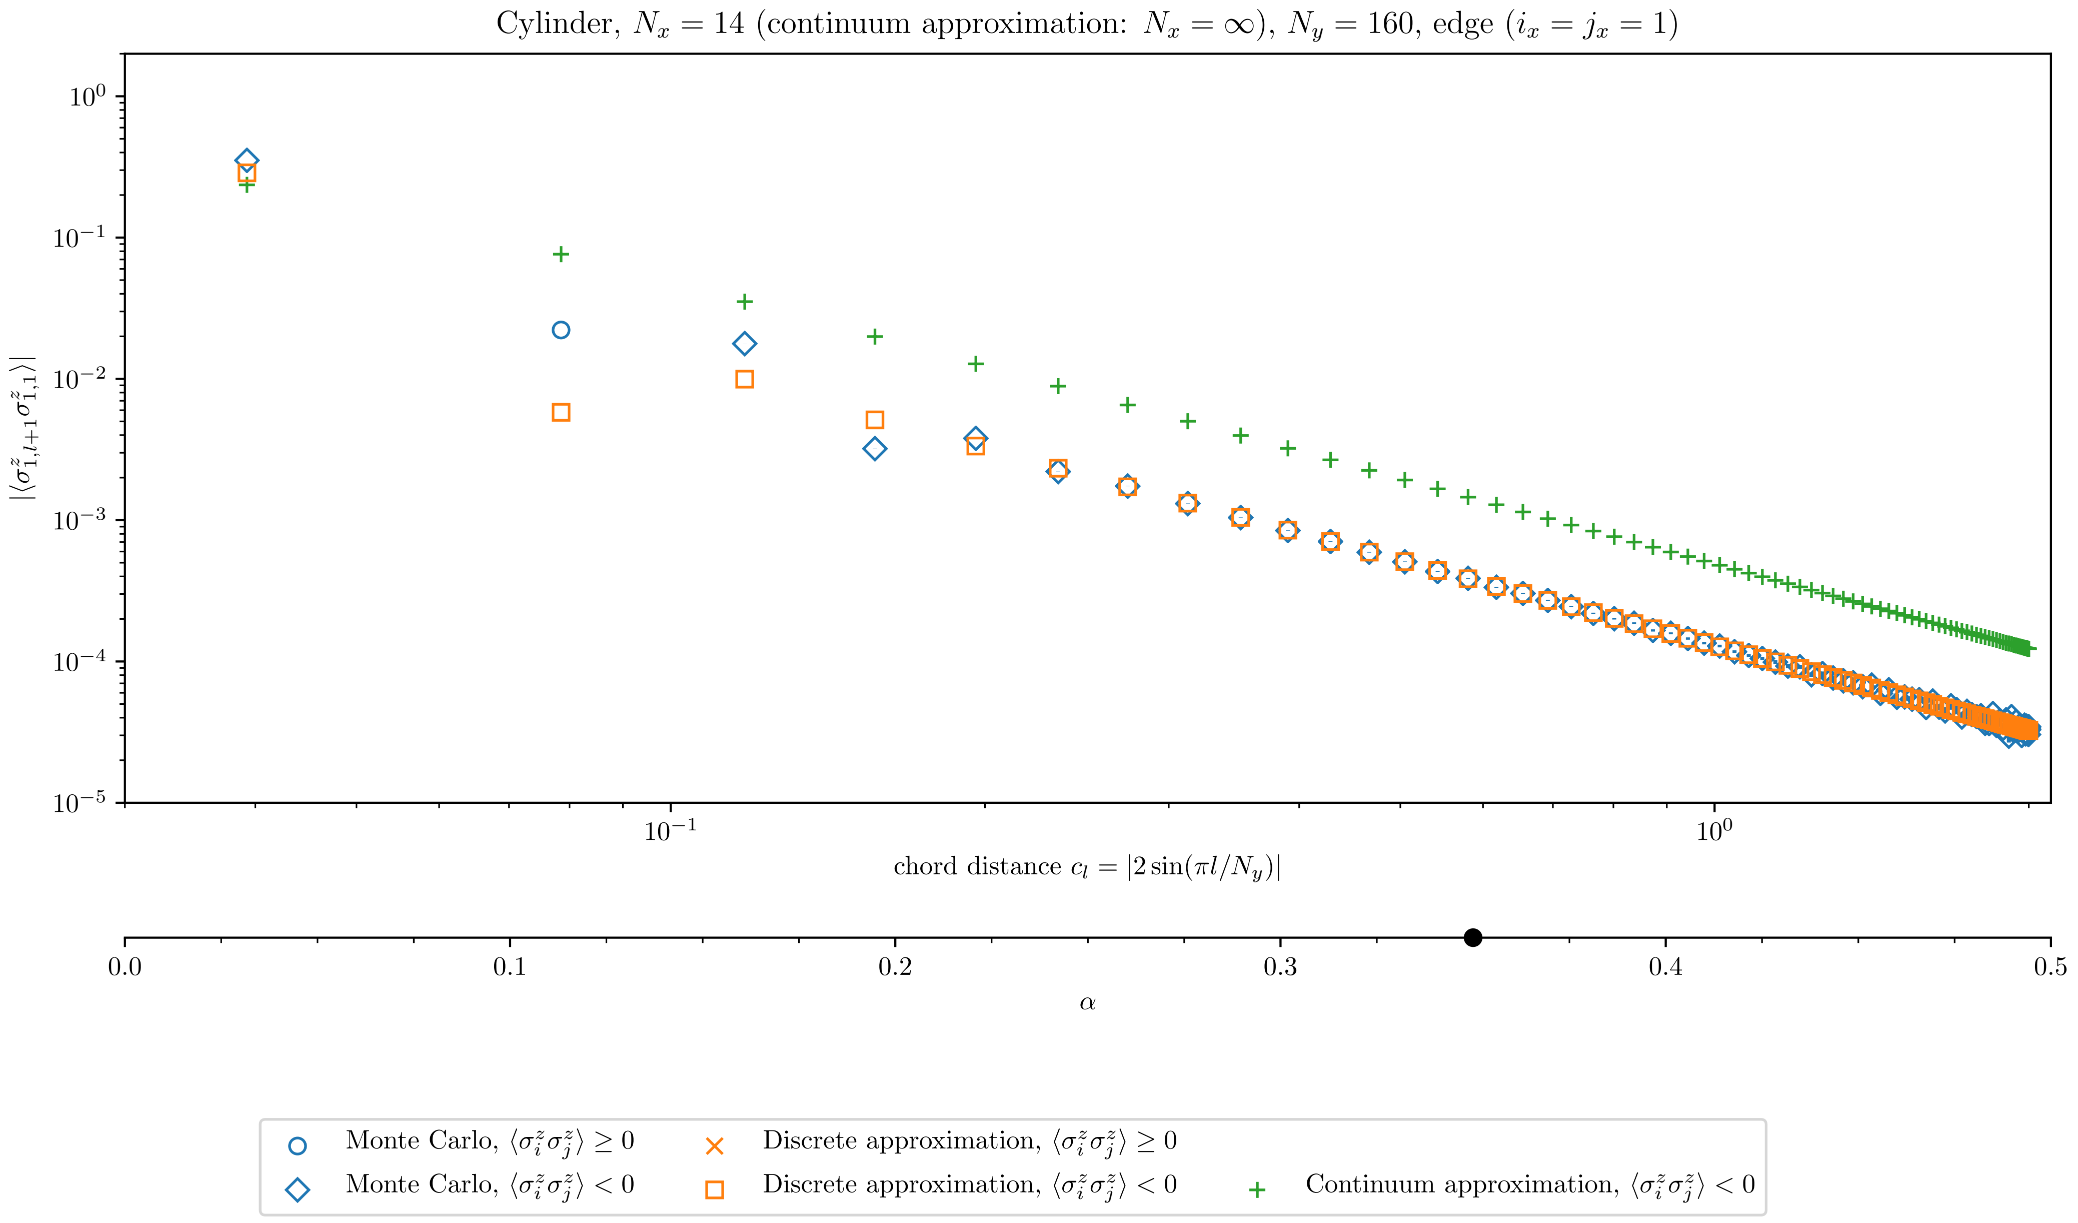

Cylinder, $N_x = 14$ (continuum approximation: $N_x = \infty$), $N_y = 160$, edge ($i_x = j_x = 1$)
$|\langle \sigma^z_{1,l+1} \sigma^z_{1,1} \rangle|$
$10^0$
$10^{-1}$
$10^{-2}$
$10^{-3}$
$10^{-4}$
$10^{-5}$
$10^{-1}$
$10^0$
chord distance $c_l = |2 \sin(\pi l / N_y)|$
0.0
0.1
0.2
0.3
0.4
0.5
$\alpha$
Monte Carlo, $\langle \sigma^z_i \sigma^z_j \rangle \geq 0$
Monte Carlo, $\langle \sigma^z_i \sigma^z_j \rangle < 0$
Discrete approximation, $\langle \sigma^z_i \sigma^z_j \rangle \geq 0$
Discrete approximation, $\langle \sigma^z_i \sigma^z_j \rangle < 0$
Continuum approximation, $\langle \sigma^z_i \sigma^z_j \rangle < 0$

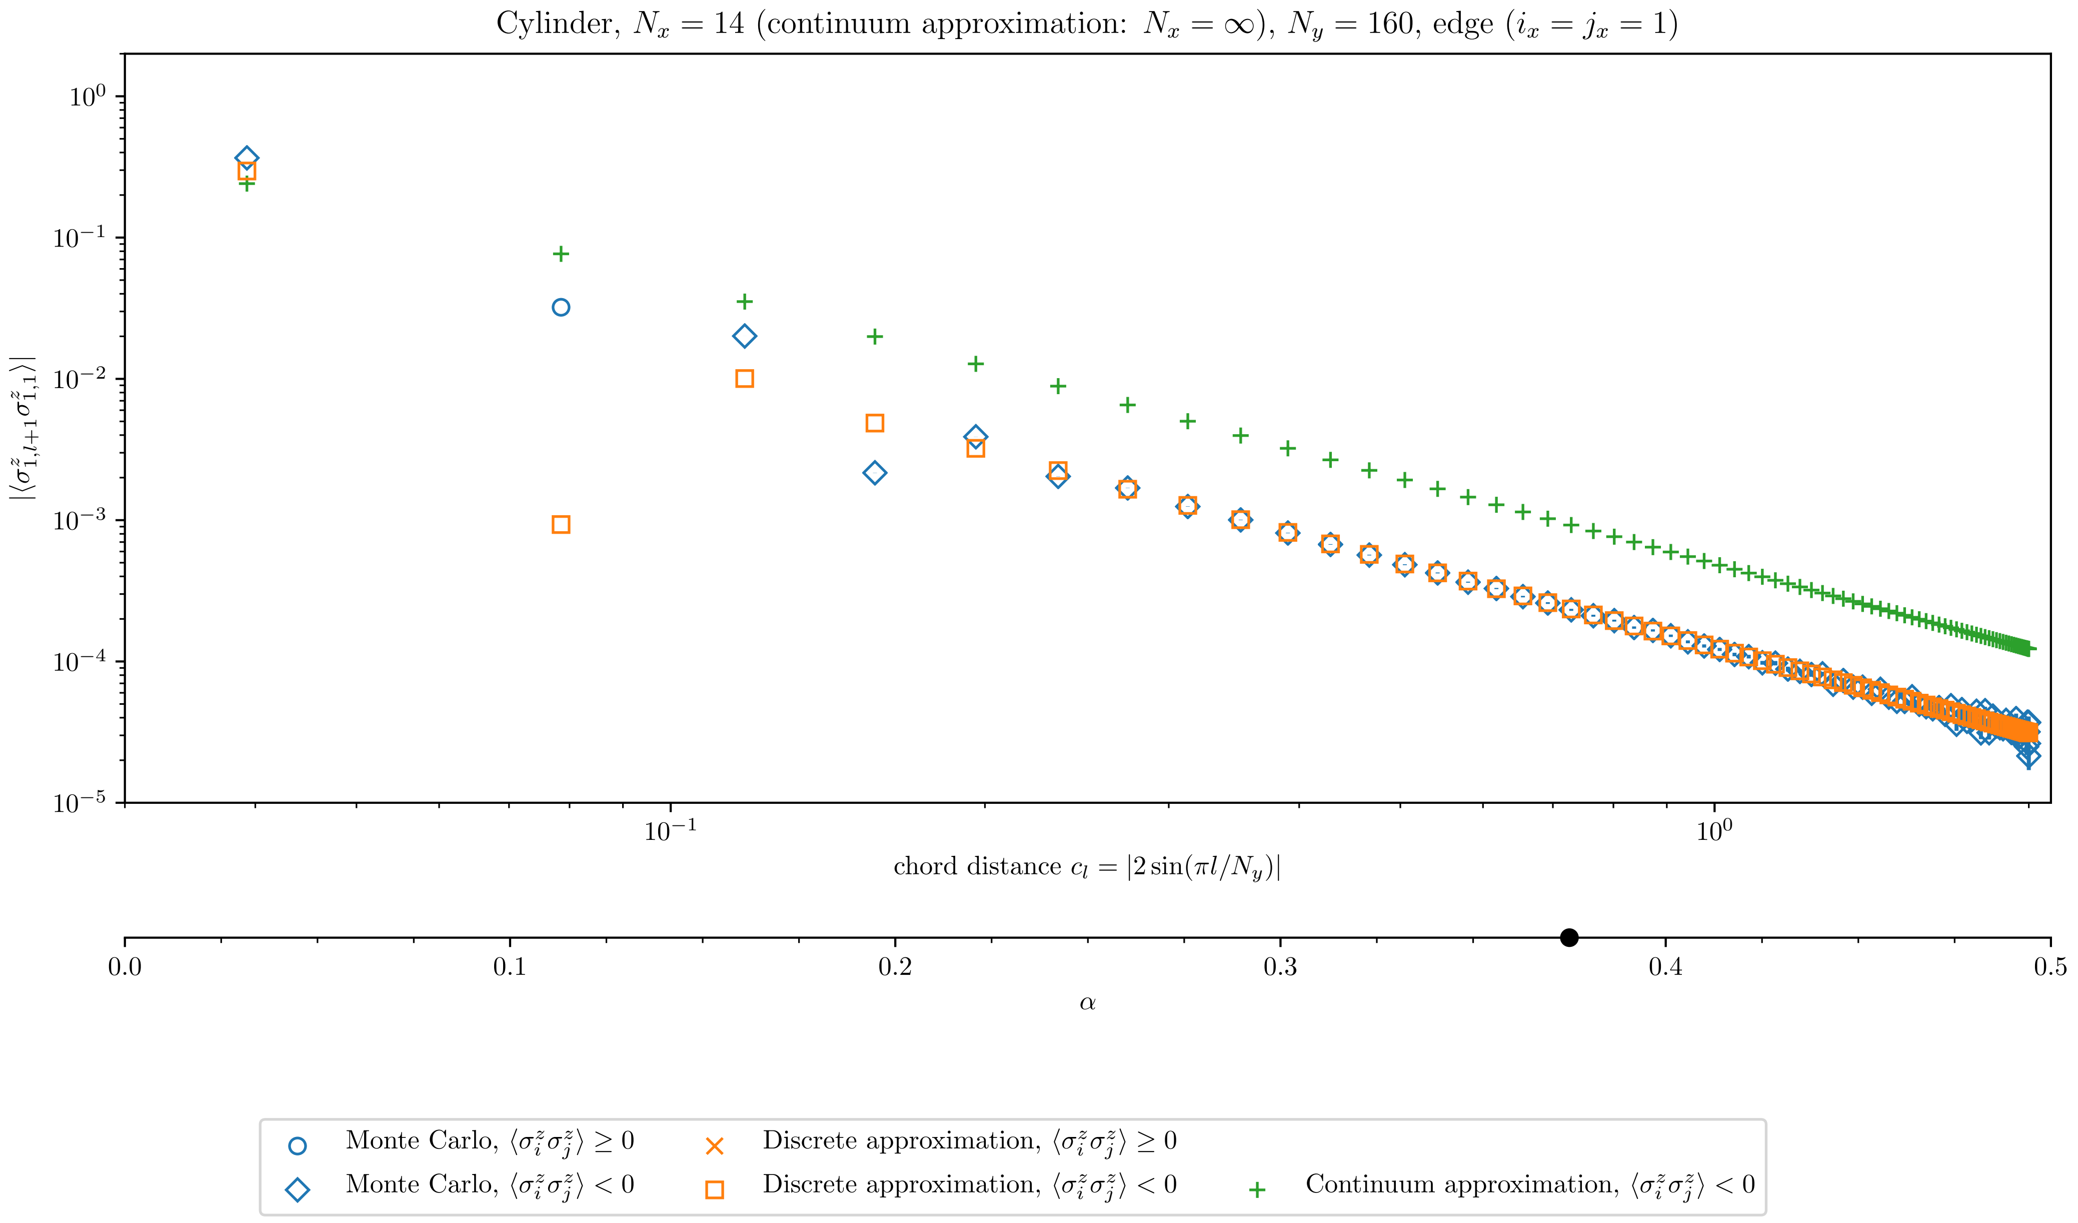

Cylinder, $N_x = 14$ (continuum approximation: $N_x = \infty$), $N_y = 160$, edge ($i_x = j_x = 1$)
$|\langle \sigma^z_{1,l+1} \sigma^z_{1,1} \rangle|$
$10^0$
$10^{-1}$
$10^{-2}$
$10^{-3}$
$10^{-4}$
$10^{-5}$
chord distance $c_l = |2\sin(\pi l/N_y)|$
$\alpha$
0.0
0.1
0.2
0.3
0.4
0.5
Monte Carlo, $\langle \sigma^z_i \sigma^z_j \rangle \geq 0$
Monte Carlo, $\langle \sigma^z_i \sigma^z_j \rangle < 0$
Discrete approximation, $\langle \sigma^z_i \sigma^z_j \rangle \geq 0$
Discrete approximation, $\langle \sigma^z_i \sigma^z_j \rangle < 0$
Continuum approximation, $\langle \sigma^z_i \sigma^z_j \rangle < 0$

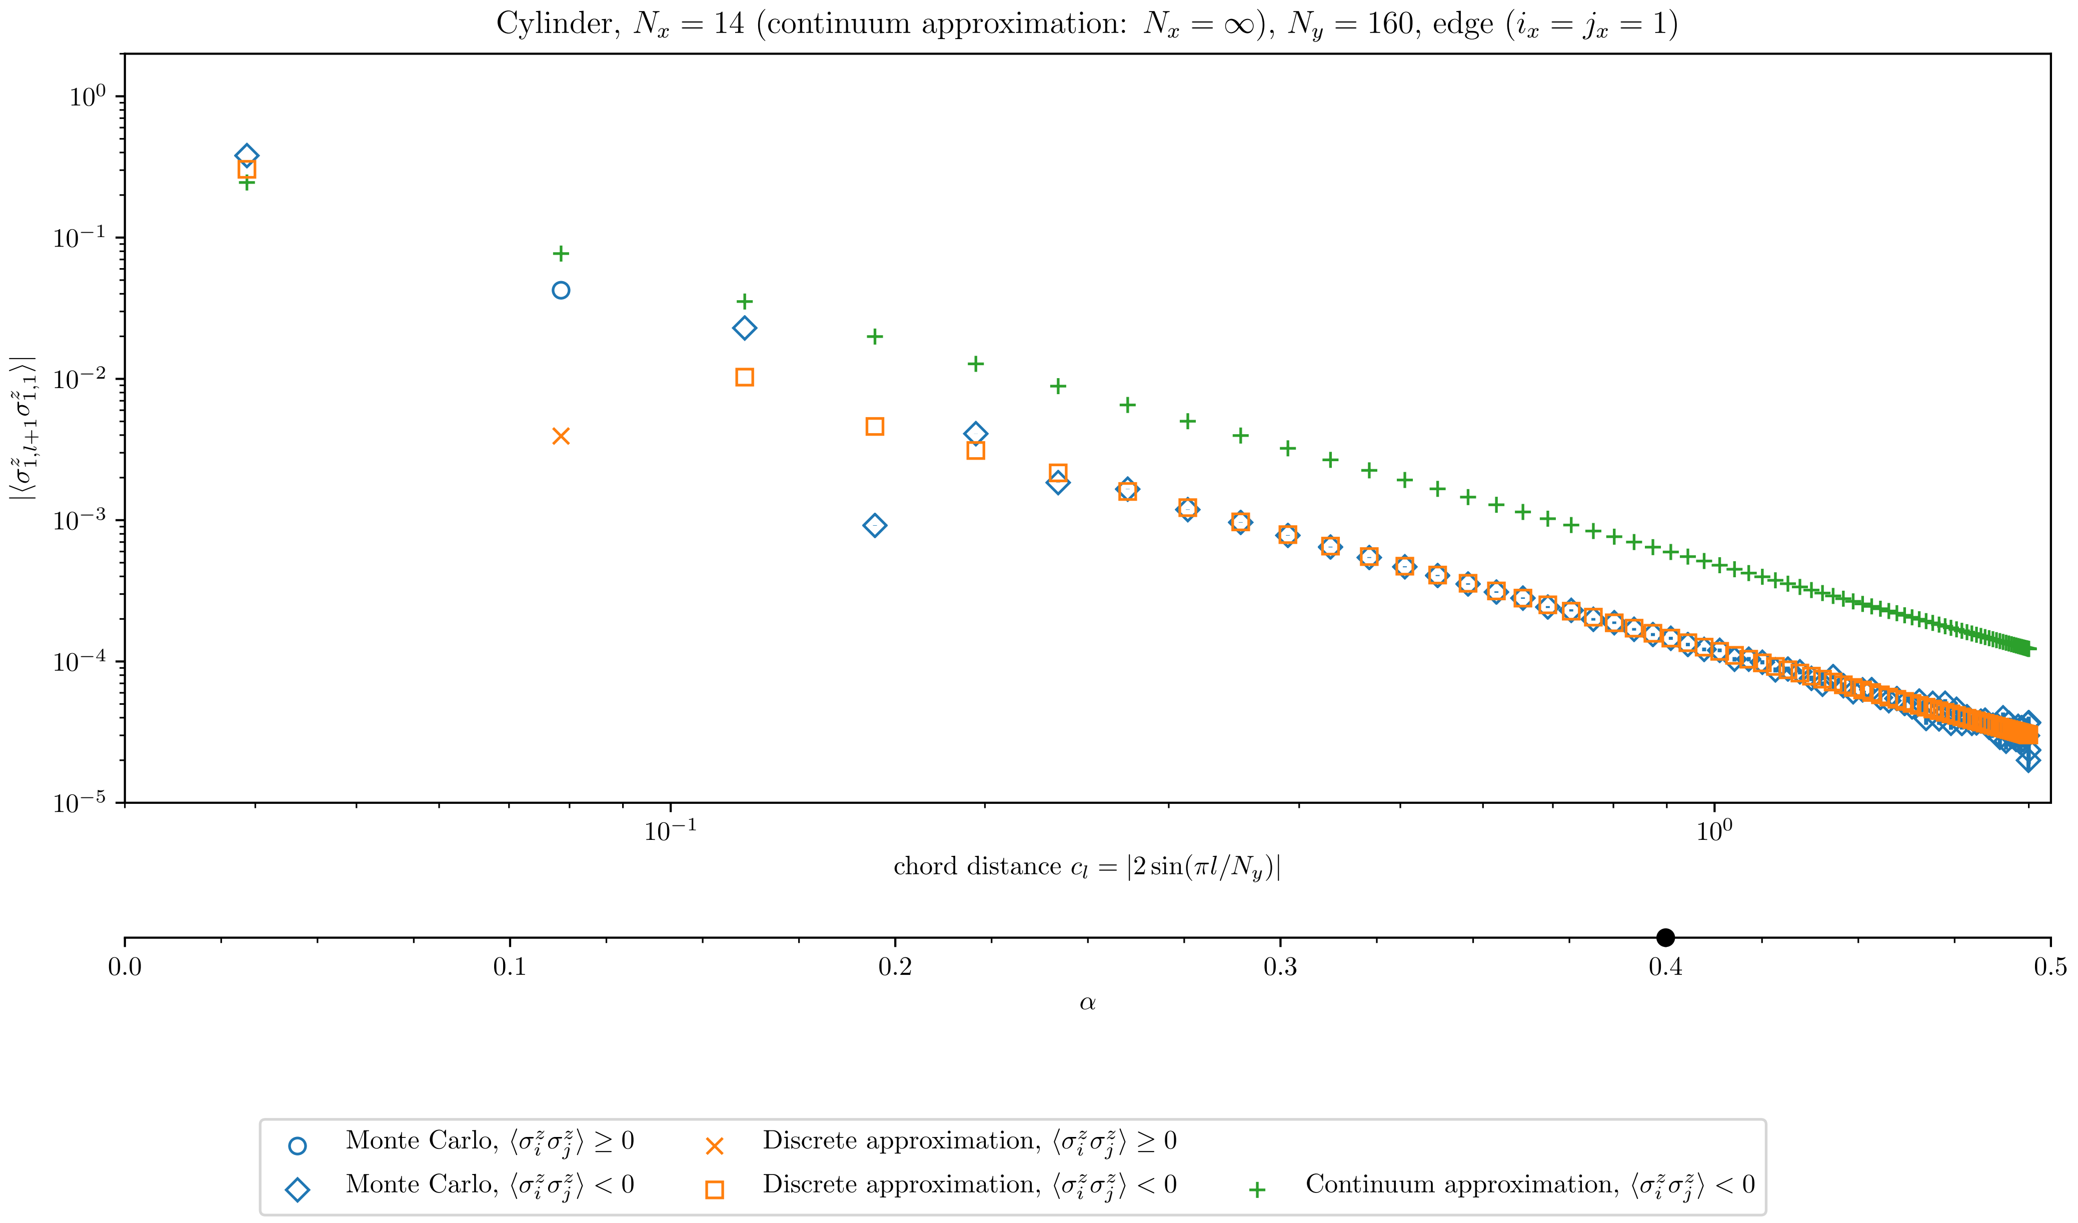

Cylinder, $N_x = 14$ (continuum approximation: $N_x = \infty$), $N_y = 160$, edge ($i_x = j_x = 1$)
$|\langle \sigma^z_{1,l+1} \sigma^z_{1,1} \rangle|$
$10^0$
$10^{-1}$
$10^{-2}$
$10^{-3}$
$10^{-4}$
$10^{-5}$
$10^{-1}$
$10^0$
chord distance $c_l = |2\sin(\pi l/N_y)|$
0.0
0.1
0.2
0.3
0.4
0.5
$\alpha$
Monte Carlo, $\langle \sigma^z_i \sigma^z_j \rangle \geq 0$
Monte Carlo, $\langle \sigma^z_i \sigma^z_j \rangle < 0$
Discrete approximation, $\langle \sigma^z_i \sigma^z_j \rangle \geq 0$
Discrete approximation, $\langle \sigma^z_i \sigma^z_j \rangle < 0$
Continuum approximation, $\langle \sigma^z_i \sigma^z_j \rangle < 0$

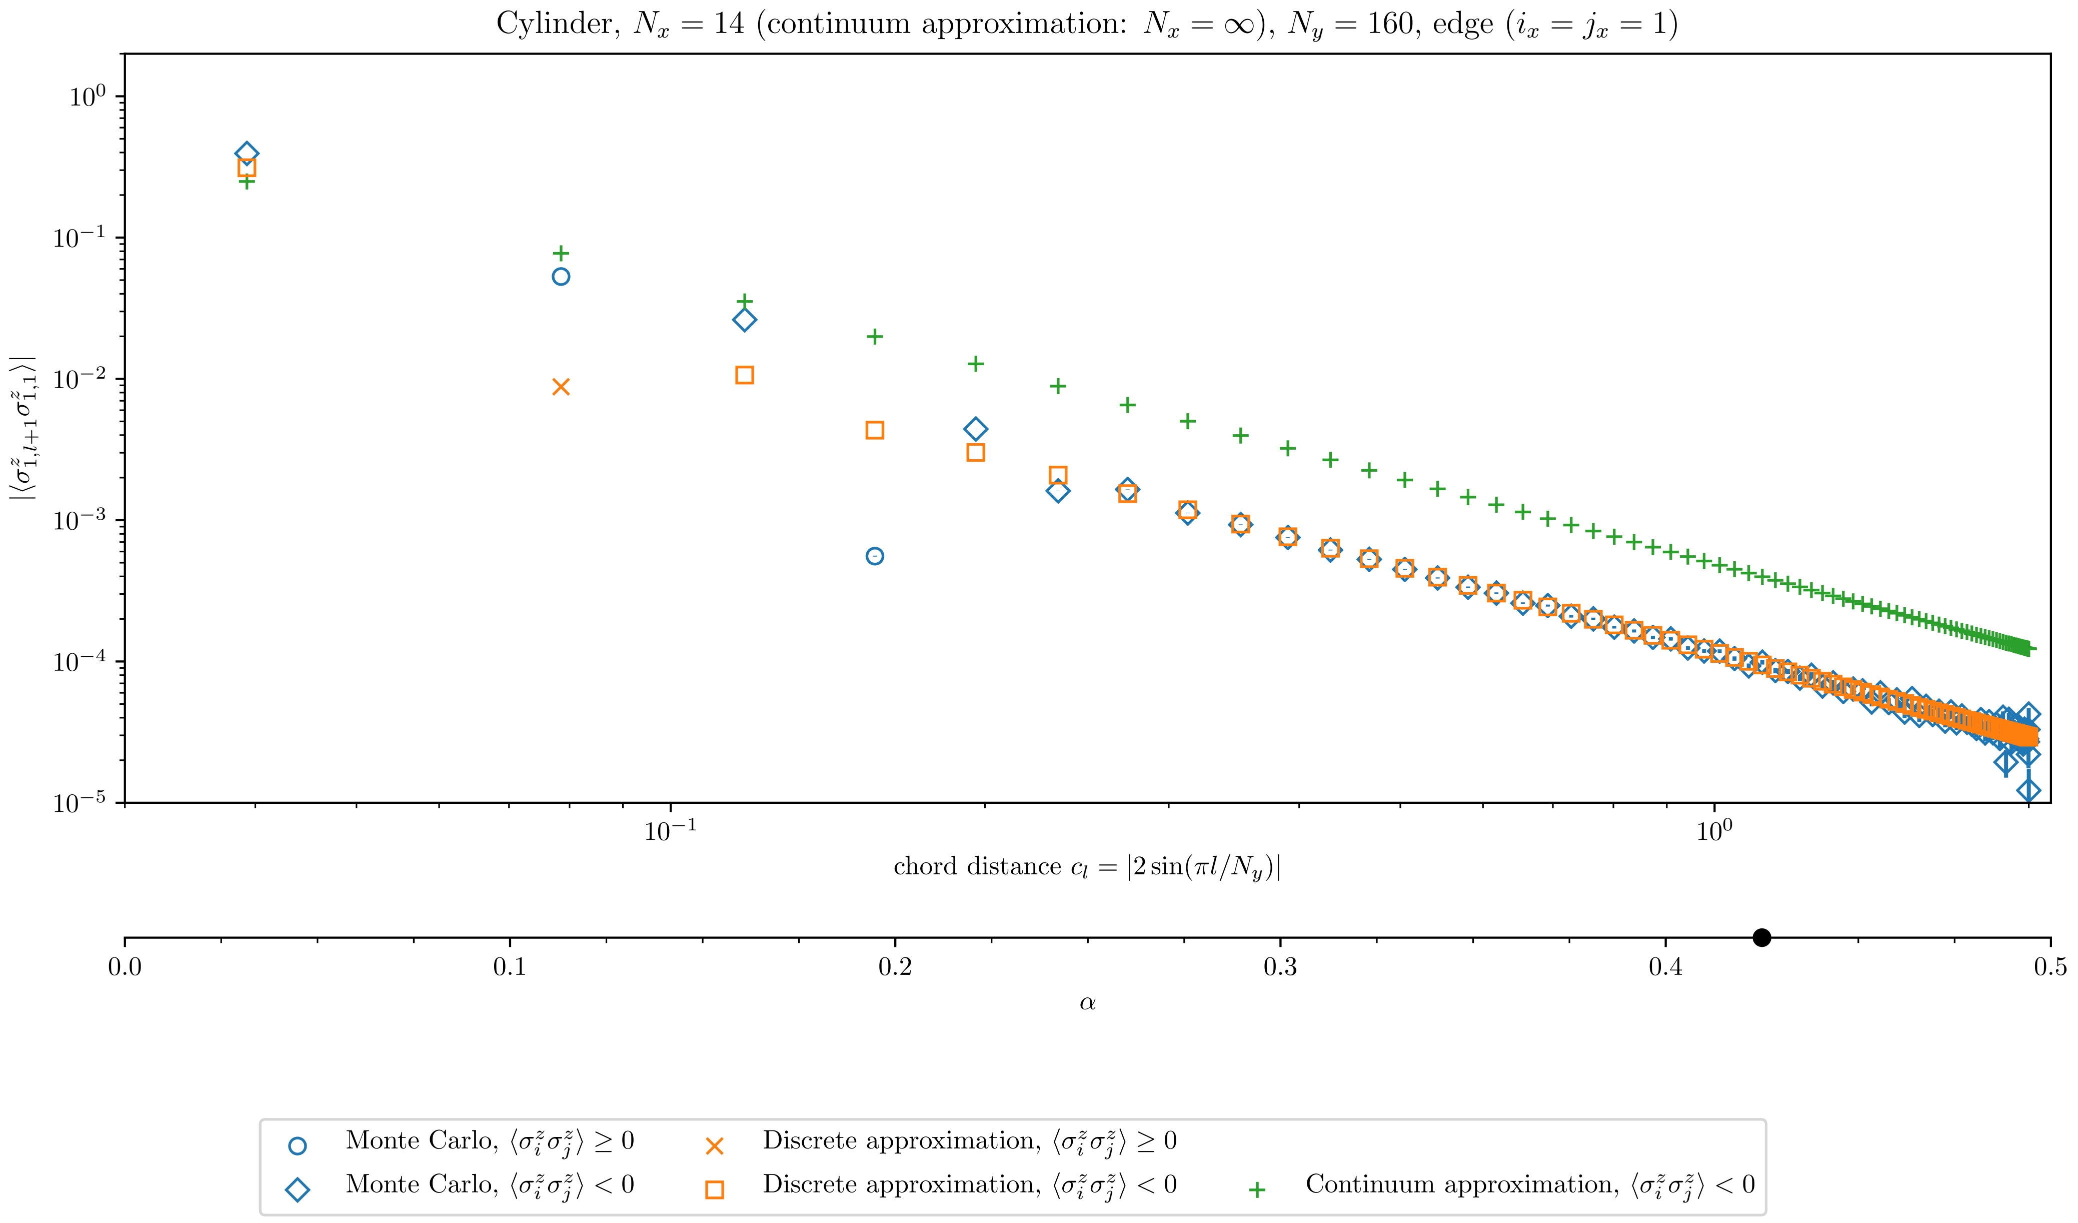
Cylinder, $N_x = 14$ (continuum approximation: $N_x = \infty$), $N_y = 160$, edge ($i_x = j_x = 1$)
$|\langle \sigma^z_{1,l+1} \sigma^z_{1,1} \rangle|$
chord distance $c_l = |2\sin(\pi l/N_y)|$
$\alpha$
Monte Carlo, $\langle \sigma^z_i \sigma^z_j \rangle \geq 0$
Monte Carlo, $\langle \sigma^z_i \sigma^z_j \rangle < 0$
Discrete approximation, $\langle \sigma^z_i \sigma^z_j \rangle \geq 0$
Discrete approximation, $\langle \sigma^z_i \sigma^z_j \rangle < 0$
Continuum approximation, $\langle \sigma^z_i \sigma^z_j \rangle < 0$

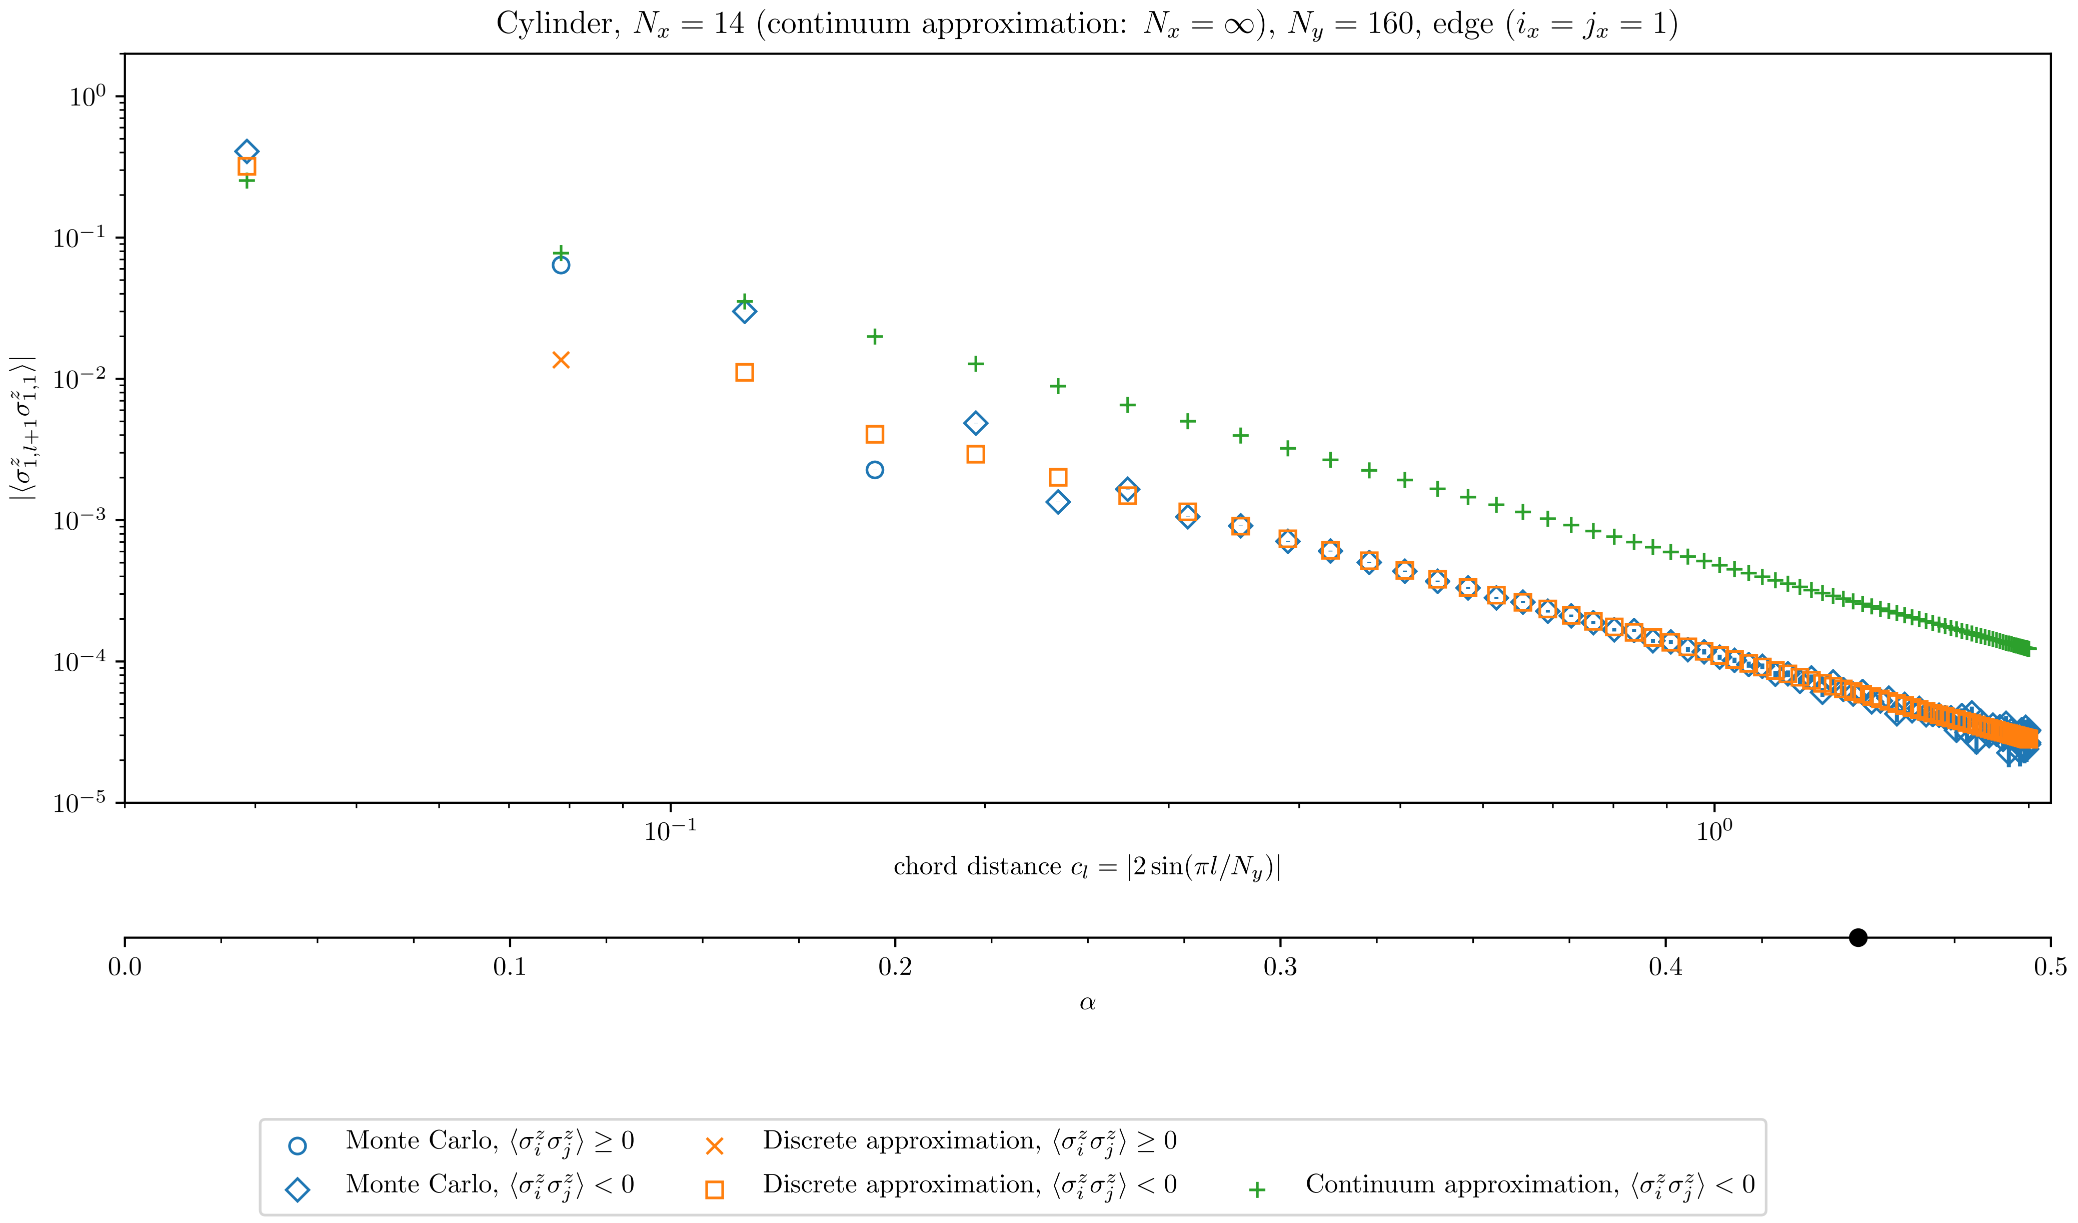

Cylinder, $N_x = 14$ (continuum approximation: $N_x = \infty$), $N_y = 160$, edge ($i_x = j_x = 1$)
$|\langle\sigma^z_{1,l+1}\sigma^z_{1,1}\rangle|$
$10^0$
$10^{-1}$
$10^{-2}$
$10^{-3}$
$10^{-4}$
$10^{-5}$
$10^{-1}$
$10^0$
chord distance $c_l = |2\sin(\pi l/N_y)|$
0.0
0.1
0.2
0.3
0.4
0.5
$\alpha$
Monte Carlo, $\langle\sigma^z_i\sigma^z_j\rangle \geq 0$
Monte Carlo, $\langle\sigma^z_i\sigma^z_j\rangle < 0$
Discrete approximation, $\langle\sigma^z_i\sigma^z_j\rangle \geq 0$
Discrete approximation, $\langle\sigma^z_i\sigma^z_j\rangle < 0$
Continuum approximation, $\langle\sigma^z_i\sigma^z_j\rangle < 0$

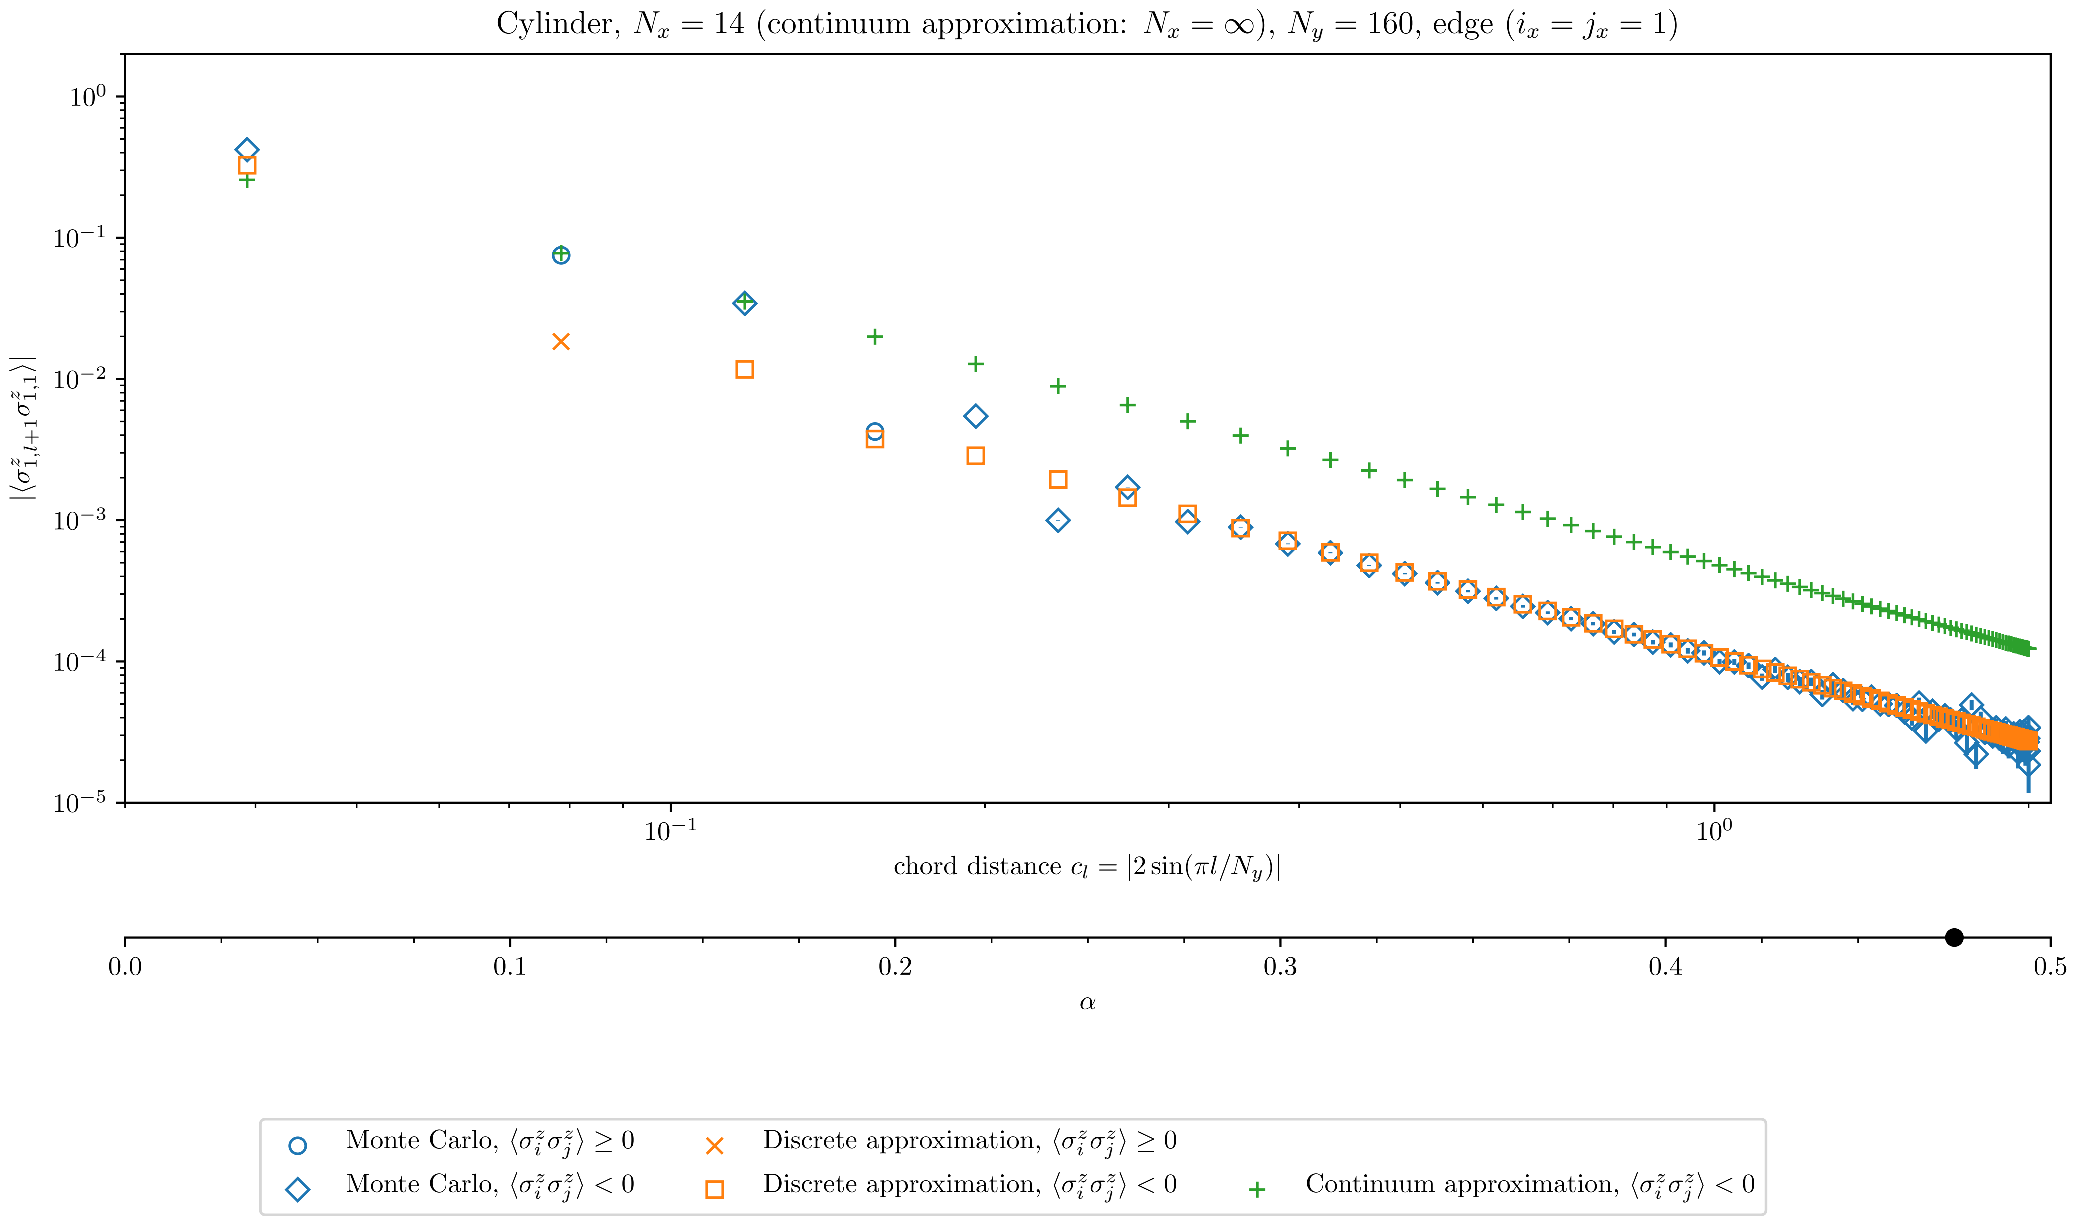

Cylinder, $N_x = 14$ (continuum approximation: $N_x = \infty$), $N_y = 160$, edge ($i_x = j_x = 1$)
$|\langle \sigma^z_{1,l+1} \sigma^z_{1,1} \rangle|$
$10^0$
$10^{-1}$
$10^{-2}$
$10^{-3}$
$10^{-4}$
$10^{-5}$
$10^{-1}$
$10^0$
chord distance $c_l = |2 \sin(\pi l / N_y)|$
0.0
0.1
0.2
0.3
0.4
0.5
$\alpha$
Monte Carlo, $\langle \sigma^z_i \sigma^z_j \rangle \geq 0$
Monte Carlo, $\langle \sigma^z_i \sigma^z_j \rangle < 0$
Discrete approximation, $\langle \sigma^z_i \sigma^z_j \rangle \geq 0$
Discrete approximation, $\langle \sigma^z_i \sigma^z_j \rangle < 0$
Continuum approximation, $\langle \sigma^z_i \sigma^z_j \rangle < 0$

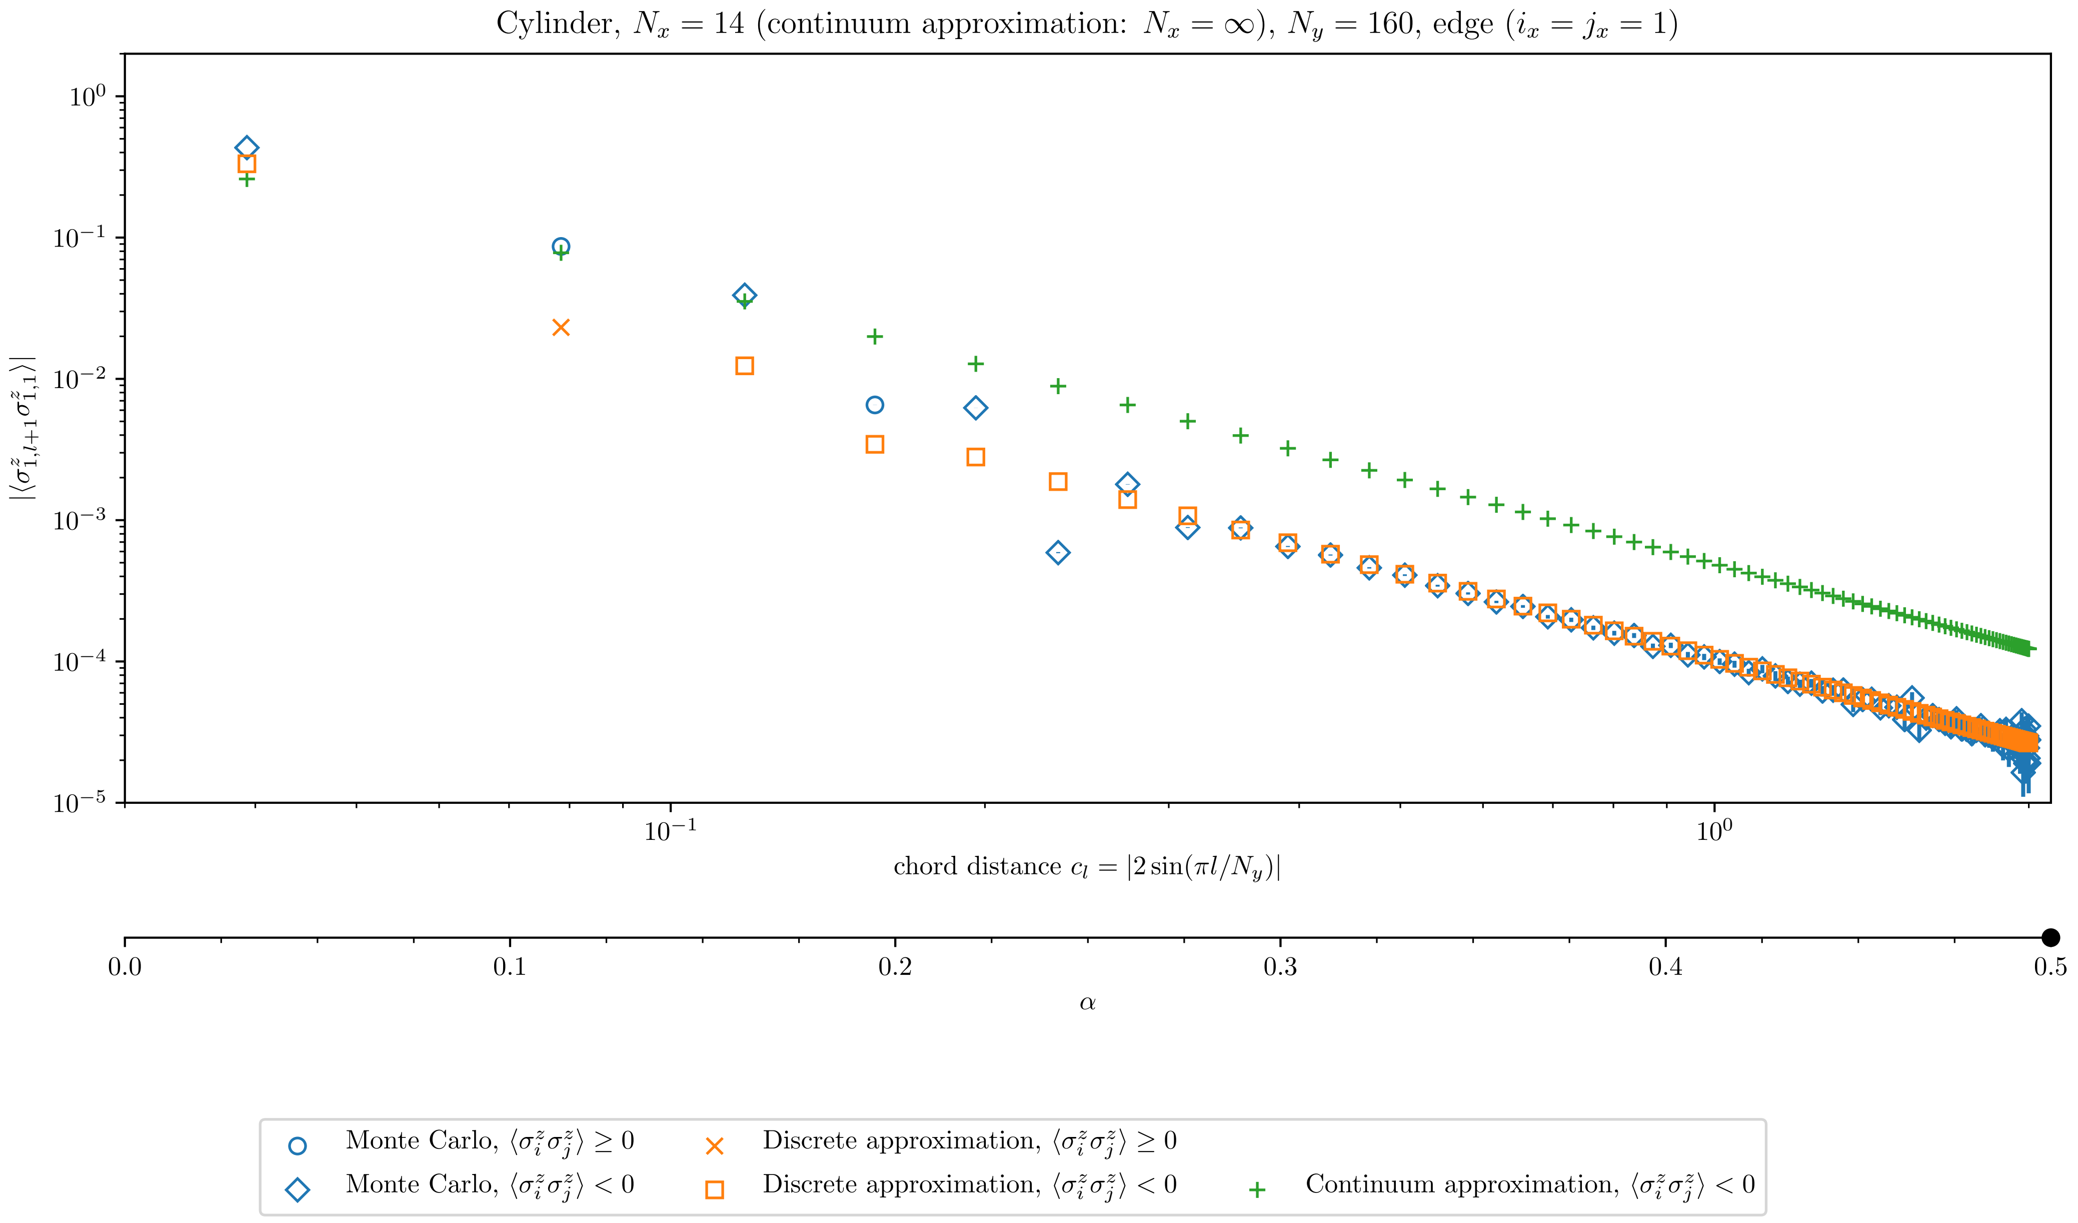

Cylinder, $N_x = 14$ (continuum approximation: $N_x = \infty$), $N_y = 160$, edge ($i_x = j_x = 1$)
$|\langle \sigma^z_{1,l+1} \sigma^z_{1,1} \rangle|$
$10^0$
$10^{-1}$
$10^{-2}$
$10^{-3}$
$10^{-4}$
$10^{-5}$
$10^{-1}$
$10^0$
chord distance $c_l = |2 \sin(\pi l / N_y)|$
0.0
0.1
0.2
0.3
0.4
0.5
$\alpha$
Monte Carlo, $\langle \sigma^z_i \sigma^z_j \rangle \geq 0$
Monte Carlo, $\langle \sigma^z_i \sigma^z_j \rangle < 0$
Discrete approximation, $\langle \sigma^z_i \sigma^z_j \rangle \geq 0$
Discrete approximation, $\langle \sigma^z_i \sigma^z_j \rangle < 0$
Continuum approximation, $\langle \sigma^z_i \sigma^z_j \rangle < 0$

I. Circle

II. Sphere

III. Cylinder (edge)

IV. Cylinder (bulk)

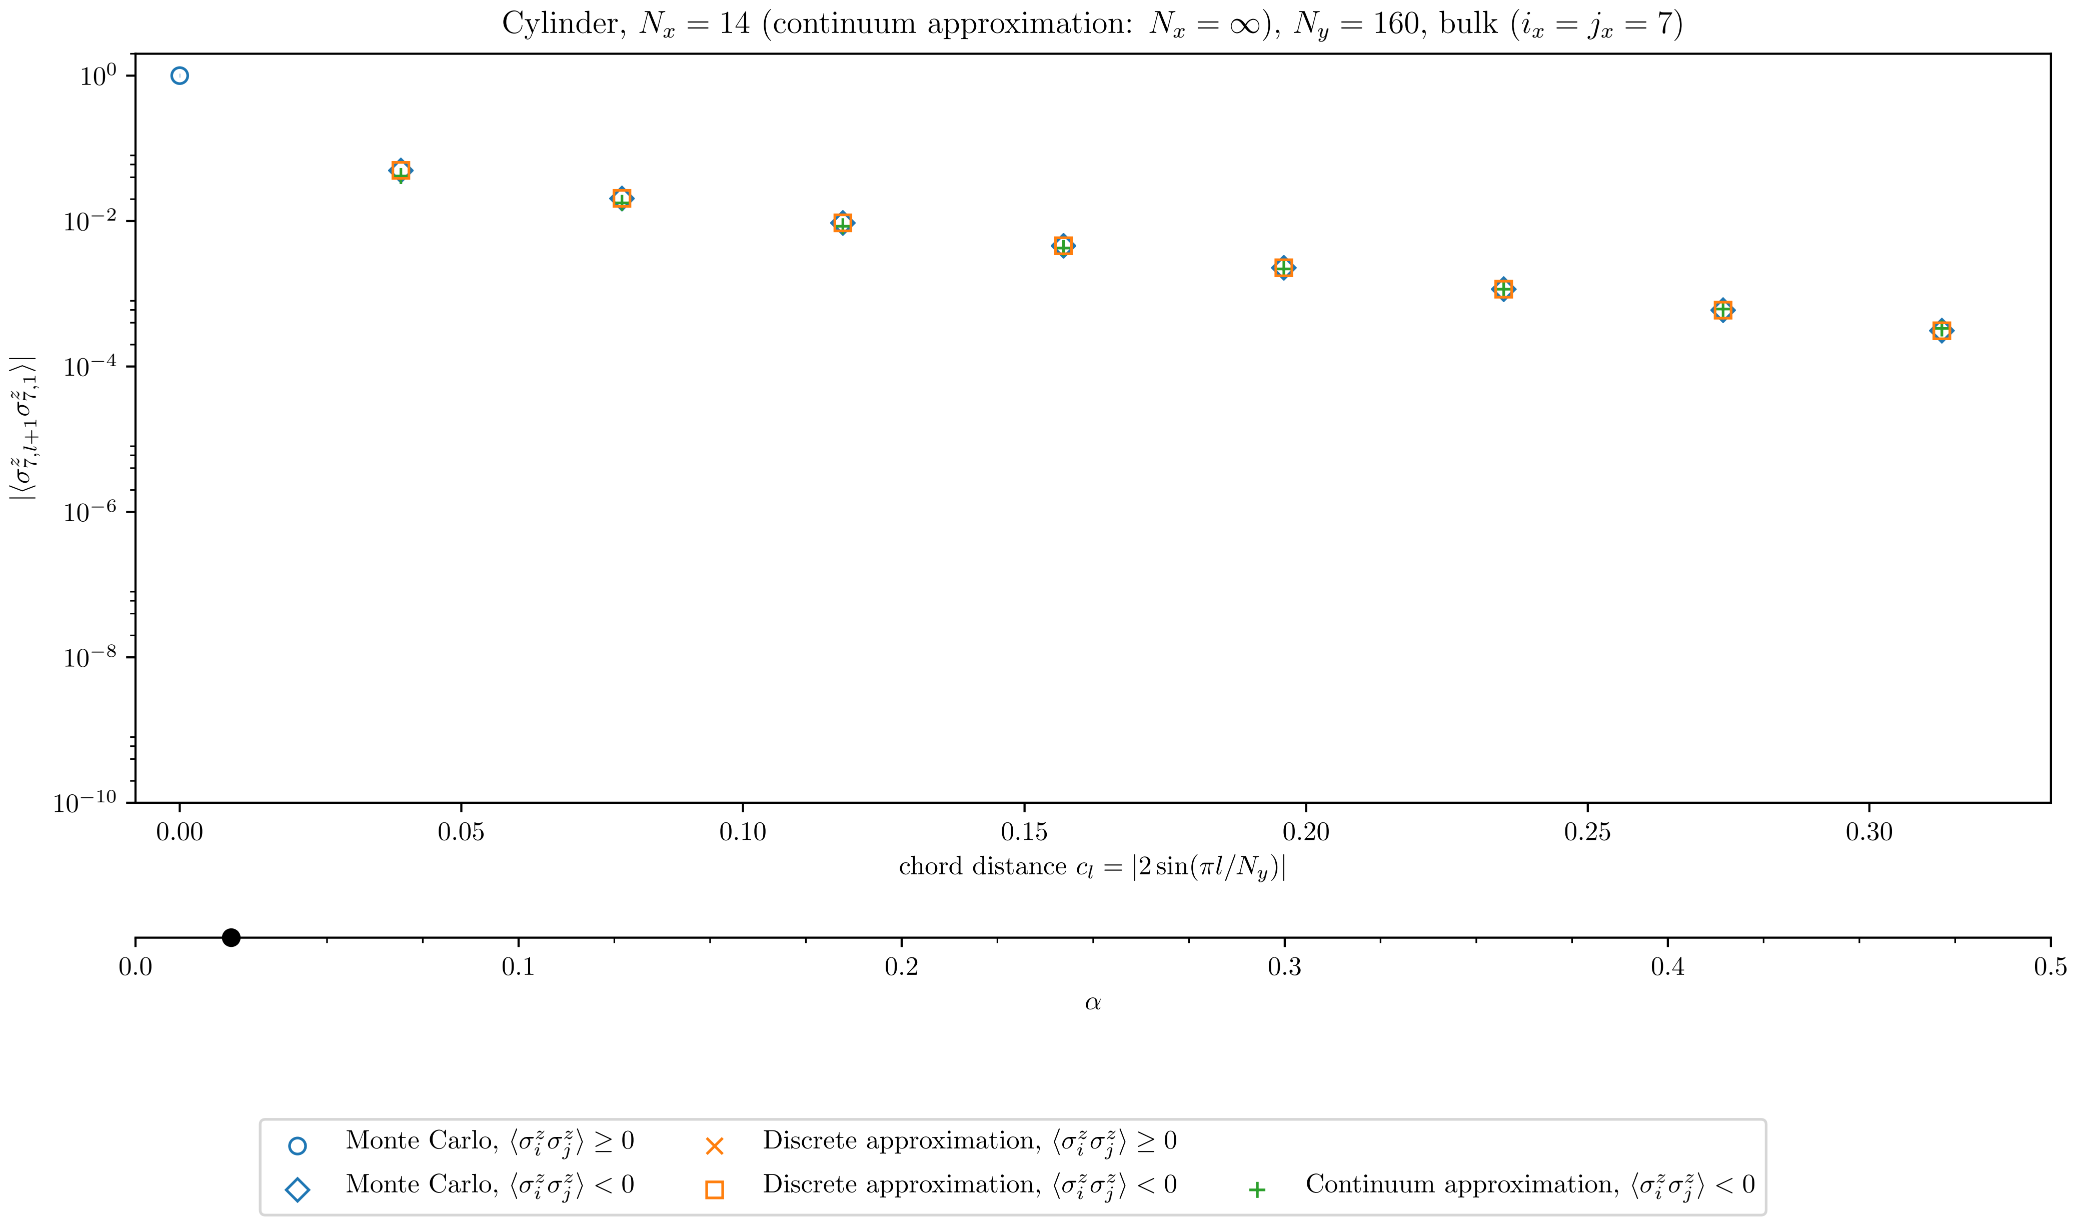

Cylinder, $N_x = 14$ (continuum approximation: $N_x = \infty$), $N_y = 160$, bulk ($i_x = j_x = 7$)
$|\langle \sigma^z_{7,l+1} \sigma^z_{7,1} \rangle|$
$10^0$
$10^{-2}$
$10^{-4}$
$10^{-6}$
$10^{-8}$
$10^{-10}$
0.00
0.05
0.10
0.15
0.20
0.25
0.30
chord distance $c_l = |2 \sin(\pi l / N_y)|$
0.0
0.1
0.2
0.3
0.4
0.5
$\alpha$
Monte Carlo, $\langle \sigma^z_i \sigma^z_j \rangle \geq 0$
Monte Carlo, $\langle \sigma^z_i \sigma^z_j \rangle < 0$
Discrete approximation, $\langle \sigma^z_i \sigma^z_j \rangle \geq 0$
Discrete approximation, $\langle \sigma^z_i \sigma^z_j \rangle < 0$
Continuum approximation, $\langle \sigma^z_i \sigma^z_j \rangle < 0$

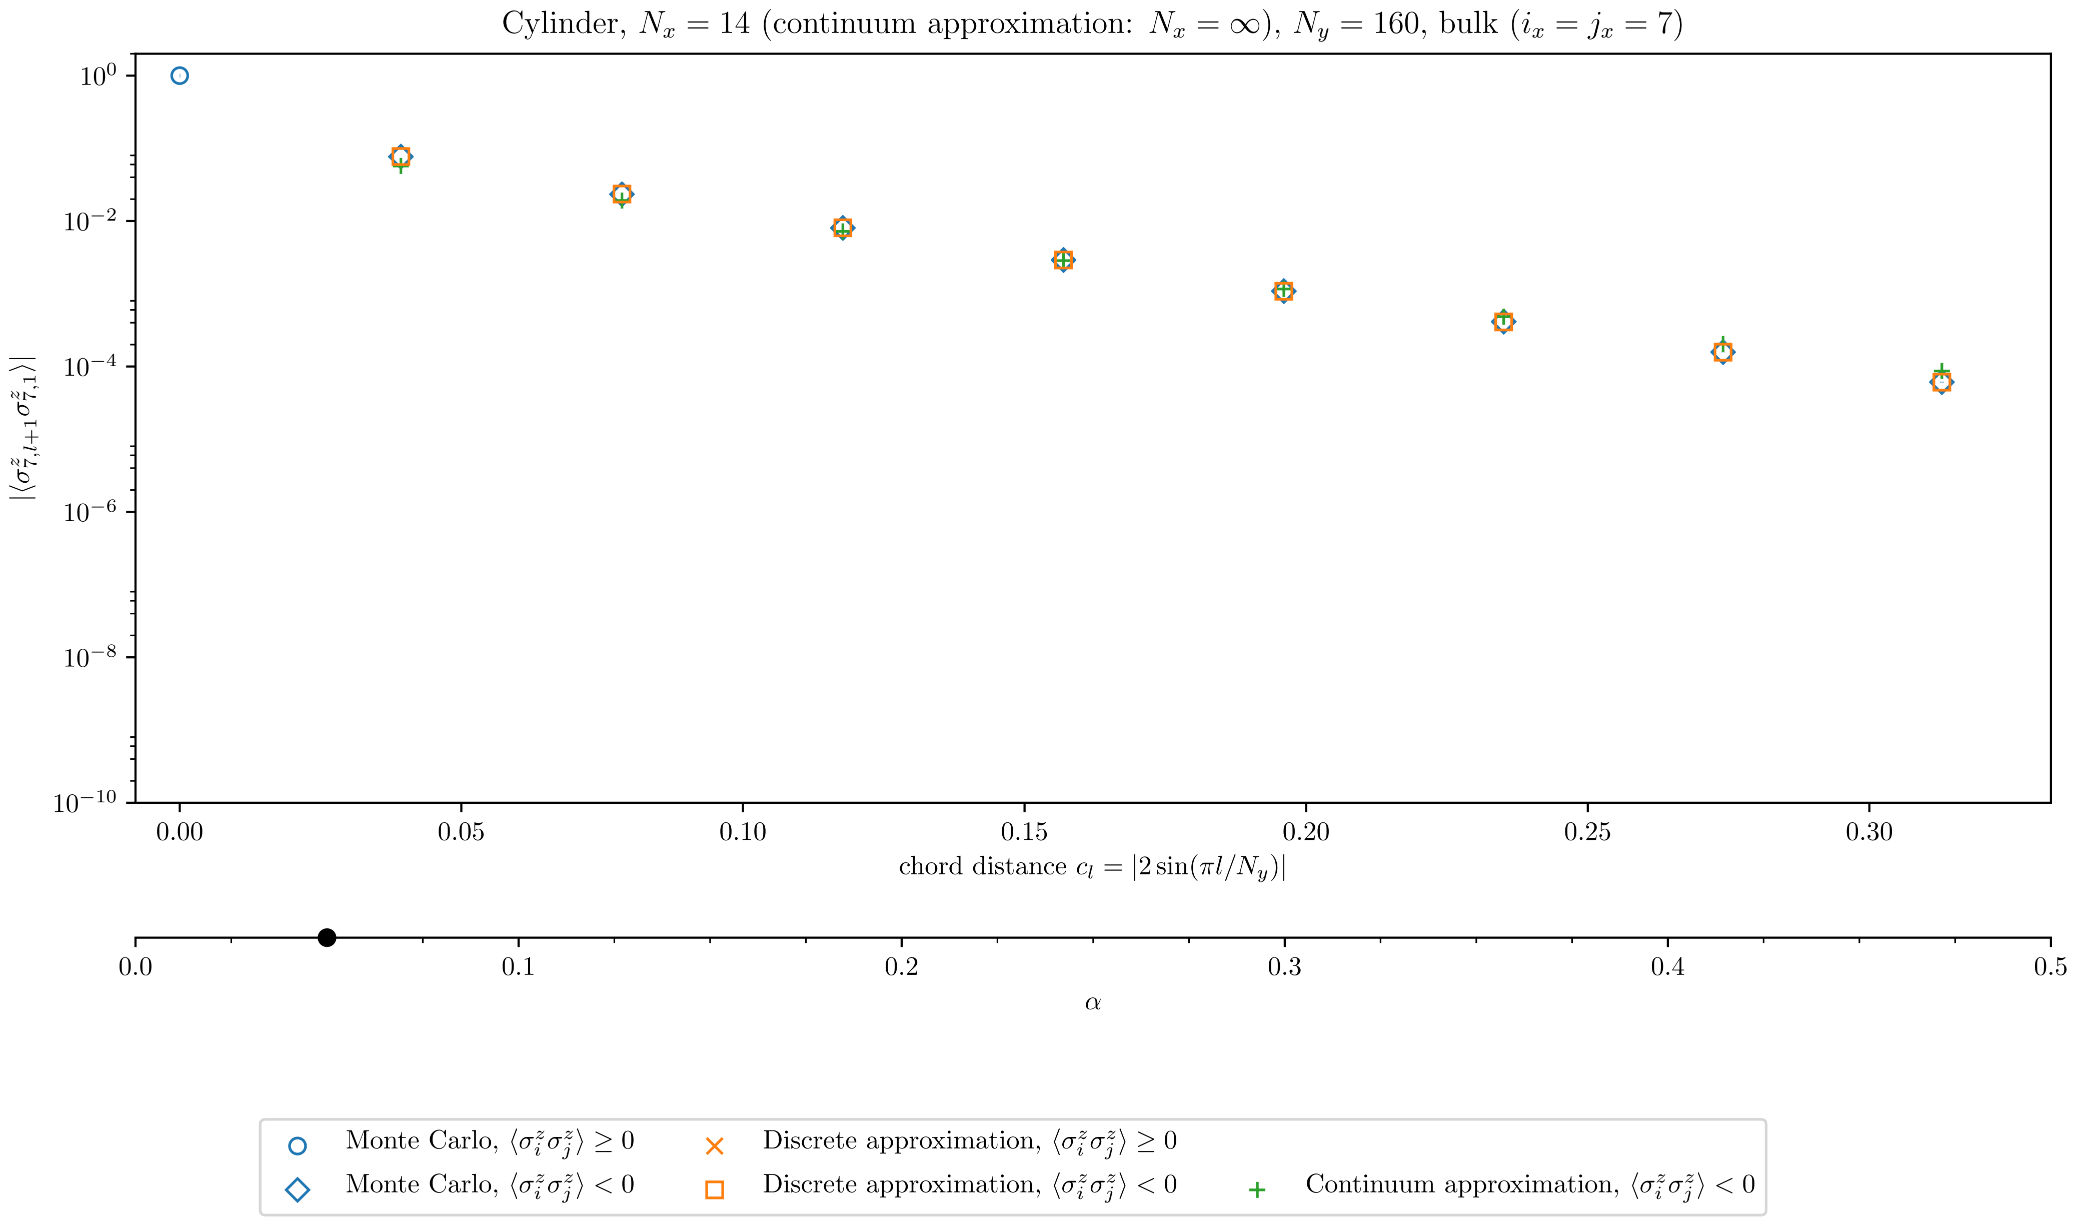

Cylinder, $N_x = 14$ (continuum approximation: $N_x = \infty$), $N_y = 160$, bulk ($i_x = j_x = 7$)
$|\langle \sigma^z_{7,l+1} \sigma^z_{7,1} \rangle|$
$10^{0}$
$10^{-2}$
$10^{-4}$
$10^{-6}$
$10^{-8}$
$10^{-10}$
0.00
0.05
0.10
0.15
0.20
0.25
0.30
chord distance $c_l = |2 \sin(\pi l / N_y)|$
0.0
0.1
0.2
0.3
0.4
0.5
$\alpha$
Monte Carlo, $\langle \sigma^z_i \sigma^z_j \rangle \geq 0$
Monte Carlo, $\langle \sigma^z_i \sigma^z_j \rangle < 0$
Discrete approximation, $\langle \sigma^z_i \sigma^z_j \rangle \geq 0$
Discrete approximation, $\langle \sigma^z_i \sigma^z_j \rangle < 0$
Continuum approximation, $\langle \sigma^z_i \sigma^z_j \rangle < 0$

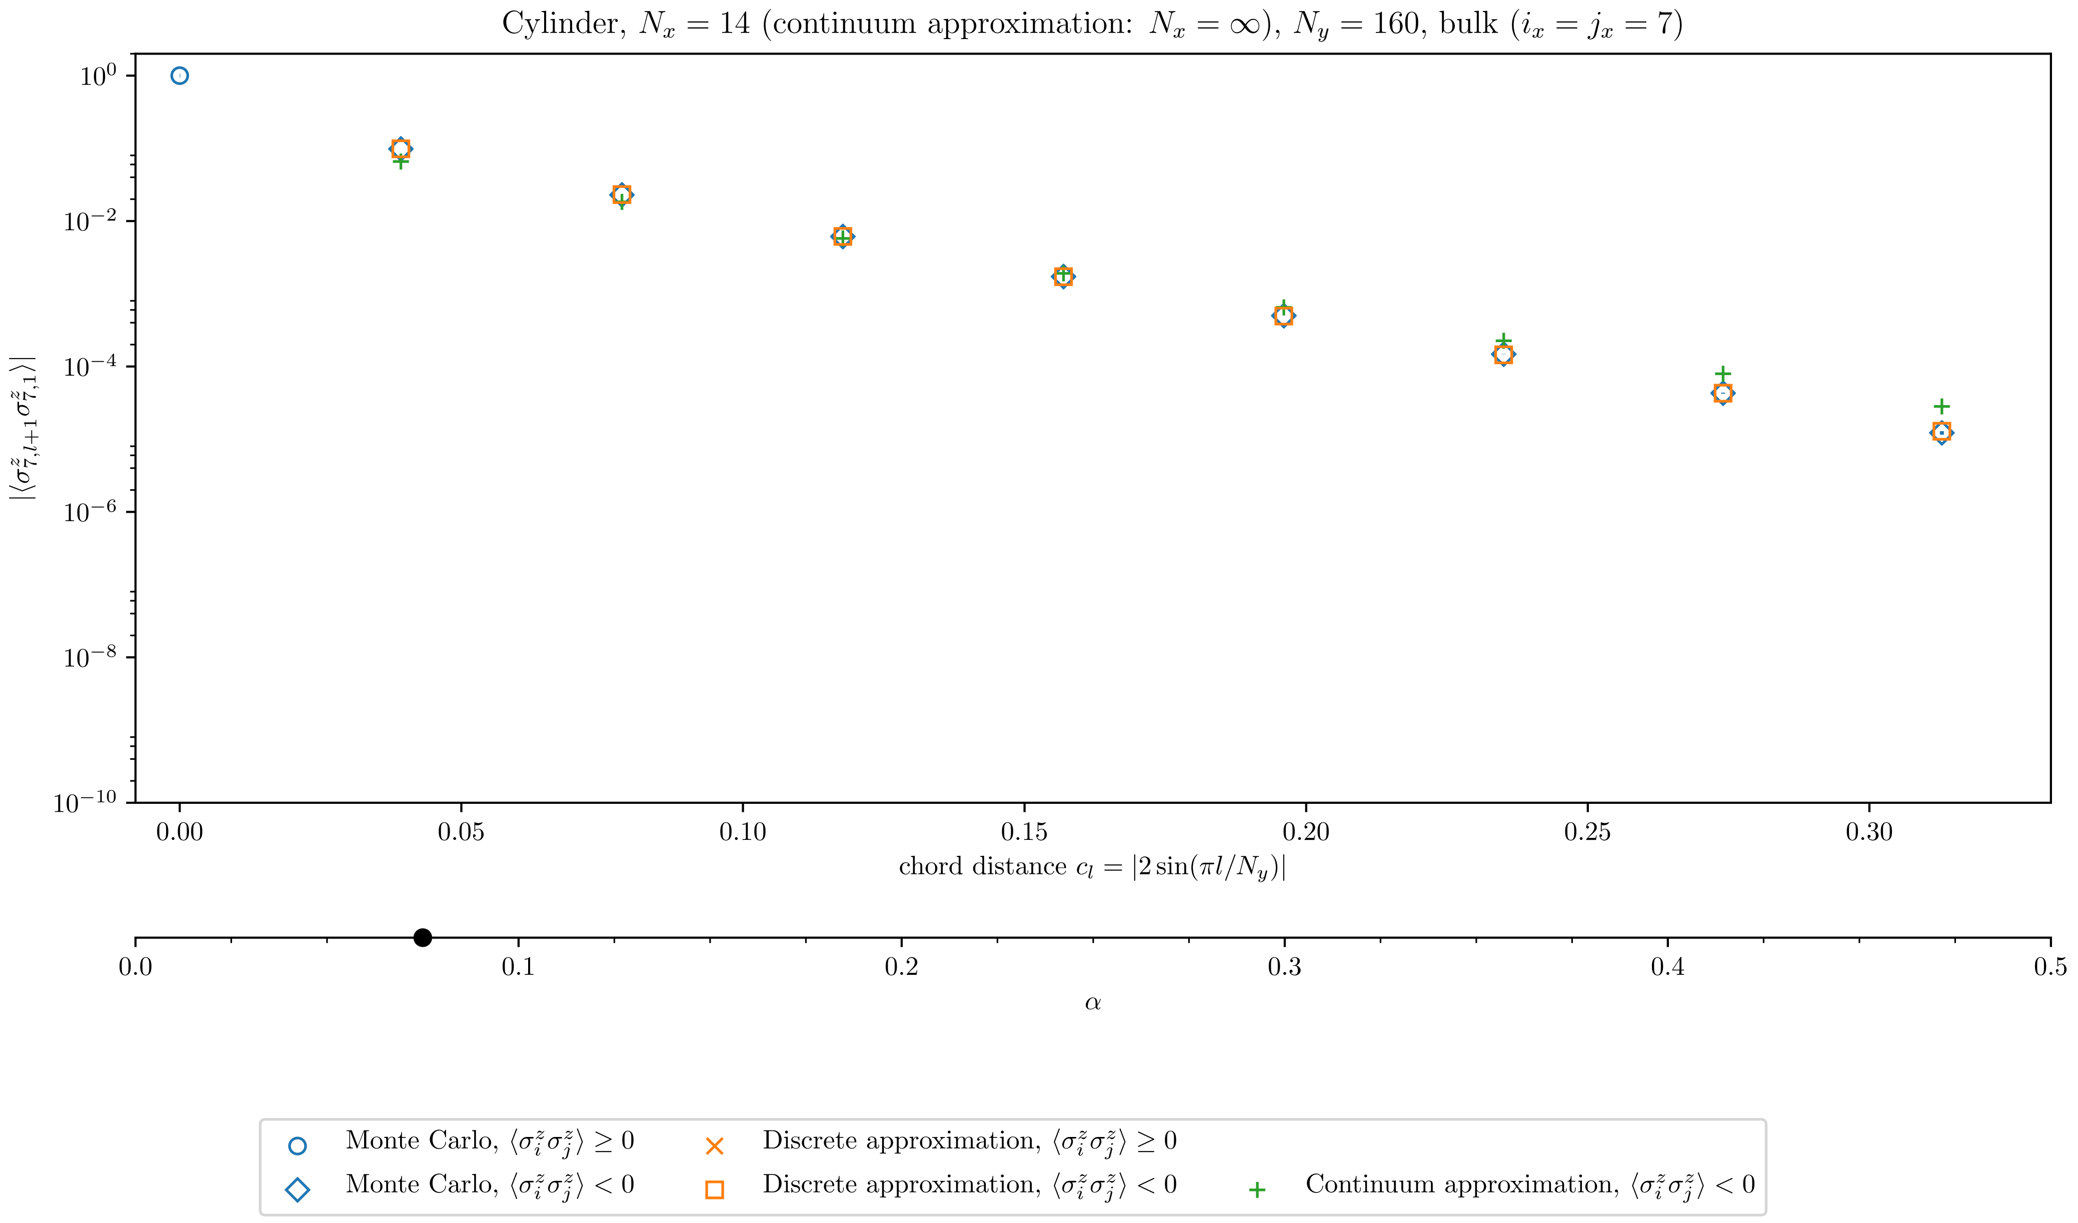

Cylinder, $N_x = 14$ (continuum approximation: $N_x = \infty$), $N_y = 160$, bulk ($i_x = j_x = 7$)
$|\langle \sigma^z_{7,l+1} \sigma^z_{7,1} \rangle|$
$10^0$
$10^{-2}$
$10^{-4}$
$10^{-6}$
$10^{-8}$
$10^{-10}$
0.00
0.05
0.10
0.15
0.20
0.25
0.30
chord distance $c_l = |2 \sin(\pi l / N_y)|$
0.0
0.1
0.2
0.3
0.4
0.5
$\alpha$
Monte Carlo, $\langle \sigma^z_i \sigma^z_j \rangle \geq 0$
Monte Carlo, $\langle \sigma^z_i \sigma^z_j \rangle < 0$
Discrete approximation, $\langle \sigma^z_i \sigma^z_j \rangle \geq 0$
Discrete approximation, $\langle \sigma^z_i \sigma^z_j \rangle < 0$
Continuum approximation, $\langle \sigma^z_i \sigma^z_j \rangle < 0$

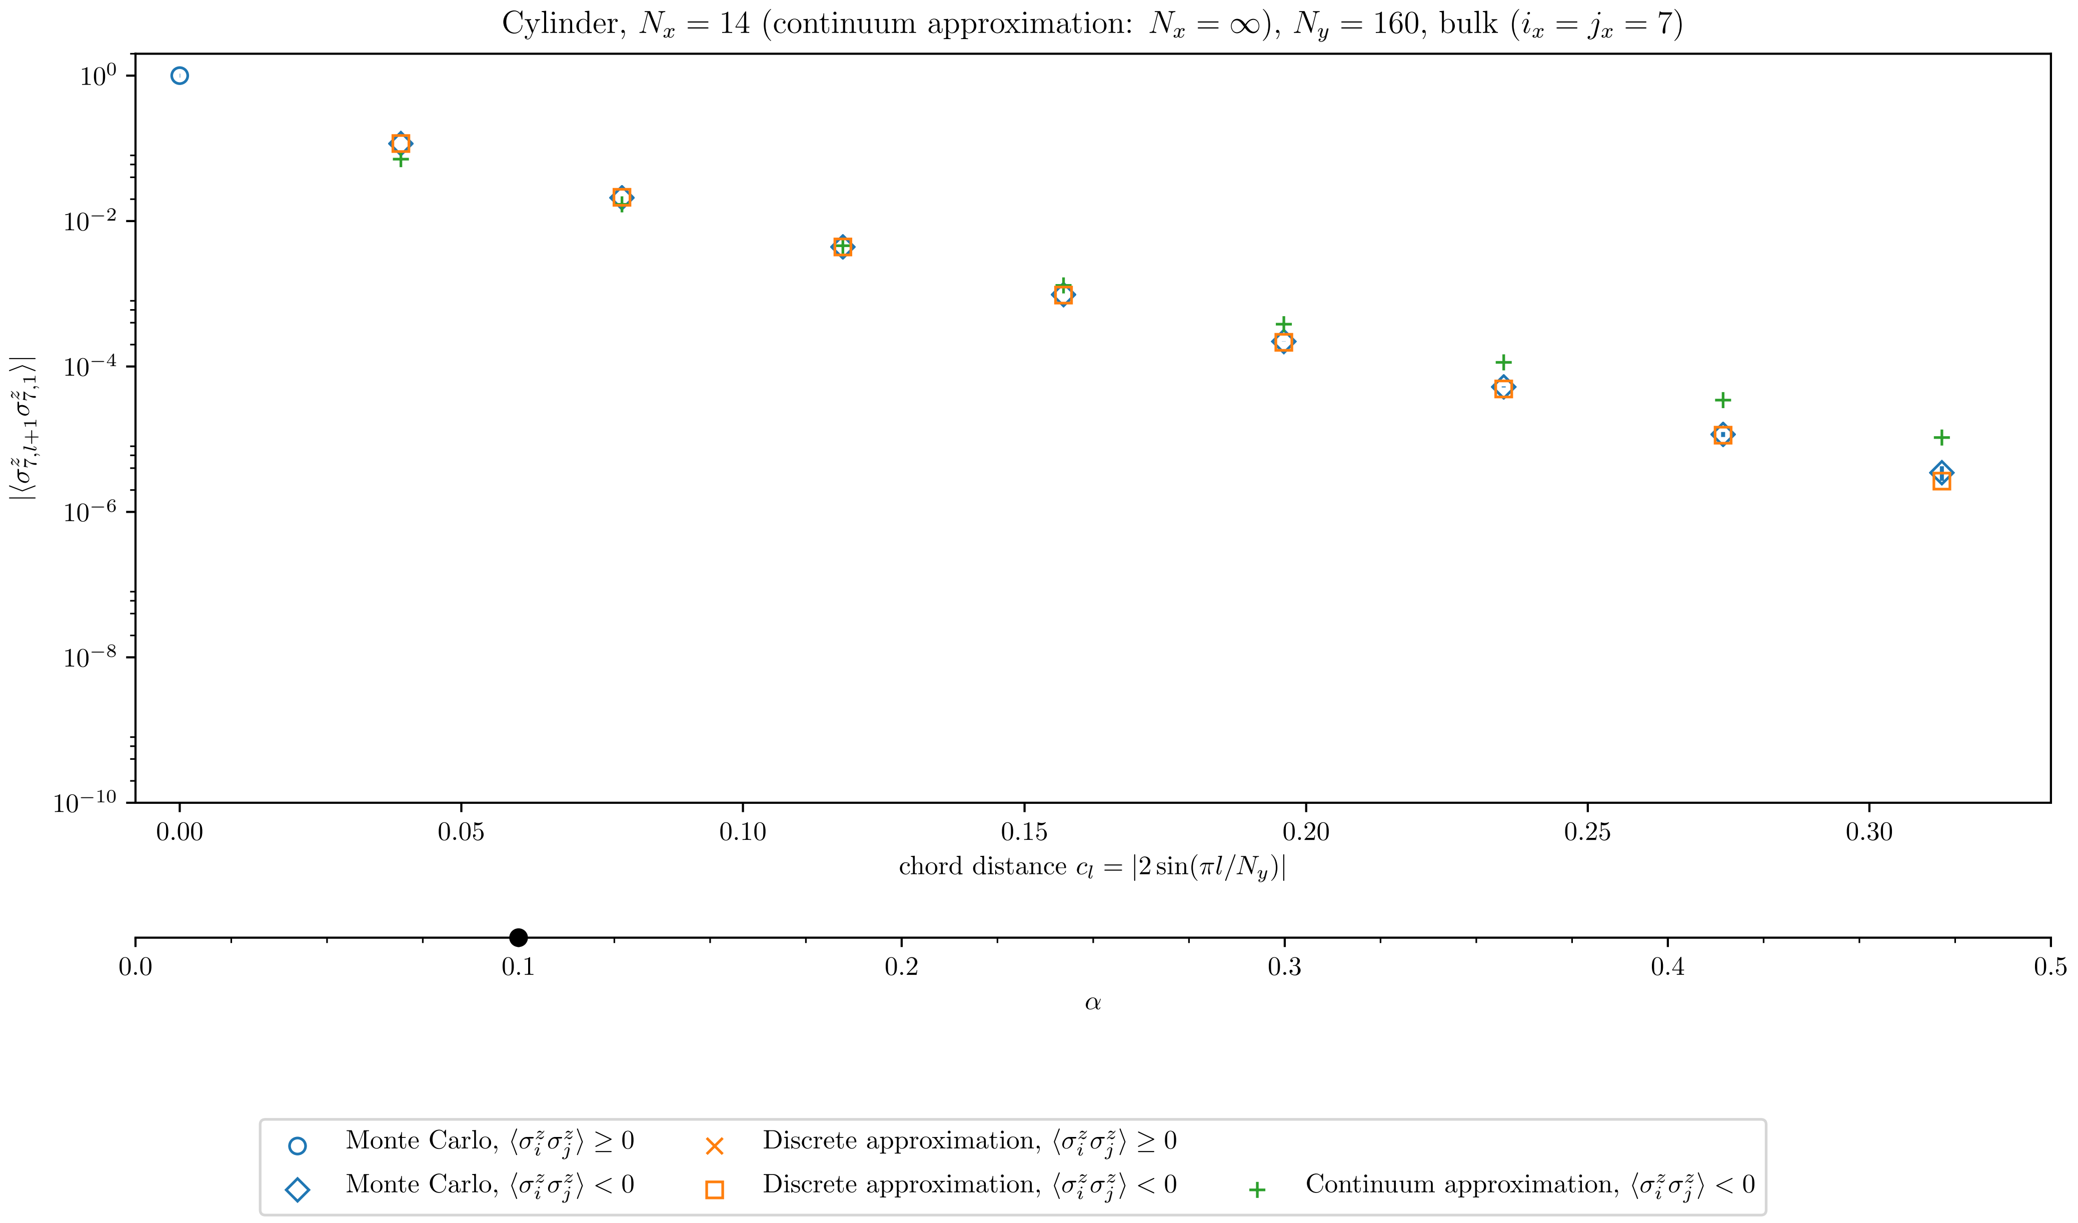
Cylinder, $N_x = 14$ (continuum approximation: $N_x = \infty$), $N_y = 160$, bulk ($i_x = j_x = 7$)
$|\langle \sigma^z_{7,l+1} \sigma^z_{7,1} \rangle|$
$10^0$
$10^{-2}$
$10^{-4}$
$10^{-6}$
$10^{-8}$
$10^{-10}$
0.00
0.05
0.10
0.15
0.20
0.25
0.30
chord distance $c_l = |2\sin(\pi l/N_y)|$
0.0
0.1
0.2
0.3
0.4
0.5
$\alpha$
Monte Carlo, $\langle \sigma^z_i \sigma^z_j \rangle \geq 0$
Monte Carlo, $\langle \sigma^z_i \sigma^z_j \rangle < 0$
Discrete approximation, $\langle \sigma^z_i \sigma^z_j \rangle \geq 0$
Discrete approximation, $\langle \sigma^z_i \sigma^z_j \rangle < 0$
Continuum approximation, $\langle \sigma^z_i \sigma^z_j \rangle < 0$

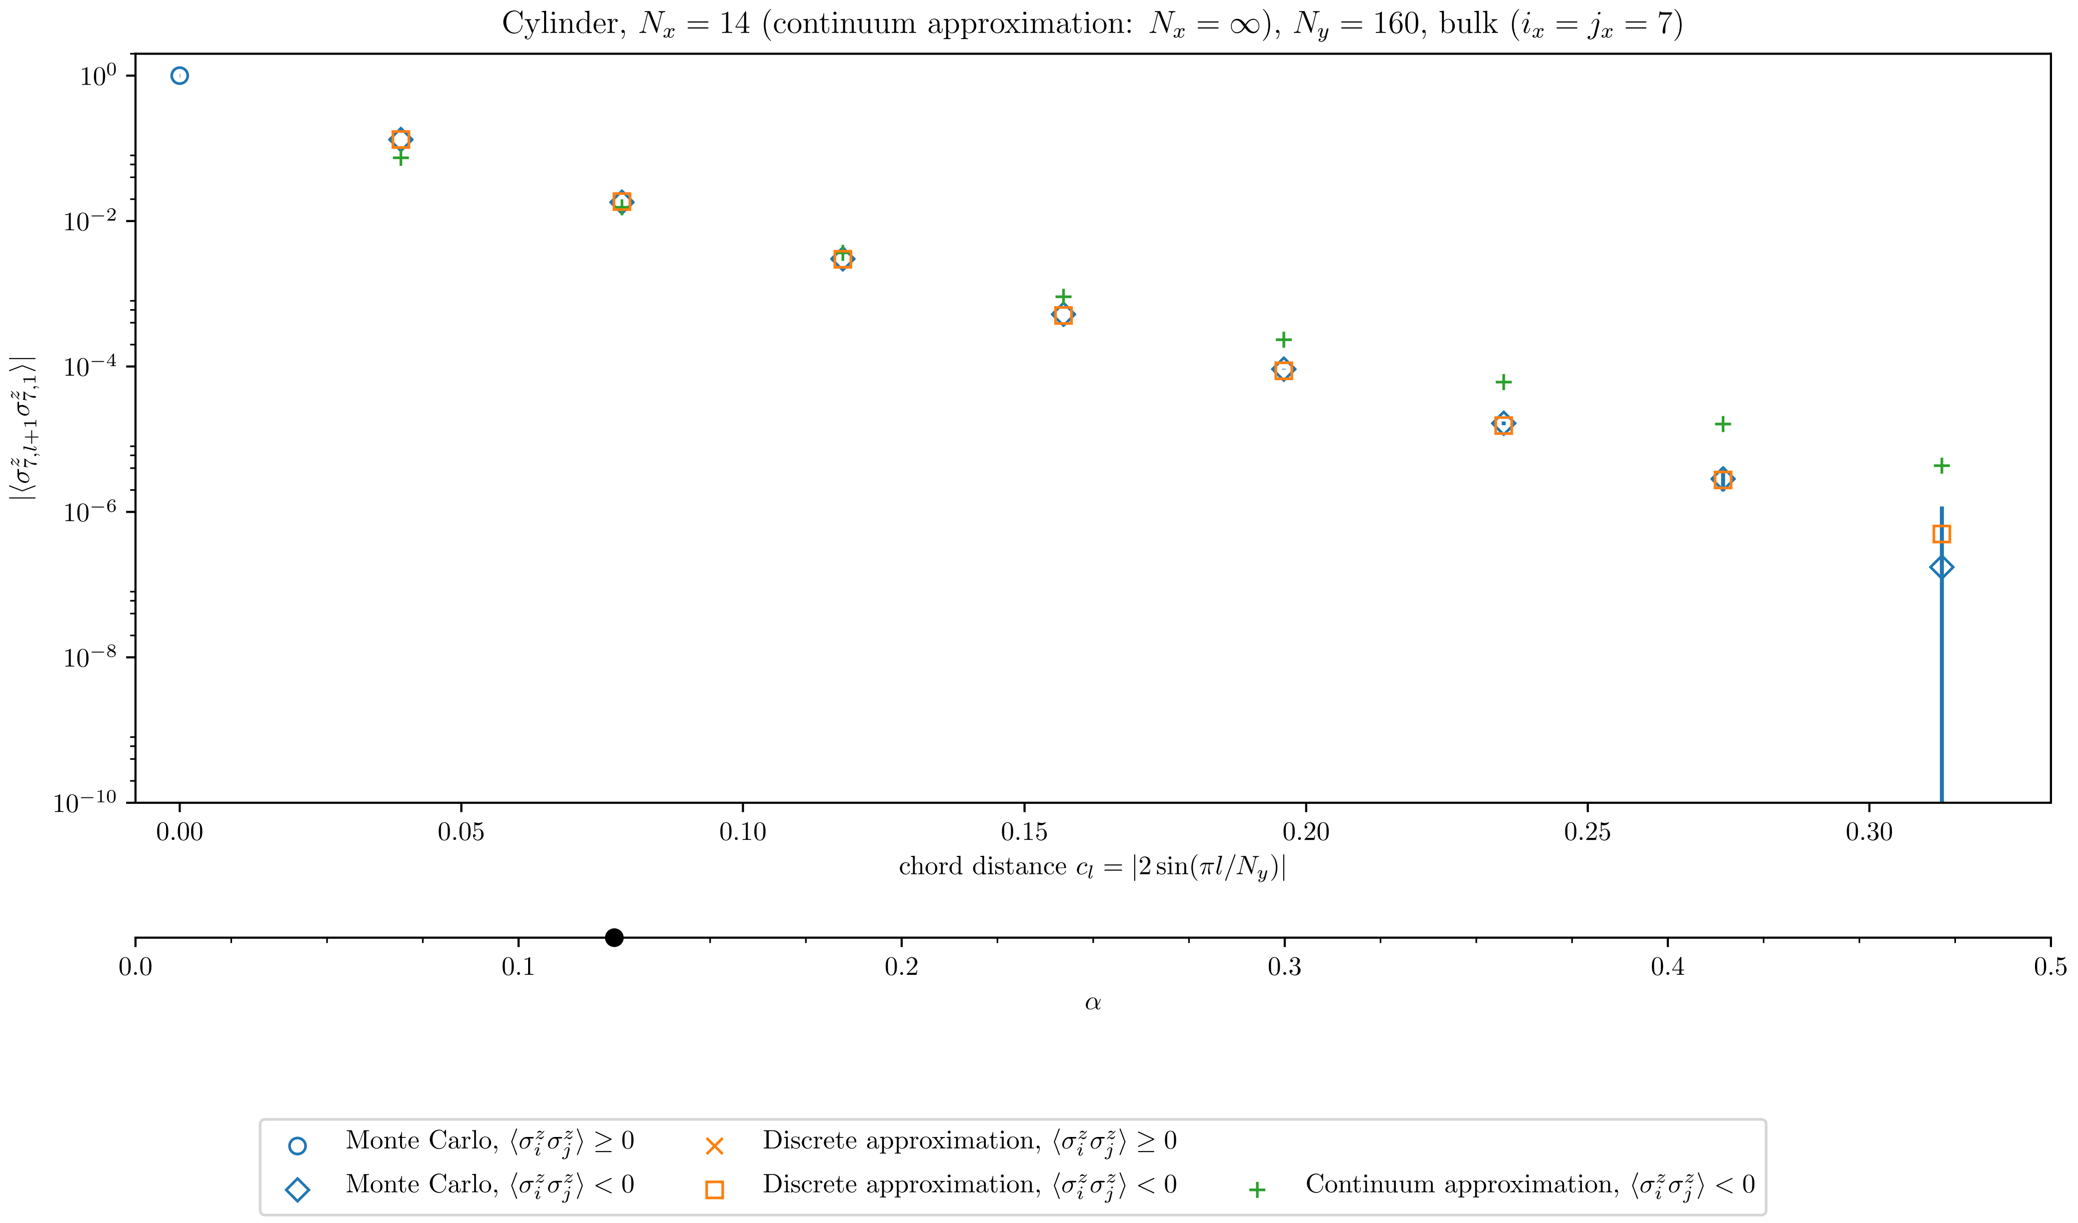

Cylinder, $N_x = 14$ (continuum approximation: $N_x = \infty$), $N_y = 160$, bulk ($i_x = j_x = 7$)
$|\langle \sigma^z_{7,l+1} \sigma^z_{7,1} \rangle|$
$10^0$
$10^{-2}$
$10^{-4}$
$10^{-6}$
$10^{-8}$
$10^{-10}$
0.00
0.05
0.10
0.15
0.20
0.25
0.30
chord distance $c_l = |2\sin(\pi l/N_y)|$
0.0
0.1
0.2
0.3
0.4
0.5
$\alpha$
Monte Carlo, $\langle \sigma^z_i \sigma^z_j \rangle \geq 0$
Monte Carlo, $\langle \sigma^z_i \sigma^z_j \rangle < 0$
Discrete approximation, $\langle \sigma^z_i \sigma^z_j \rangle \geq 0$
Discrete approximation, $\langle \sigma^z_i \sigma^z_j \rangle < 0$
Continuum approximation, $\langle \sigma^z_i \sigma^z_j \rangle < 0$

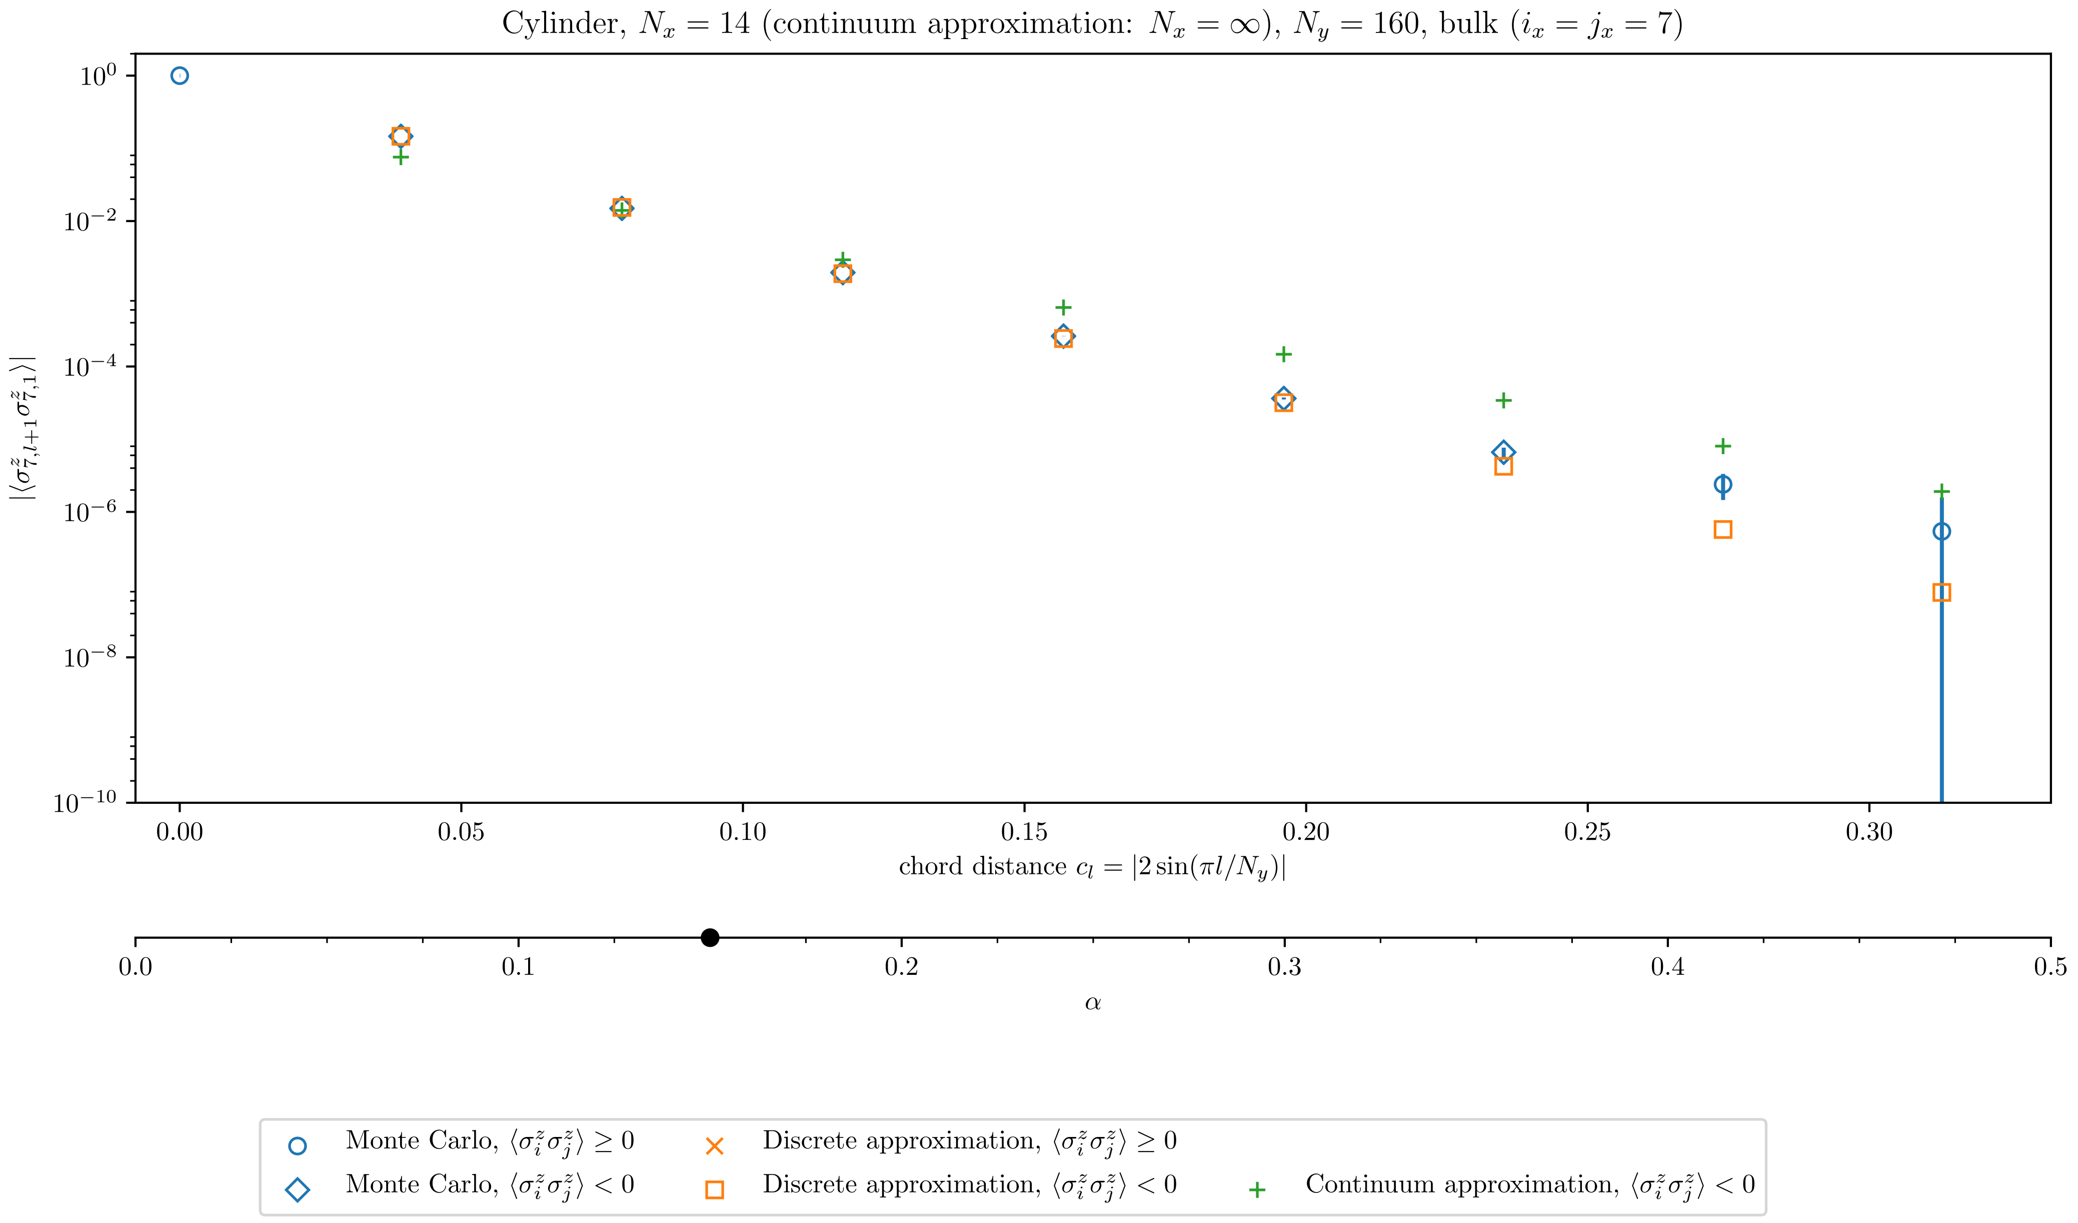

Cylinder, $N_x = 14$ (continuum approximation: $N_x = \infty$), $N_y = 160$, bulk ($i_x = j_x = 7$)
$|\langle \sigma^z_{7,l+1} \sigma^z_{7,1} \rangle|$
$10^0$
$10^{-2}$
$10^{-4}$
$10^{-6}$
$10^{-8}$
$10^{-10}$
0.00
0.05
0.10
0.15
0.20
0.25
0.30
chord distance $c_l = |2\sin(\pi l/N_y)|$
0.0
0.1
0.2
0.3
0.4
0.5
$\alpha$
Monte Carlo, $\langle \sigma^z_i \sigma^z_j \rangle \geq 0$
Monte Carlo, $\langle \sigma^z_i \sigma^z_j \rangle < 0$
Discrete approximation, $\langle \sigma^z_i \sigma^z_j \rangle \geq 0$
Discrete approximation, $\langle \sigma^z_i \sigma^z_j \rangle < 0$
Continuum approximation, $\langle \sigma^z_i \sigma^z_j \rangle < 0$

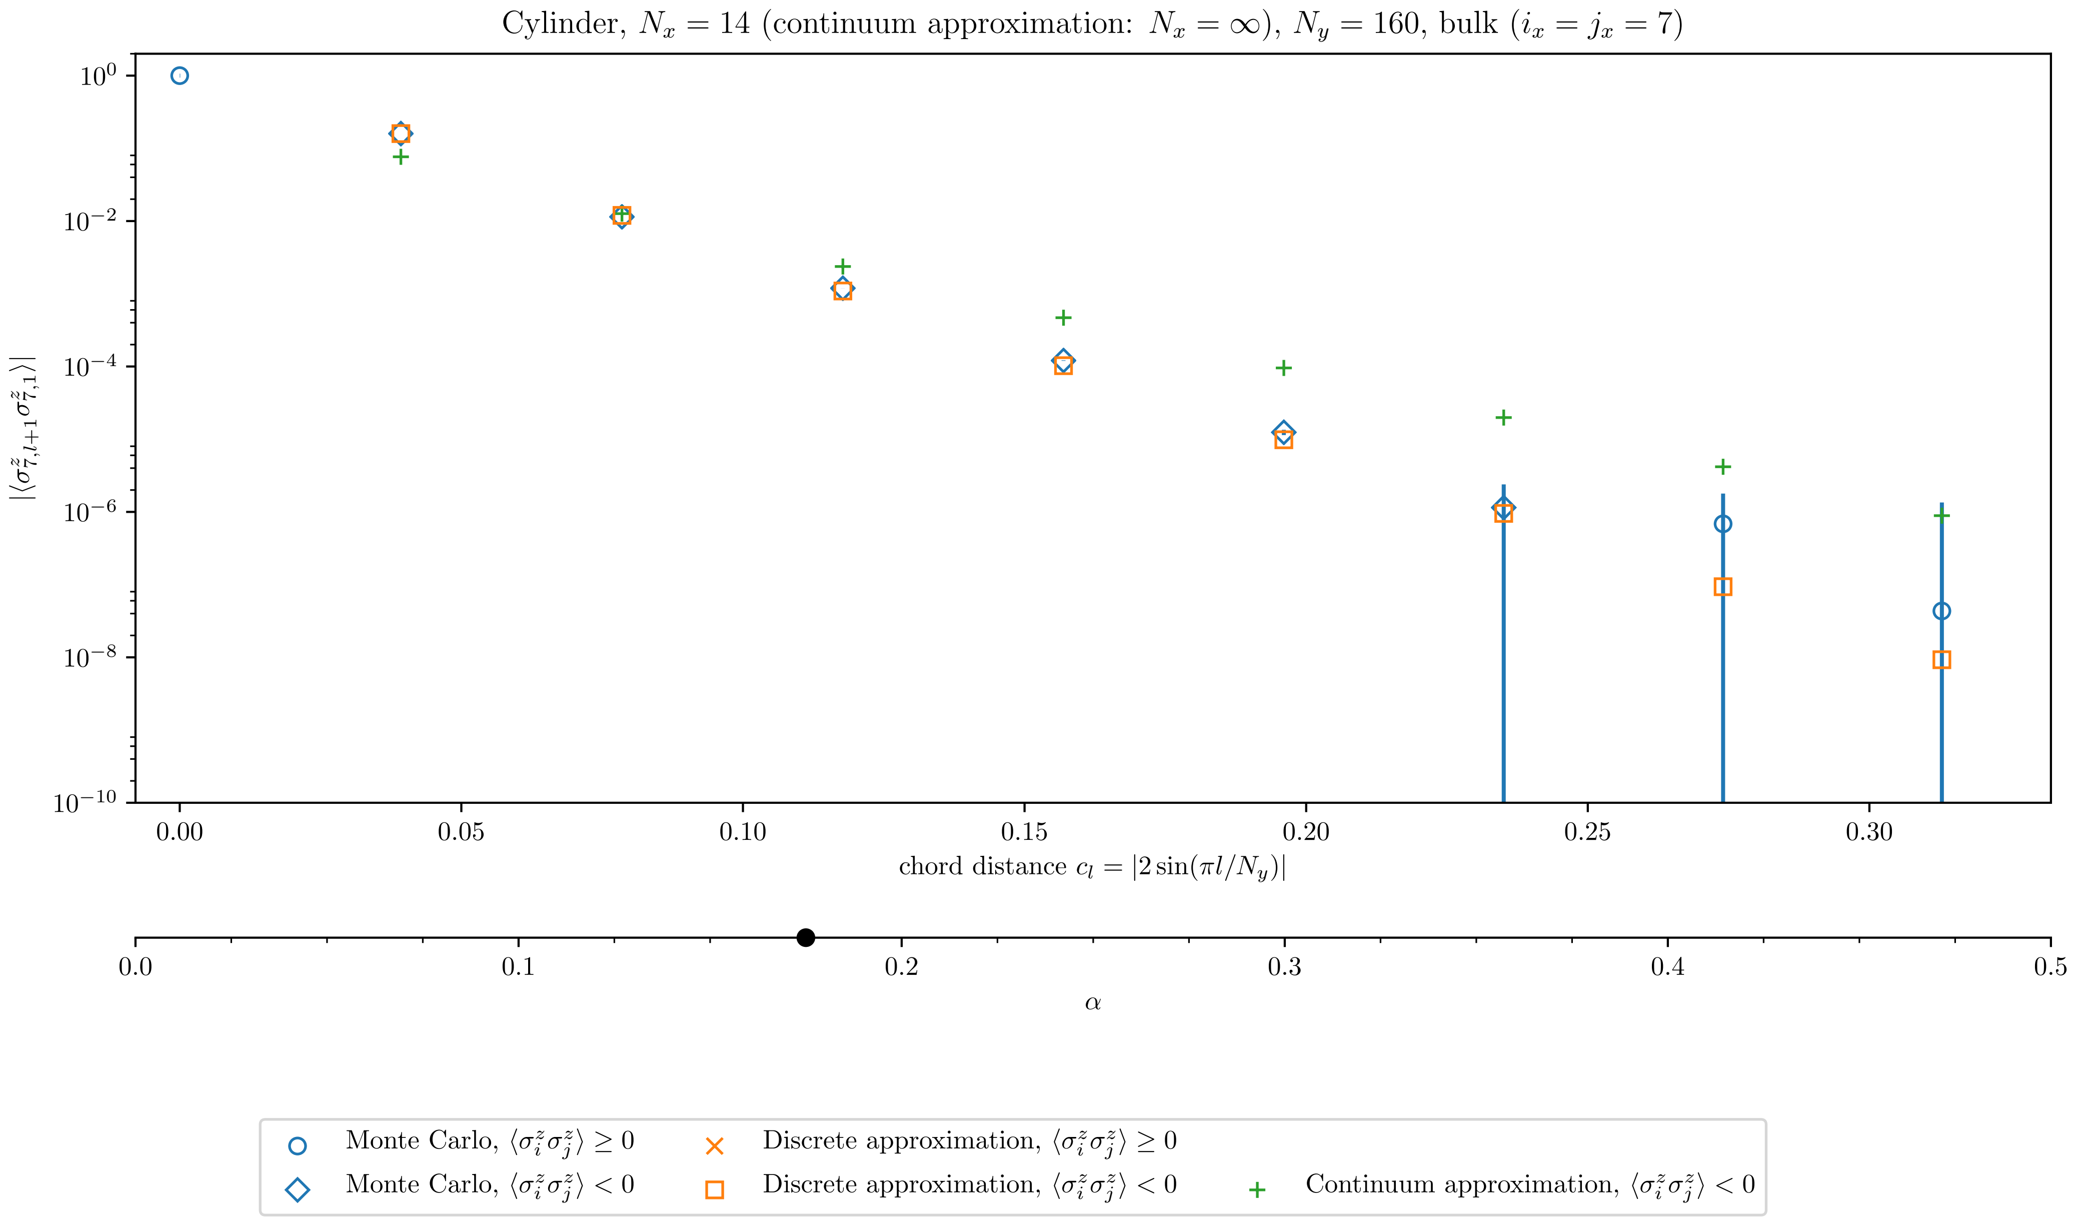

Cylinder, $N_x = 14$ (continuum approximation: $N_x = \infty$), $N_y = 160$, bulk ($i_x = j_x = 7$)
$|\langle\sigma^z_{7,l+1}\sigma^z_{7,1}\rangle|$
$10^0$
$10^{-2}$
$10^{-4}$
$10^{-6}$
$10^{-8}$
$10^{-10}$
0.00
0.05
0.10
0.15
0.20
0.25
0.30
chord distance $c_l = |2\sin(\pi l/N_y)|$
0.0
0.1
0.2
0.3
0.4
0.5
$\alpha$
Monte Carlo, $\langle\sigma^z_i\sigma^z_j\rangle \geq 0$
Monte Carlo, $\langle\sigma^z_i\sigma^z_j\rangle < 0$
Discrete approximation, $\langle\sigma^z_i\sigma^z_j\rangle \geq 0$
Discrete approximation, $\langle\sigma^z_i\sigma^z_j\rangle < 0$
Continuum approximation, $\langle\sigma^z_i\sigma^z_j\rangle < 0$

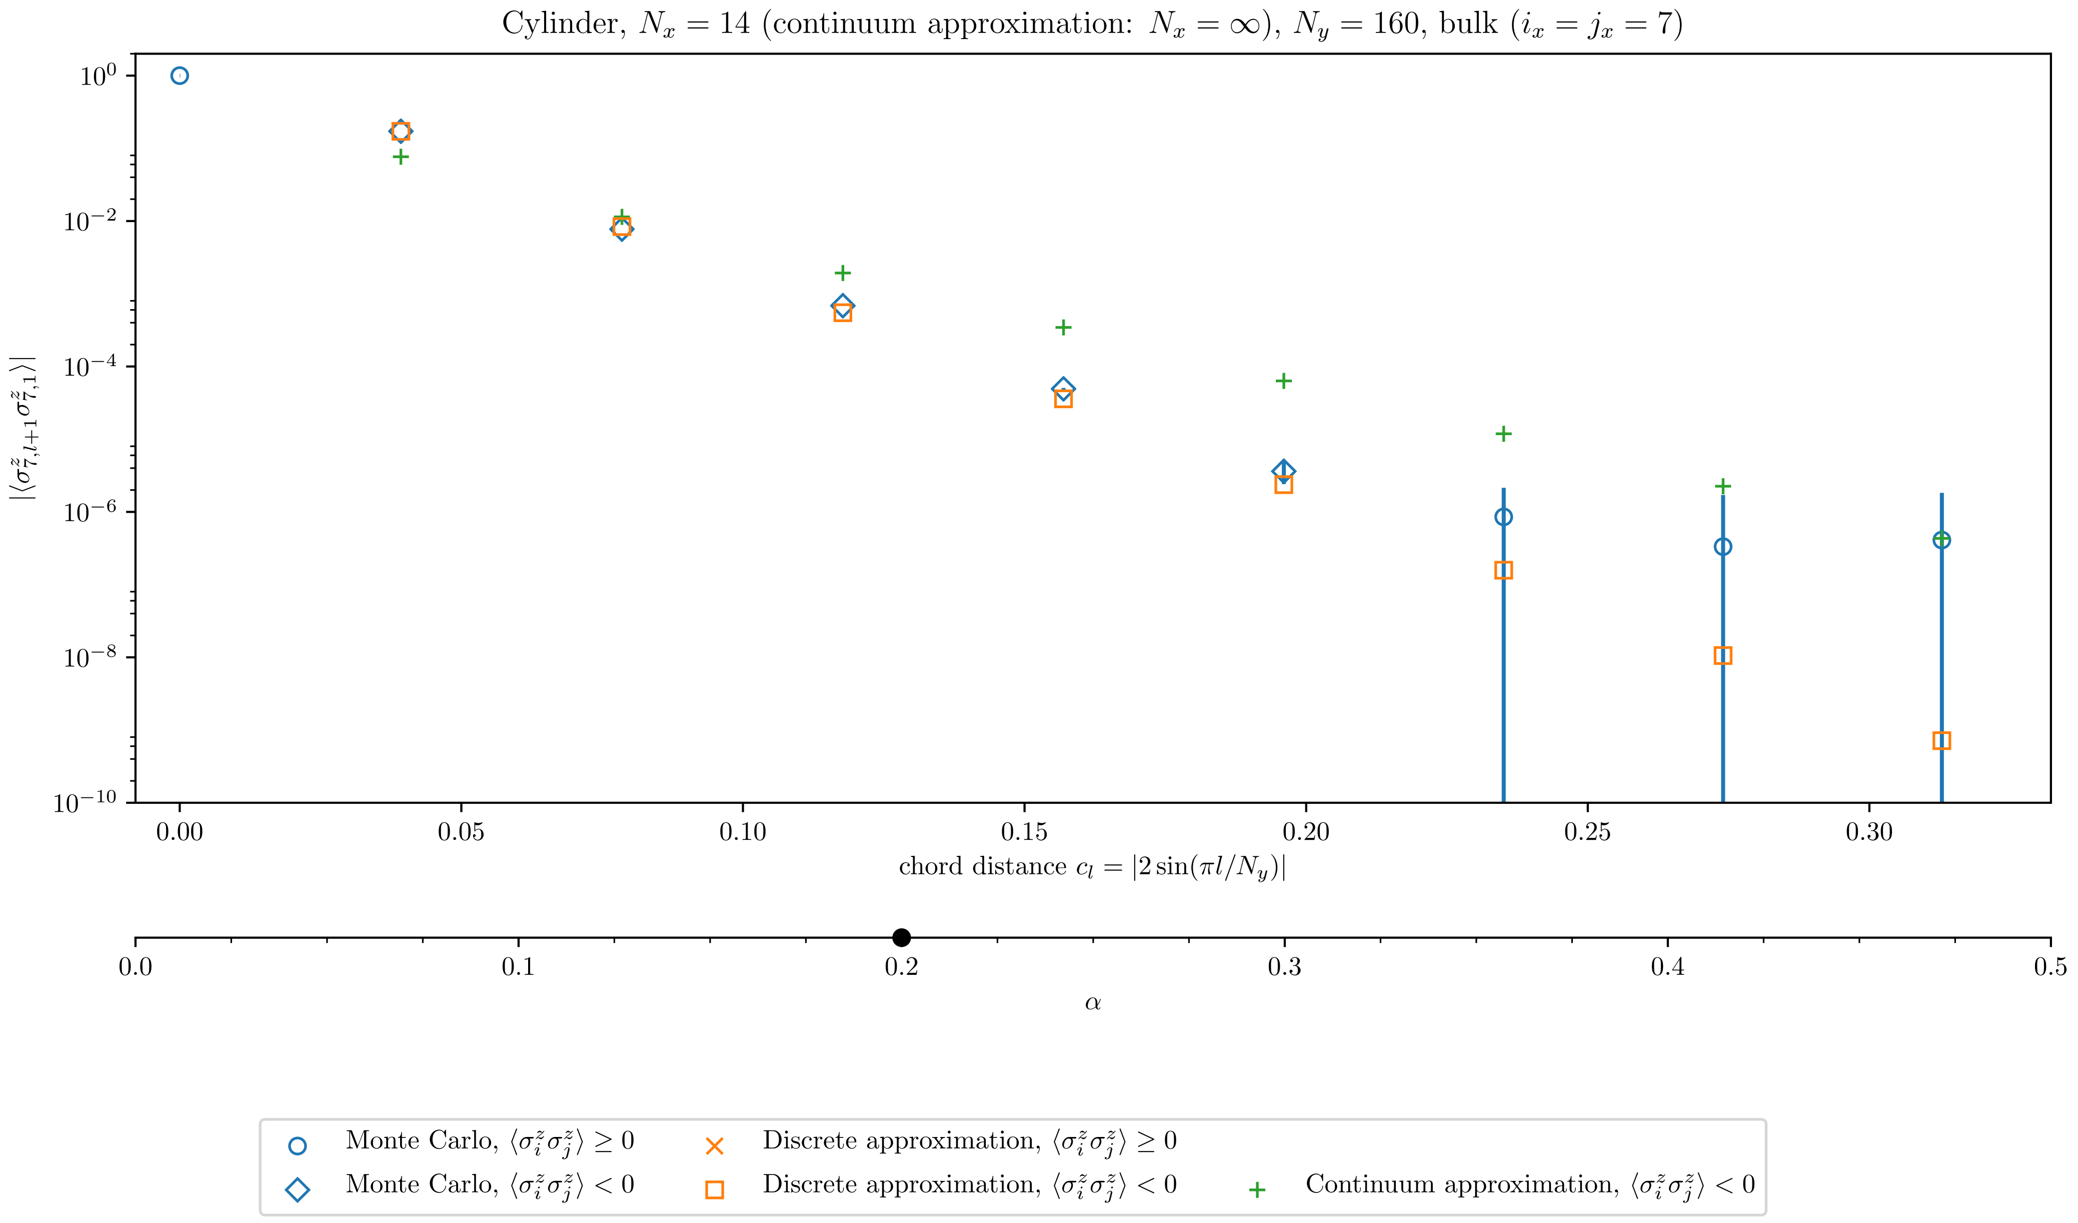

Cylinder, $N_x = 14$ (continuum approximation: $N_x = \infty$), $N_y = 160$, bulk ($i_x = j_x = 7$)
$|\langle \sigma^z_{7,l+1} \sigma^z_{7,1} \rangle|$
$10^{0}$
$10^{-2}$
$10^{-4}$
$10^{-6}$
$10^{-8}$
$10^{-10}$
0.00
0.05
0.10
0.15
0.20
0.25
0.30
chord distance $c_l = |2\sin(\pi l/N_y)|$
0.0
0.1
0.2
0.3
0.4
0.5
$\alpha$
Monte Carlo, $\langle \sigma^z_i \sigma^z_j \rangle \geq 0$
Monte Carlo, $\langle \sigma^z_i \sigma^z_j \rangle < 0$
Discrete approximation, $\langle \sigma^z_i \sigma^z_j \rangle \geq 0$
Discrete approximation, $\langle \sigma^z_i \sigma^z_j \rangle < 0$
Continuum approximation, $\langle \sigma^z_i \sigma^z_j \rangle < 0$

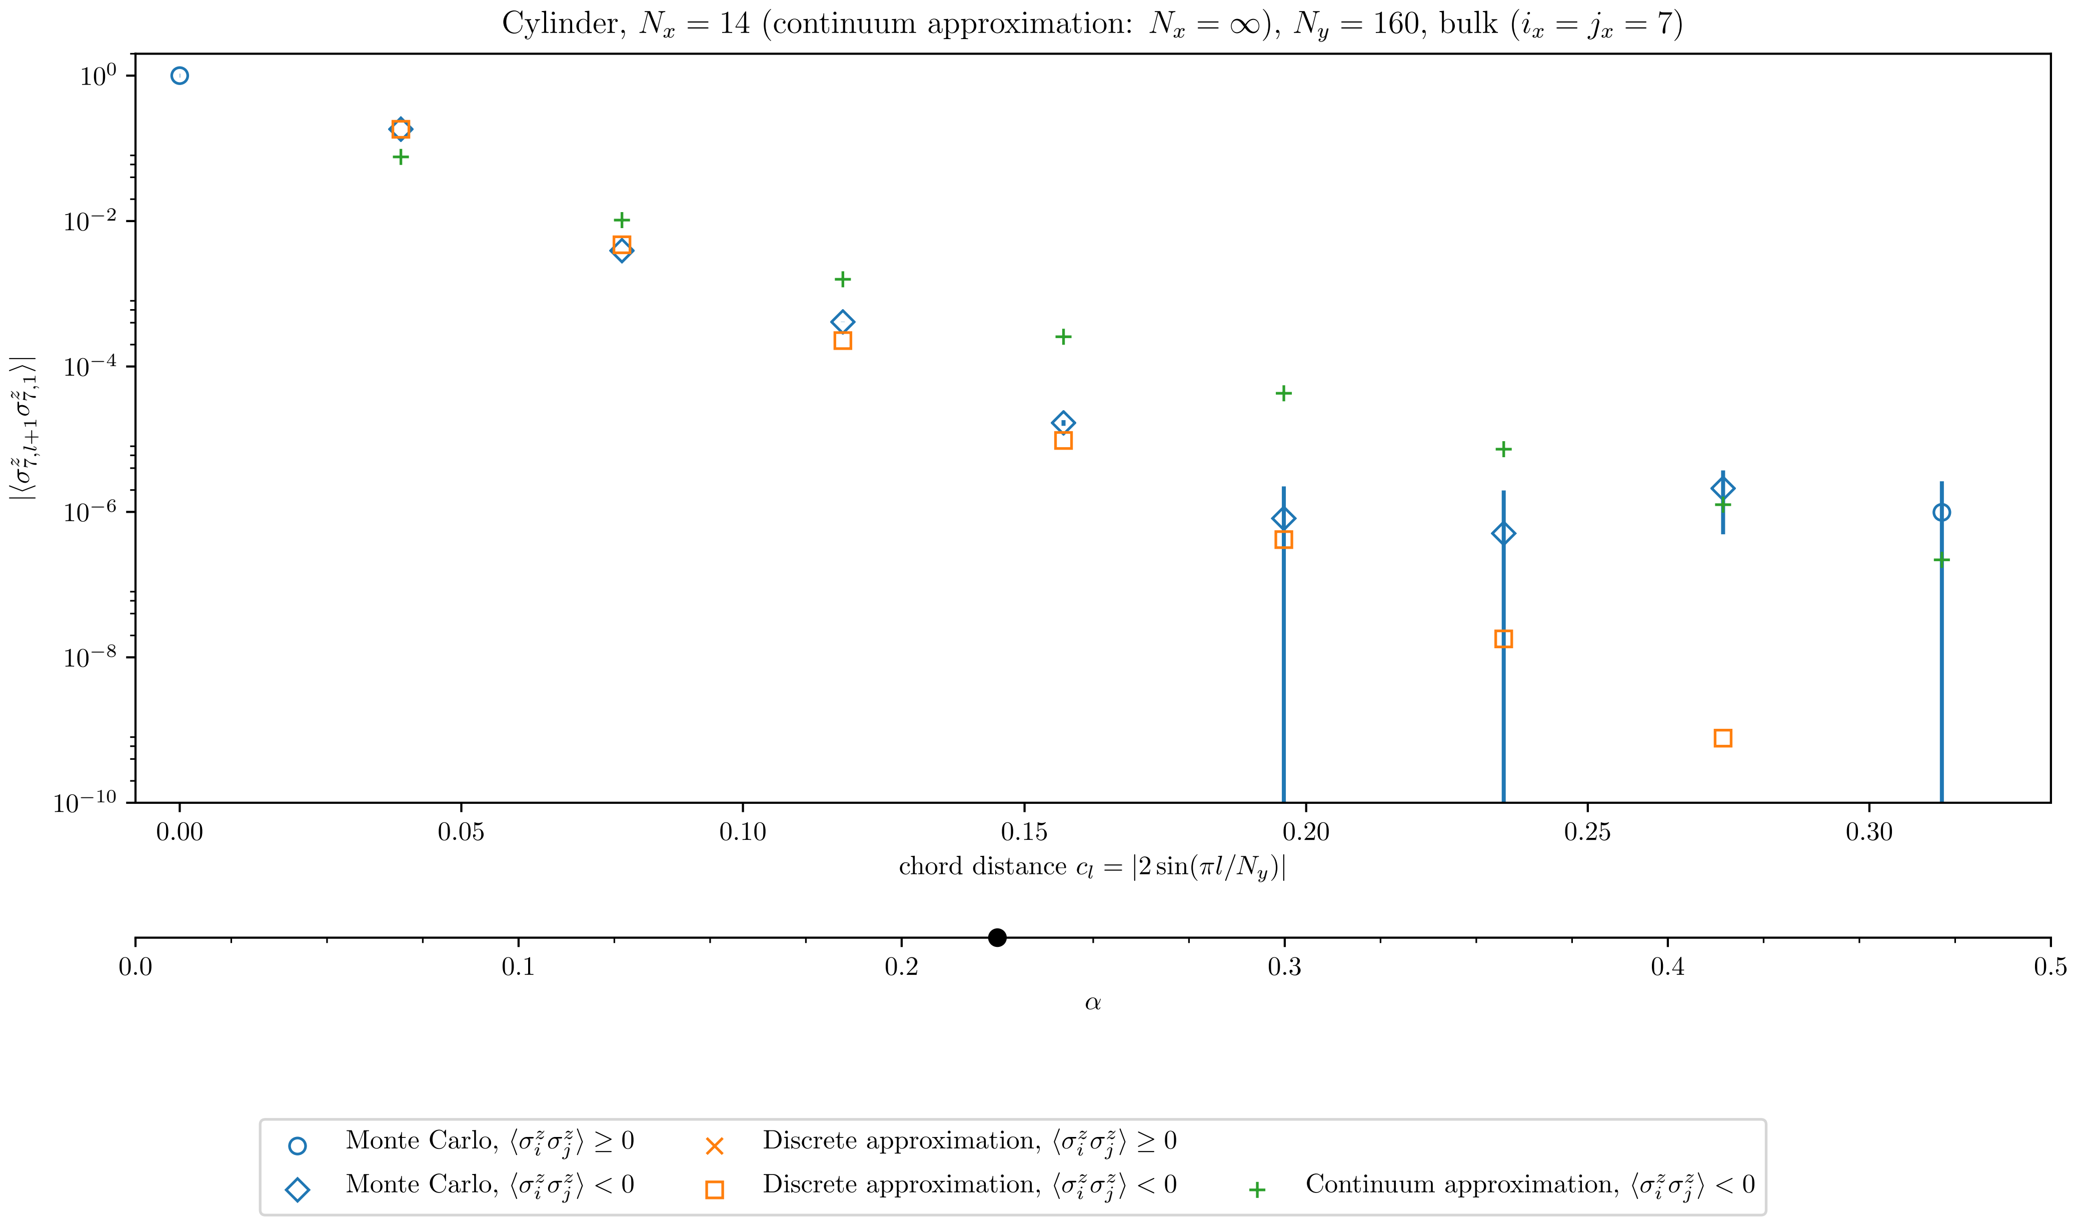

Cylinder, $N_x = 14$ (continuum approximation: $N_x = \infty$), $N_y = 160$, bulk ($i_x = j_x = 7$)
$|\langle \sigma^z_{7,l+1} \sigma^z_{7,1} \rangle|$
$10^0$
$10^{-2}$
$10^{-4}$
$10^{-6}$
$10^{-8}$
$10^{-10}$
0.00
0.05
0.10
0.15
0.20
0.25
0.30
chord distance $c_l = |2 \sin(\pi l / N_y)|$
0.0
0.1
0.2
0.3
0.4
0.5
$\alpha$
Monte Carlo, $\langle \sigma^z_i \sigma^z_j \rangle \geq 0$
Monte Carlo, $\langle \sigma^z_i \sigma^z_j \rangle < 0$
Discrete approximation, $\langle \sigma^z_i \sigma^z_j \rangle \geq 0$
Discrete approximation, $\langle \sigma^z_i \sigma^z_j \rangle < 0$
Continuum approximation, $\langle \sigma^z_i \sigma^z_j \rangle < 0$

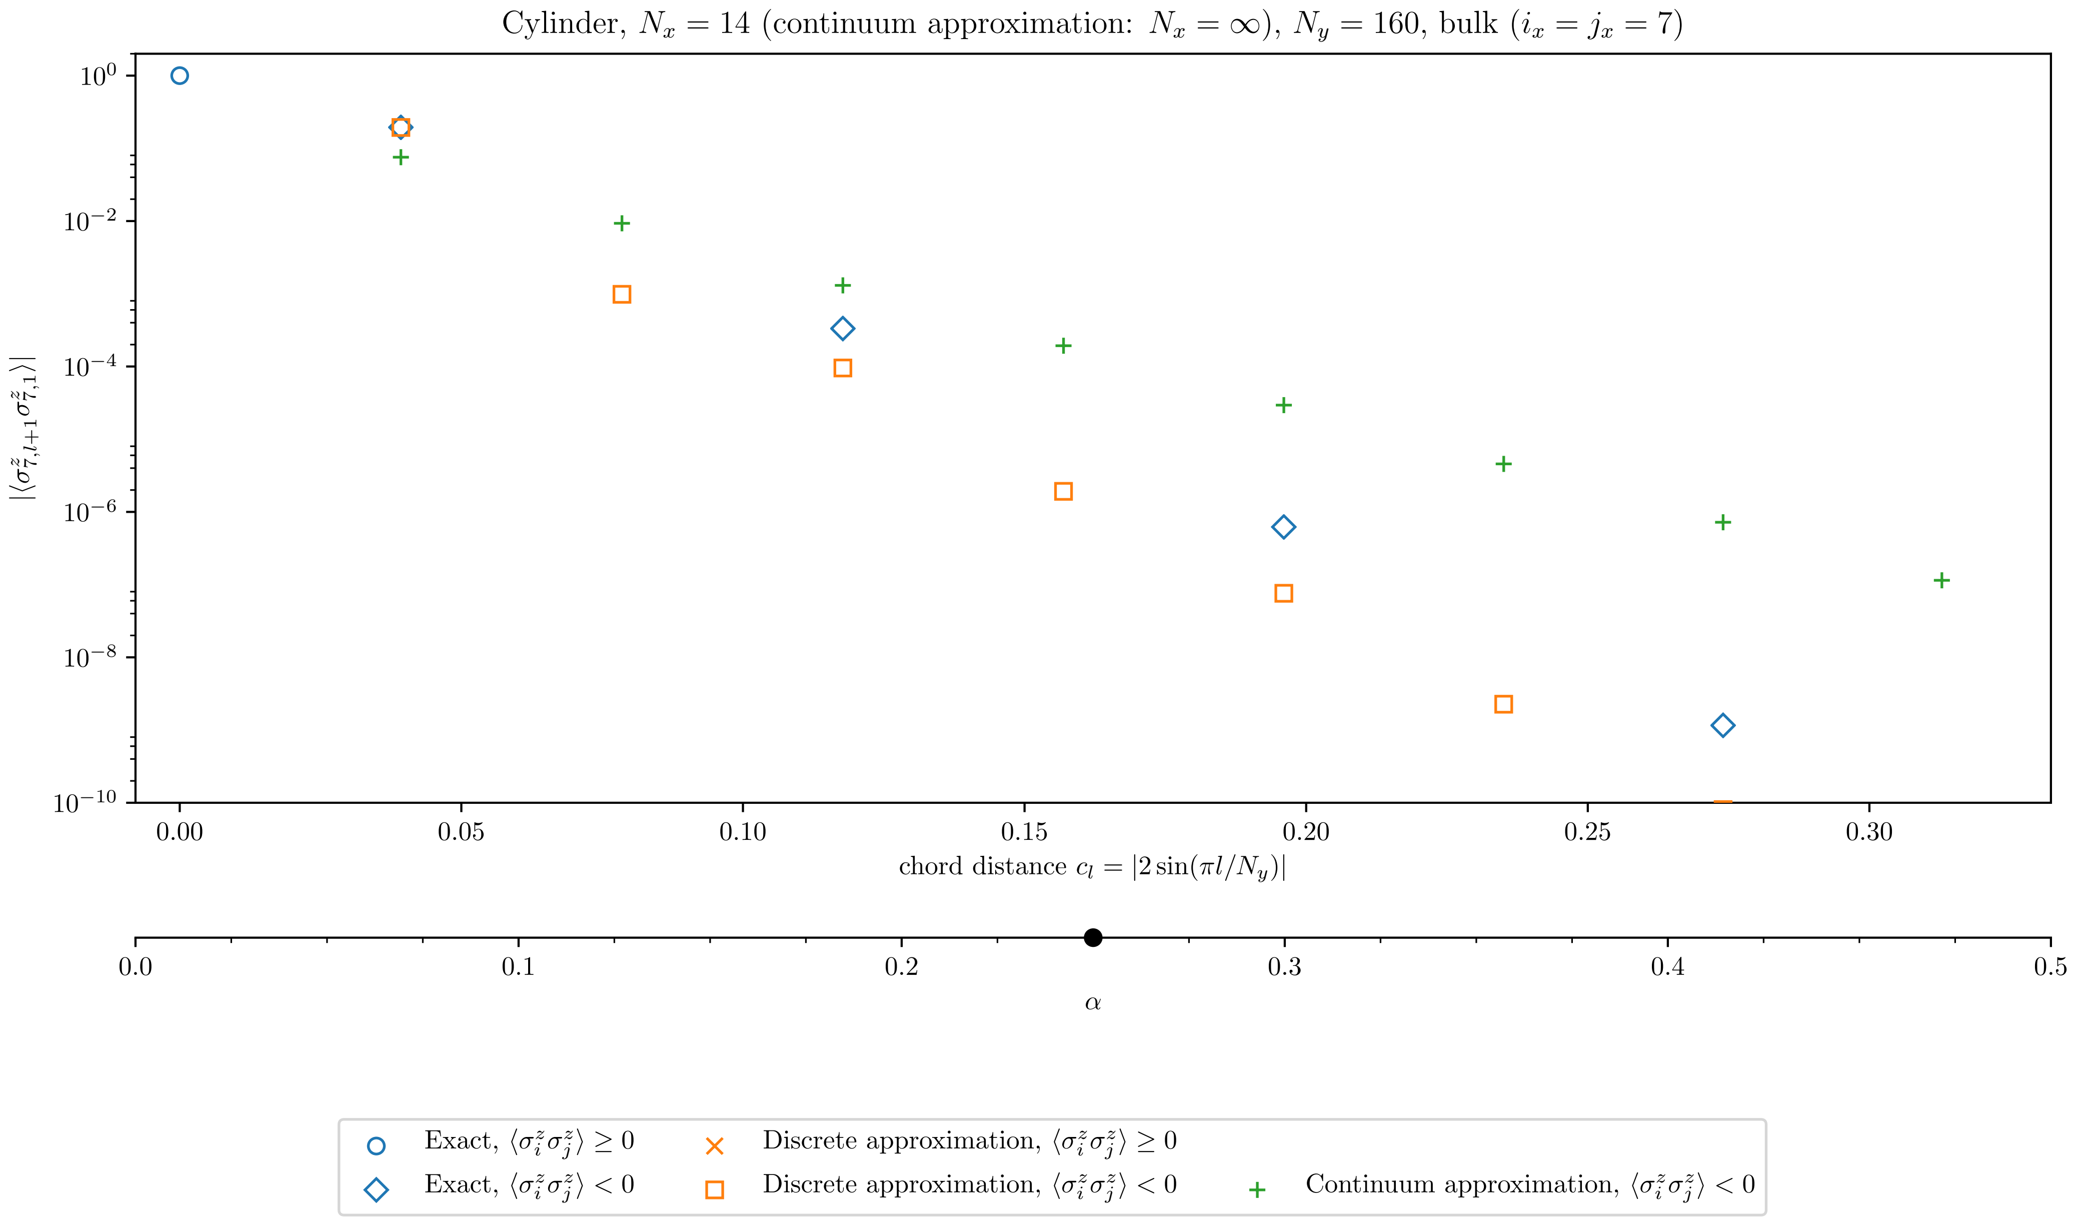

Cylinder, $N_x = 14$ (continuum approximation: $N_x = \infty$), $N_y = 160$, bulk ($i_x = j_x = 7$)
$|\langle \sigma^z_{7,l+1} \sigma^z_{7,1} \rangle|$
$10^0$
$10^{-2}$
$10^{-4}$
$10^{-6}$
$10^{-8}$
$10^{-10}$
0.00
0.05
0.10
0.15
0.20
0.25
0.30
chord distance $c_l = |2 \sin(\pi l / N_y)|$
0.0
0.1
0.2
0.3
0.4
0.5
$\alpha$
Exact, $\langle \sigma^z_i \sigma^z_j \rangle \geq 0$
Exact, $\langle \sigma^z_i \sigma^z_j \rangle < 0$
Discrete approximation, $\langle \sigma^z_i \sigma^z_j \rangle \geq 0$
Discrete approximation, $\langle \sigma^z_i \sigma^z_j \rangle < 0$
Continuum approximation, $\langle \sigma^z_i \sigma^z_j \rangle < 0$

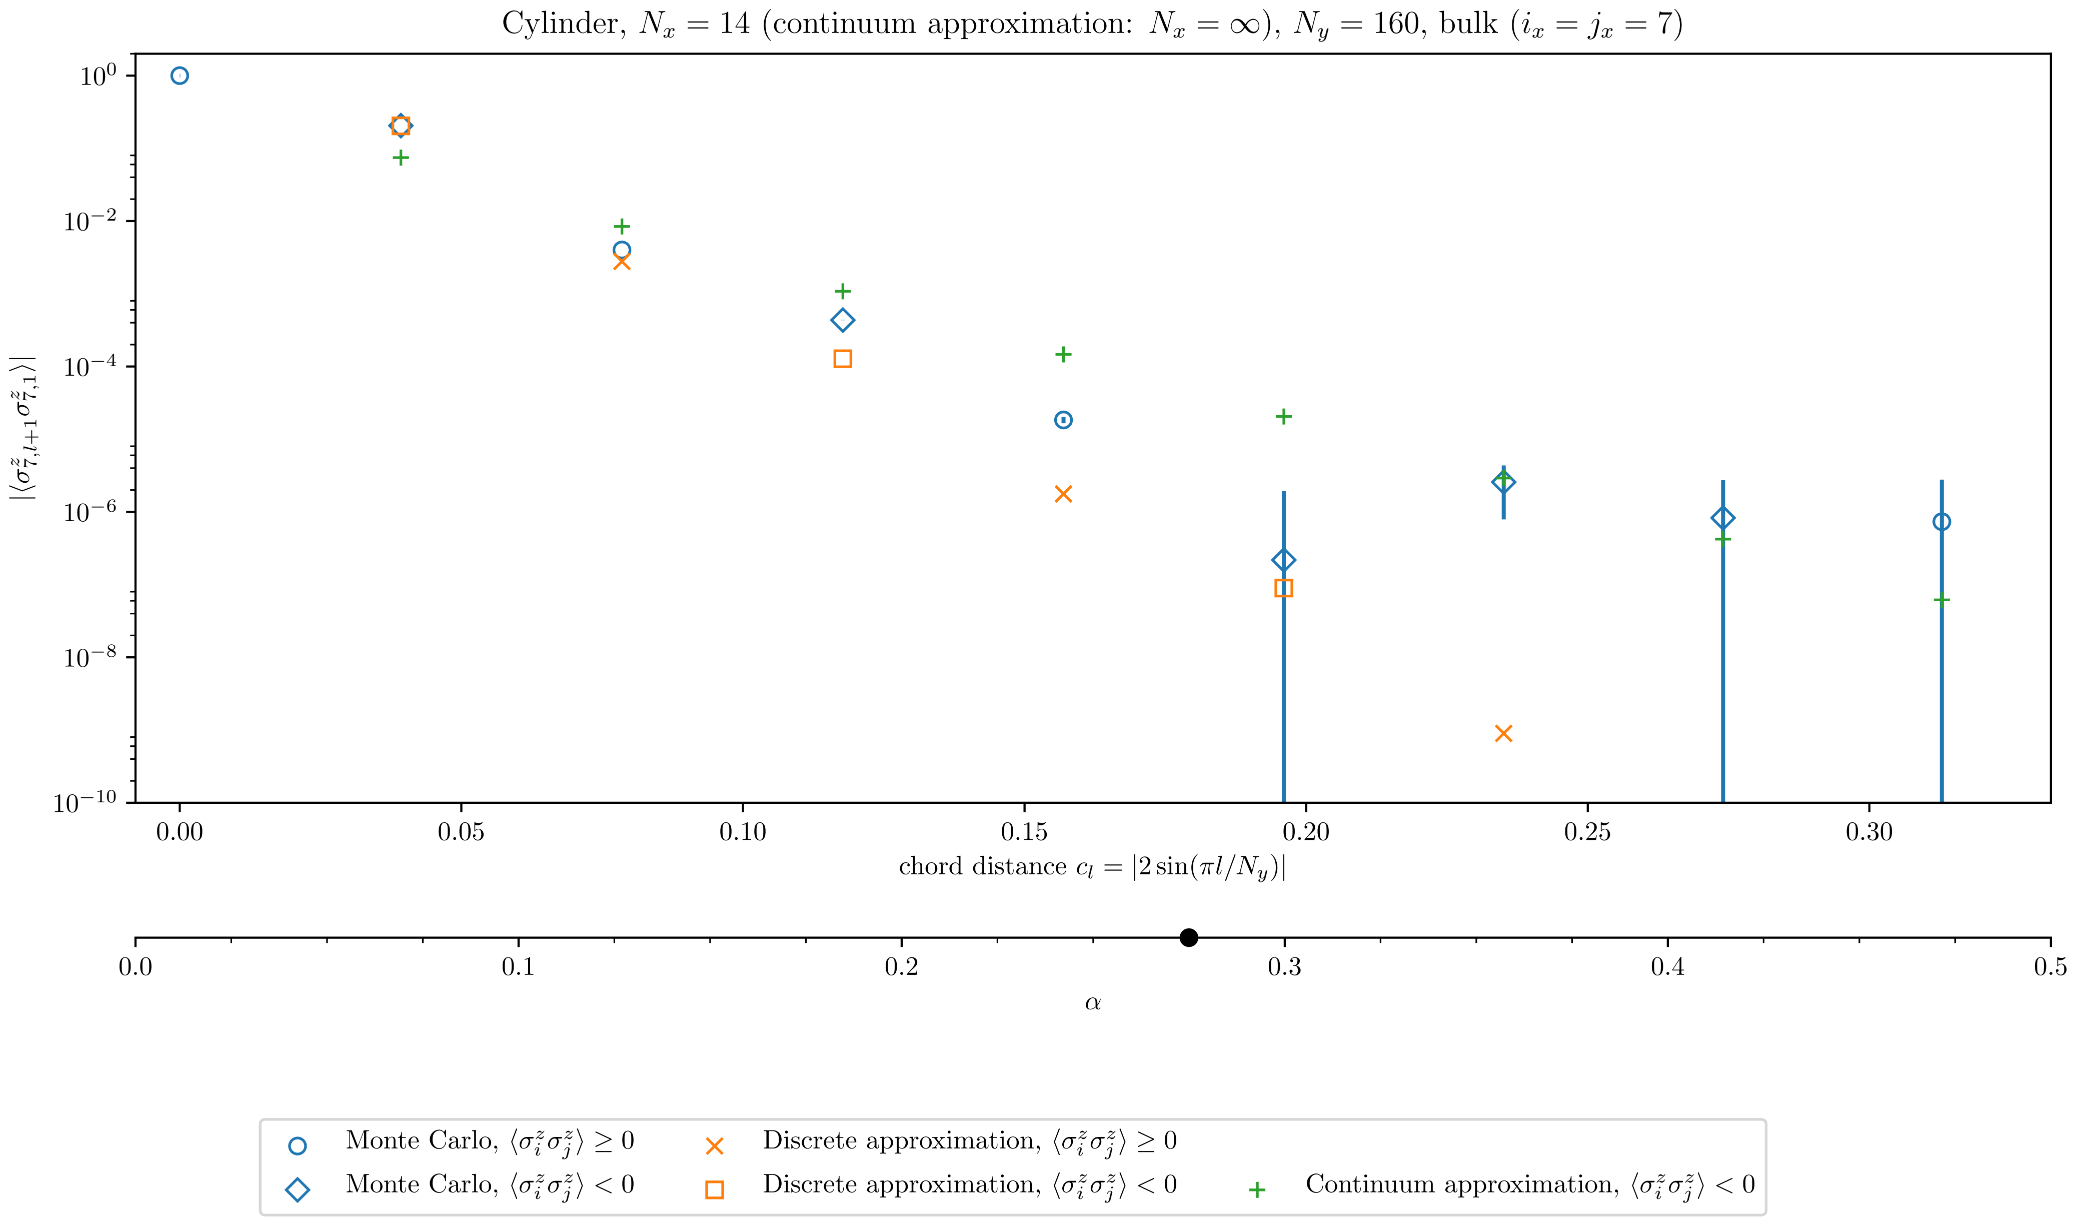

Cylinder, $N_x = 14$ (continuum approximation: $N_x = \infty$), $N_y = 160$, bulk ($i_x = j_x = 7$)
$|\langle \sigma^z_{7,l+1} \sigma^z_{7,1} \rangle|$
$10^0$
$10^{-2}$
$10^{-4}$
$10^{-6}$
$10^{-8}$
$10^{-10}$
0.00
0.05
0.10
0.15
0.20
0.25
0.30
chord distance $c_l = |2\sin(\pi l/N_y)|$
0.0
0.1
0.2
0.3
0.4
0.5
$\alpha$
Monte Carlo, $\langle \sigma^z_i \sigma^z_j \rangle \geq 0$
Monte Carlo, $\langle \sigma^z_i \sigma^z_j \rangle < 0$
Discrete approximation, $\langle \sigma^z_i \sigma^z_j \rangle \geq 0$
Discrete approximation, $\langle \sigma^z_i \sigma^z_j \rangle < 0$
Continuum approximation, $\langle \sigma^z_i \sigma^z_j \rangle < 0$

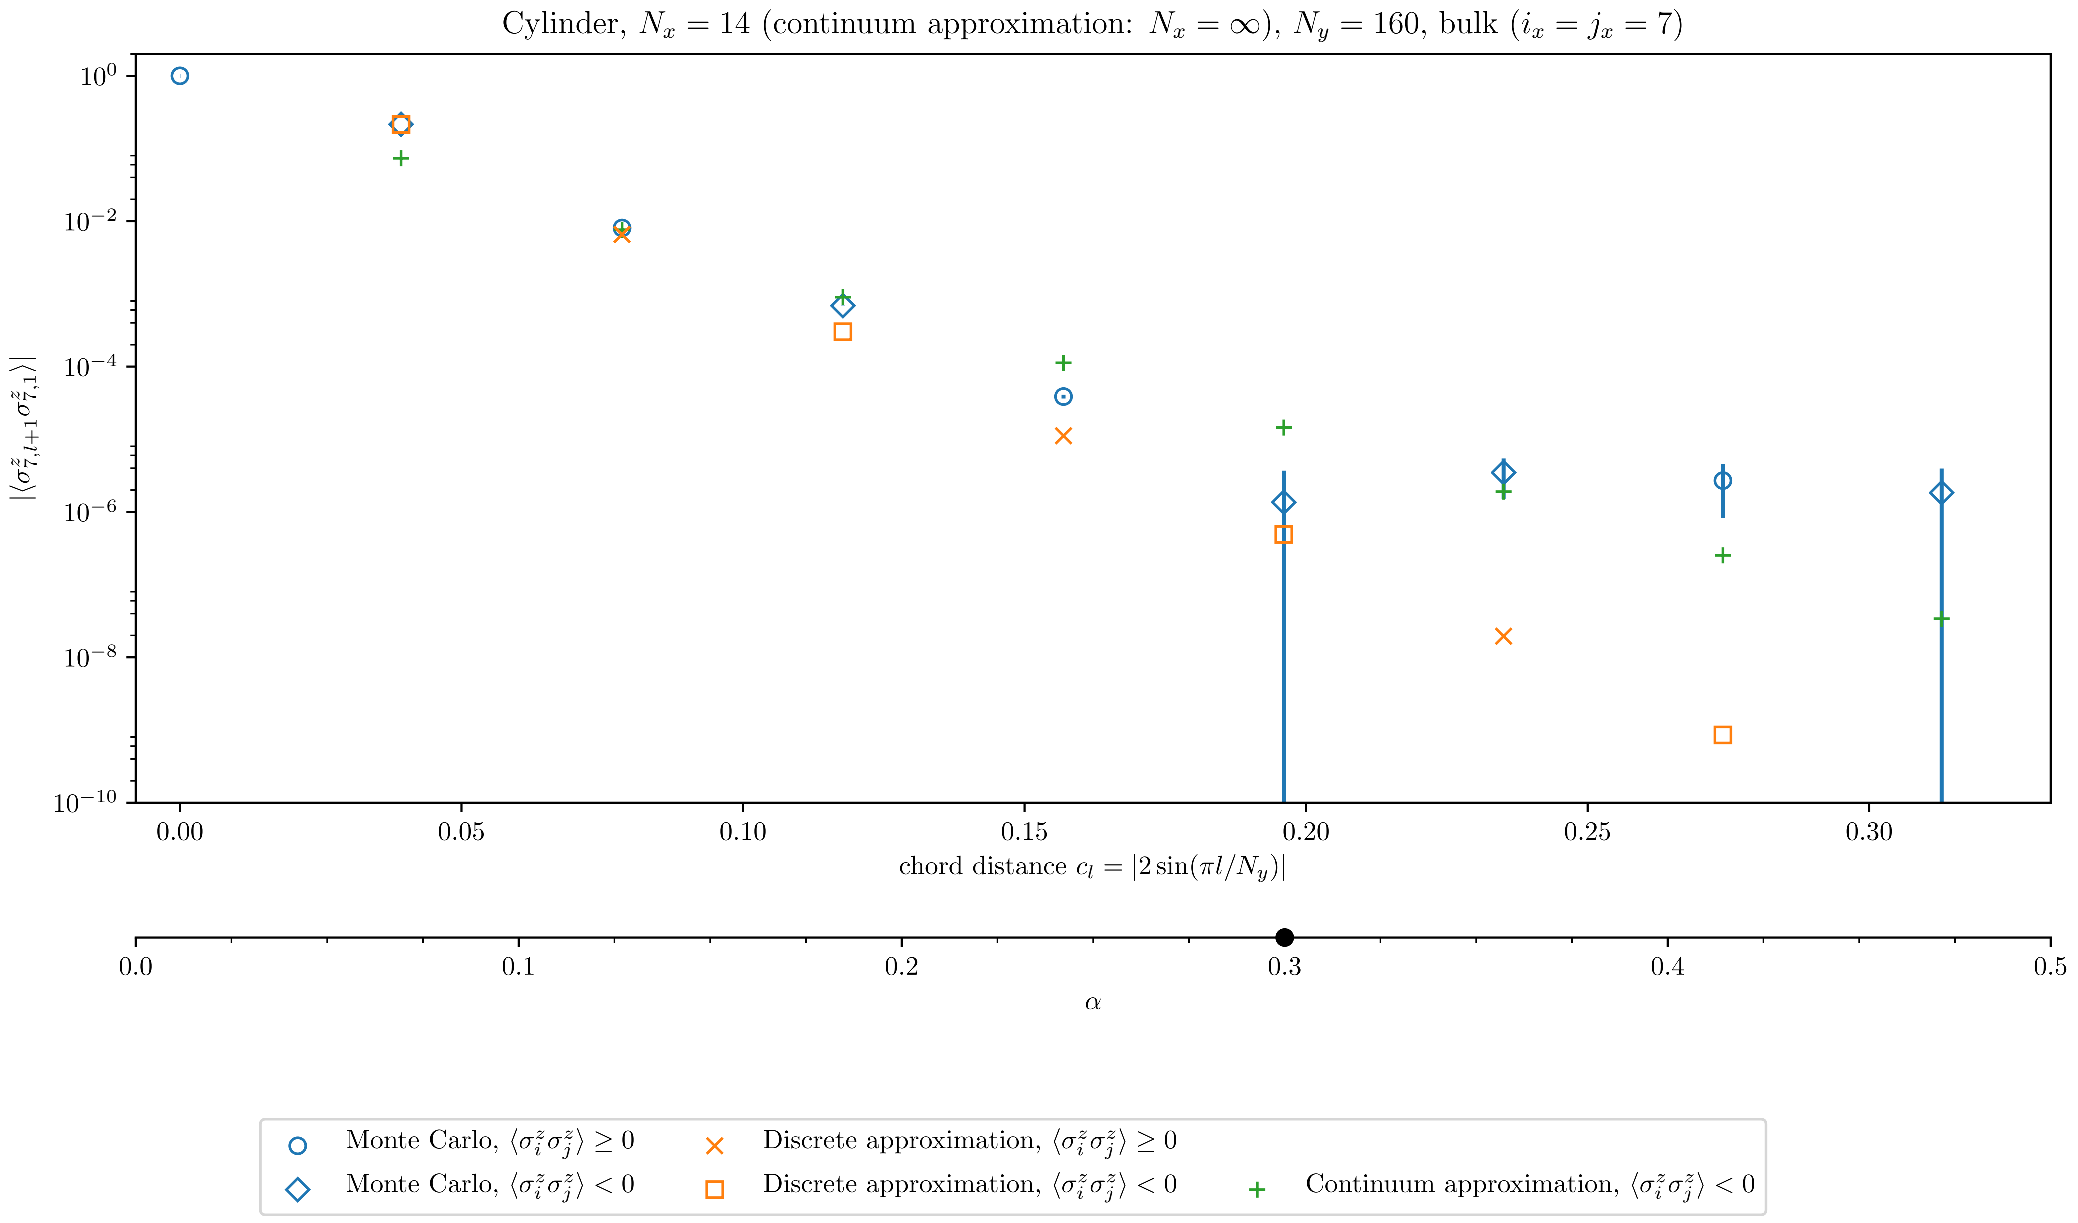

Cylinder, $N_x = 14$ (continuum approximation: $N_x = \infty$), $N_y = 160$, bulk ($i_x = j_x = 7$)
$|\langle \sigma^z_{7,l+1} \sigma^z_{7,1} \rangle|$
$10^0$
$10^{-2}$
$10^{-4}$
$10^{-6}$
$10^{-8}$
$10^{-10}$
0.00
0.05
0.10
0.15
0.20
0.25
0.30
chord distance $c_l = |2 \sin(\pi l / N_y)|$
0.0
0.1
0.2
0.3
0.4
0.5
$\alpha$
Monte Carlo, $\langle \sigma^z_i \sigma^z_j \rangle \geq 0$
Monte Carlo, $\langle \sigma^z_i \sigma^z_j \rangle < 0$
Discrete approximation, $\langle \sigma^z_i \sigma^z_j \rangle \geq 0$
Discrete approximation, $\langle \sigma^z_i \sigma^z_j \rangle < 0$
Continuum approximation, $\langle \sigma^z_i \sigma^z_j \rangle < 0$

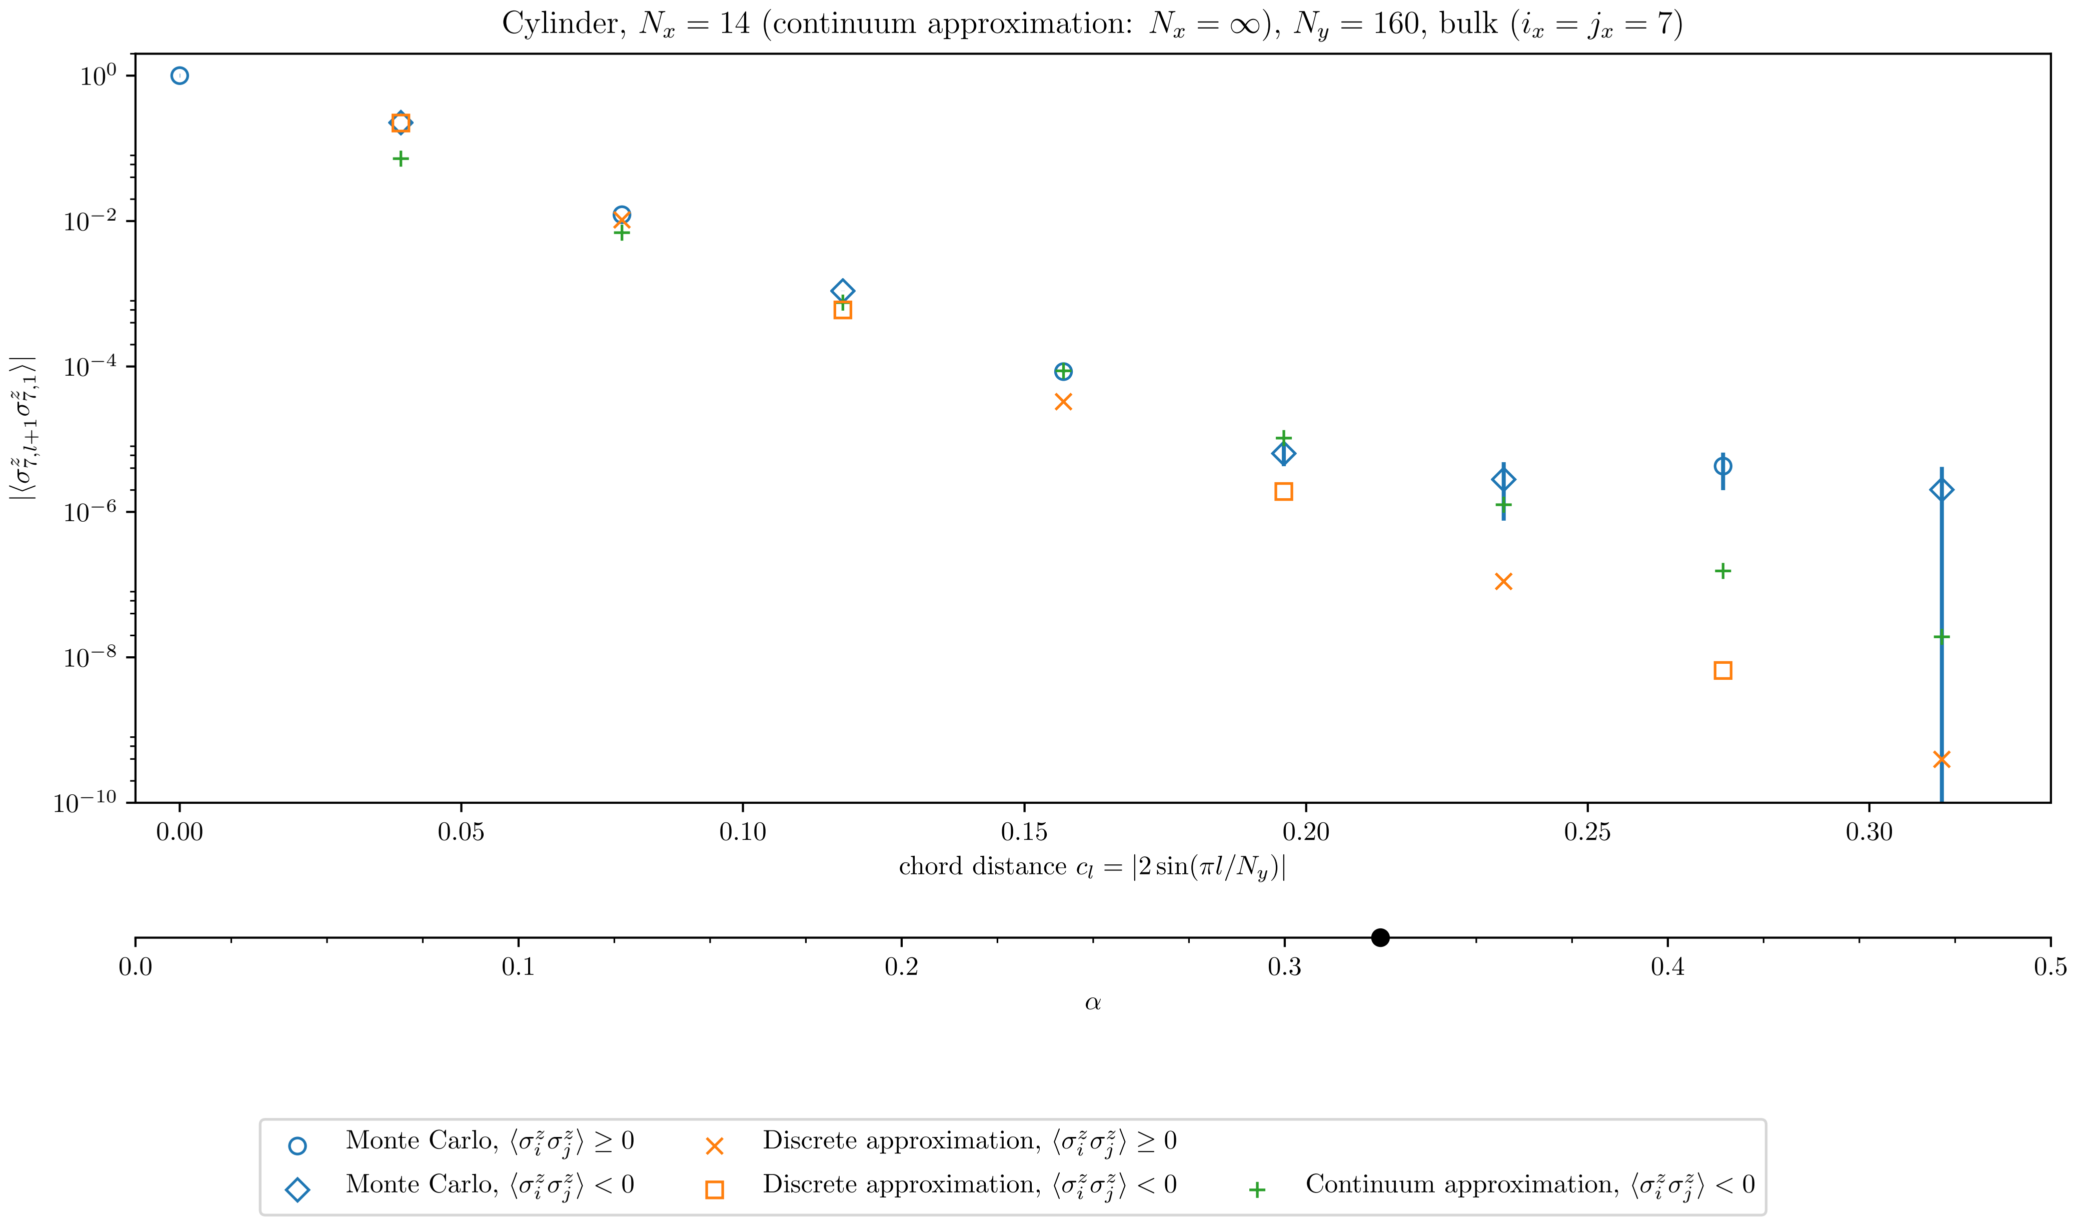

Cylinder, $N_x = 14$ (continuum approximation: $N_x = \infty$), $N_y = 160$, bulk ($i_x = j_x = 7$)
$|\langle \sigma^z_{7,l+1} \sigma^z_{7,1} \rangle|$
$10^0$
$10^{-2}$
$10^{-4}$
$10^{-6}$
$10^{-8}$
$10^{-10}$
0.00
0.05
0.10
0.15
0.20
0.25
0.30
chord distance $c_l = |2\sin(\pi l/N_y)|$
0.0
0.1
0.2
0.3
0.4
0.5
$\alpha$
Monte Carlo, $\langle \sigma^z_i \sigma^z_j \rangle \geq 0$
Monte Carlo, $\langle \sigma^z_i \sigma^z_j \rangle < 0$
Discrete approximation, $\langle \sigma^z_i \sigma^z_j \rangle \geq 0$
Discrete approximation, $\langle \sigma^z_i \sigma^z_j \rangle < 0$
Continuum approximation, $\langle \sigma^z_i \sigma^z_j \rangle < 0$

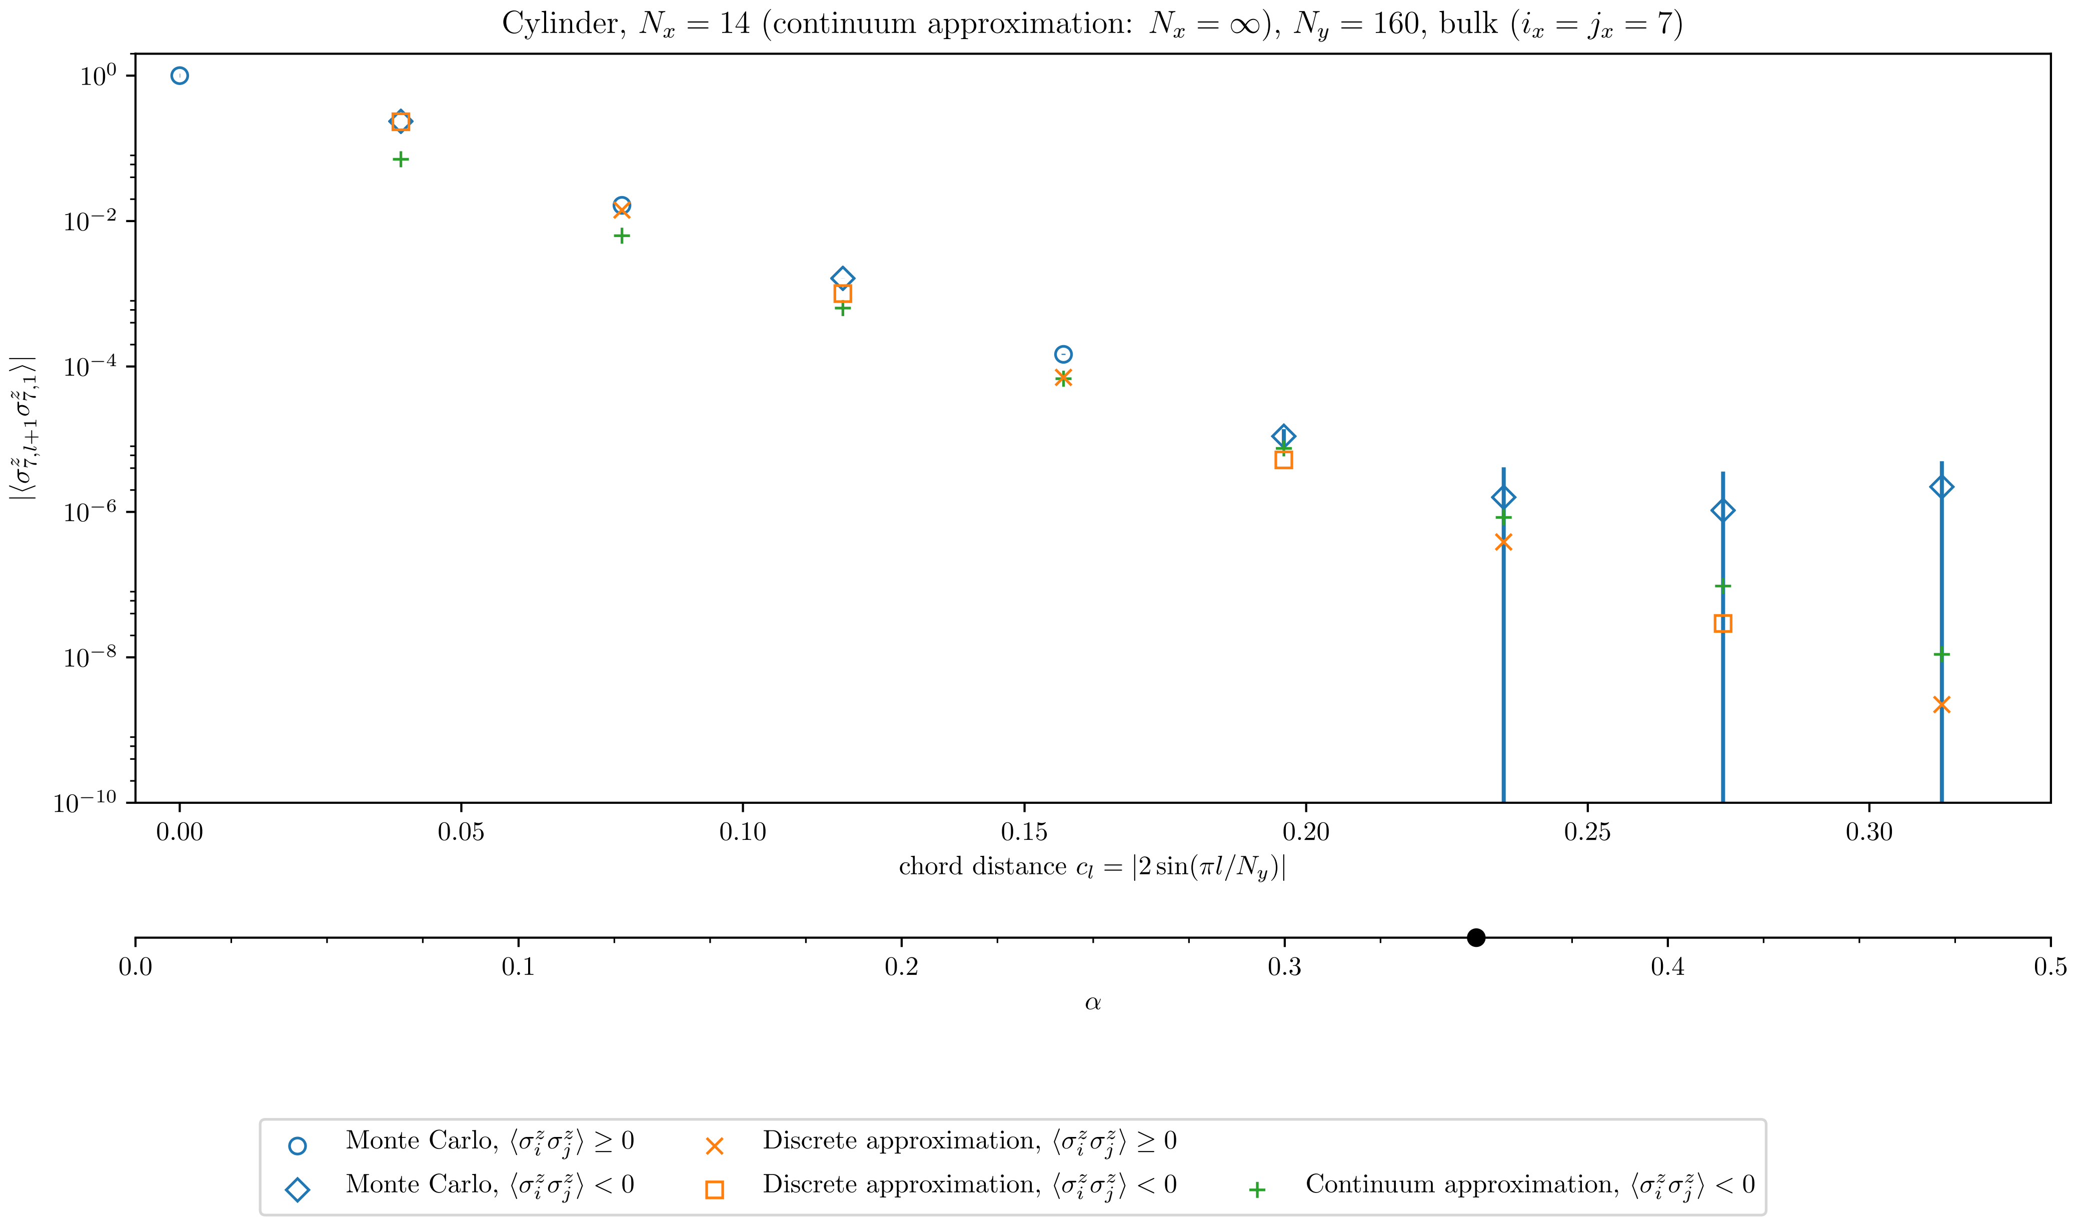
Cylinder, $N_x = 14$ (continuum approximation: $N_x = \infty$), $N_y = 160$, bulk ($i_x = j_x = 7$)
$|\langle \sigma^z_{7,l+1} \sigma^z_{7,1} \rangle|$
$10^0$
$10^{-2}$
$10^{-4}$
$10^{-6}$
$10^{-8}$
$10^{-10}$
0.00
0.05
0.10
0.15
0.20
0.25
0.30
chord distance $c_l = |2\sin(\pi l / N_y)|$
0.0
0.1
0.2
0.3
0.4
0.5
$\alpha$
Monte Carlo, $\langle \sigma^z_i \sigma^z_j \rangle \geq 0$
Monte Carlo, $\langle \sigma^z_i \sigma^z_j \rangle < 0$
Discrete approximation, $\langle \sigma^z_i \sigma^z_j \rangle \geq 0$
Discrete approximation, $\langle \sigma^z_i \sigma^z_j \rangle < 0$
Continuum approximation, $\langle \sigma^z_i \sigma^z_j \rangle < 0$

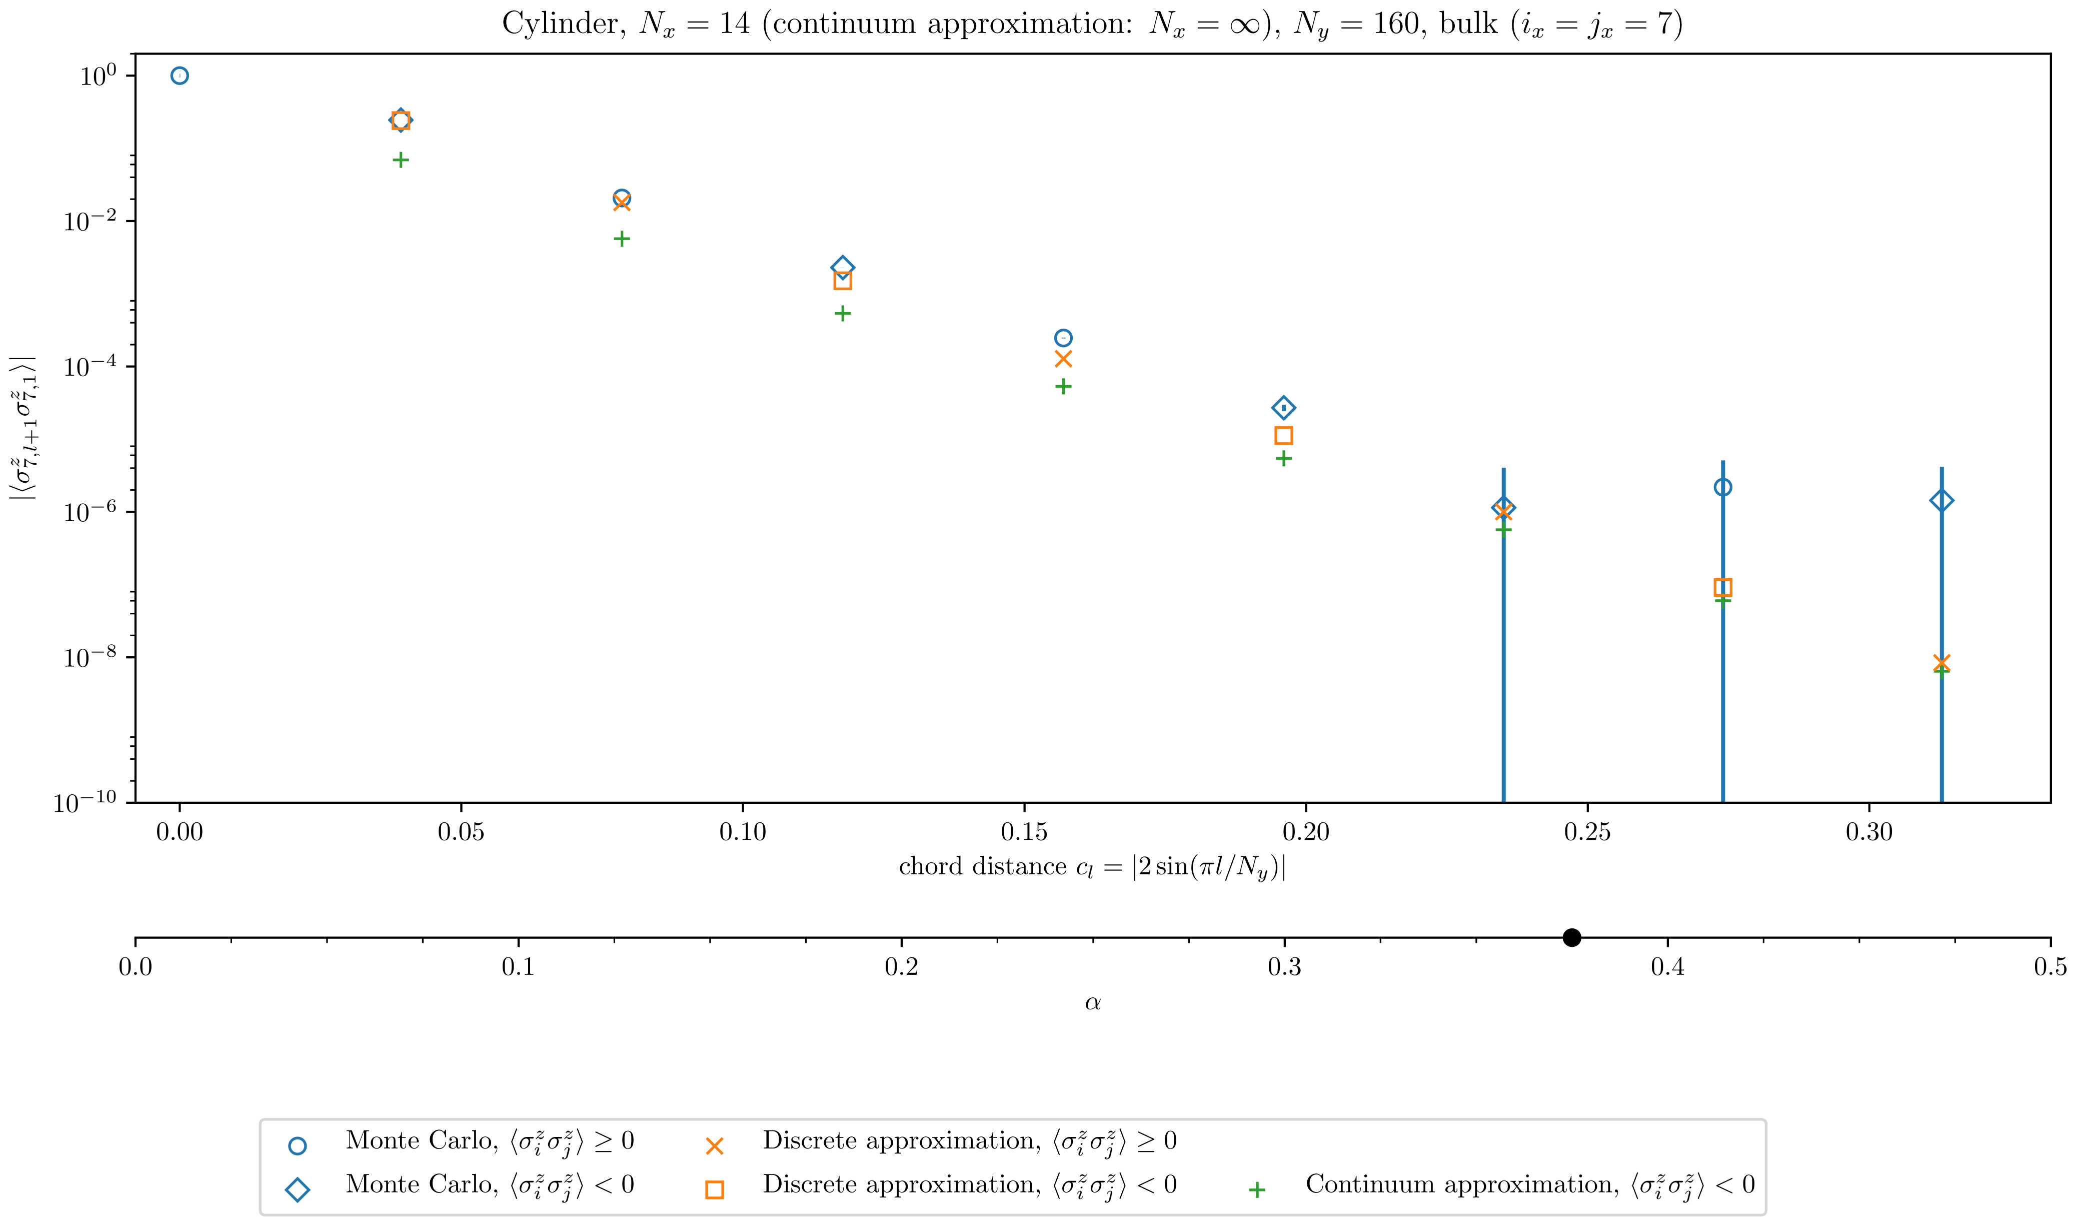

Cylinder, $N_x = 14$ (continuum approximation: $N_x = \infty$), $N_y = 160$, bulk ($i_x = j_x = 7$)
$|\langle \sigma^z_{7,l+1} \sigma^z_{7,1} \rangle|$
$10^0$
$10^{-2}$
$10^{-4}$
$10^{-6}$
$10^{-8}$
$10^{-10}$
0.00
0.05
0.10
0.15
0.20
0.25
0.30
chord distance $c_l = |2\sin(\pi l/N_y)|$
0.0
0.1
0.2
0.3
0.4
0.5
$\alpha$
Monte Carlo, $\langle \sigma^z_i \sigma^z_j \rangle \geq 0$
Monte Carlo, $\langle \sigma^z_i \sigma^z_j \rangle < 0$
Discrete approximation, $\langle \sigma^z_i \sigma^z_j \rangle \geq 0$
Discrete approximation, $\langle \sigma^z_i \sigma^z_j \rangle < 0$
Continuum approximation, $\langle \sigma^z_i \sigma^z_j \rangle < 0$

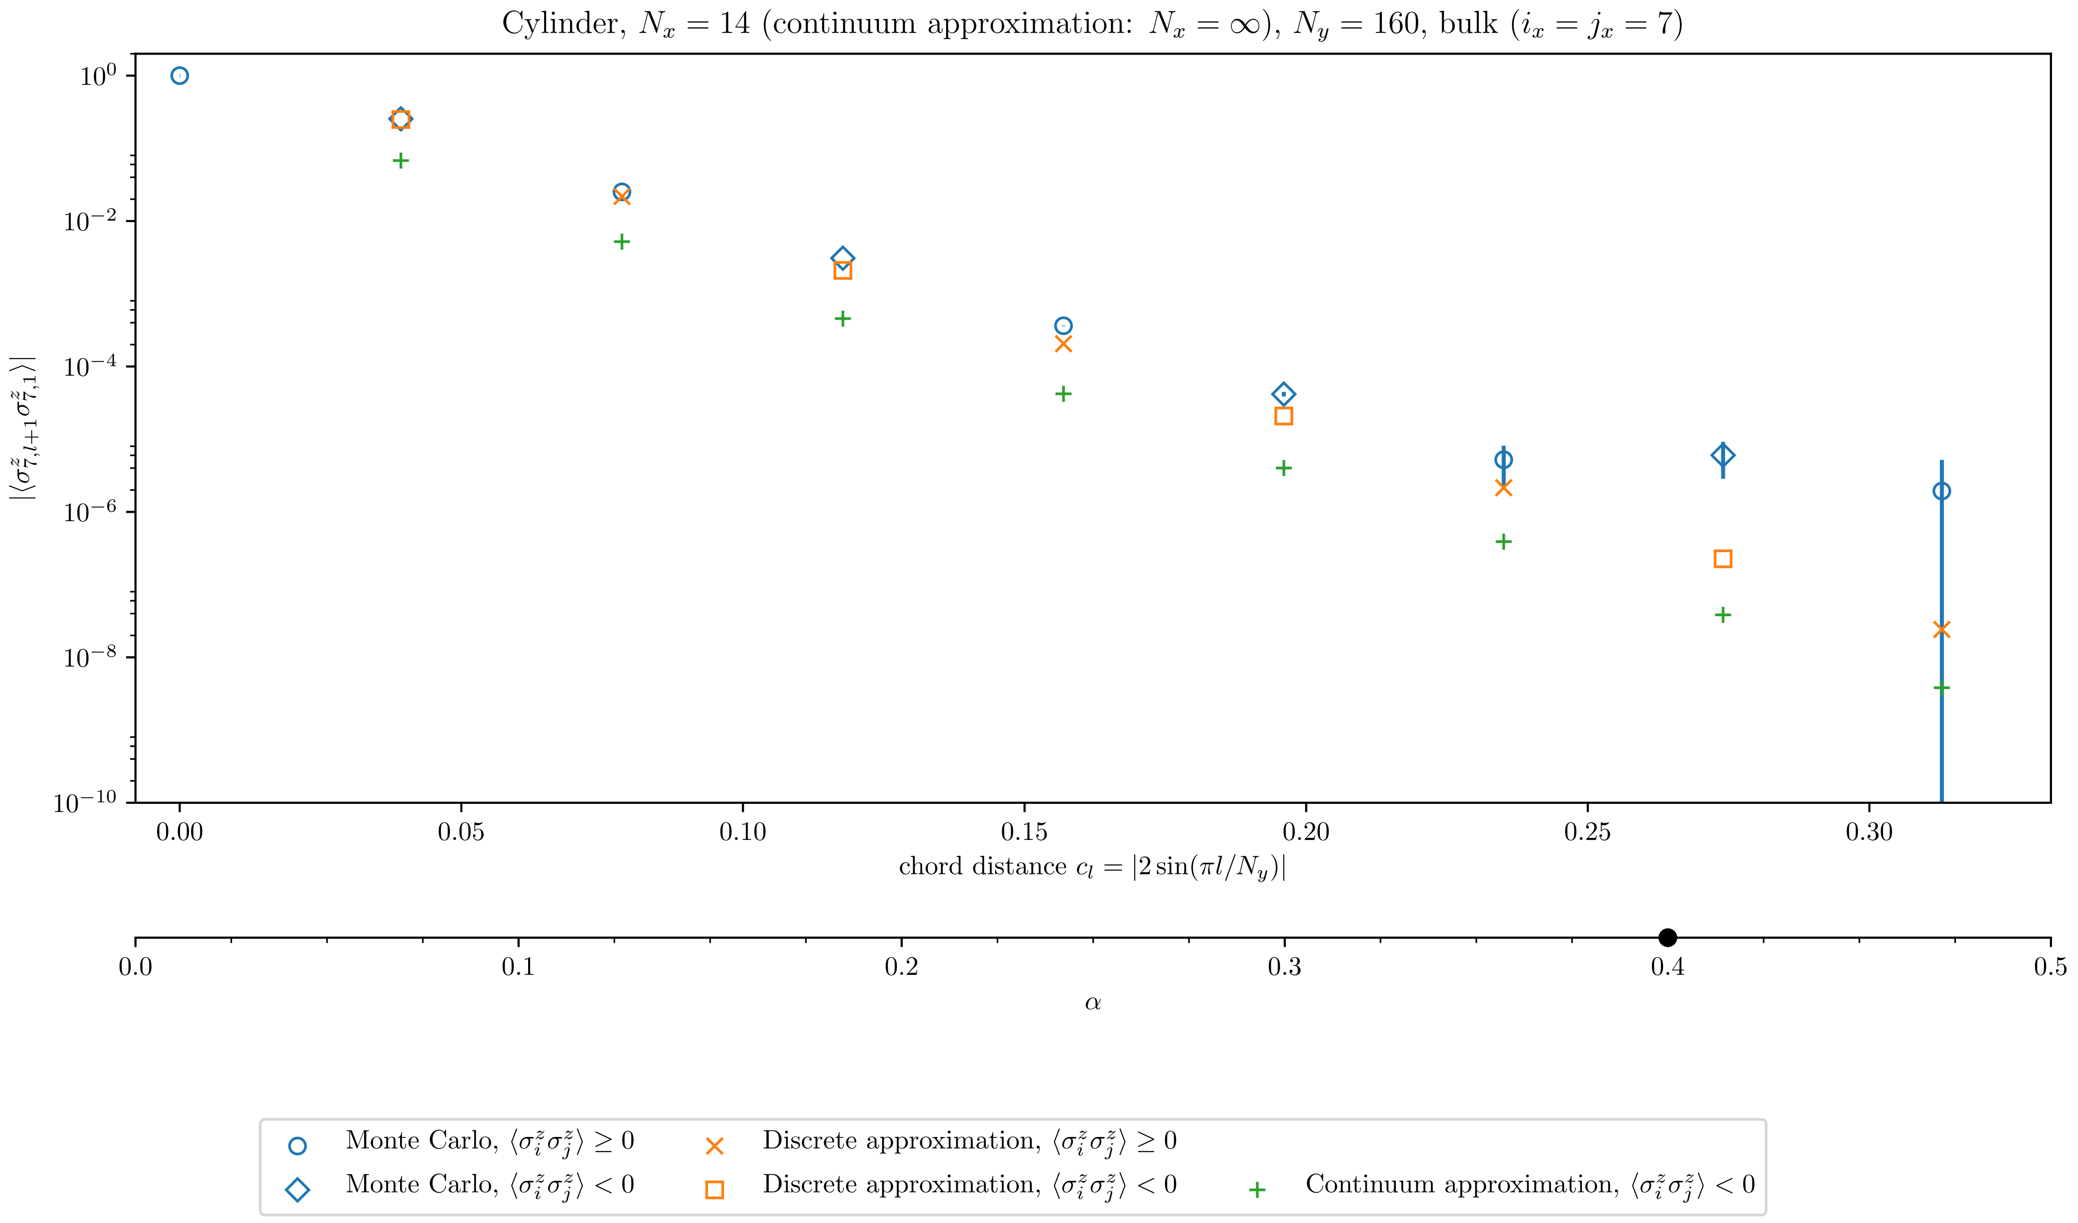
Cylinder, $N_x = 14$ (continuum approximation: $N_x = \infty$), $N_y = 160$, bulk ($i_x = j_x = 7$)
$|\langle \sigma^z_{7,l+1} \sigma^z_{7,1} \rangle|$
$10^0$
$10^{-2}$
$10^{-4}$
$10^{-6}$
$10^{-8}$
$10^{-10}$
0.00
0.05
0.10
0.15
0.20
0.25
0.30
chord distance $c_l = |2\sin(\pi l / N_y)|$
0.0
0.1
0.2
0.3
0.4
0.5
$\alpha$
Monte Carlo, $\langle \sigma^z_i \sigma^z_j \rangle \geq 0$
Monte Carlo, $\langle \sigma^z_i \sigma^z_j \rangle < 0$
Discrete approximation, $\langle \sigma^z_i \sigma^z_j \rangle \geq 0$
Discrete approximation, $\langle \sigma^z_i \sigma^z_j \rangle < 0$
Continuum approximation, $\langle \sigma^z_i \sigma^z_j \rangle < 0$

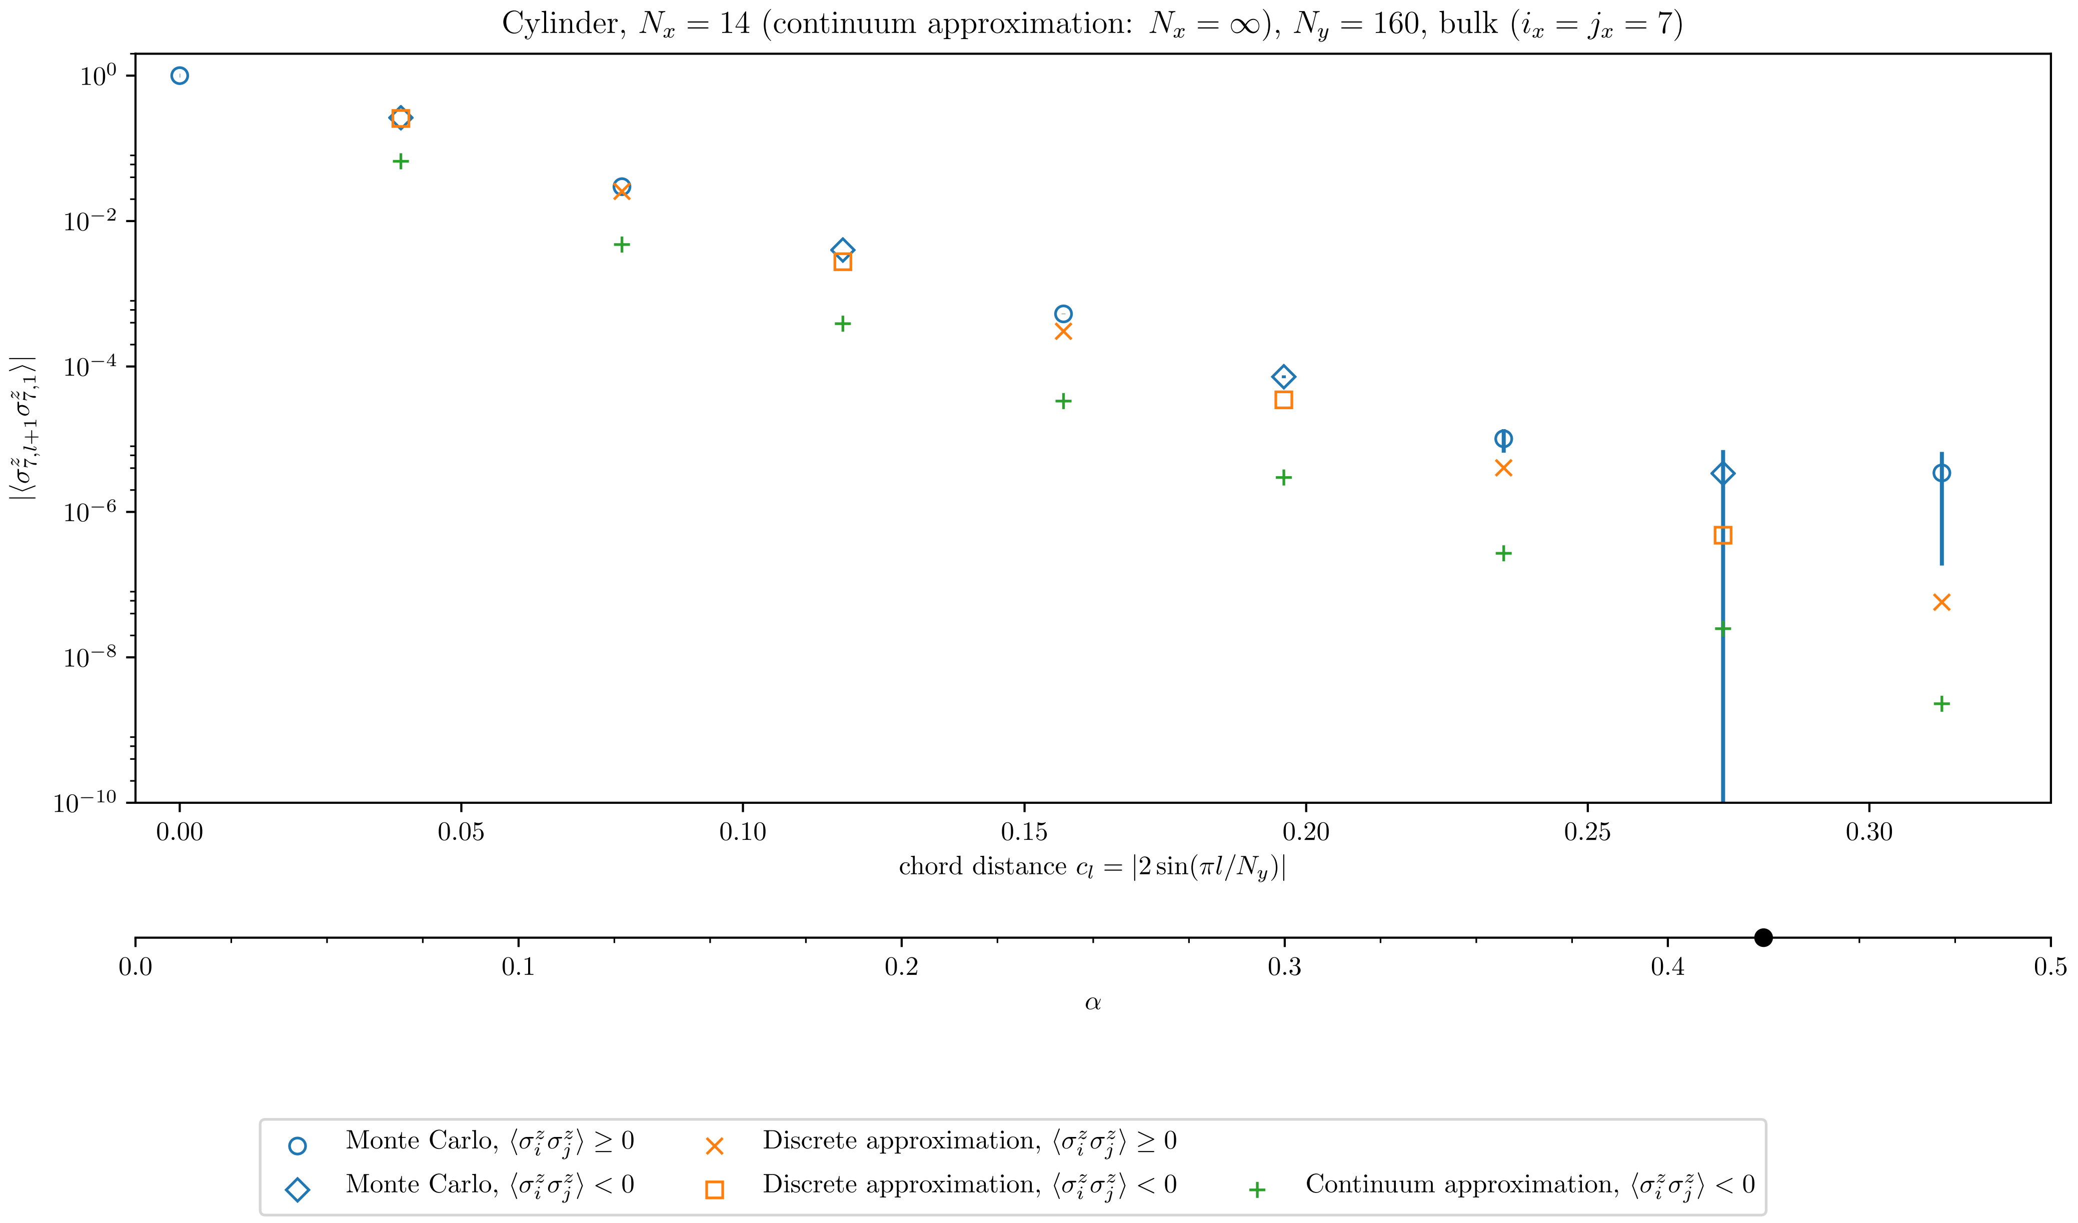

Cylinder, $N_x = 14$ (continuum approximation: $N_x = \infty$), $N_y = 160$, bulk ($i_x = j_x = 7$)
$|\langle \sigma^z_{7,l+1} \sigma^z_{7,1} \rangle|$
$10^{0}$
$10^{-2}$
$10^{-4}$
$10^{-6}$
$10^{-8}$
$10^{-10}$
0.00
0.05
0.10
0.15
0.20
0.25
0.30
chord distance $c_l = |2 \sin(\pi l / N_y)|$
0.0
0.1
0.2
0.3
0.4
0.5
$\alpha$
Monte Carlo, $\langle \sigma^z_i \sigma^z_j \rangle \geq 0$
Monte Carlo, $\langle \sigma^z_i \sigma^z_j \rangle < 0$
Discrete approximation, $\langle \sigma^z_i \sigma^z_j \rangle \geq 0$
Discrete approximation, $\langle \sigma^z_i \sigma^z_j \rangle < 0$
Continuum approximation, $\langle \sigma^z_i \sigma^z_j \rangle < 0$

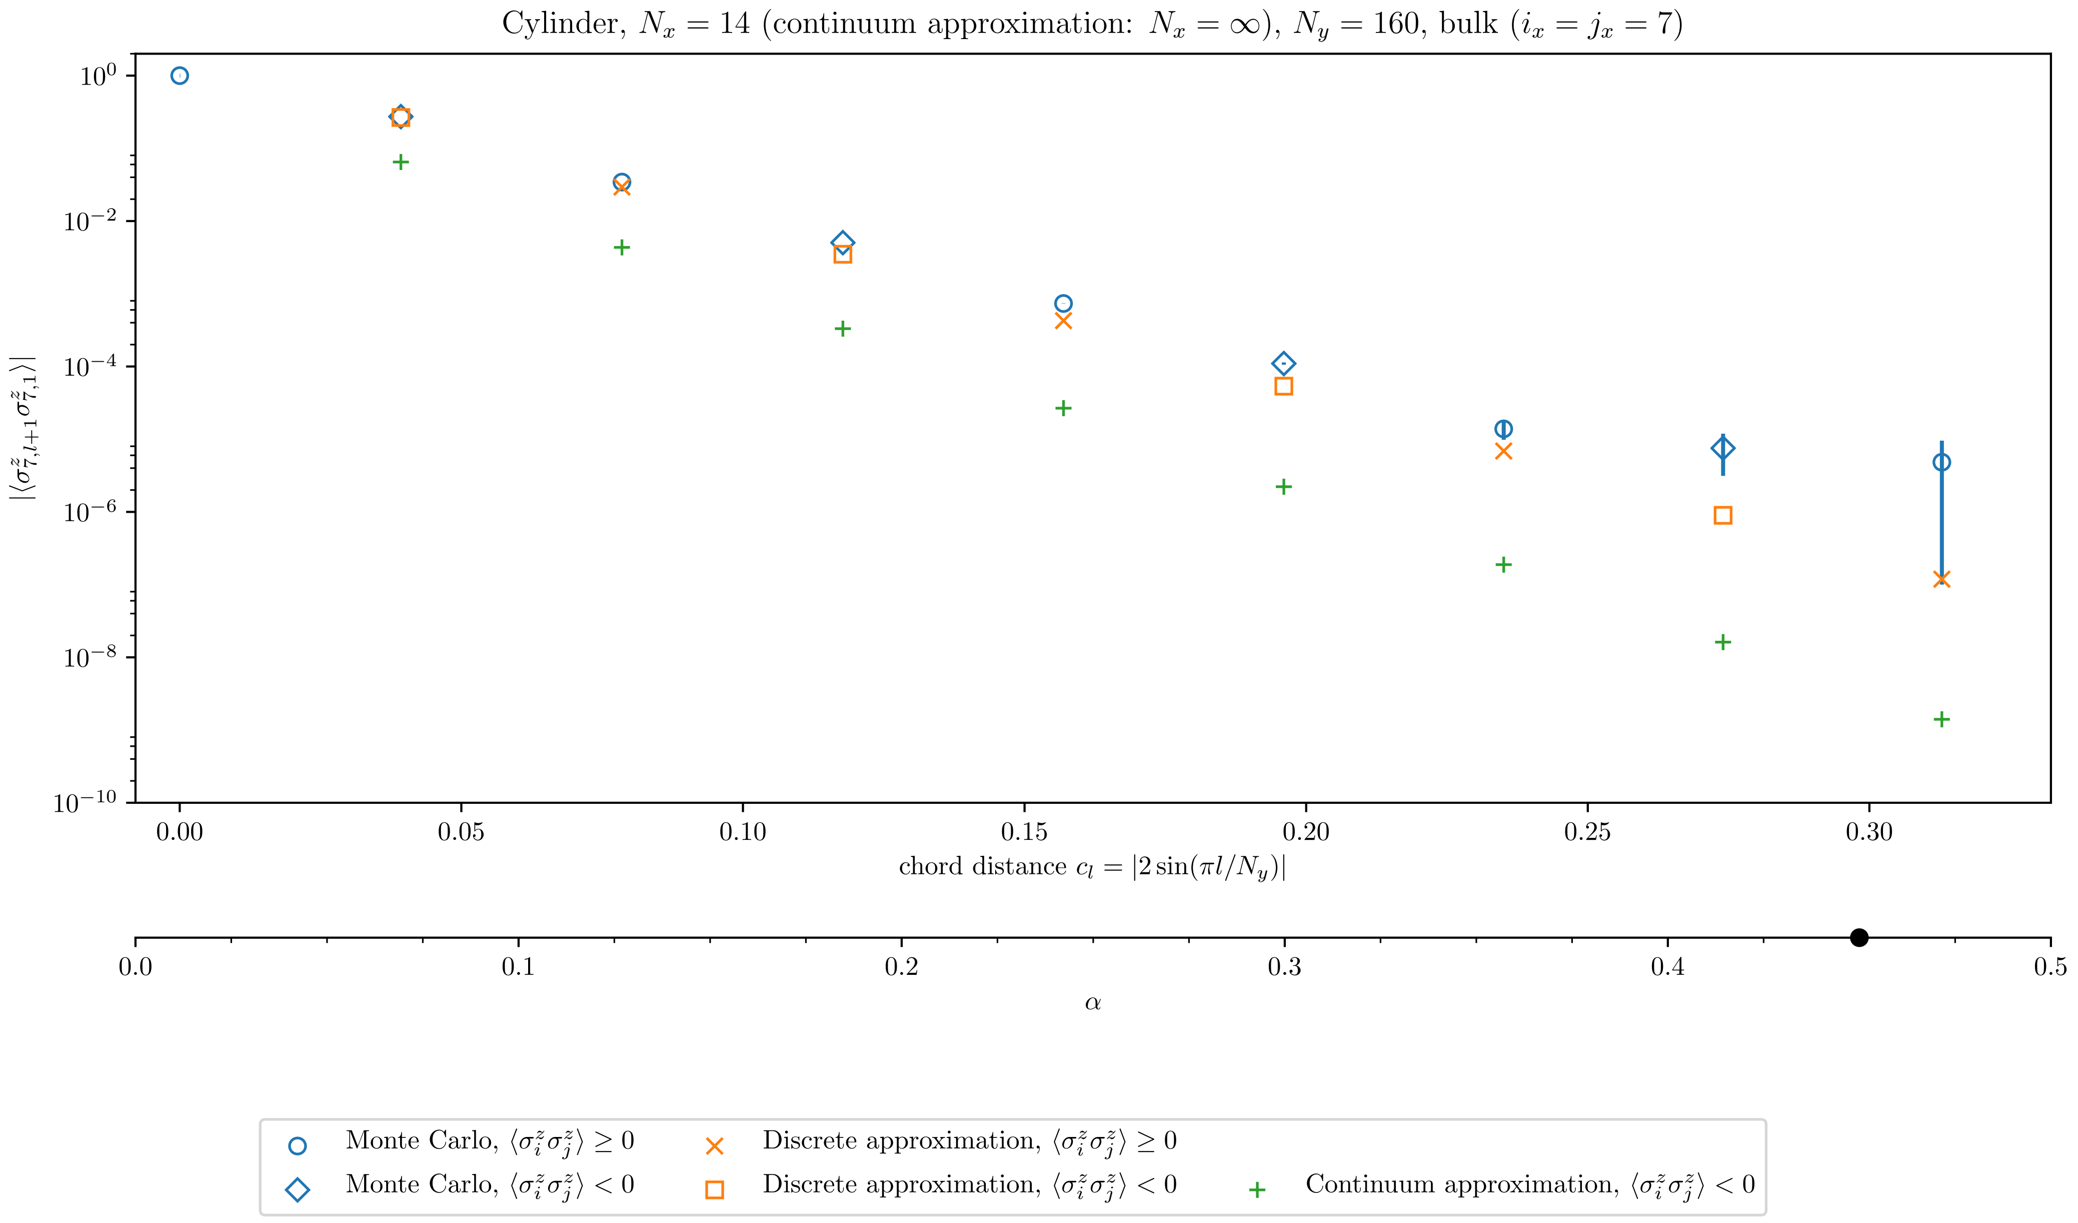

Cylinder, $N_x = 14$ (continuum approximation: $N_x = \infty$), $N_y = 160$, bulk ($i_x = j_x = 7$)
$|\langle \sigma^z_{7,l+1} \sigma^z_{7,1} \rangle|$
$10^{0}$
$10^{-2}$
$10^{-4}$
$10^{-6}$
$10^{-8}$
$10^{-10}$
0.00
0.05
0.10
0.15
0.20
0.25
0.30
chord distance $c_l = |2\sin(\pi l/N_y)|$
0.0
0.1
0.2
0.3
0.4
0.5
$\alpha$
Monte Carlo, $\langle \sigma^z_i \sigma^z_j \rangle \geq 0$
Monte Carlo, $\langle \sigma^z_i \sigma^z_j \rangle < 0$
Discrete approximation, $\langle \sigma^z_i \sigma^z_j \rangle \geq 0$
Discrete approximation, $\langle \sigma^z_i \sigma^z_j \rangle < 0$
Continuum approximation, $\langle \sigma^z_i \sigma^z_j \rangle < 0$

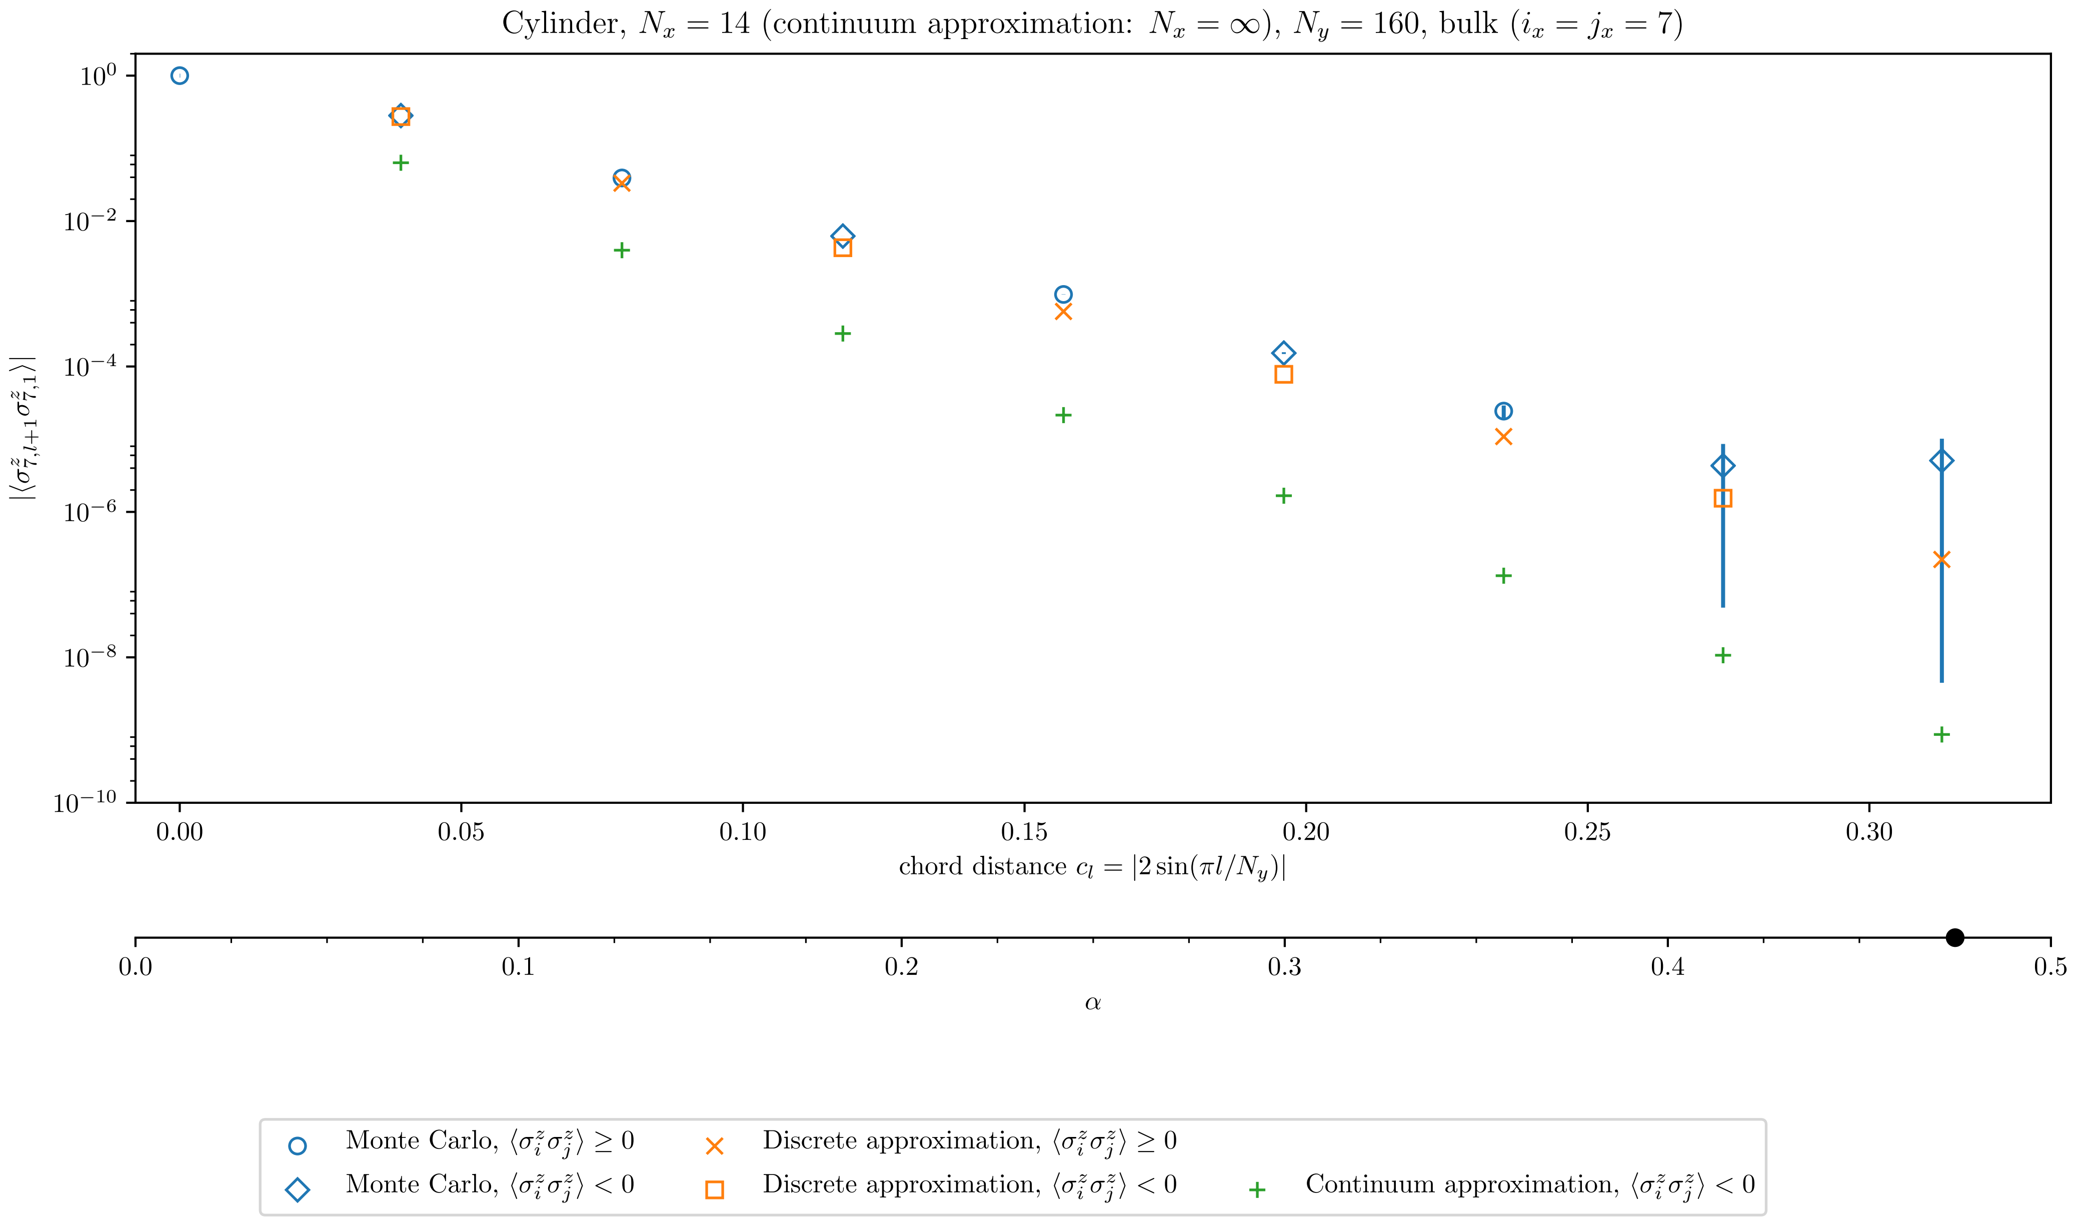
Cylinder, $N_x = 14$ (continuum approximation: $N_x = \infty$), $N_y = 160$, bulk ($i_x = j_x = 7$)
$|\langle \sigma^z_{7,l+1} \sigma^z_{7,1} \rangle|$
$10^{0}$
$10^{-2}$
$10^{-4}$
$10^{-6}$
$10^{-8}$
$10^{-10}$
0.00
0.05
0.10
0.15
0.20
0.25
0.30
chord distance $c_l = |2\sin(\pi l / N_y)|$
0.0
0.1
0.2
0.3
0.4
0.5
$\alpha$
Monte Carlo, $\langle \sigma^z_i \sigma^z_j \rangle \geq 0$
Monte Carlo, $\langle \sigma^z_i \sigma^z_j \rangle < 0$
Discrete approximation, $\langle \sigma^z_i \sigma^z_j \rangle \geq 0$
Discrete approximation, $\langle \sigma^z_i \sigma^z_j \rangle < 0$
Continuum approximation, $\langle \sigma^z_i \sigma^z_j \rangle < 0$

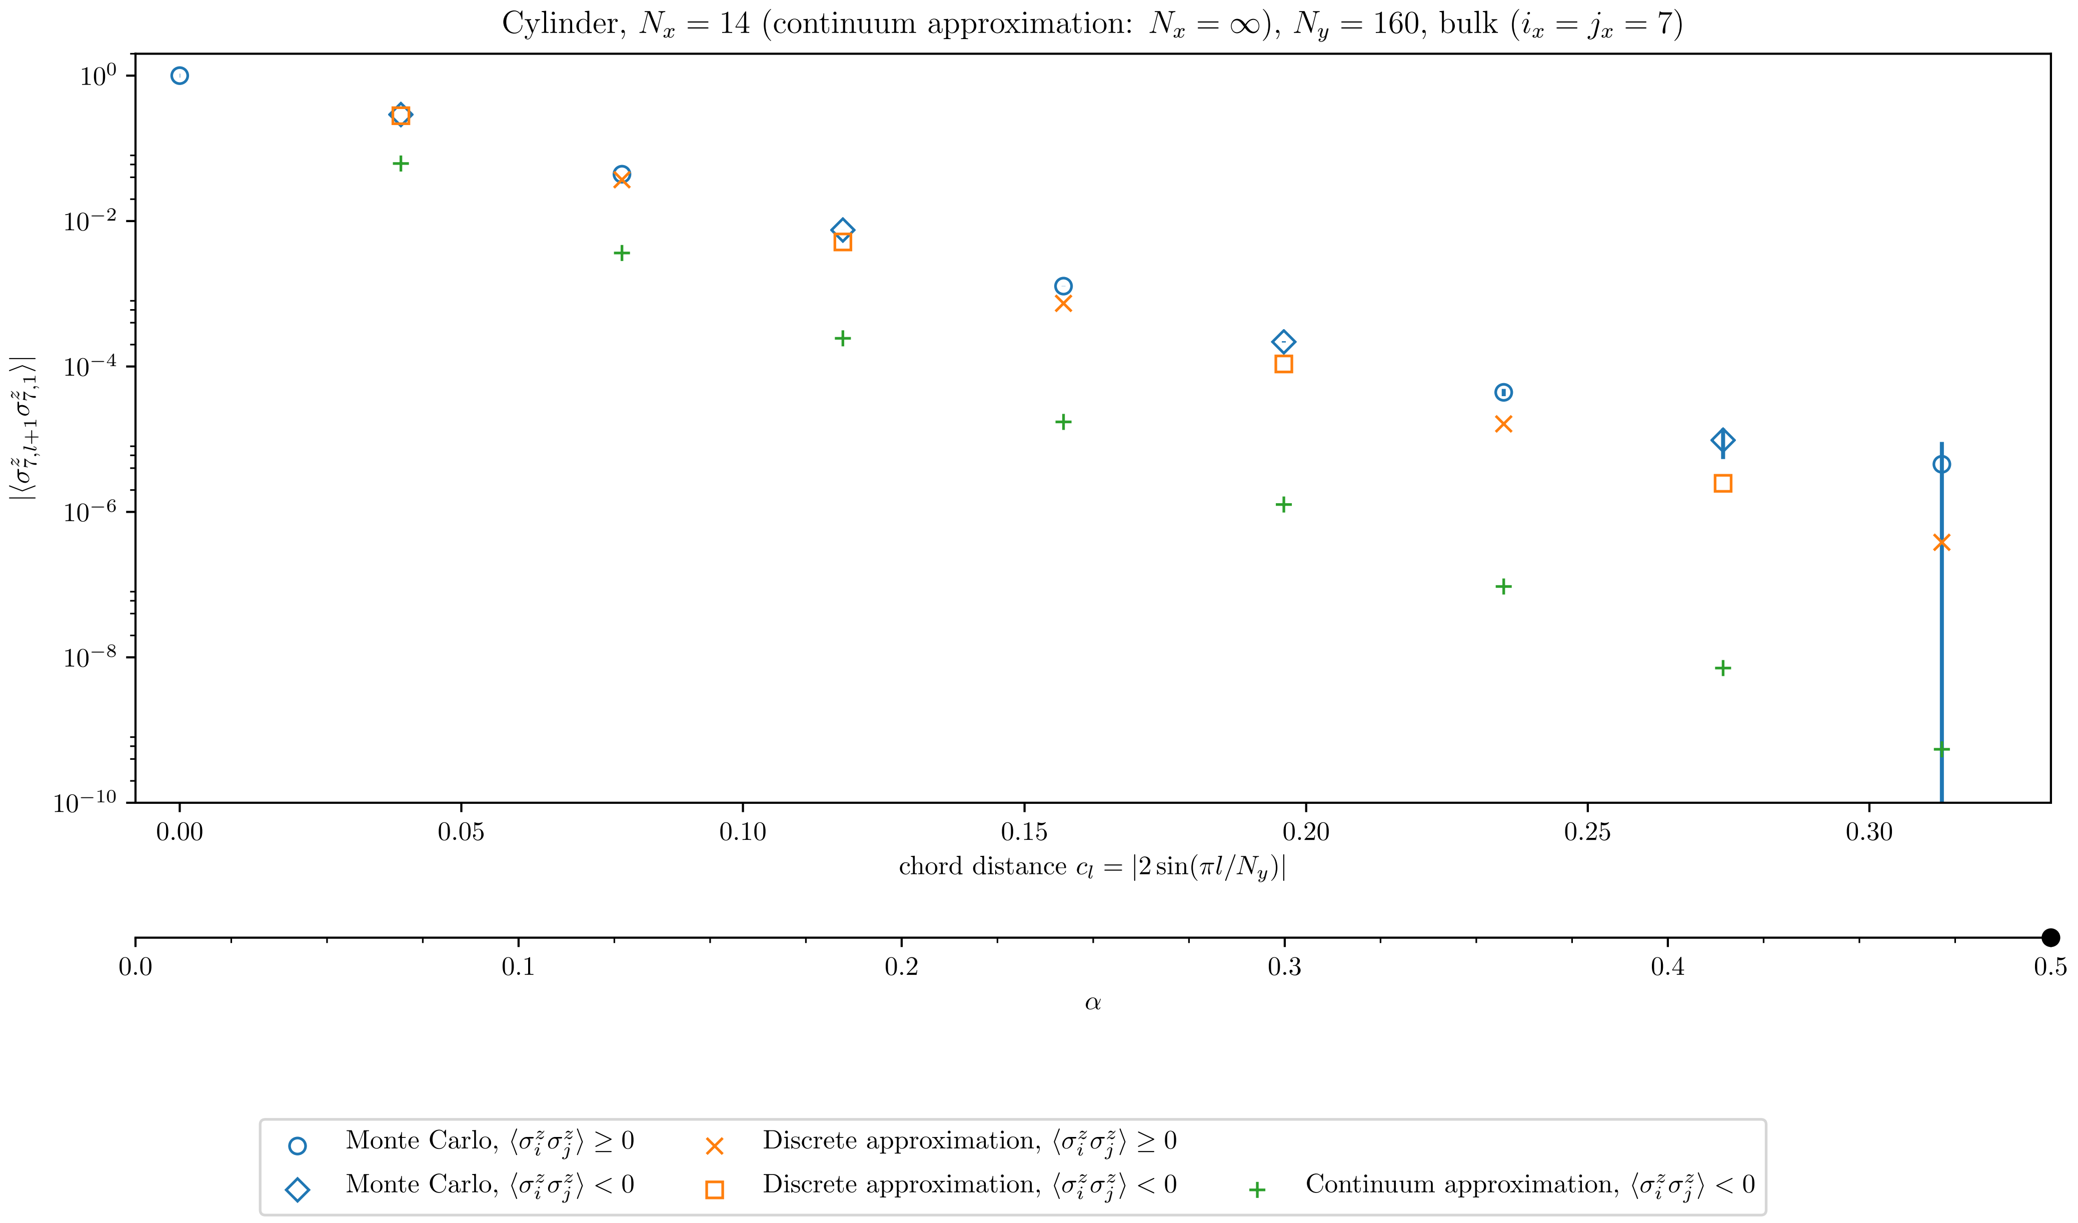

Cylinder, $N_x = 14$ (continuum approximation: $N_x = \infty$), $N_y = 160$, bulk ($i_x = j_x = 7$)
$|\langle\sigma^z_{7,l+1}\sigma^z_{7,1}\rangle|$
$10^0$
$10^{-2}$
$10^{-4}$
$10^{-6}$
$10^{-8}$
$10^{-10}$
0.00
0.05
0.10
0.15
0.20
0.25
0.30
chord distance $c_l = |2\sin(\pi l/N_y)|$
0.0
0.1
0.2
0.3
0.4
0.5
$\alpha$
Monte Carlo, $\langle\sigma^z_i\sigma^z_j\rangle \geq 0$
Monte Carlo, $\langle\sigma^z_i\sigma^z_j\rangle < 0$
Discrete approximation, $\langle\sigma^z_i\sigma^z_j\rangle \geq 0$
Discrete approximation, $\langle\sigma^z_i\sigma^z_j\rangle < 0$
Continuum approximation, $\langle\sigma^z_i\sigma^z_j\rangle < 0$
